# Supplementary material for: Model-independent comparison of simulation output
Source: arXiv:1509.09174 source file (2017-01-06)
Supplement: Supplementary file 1 [file supptables.pdf]

## Supplementary tables

| Comp. | Stat.          | Outputs          |                  |                  |                  |                  |                  |
|-------|----------------|------------------|------------------|------------------|------------------|------------------|------------------|
|       |                | $P^s$            | $P^w$            | $P^c$            | $\bar{E}^s$      | $\bar{E}^w$      | $\bar{C}$        |
| I     | max            | 0.151            | 0.620            | <u>0.016</u>     | <u>0.028</u>     | 0.343            | 0.138            |
|       | arg max        | 0.424            | 0.853            | <u>0.033</u>     | 0.106            | 0.264            | <u>0.005</u>     |
|       | min            | <u>0.007</u>     | 0.054            | 0.082            | <u>3e-5</u>      | 0.152            | <u>0.014</u>     |
|       | arg min        | 0.623            | 0.842            | <u>0.014</u>     | 1.000            | 0.168            | 0.140            |
|       | $\bar{X}^{ss}$ | 0.446            | 0.292            | 0.212            | 0.838            | 0.945            | 0.211            |
|       | $S^{ss}$       | 0.143            | 0.226            | 0.131            | 0.109            | 0.237            | 0.130            |
| II    | max            | 0.924            | <u>0.017</u>     | <u>4e-5</u>      | <u>4e-6</u>      | 0.250            | 0.974            |
|       | arg max        | <u>2e-4</u>      | 0.355            | 0.223            | <u>0.002</u>     | 0.147            | <u>4e-5</u>      |
|       | min            | <u>8e-5</u>      | <u>0.009</u>     | 0.830            | <u>2e-5</u>      | 0.025            | <u>6e-5</u>      |
|       | arg min        | <u>0.043</u>     | 0.544            | <u>0.001</u>     | 1.000            | 0.795            | 0.591            |
|       | $\bar{X}^{ss}$ | <u>0.005</u>     | <u>&lt; 1e-8</u> | 0.325            | <u>&lt; 1e-8</u> | 0.337            | 0.323            |
|       | $S^{ss}$       | <u>0.004</u>     | <u>0.007</u>     | <u>0.005</u>     | <u>0.005</u>     | 0.204            | <u>0.005</u>     |
| III   | max            | <u>&lt; 1e-8</u> | <u>&lt; 1e-8</u> | <u>2e-5</u>      | 0.029            | 0.303            | <u>&lt; 1e-8</u> |
|       | arg max        | <u>0.015</u>     | 0.652            | <u>&lt; 1e-8</u> | 0.876            | 0.399            | <u>2e-4</u>      |
|       | min            | <u>0.013</u>     | <u>6e-5</u>      | 0.463            | <u>0.001</u>     | 0.094            | <u>&lt; 1e-8</u> |
|       | arg min        | <u>0.042</u>     | 0.636            | <u>0.001</u>     | 1.000            | 0.378            | <u>&lt; 1e-8</u> |
|       | $\bar{X}^{ss}$ | <u>&lt; 1e-8</u> | <u>&lt; 1e-8</u> | <u>&lt; 1e-8</u> | <u>&lt; 1e-8</u> | <u>&lt; 1e-8</u> | <u>&lt; 1e-8</u> |
|       | $S^{ss}$       | <u>9e-8</u>      | <u>&lt; 1e-8</u> | <u>5e-6</u>      | <u>&lt; 1e-8</u> | <u>0.002</u>     | <u>0.003</u>     |

**Table S1.1**  $P$ -values for the empirical selection of FMs for model size 100, parameter set 1, and  $n = 30$  runs per configuration.  $P$ -values were obtained with the  $t$ -test for max, min,  $\bar{X}^{ss}$  and  $S^{ss}$  statistics, and with the Mann-Whitney U test for arg max and arg min statistics. Case I weights two similar configurations, case II compares configurations with a small implementation difference, and case III compares configurations with a different parameter. Values lower than 0.05 are underlined, while values lower than 0.01 are double-underlined.

| Comp. | Stat.               | Outputs          |                  |                  |                  |                  |                  |
|-------|---------------------|------------------|------------------|------------------|------------------|------------------|------------------|
|       |                     | $P^s$            | $P^w$            | $P^c$            | $\overline{E}^s$ | $\overline{E}^w$ | $\overline{C}$   |
| I     | max                 | 0.012            | 0.610            | 0.561            | 0.473            | 0.566            | 0.969            |
|       | arg max             | 0.792            | 0.085            | 0.273            | 0.602            | 0.292            | 0.050            |
|       | min                 | 0.429            | 0.065            | 0.156            | 0.015            | 0.550            | 0.546            |
|       | arg min             | 0.636            | 0.894            | 0.209            | 0.145            | 1.000            | 0.424            |
|       | $\overline{X}^{ss}$ | 0.675            | 0.926            | 0.960            | 0.970            | 0.594            | 0.973            |
|       | $S^{ss}$            | 0.615            | 0.776            | 0.781            | 0.898            | 0.789            | 0.782            |
| II    | max                 | <u>&lt; 1e-8</u> | <u>2e-6</u>      | <u>0.001</u>     | 0.087            | <u>1e-6</u>      | <u>9e-5</u>      |
|       | arg max             | <u>0.014</u>     | <u>0.047</u>     | 0.554            | 0.024            | 0.350            | 0.542            |
|       | min                 | <u>0.009</u>     | 0.630            | <u>8e-8</u>      | <u>&lt; 1e-8</u> | 0.898            | <u>0.001</u>     |
|       | arg min             | 0.112            | 0.542            | 0.096            | <u>9e-5</u>      | 0.392            | 0.492            |
|       | $\overline{X}^{ss}$ | <u>&lt; 1e-8</u> | <u>&lt; 1e-8</u> | <u>&lt; 1e-8</u> | <u>&lt; 1e-8</u> | <u>&lt; 1e-8</u> | <u>&lt; 1e-8</u> |
|       | $S^{ss}$            | 0.090            | 0.058            | 0.699            | 0.870            | <u>0.028</u>     | 0.706            |
| III   | max                 | <u>&lt; 1e-8</u> | <u>0.009</u>     | 0.040            | 0.175            | 0.155            | <u>&lt; 1e-8</u> |
|       | arg max             | 0.893            | 0.745            | 0.824            | 0.701            | 0.059            | 0.402            |
|       | min                 | 0.147            | 0.058            | 0.616            | 0.975            | 0.503            | <u>0.009</u>     |
|       | arg min             | 0.069            | 0.917            | 0.152            | 0.274            | 0.459            | 0.982            |
|       | $\overline{X}^{ss}$ | <u>5e-5</u>      | <u>&lt; 1e-8</u> | <u>&lt; 1e-8</u> | 0.762            | <u>&lt; 1e-8</u> | <u>&lt; 1e-8</u> |
|       | $S^{ss}$            | <u>0.010</u>     | <u>0.011</u>     | <u>0.026</u>     | <u>0.010</u>     | <u>0.037</u>     | 0.277            |

**Table S1.2**  $P$ -values for the empirical selection of FMs for model size 100, parameter set 2, and  $n = 30$  runs per configuration.  $P$ -values were obtained with the  $t$ -test for max, min,  $\overline{X}^{ss}$  and  $S^{ss}$  statistics, and with the Mann-Whitney U test for arg max and arg min statistics. Case I weights two similar configurations, case II compares configurations with a small implementation difference, and case III compares configurations with a different parameter. Values lower than 0.05 are underlined, while values lower than 0.01 are double-underlined.

| Comp. | Stat.               | Outputs          |                  |                  |                  |                  |                  |
|-------|---------------------|------------------|------------------|------------------|------------------|------------------|------------------|
|       |                     | $P^s$            | $P^w$            | $P^c$            | $\overline{E}^s$ | $\overline{E}^w$ | $\overline{C}$   |
| I     | max                 | 0.336            | 0.372            | 0.943            | 0.924            | 0.320            | 0.392            |
|       | arg max             | 0.524            | 0.267            | 1.000            | 0.625            | 1.000            | 0.917            |
|       | min                 | 0.821            | 0.069            | 0.322            | 0.081            | 0.268            | 0.986            |
|       | arg min             | 0.391            | 0.641            | 0.894            | 1.000            | 0.111            | 0.654            |
|       | $\overline{X}^{ss}$ | 0.383            | 0.924            | 0.339            | 0.252            | 0.075            | 0.336            |
|       | $S^{ss}$            | 0.173            | 0.408            | 0.162            | 0.879            | 0.540            | 0.162            |
| II    | max                 | <u>0.003</u>     | <u>2e-7</u>      | 0.349            | <u>6e-7</u>      | 0.236            | <u>0.013</u>     |
|       | arg max             | <u>0.003</u>     | 0.446            | 0.764            | <u>0.005</u>     | 0.464            | 0.073            |
|       | min                 | 0.274            | 0.870            | <u>0.007</u>     | <u>3e-4</u>      | 0.907            | 0.258            |
|       | arg min             | 0.197            | 0.906            | 0.060            | 1.000            | 0.853            | 0.654            |
|       | $\overline{X}^{ss}$ | 0.617            | <u>&lt; 1e-8</u> | <u>0.001</u>     | <u>&lt; 1e-8</u> | 0.788            | <u>0.001</u>     |
|       | $S^{ss}$            | 0.090            | 0.078            | 0.124            | <u>0.029</u>     | 0.646            | 0.123            |
| III   | max                 | <u>&lt; 1e-8</u> | <u>&lt; 1e-8</u> | <u>&lt; 1e-8</u> | <u>&lt; 1e-8</u> | <u>5e-4</u>      | <u>&lt; 1e-8</u> |
|       | arg max             | 0.095            | 0.912            | <u>&lt; 1e-8</u> | 0.640            | 0.982            | <u>0.005</u>     |
|       | min                 | 0.155            | <u>0.004</u>     | <u>3e-6</u>      | <u>0.021</u>     | 0.908            | <u>&lt; 1e-8</u> |
|       | arg min             | <u>0.034</u>     | 0.111            | <u>0.005</u>     | 1.000            | 0.864            | <u>&lt; 1e-8</u> |
|       | $\overline{X}^{ss}$ | <u>&lt; 1e-8</u> | <u>&lt; 1e-8</u> | <u>&lt; 1e-8</u> | <u>&lt; 1e-8</u> | <u>&lt; 1e-8</u> | <u>&lt; 1e-8</u> |
|       | $S^{ss}$            | <u>1e-8</u>      | <u>&lt; 1e-8</u> | <u>9e-7</u>      | <u>6e-8</u>      | <u>1e-5</u>      | <u>0.001</u>     |

**Table S1.3**  $P$ -values for the empirical selection of FMs for model size 200, parameter set 1, and  $n = 30$  runs per configuration.  $P$ -values were obtained with the  $t$ -test for max, min,  $\overline{X}^{ss}$  and  $S^{ss}$  statistics, and with the Mann-Whitney U test for arg max and arg min statistics. Case I weights two similar configurations, case II compares configurations with a small implementation difference, and case III compares configurations with a different parameter. Values lower than 0.05 are underlined, while values lower than 0.01 are double-underlined.

| Comp. | Stat.               | Outputs          |                  |                  |                  |                  |                  |
|-------|---------------------|------------------|------------------|------------------|------------------|------------------|------------------|
|       |                     | $P^s$            | $P^w$            | $P^c$            | $\overline{E}^s$ | $\overline{E}^w$ | $\overline{C}$   |
| I     | max                 | 0.499            | 0.992            | 0.578            | <u>3e-4</u>      | 0.819            | 0.815            |
|       | arg max             | 0.068            | 0.354            | 0.911            | <u>0.387</u>     | 0.738            | 0.472            |
|       | min                 | 0.132            | 0.602            | 0.796            | 0.387            | 0.314            | 0.575            |
|       | arg min             | 0.157            | 0.777            | 0.869            | 0.643            | 0.461            | 0.749            |
|       | $\overline{X}^{ss}$ | 0.448            | 0.318            | 0.475            | <u>0.041</u>     | 0.139            | 0.472            |
|       | $S^{ss}$            | 0.543            | 0.754            | 0.672            | 0.481            | 0.987            | 0.670            |
| II    | max                 | <u>&lt; 1e-8</u> | <u>&lt; 1e-8</u> | <u>9e-6</u>      | <u>0.001</u>     | <u>&lt; 1e-8</u> | <u>&lt; 1e-8</u> |
|       | arg max             | <u>2e-8</u>      | 0.784            | <u>1e-4</u>      | 0.267            | 0.598            | 0.256            |
|       | min                 | <u>0.036</u>     | 0.855            | <u>&lt; 1e-8</u> | <u>&lt; 1e-8</u> | 0.886            | <u>1e-5</u>      |
|       | arg min             | 0.061            | 0.497            | 0.887            | <u>&lt; 1e-8</u> | 0.068            | <u>8e-5</u>      |
|       | $\overline{X}^{ss}$ | <u>&lt; 1e-8</u> | <u>&lt; 1e-8</u> | <u>&lt; 1e-8</u> | <u>&lt; 1e-8</u> | <u>&lt; 1e-8</u> | <u>&lt; 1e-8</u> |
|       | $S^{ss}$            | 0.093            | 0.135            | 0.797            | 0.219            | 0.099            | 0.804            |
| III   | max                 | <u>&lt; 1e-8</u> | <u>1e-8</u>      | <u>3e-5</u>      | <u>3e-6</u>      | <u>4e-5</u>      | <u>&lt; 1e-8</u> |
|       | arg max             | 0.246            | 0.667            | 0.079            | 0.164            | 0.431            | <u>1e-6</u>      |
|       | min                 | <u>0.041</u>     | 0.132            | <u>0.001</u>     | 0.652            | 0.980            | <u>2e-6</u>      |
|       | arg min             | 0.118            | <u>0.011</u>     | 0.398            | <u>0.001</u>     | 0.366            | 0.109            |
|       | $\overline{X}^{ss}$ | <u>&lt; 1e-8</u> | <u>&lt; 1e-8</u> | <u>&lt; 1e-8</u> | <u>0.001</u>     | <u>&lt; 1e-8</u> | <u>&lt; 1e-8</u> |
|       | $S^{ss}$            | 0.271            | 0.417            | 0.723            | 0.804            | 0.421            | 0.605            |

**Table S1.4**  $P$ -values for the empirical selection of FMs for model size 200, parameter set 2, and  $n = 30$  runs per configuration.  $P$ -values were obtained with the  $t$ -test for max, min,  $\overline{X}^{ss}$  and  $S^{ss}$  statistics, and with the Mann-Whitney U test for arg max and arg min statistics. Case I weights two similar configurations, case II compares configurations with a small implementation difference, and case III compares configurations with a different parameter. Values lower than 0.05 are underlined, while values lower than 0.01 are double-underlined.

| Comp. | Stat.          | Outputs          |                  |                  |                  |                  |                  |
|-------|----------------|------------------|------------------|------------------|------------------|------------------|------------------|
|       |                | $P^s$            | $P^w$            | $P^c$            | $\bar{E}^s$      | $\bar{E}^w$      | $\bar{C}$        |
| I     | max            | 0.213            | 0.288            | <u>0.011</u>     | 0.231            | 0.774            | 0.086            |
|       | arg max        | 0.733            | 0.802            | <u>0.056</u>     | 0.858            | 0.284            | 0.279            |
|       | min            | <u>0.002</u>     | 0.088            | 0.094            | 0.275            | 0.076            | <u>0.011</u>     |
|       | arg min        | <u>0.048</u>     | 0.350            | 0.279            | 1.000            | 0.091            | 1.000            |
|       | $\bar{X}^{ss}$ | 0.457            | 0.905            | 0.546            | 0.833            | <u>0.049</u>     | 0.551            |
|       | $S^{ss}$       | 0.242            | 0.282            | 0.285            | 0.474            | 0.109            | 0.285            |
| II    | max            | <u>7e-6</u>      | <u>1e-7</u>      | <u>2e-4</u>      | <u>2e-7</u>      | 0.322            | <u>0.004</u>     |
|       | arg max        | <u>1e-4</u>      | 0.540            | 0.230            | 0.703            | 0.052            | <u>1e-4</u>      |
|       | min            | <u>1e-5</u>      | <u>4e-4</u>      | <u>0.009</u>     | 0.508            | <u>0.017</u>     | <u>0.001</u>     |
|       | arg min        | 0.712            | 0.906            | <u>0.001</u>     | 1.000            | <u>0.009</u>     | 1.000            |
|       | $\bar{X}^{ss}$ | 0.206            | <u>&lt; 1e-8</u> | <u>6e-8</u>      | <u>&lt; 1e-8</u> | 0.938            | <u>6e-8</u>      |
|       | $S^{ss}$       | 0.735            | 0.324            | 0.712            | 0.218            | 0.688            | 0.713            |
| III   | max            | <u>&lt; 1e-8</u> | <u>&lt; 1e-8</u> | <u>&lt; 1e-8</u> | <u>&lt; 1e-8</u> | <u>&lt; 1e-8</u> | <u>&lt; 1e-8</u> |
|       | arg max        | <u>2e-5</u>      | 0.115            | <u>&lt; 1e-8</u> | 0.134            | 0.332            | <u>1e-5</u>      |
|       | min            | <u>7e-8</u>      | <u>&lt; 1e-8</u> | <u>&lt; 1e-8</u> | 0.582            | <u>0.003</u>     | <u>&lt; 1e-8</u> |
|       | arg min        | <u>2e-5</u>      | 0.070            | <u>2e-5</u>      | 1.000            | <u>0.004</u>     | <u>&lt; 1e-8</u> |
|       | $\bar{X}^{ss}$ | <u>&lt; 1e-8</u> | <u>&lt; 1e-8</u> | <u>&lt; 1e-8</u> | <u>&lt; 1e-8</u> | <u>&lt; 1e-8</u> | <u>&lt; 1e-8</u> |
|       | $S^{ss}$       | <u>3e-7</u>      | <u>7e-8</u>      | <u>5e-5</u>      | <u>4e-8</u>      | 0.013            | 0.013            |

**Table S1.5**  $P$ -values for the empirical selection of FMs for model size 400, parameter set 1, and  $n = 30$  runs per configuration.  $P$ -values were obtained with the  $t$ -test for max, min,  $\bar{X}^{ss}$  and  $S^{ss}$  statistics, and with the Mann-Whitney U test for arg max and arg min statistics. Case I weights two similar configurations, case II compares configurations with a small implementation difference, and case III compares configurations with a different parameter. Values lower than 0.05 are underlined, while values lower than 0.01 are double-underlined.

| Comp. | Stat.               | Outputs          |                  |                  |                  |                  |                  |
|-------|---------------------|------------------|------------------|------------------|------------------|------------------|------------------|
|       |                     | $P^s$            | $P^w$            | $P^c$            | $\overline{E}^s$ | $\overline{E}^w$ | $\overline{C}$   |
| I     | max                 | 0.840            | 0.982            | 0.933            | 0.552            | 0.132            | 0.878            |
|       | arg max             | 0.742            | 0.509            | 0.887            | 0.689            | 0.126            | 0.098            |
|       | min                 | 0.255            | 0.944            | 0.289            | 0.509            | 0.138            | 0.956            |
|       | arg min             | 0.161            | 0.473            | 0.081            | 0.132            | <u>0.004</u>     | 0.470            |
|       | $\overline{X}^{ss}$ | 0.528            | 0.469            | 0.379            | 0.326            | 0.786            | 0.362            |
|       | $S^{ss}$            | 0.631            | 0.634            | 0.685            | 0.669            | 0.657            | 0.684            |
| II    | max                 | <u>&lt; 1e-8</u> | <u>&lt; 1e-8</u> | <u>&lt; 1e-8</u> | 0.169            | <u>&lt; 1e-8</u> | <u>&lt; 1e-8</u> |
|       | arg max             | <u>&lt; 1e-8</u> | 0.423            | <u>&lt; 1e-8</u> | 0.649            | 0.161            | 0.207            |
|       | min                 | <u>0.019</u>     | 0.173            | <u>&lt; 1e-8</u> | <u>&lt; 1e-8</u> | 0.056            | <u>&lt; 1e-8</u> |
|       | arg min             | <u>0.006</u>     | 0.091            | 0.988            | <u>&lt; 1e-8</u> | 0.055            | <u>&lt; 1e-8</u> |
|       | $\overline{X}^{ss}$ | <u>&lt; 1e-8</u> | <u>&lt; 1e-8</u> | <u>&lt; 1e-8</u> | <u>&lt; 1e-8</u> | <u>&lt; 1e-8</u> | <u>&lt; 1e-8</u> |
|       | $S^{ss}$            | 0.135            | 0.289            | 0.871            | 0.245            | 0.258            | 0.870            |
| III   | max                 | <u>&lt; 1e-8</u> | <u>&lt; 1e-8</u> | <u>&lt; 1e-8</u> | <u>&lt; 1e-8</u> | <u>&lt; 1e-8</u> | <u>&lt; 1e-8</u> |
|       | arg max             | <u>0.035</u>     | 0.315            | <u>2e-6</u>      | 0.100            | <u>0.001</u>     | <u>1e-7</u>      |
|       | min                 | <u>0.038</u>     | 0.236            | <u>&lt; 1e-8</u> | 0.997            | 0.488            | <u>&lt; 1e-8</u> |
|       | arg min             | <u>0.022</u>     | 0.442            | <u>0.020</u>     | <u>0.001</u>     | 0.190            | <u>1e-6</u>      |
|       | $\overline{X}^{ss}$ | <u>&lt; 1e-8</u> | <u>&lt; 1e-8</u> | <u>&lt; 1e-8</u> | <u>2e-6</u>      | <u>&lt; 1e-8</u> | <u>&lt; 1e-8</u> |
|       | $S^{ss}$            | 0.164            | 0.110            | <u>0.043</u>     | <u>0.027</u>     | 0.135            | <u>0.006</u>     |

**Table S1.6**  $P$ -values for the empirical selection of FMs for model size 400, parameter set 2, and  $n = 30$  runs per configuration.  $P$ -values were obtained with the  $t$ -test for max, min,  $\overline{X}^{ss}$  and  $S^{ss}$  statistics, and with the Mann-Whitney U test for arg max and arg min statistics. Case I weights two similar configurations, case II compares configurations with a small implementation difference, and case III compares configurations with a different parameter. Values lower than 0.05 are underlined, while values lower than 0.01 are double-underlined.

| Comp. | Stat.               | Outputs          |                  |                  |                  |                  |                  |
|-------|---------------------|------------------|------------------|------------------|------------------|------------------|------------------|
|       |                     | $P^s$            | $P^w$            | $P^c$            | $\overline{E}^s$ | $\overline{E}^w$ | $\overline{C}$   |
| I     | max                 | 0.371            | 0.729            | <u>0.001</u>     | 0.300            | 0.834            | 0.125            |
|       | arg max             | 1.000            | 0.813            | 1.000            | 0.406            | 0.407            | 0.618            |
|       | min                 | 0.047            | 0.434            | 0.177            | <u>0.042</u>     | 0.789            | <u>0.016</u>     |
|       | arg min             | <u>0.001</u>     | 0.448            | 0.463            | 1.000            | 0.945            | 1.000            |
|       | $\overline{X}^{ss}$ | 0.782            | 0.075            | 0.820            | <u>0.041</u>     | 0.080            | 0.818            |
|       | $S^{ss}$            | 0.111            | 0.116            | 0.161            | 0.131            | 0.434            | 0.159            |
| II    | max                 | <u>&lt; 1e-8</u> | <u>&lt; 1e-8</u> | <u>&lt; 1e-8</u> | <u>&lt; 1e-8</u> | 0.168            | <u>3e-8</u>      |
|       | arg max             | <u>&lt; 1e-8</u> | 0.947            | 1.000            | 0.464            | 0.143            | <u>9e-5</u>      |
|       | min                 | <u>4e-6</u>      | <u>6e-8</u>      | <u>3e-8</u>      | <u>0.045</u>     | 0.348            | <u>&lt; 1e-8</u> |
|       | arg min             | 0.094            | <u>0.001</u>     | <u>2e-6</u>      | 1.000            | 0.916            | 1.000            |
|       | $\overline{X}^{ss}$ | <u>0.005</u>     | <u>&lt; 1e-8</u> | <u>&lt; 1e-8</u> | <u>&lt; 1e-8</u> | 0.018            | <u>&lt; 1e-8</u> |
|       | $S^{ss}$            | 0.580            | 0.398            | 0.553            | 0.431            | 0.593            | 0.552            |
| III   | max                 | <u>&lt; 1e-8</u> | <u>&lt; 1e-8</u> | <u>&lt; 1e-8</u> | <u>&lt; 1e-8</u> | <u>&lt; 1e-8</u> | <u>&lt; 1e-8</u> |
|       | arg max             | <u>1e-8</u>      | <u>&lt; 1e-8</u> | <u>&lt; 1e-8</u> | 0.647            | 0.145            | <u>&lt; 1e-8</u> |
|       | min                 | <u>&lt; 1e-8</u> | <u>&lt; 1e-8</u> | <u>&lt; 1e-8</u> | 0.063            | <u>0.001</u>     | <u>&lt; 1e-8</u> |
|       | arg min             | <u>1e-4</u>      | <u>6e-7</u>      | <u>&lt; 1e-8</u> | 1.000            | 0.456            | <u>&lt; 1e-8</u> |
|       | $\overline{X}^{ss}$ | <u>&lt; 1e-8</u> | <u>&lt; 1e-8</u> | <u>&lt; 1e-8</u> | <u>&lt; 1e-8</u> | <u>&lt; 1e-8</u> | <u>&lt; 1e-8</u> |
|       | $S^{ss}$            | <u>1e-5</u>      | <u>2e-6</u>      | <u>0.001</u>     | <u>4e-6</u>      | 0.049            | 0.188            |

**Table S1.7**  $P$ -values for the empirical selection of FMs for model size 800, parameter set 1, and  $n = 30$  runs per configuration.  $P$ -values were obtained with the  $t$ -test for max, min,  $\overline{X}^{ss}$  and  $S^{ss}$  statistics, and with the Mann-Whitney U test for arg max and arg min statistics. Case I weights two similar configurations, case II compares configurations with a small implementation difference, and case III compares configurations with a different parameter. Values lower than 0.05 are underlined, while values lower than 0.01 are double-underlined.



| Comp. | Stat.               | Outputs          |                  |                  |                  |                  |                  |
|-------|---------------------|------------------|------------------|------------------|------------------|------------------|------------------|
|       |                     | $P^s$            | $P^w$            | $P^c$            | $\overline{E}^s$ | $\overline{E}^w$ | $\overline{C}$   |
| I     | max                 | 0.913            | <u>0.018</u>     | 0.178            | 0.444            | 0.347            | 0.194            |
|       | arg max             | 1.000            | <u>0.203</u>     | 0.774            | 1.000            | 0.068            | 0.510            |
|       | min                 | 1.000            | <u>0.024</u>     | 0.728            | <u>8e-6</u>      | 0.053            | 0.182            |
|       | arg min             | 1.000            | <u>0.047</u>     | 0.876            | <u>0.974</u>     | 0.954            | 0.397            |
|       | $\overline{X}^{ss}$ | 0.638            | <u>0.515</u>     | <u>0.028</u>     | 0.136            | 0.261            | <u>0.029</u>     |
|       | $S^{ss}$            | 0.718            | 0.609            | <u>0.639</u>     | 0.696            | 0.646            | <u>0.642</u>     |
| II    | max                 | <u>&lt; 1e-8</u> | <u>&lt; 1e-8</u> | <u>&lt; 1e-8</u> | 0.379            | <u>&lt; 1e-8</u> | <u>&lt; 1e-8</u> |
|       | arg max             | <u>&lt; 1e-8</u> | <u>0.006</u>     | <u>&lt; 1e-8</u> | <u>0.002</u>     | 0.065            | 0.249            |
|       | min                 | 0.108            | <u>1e-5</u>      | <u>&lt; 1e-8</u> | <u>&lt; 1e-8</u> | <u>0.001</u>     | <u>&lt; 1e-8</u> |
|       | arg min             | <u>0.042</u>     | <u>0.007</u>     | <u>0.006</u>     | <u>&lt; 1e-8</u> | 0.081            | <u>&lt; 1e-8</u> |
|       | $\overline{X}^{ss}$ | <u>&lt; 1e-8</u> | <u>&lt; 1e-8</u> | <u>&lt; 1e-8</u> | <u>&lt; 1e-8</u> | <u>&lt; 1e-8</u> | <u>&lt; 1e-8</u> |
|       | $S^{ss}$            | 0.619            | 0.773            | 0.469            | <u>0.022</u>     | 0.977            | 0.476            |
| III   | max                 | <u>&lt; 1e-8</u> | <u>&lt; 1e-8</u> | <u>&lt; 1e-8</u> | <u>&lt; 1e-8</u> | <u>&lt; 1e-8</u> | <u>&lt; 1e-8</u> |
|       | arg max             | <u>2e-5</u>      | <u>0.012</u>     | <u>&lt; 1e-8</u> | <u>0.001</u>     | 1.000            | <u>&lt; 1e-8</u> |
|       | min                 | 1.000            | 0.911            | <u>&lt; 1e-8</u> | 0.178            | 0.104            | <u>&lt; 1e-8</u> |
|       | arg min             | 1.000            | 0.239            | 0.605            | <u>2e-4</u>      | 0.132            | <u>&lt; 1e-8</u> |
|       | $\overline{X}^{ss}$ | <u>&lt; 1e-8</u> | <u>&lt; 1e-8</u> | <u>&lt; 1e-8</u> | <u>&lt; 1e-8</u> | <u>&lt; 1e-8</u> | <u>&lt; 1e-8</u> |
|       | $S^{ss}$            | 0.775            | 0.783            | 0.337            | 0.317            | 0.924            | 0.084            |

**Table S1.8**  $P$ -values for the empirical selection of FMs for model size 800, parameter set 2, and  $n = 30$  runs per configuration.  $P$ -values were obtained with the  $t$ -test for max, min,  $\overline{X}^{ss}$  and  $S^{ss}$  statistics, and with the Mann-Whitney U test for arg max and arg min statistics. Case I weights two similar configurations, case II compares configurations with a small implementation difference, and case III compares configurations with a different parameter. Values lower than 0.05 are underlined, while values lower than 0.01 are double-underlined.

| Comp. | Data      | Outputs                                                                           |                                                                                   |                                                                                   |                                                                                   |                                                                                    |                                                                                     |                                                                                     |
|-------|-----------|-----------------------------------------------------------------------------------|-----------------------------------------------------------------------------------|-----------------------------------------------------------------------------------|-----------------------------------------------------------------------------------|------------------------------------------------------------------------------------|-------------------------------------------------------------------------------------|-------------------------------------------------------------------------------------|
|       |           | $P^s$                                                                             | $P^w$                                                                             | $P^c$                                                                             | $\overline{E}^s$                                                                  | $\overline{E}^w$                                                                   | $\overline{C}$                                                                      | $\tilde{A}$                                                                         |
| I     | #PCs      | 26                                                                                | 32                                                                                | 26                                                                                | 37                                                                                | 43                                                                                 | 27                                                                                  | 38                                                                                  |
|       | MNV       | 0.852                                                                             | 0.509                                                                             | 0.851                                                                             | 0.966                                                                             | 0.285                                                                              | 0.879                                                                               | 0.486                                                                               |
|       | $t$ -test | <u>0.036</u>                                                                      | <u>0.057</u>                                                                      | <u>0.049</u>                                                                      | <u>0.023</u>                                                                      | 0.503                                                                              | <u>0.049</u>                                                                        | 0.077                                                                               |
|       | PCS       | 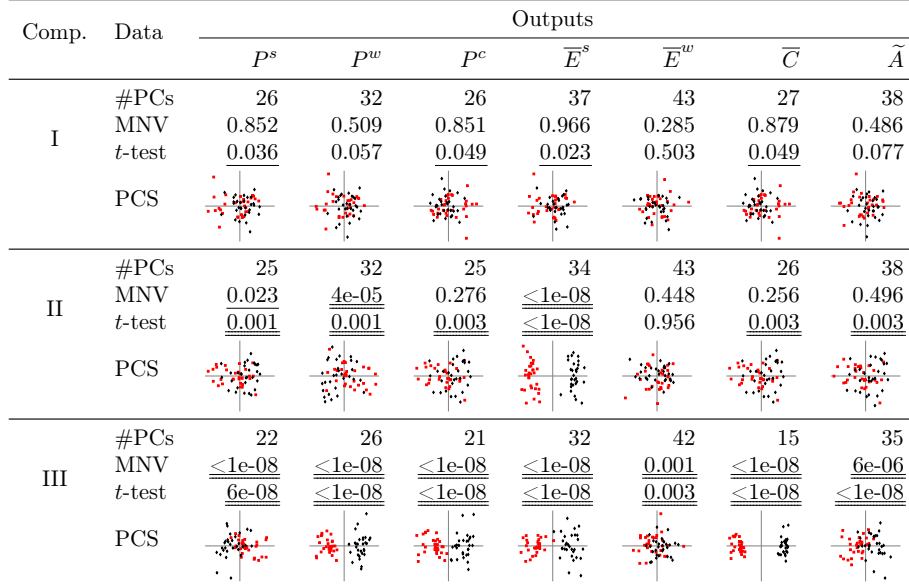 | 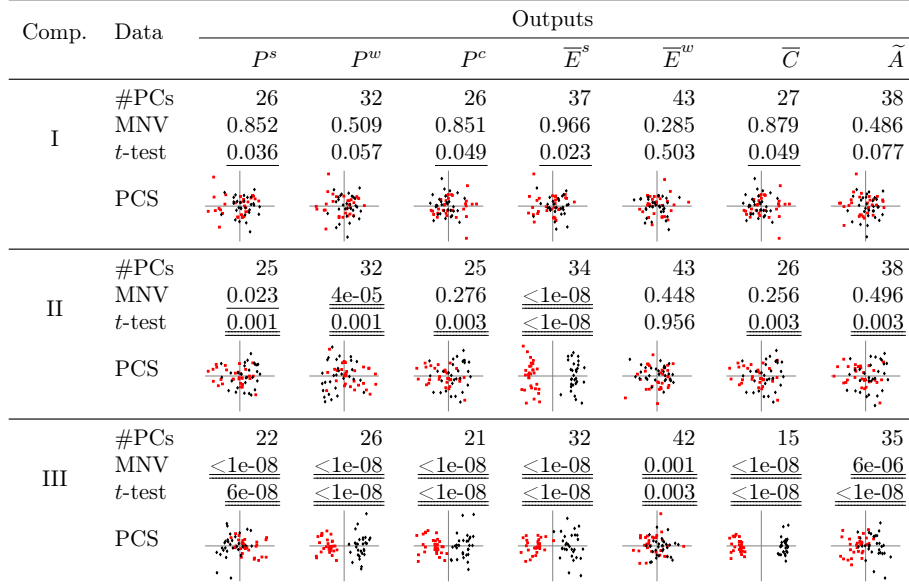 | 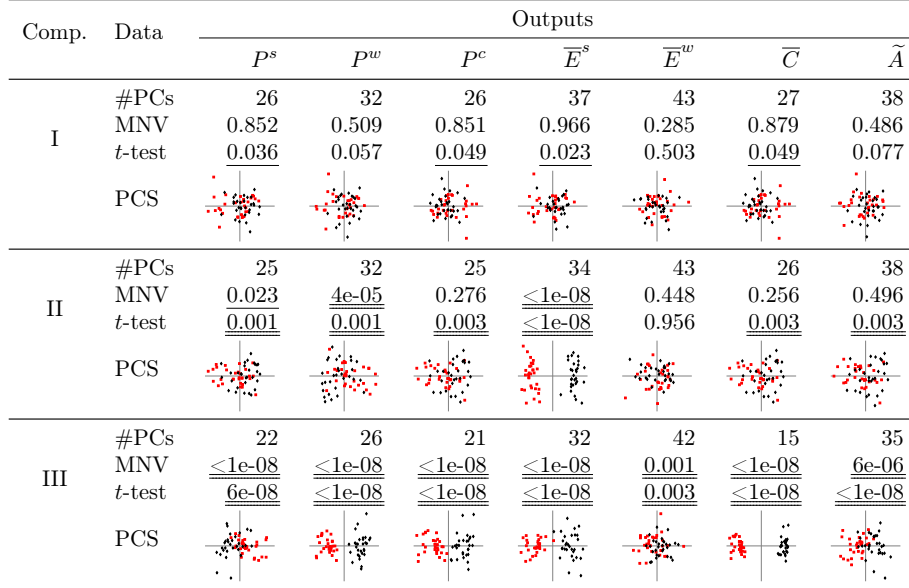 | 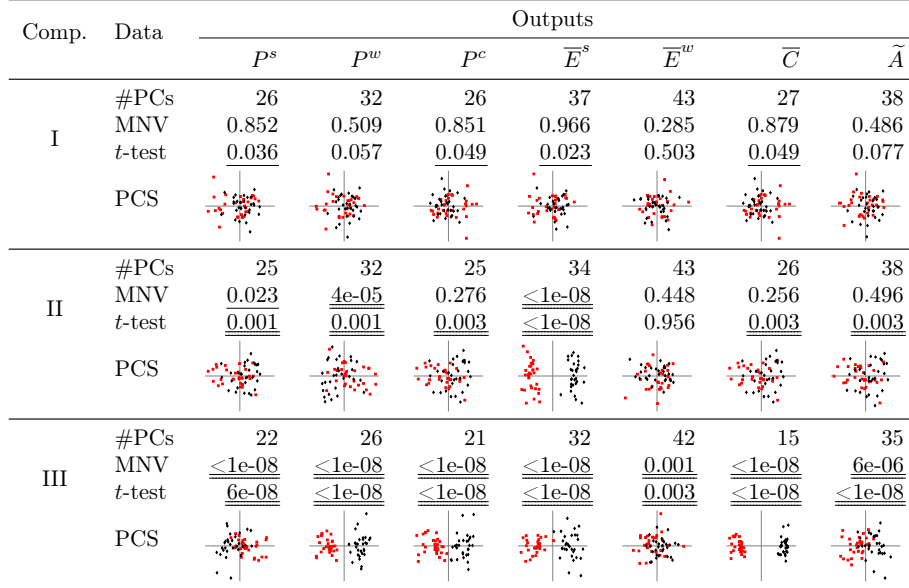 | 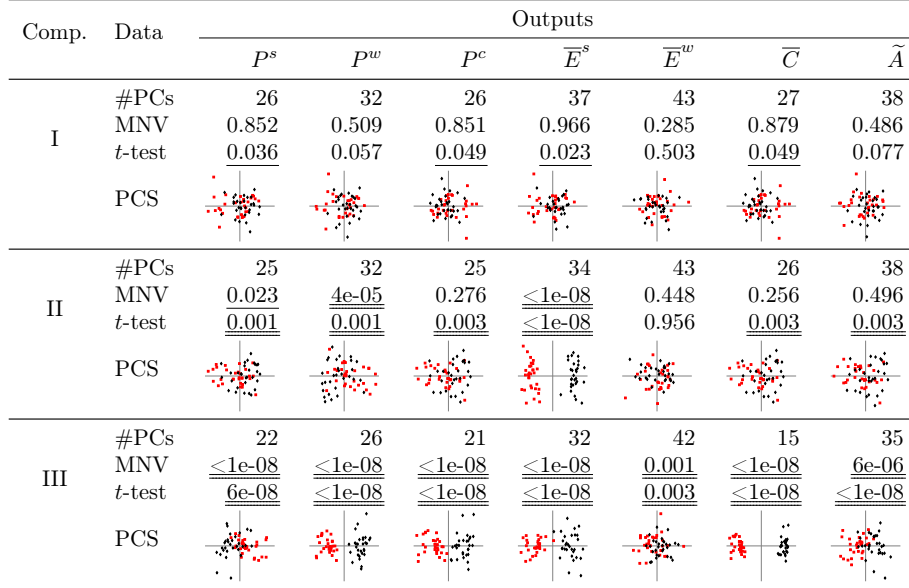 | 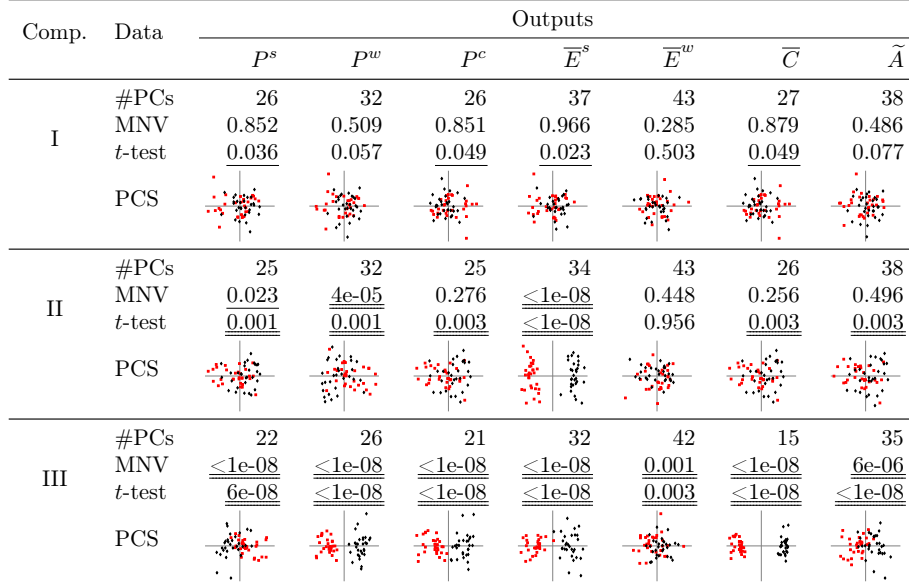 | 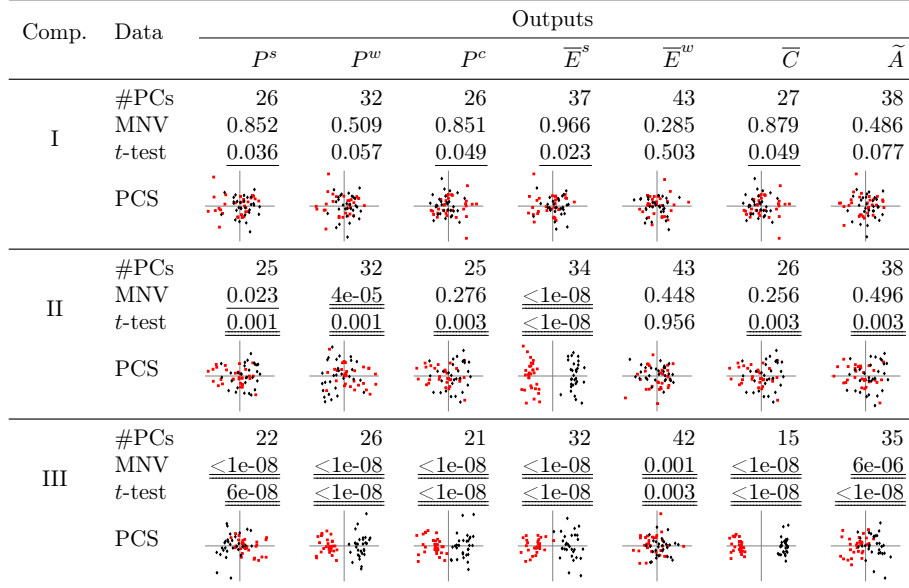 |
| II    | #PCs      | 25                                                                                | 32                                                                                | 25                                                                                | 34                                                                                | 43                                                                                 | 26                                                                                  | 38                                                                                  |
|       | MNV       | <u>0.023</u>                                                                      | <u>4e-05</u>                                                                      | 0.276                                                                             | <u>&lt;1e-08</u>                                                                  | 0.448                                                                              | 0.256                                                                               | 0.496                                                                               |
|       | $t$ -test | <u>0.001</u>                                                                      | <u>0.001</u>                                                                      | <u>0.003</u>                                                                      | <u>&lt;1e-08</u>                                                                  | 0.956                                                                              | <u>0.003</u>                                                                        | <u>0.003</u>                                                                        |
|       | PCS       | 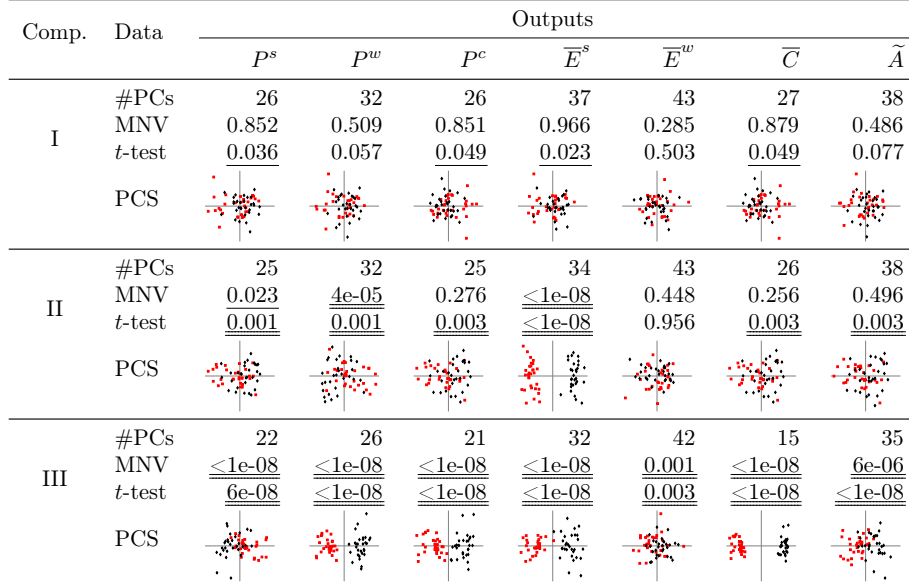 | 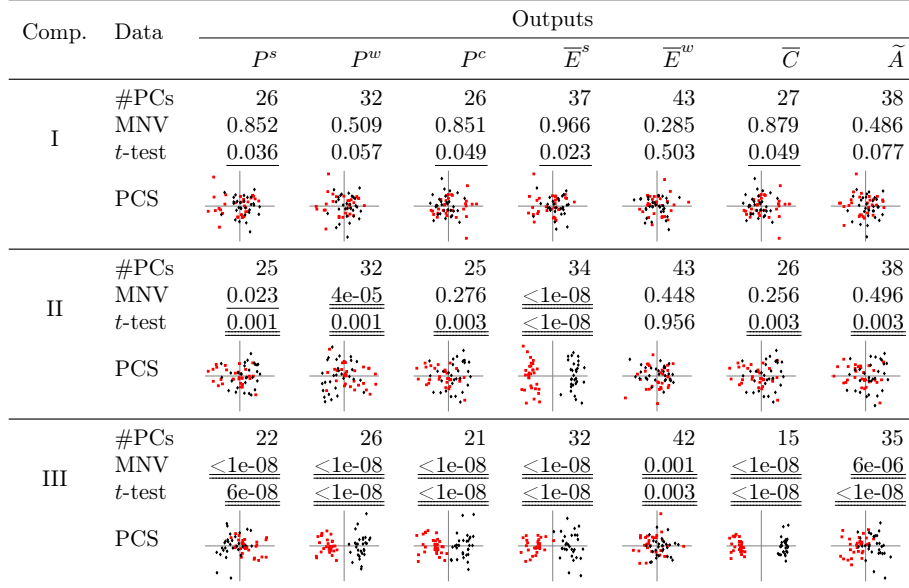 | 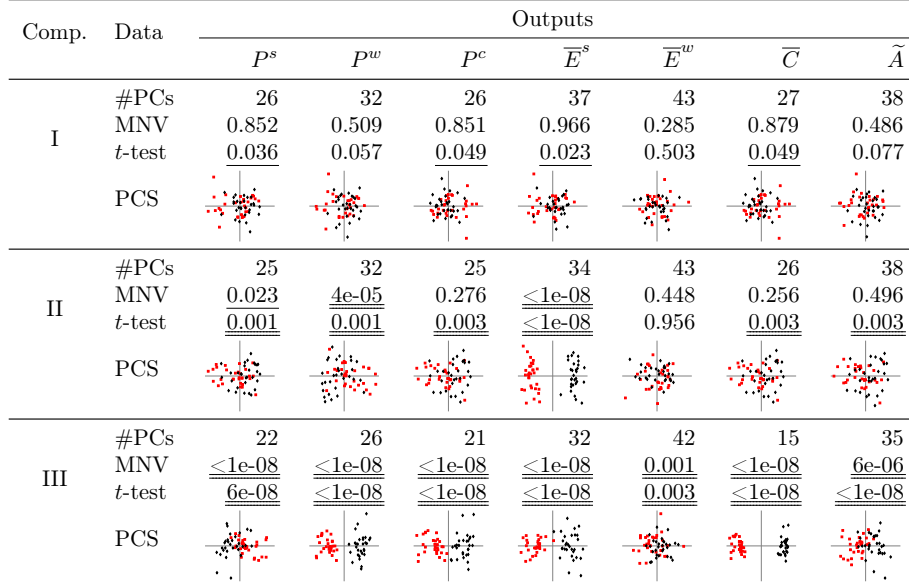 | 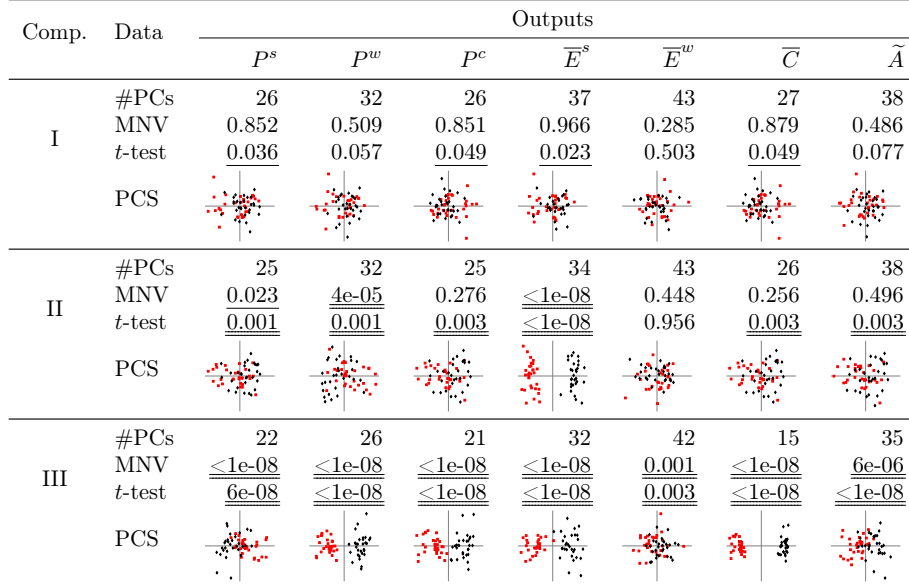 | 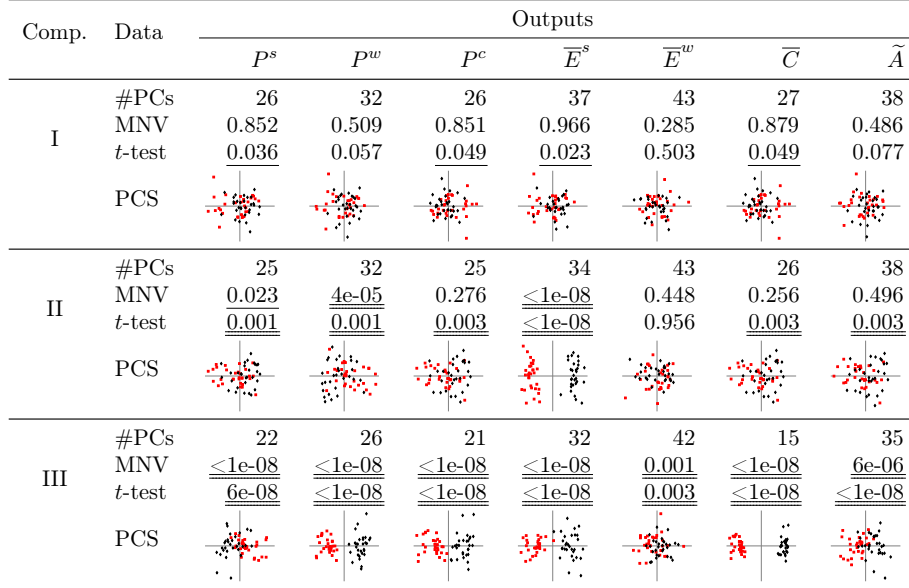 | 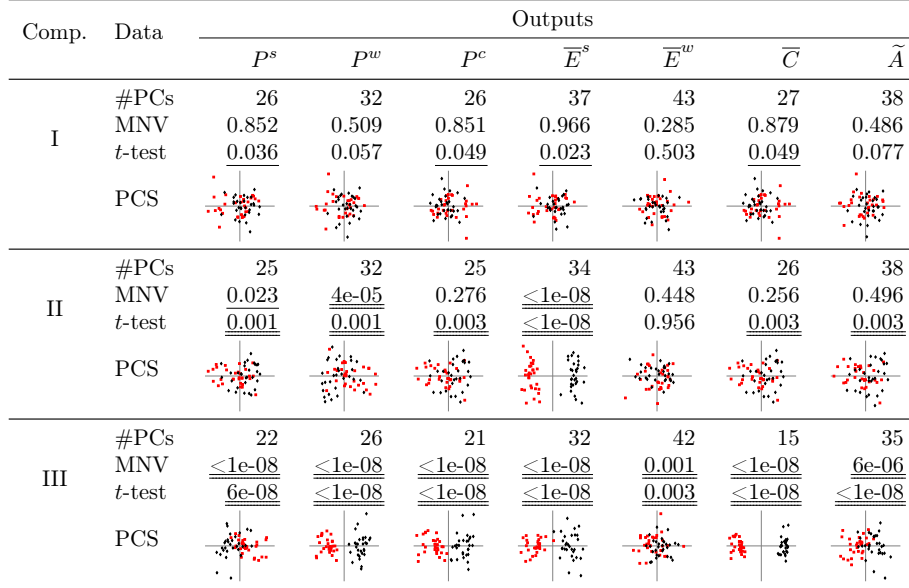 | 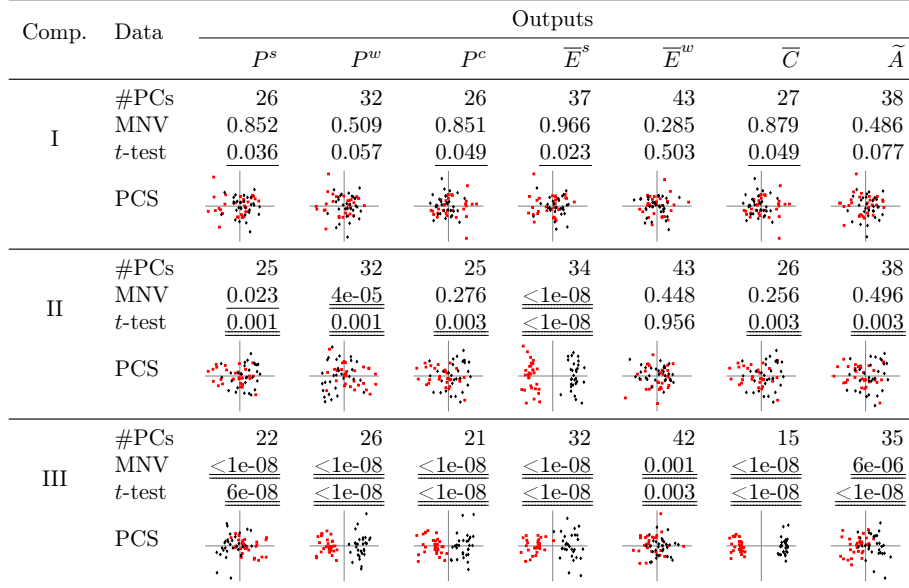 |
| III   | #PCs      | 22                                                                                | 26                                                                                | 21                                                                                | 32                                                                                | 42                                                                                 | 15                                                                                  | 35                                                                                  |
|       | MNV       | <u>&lt;1e-08</u>                                                                  | <u>&lt;1e-08</u>                                                                  | <u>&lt;1e-08</u>                                                                  | <u>&lt;1e-08</u>                                                                  | <u>0.001</u>                                                                       | <u>&lt;1e-08</u>                                                                    | <u>6e-06</u>                                                                        |
|       | $t$ -test | <u>6e-08</u>                                                                      | <u>&lt;1e-08</u>                                                                  | <u>&lt;1e-08</u>                                                                  | <u>&lt;1e-08</u>                                                                  | <u>0.003</u>                                                                       | <u>&lt;1e-08</u>                                                                    | <u>&lt;1e-08</u>                                                                    |
|       | PCS       | 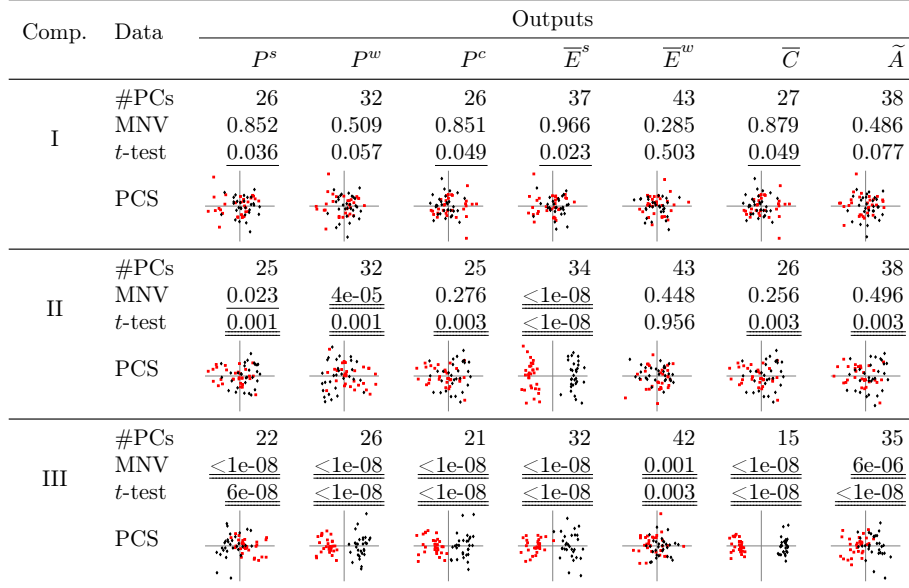 | 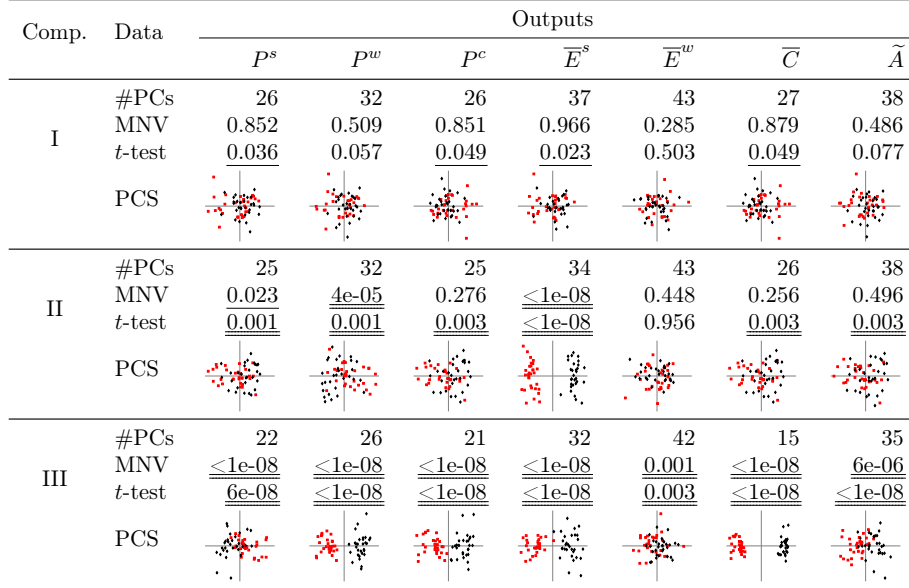 | 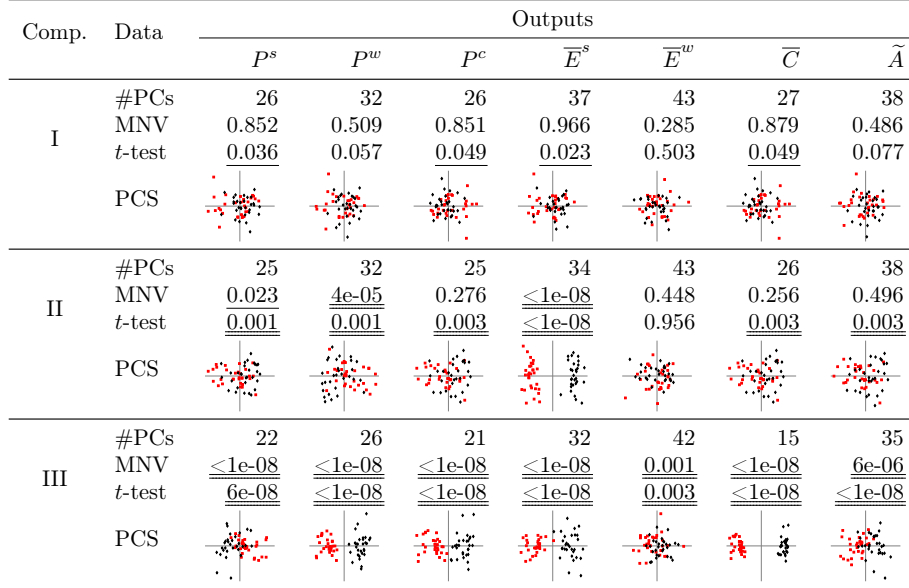 | 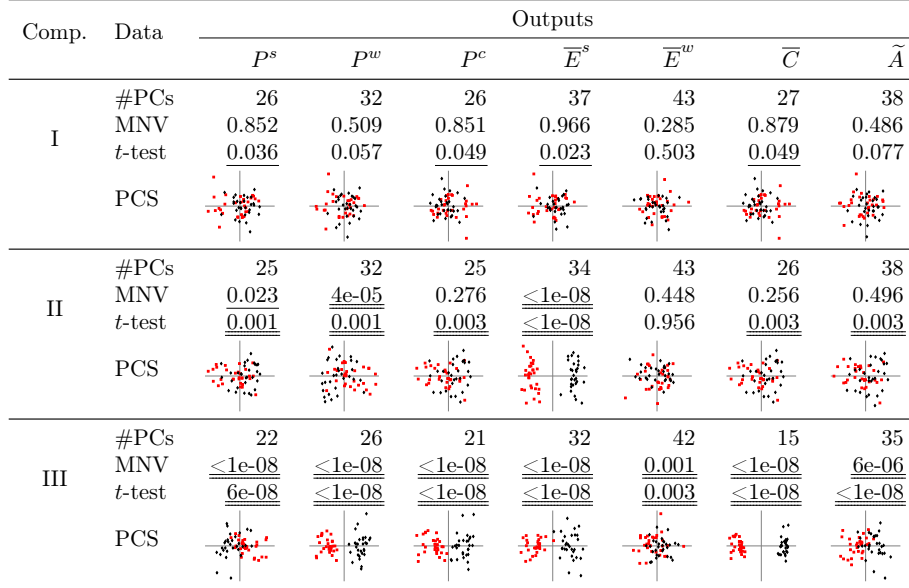 | 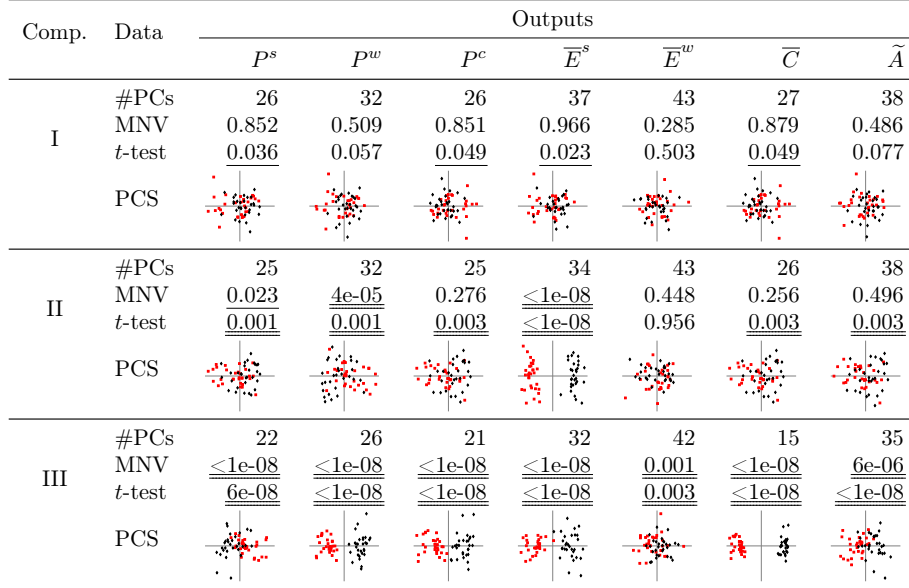 | 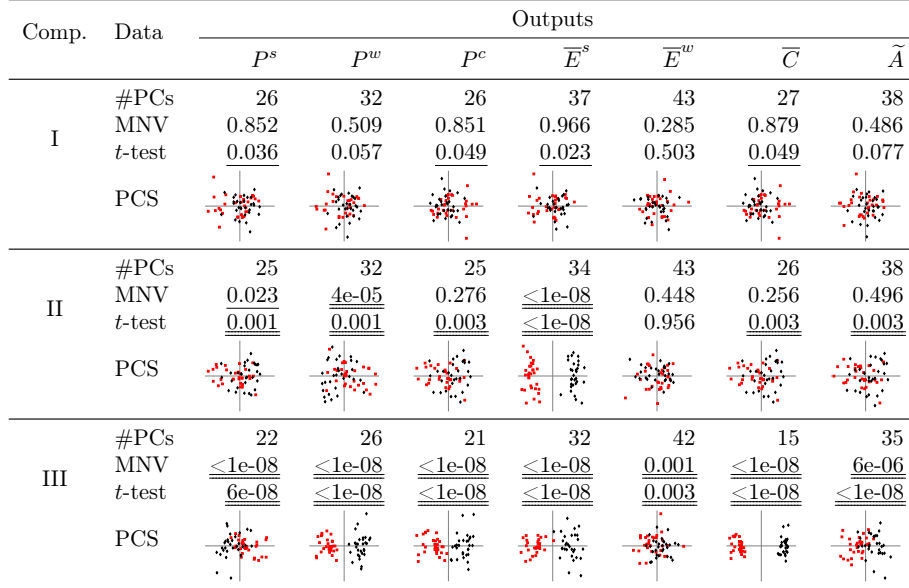 | 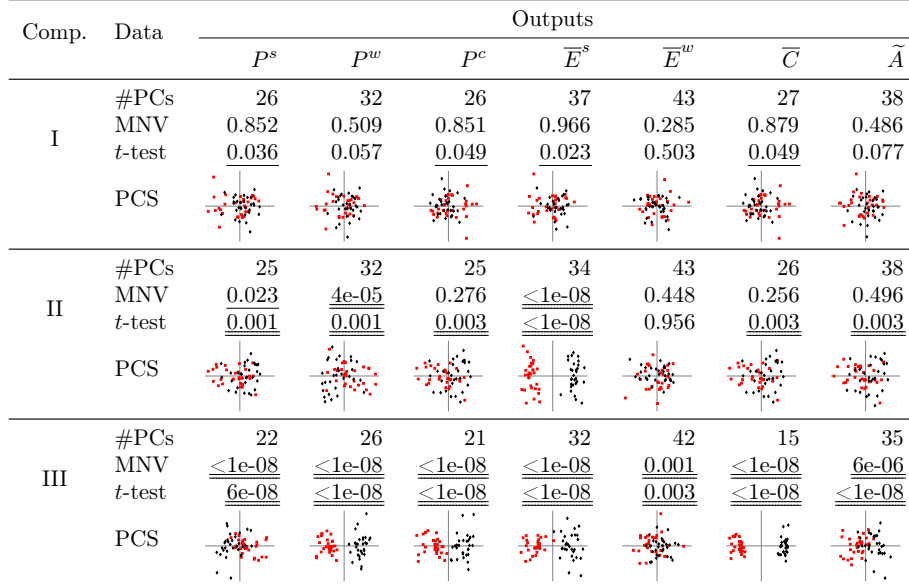 |

**Table S2.1** Model-independent comparison for model size 100, parameter set 1, and  $n = 30$  runs per configuration. Case I weights two similar setups, case II compares setups with a small implementation difference, and case III compares setups with a different parameter. #PCs is the number of PCs which explain at least 90% of variance, while MNV and  $t$ -test refer to the  $p$ -value yielded by the MANOVA (#PCs) and  $t$  (first PC) hypothesis tests, respectively. PCS shows the representation of the respective output in the first two dimensions of the PC space. Output  $\tilde{A}$  refers to the concatenation of all outputs (range scaled). The MANOVA test is not applicable to one PC, and the respective  $p$ -values are replaced with an asterisk (\*).  $P$ -values lower than 0.05 are underlined, while  $p$ -values lower than 0.01 are double-underlined.

| Comp. | Data      | Outputs                                                                             |                                                                                     |                                                                                     |                                                                                     |                                                                                      |                                                                                       |                                                                                       |
|-------|-----------|-------------------------------------------------------------------------------------|-------------------------------------------------------------------------------------|-------------------------------------------------------------------------------------|-------------------------------------------------------------------------------------|--------------------------------------------------------------------------------------|---------------------------------------------------------------------------------------|---------------------------------------------------------------------------------------|
|       |           | $P^s$                                                                               | $P^w$                                                                               | $P^c$                                                                               | $\bar{E}^s$                                                                         | $\bar{E}^w$                                                                          | $\bar{C}$                                                                             | $\tilde{A}$                                                                           |
| I     | #PCs      | 20                                                                                  | 19                                                                                  | 15                                                                                  | 29                                                                                  | 31                                                                                   | 15                                                                                    | 22                                                                                    |
|       | MNV       | 0.116                                                                               | 0.141                                                                               | 0.175                                                                               | 0.085                                                                               | 0.121                                                                                | 0.175                                                                                 | 0.125                                                                                 |
|       | $t$ -test | 0.108                                                                               | 0.128                                                                               | 0.106                                                                               | 0.111                                                                               | 0.067                                                                                | 0.106                                                                                 | 0.099                                                                                 |
|       | PCS       | 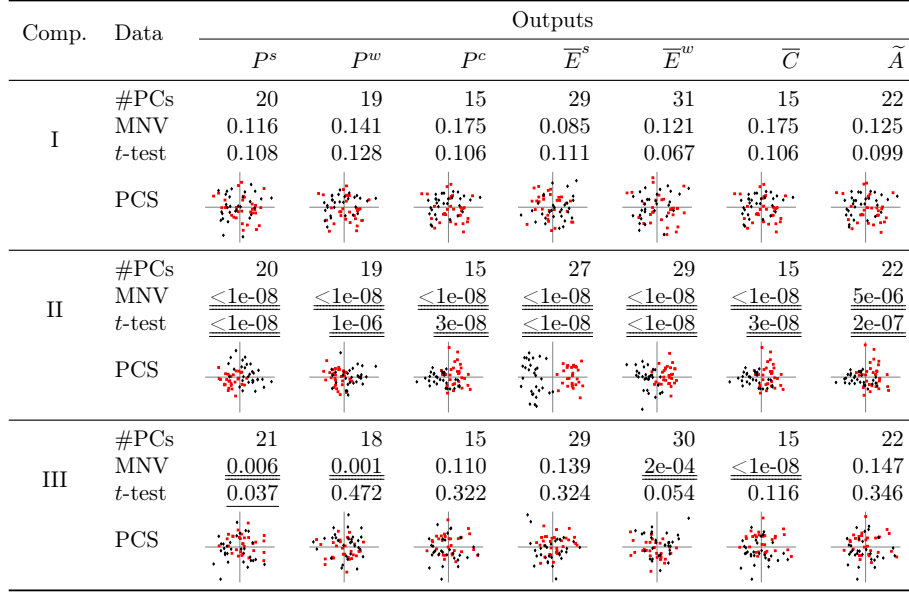   | 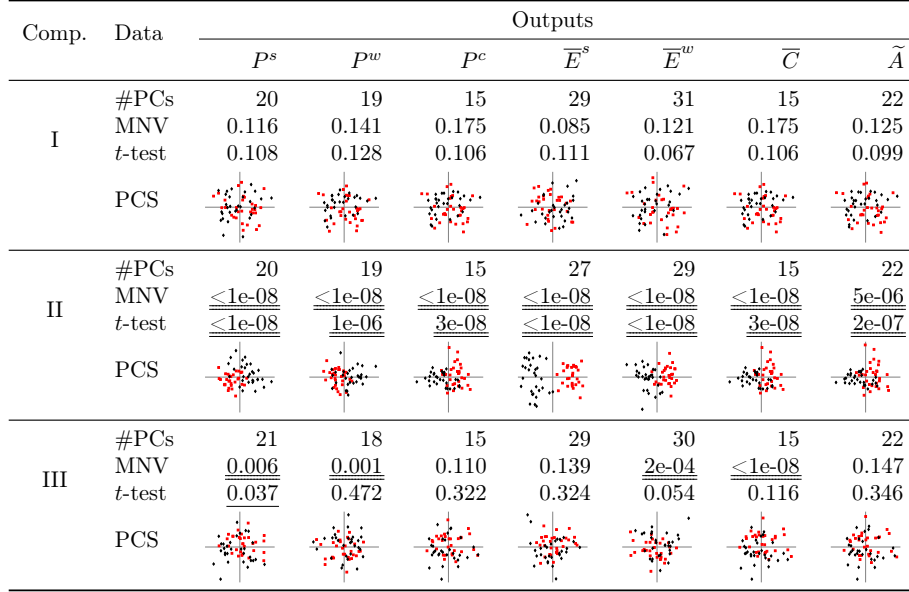   | 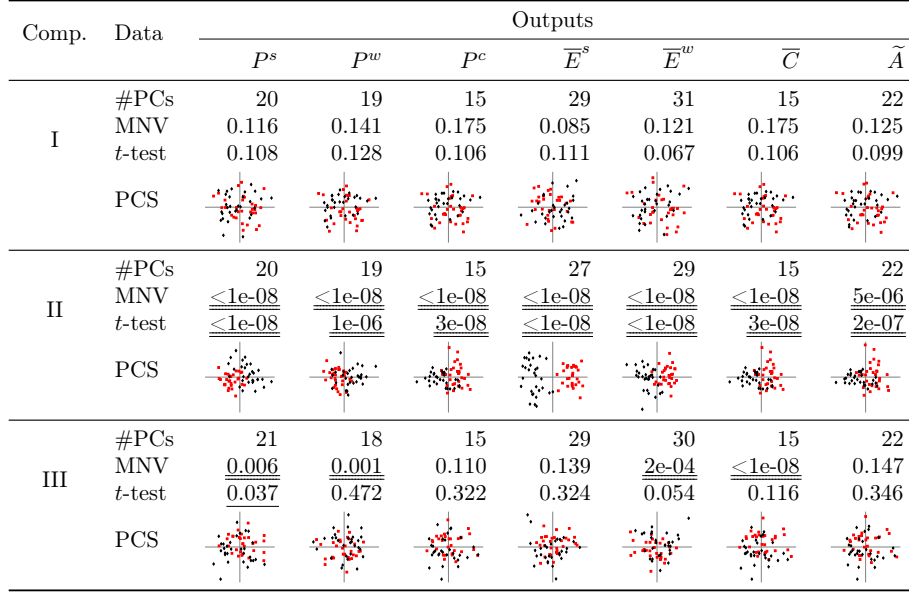   | 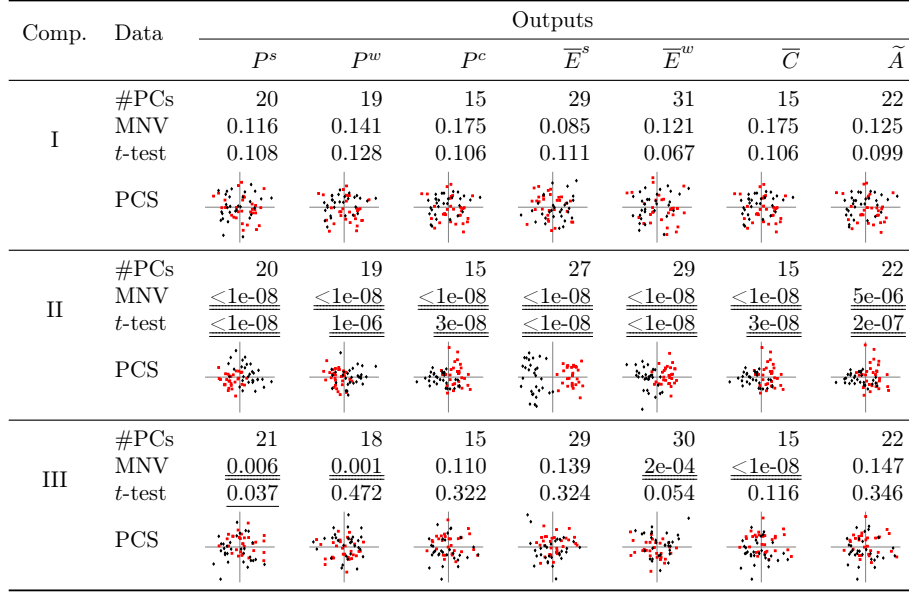   | 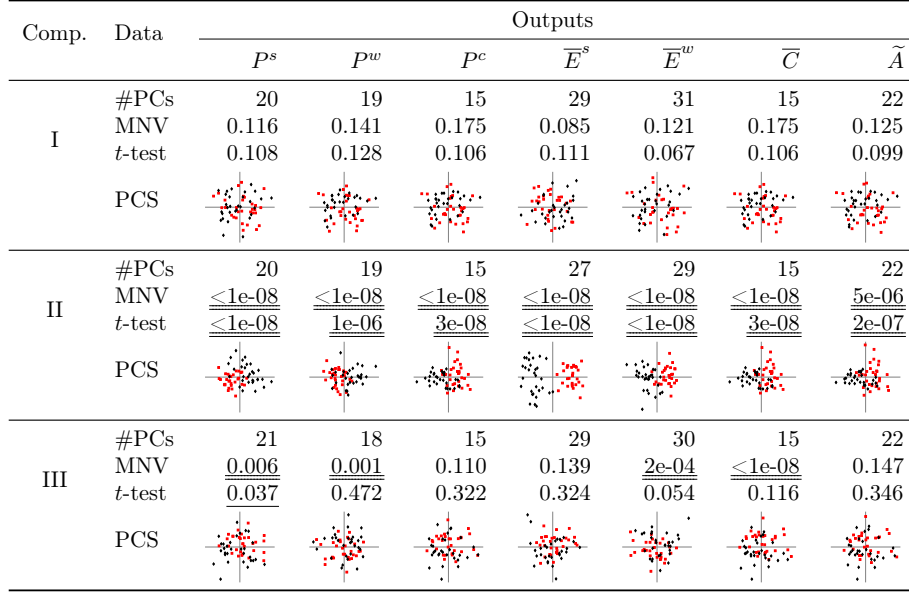   | 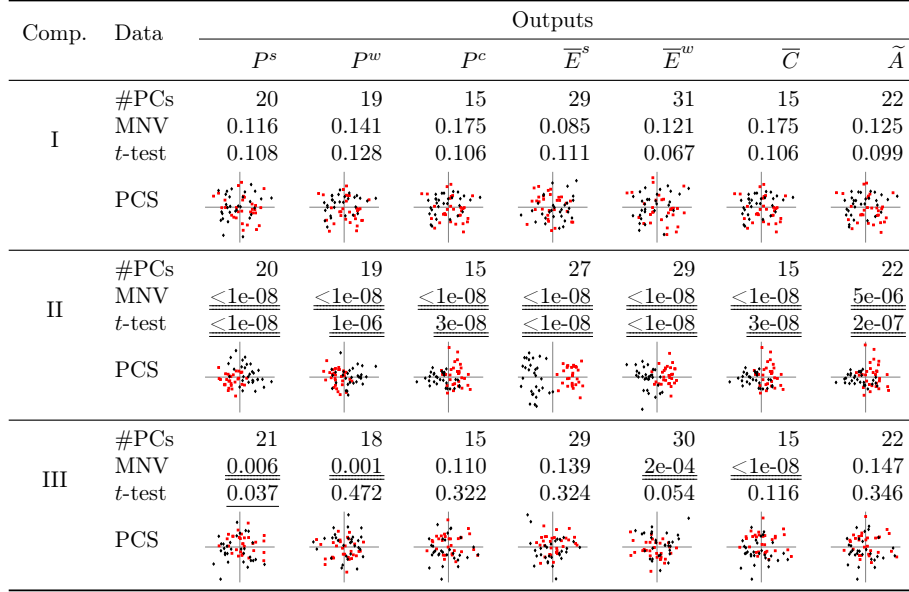   | 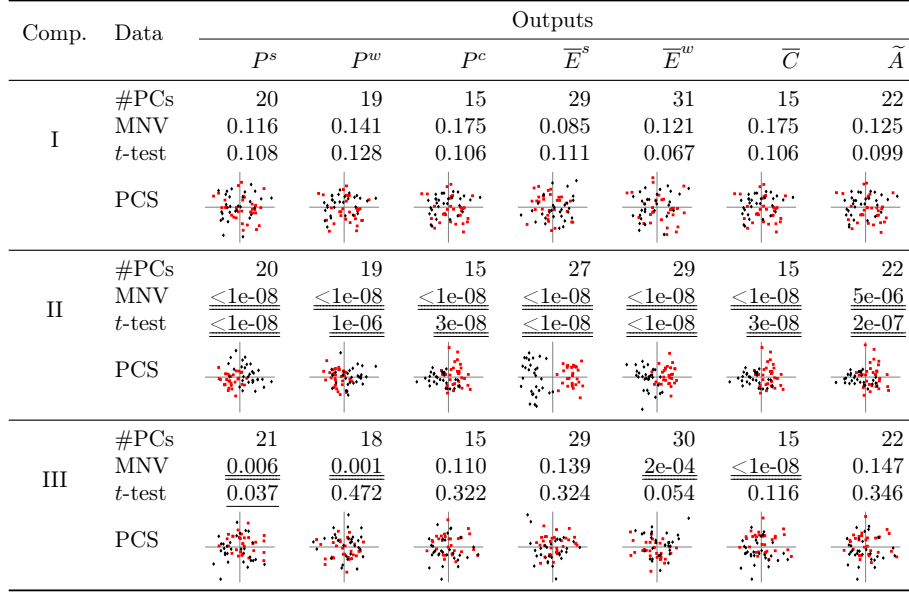   |
| II    | #PCs      | 20                                                                                  | 19                                                                                  | 15                                                                                  | 27                                                                                  | 29                                                                                   | 15                                                                                    | 22                                                                                    |
|       | MNV       | <u>&lt;1e-08</u>                                                                    | <u>&lt;1e-08</u>                                                                    | <u>&lt;1e-08</u>                                                                    | <u>&lt;1e-08</u>                                                                    | <u>&lt;1e-08</u>                                                                     | <u>&lt;1e-08</u>                                                                      | <u>5e-06</u>                                                                          |
|       | $t$ -test | <u>&lt;1e-08</u>                                                                    | <u>1e-06</u>                                                                        | <u>3e-08</u>                                                                        | <u>&lt;1e-08</u>                                                                    | <u>&lt;1e-08</u>                                                                     | <u>3e-08</u>                                                                          | <u>2e-07</u>                                                                          |
|       | PCS       | 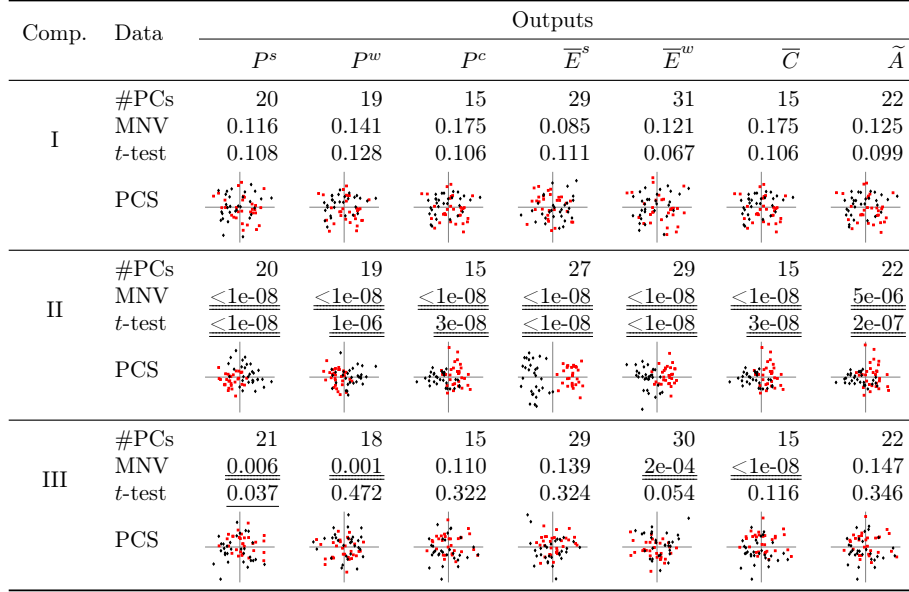   | 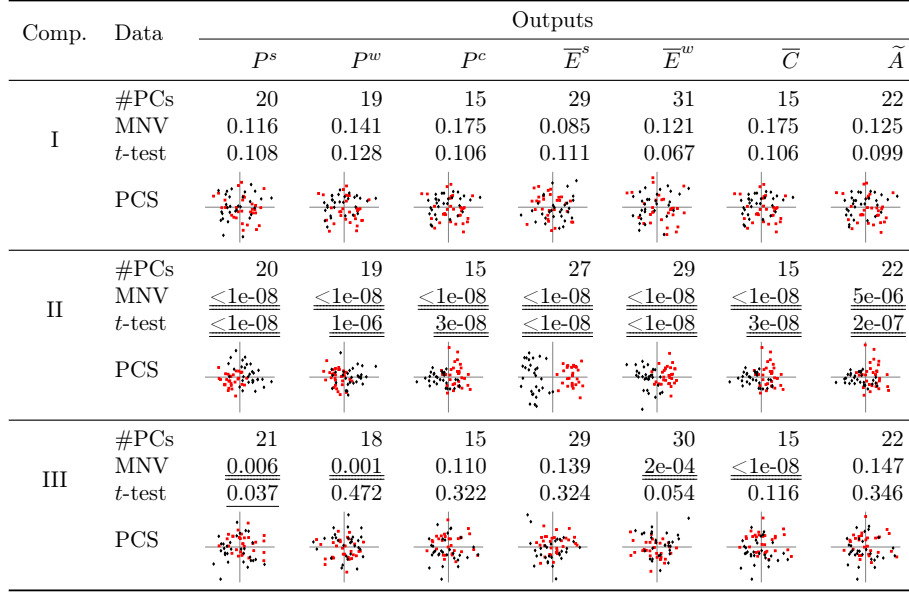   | 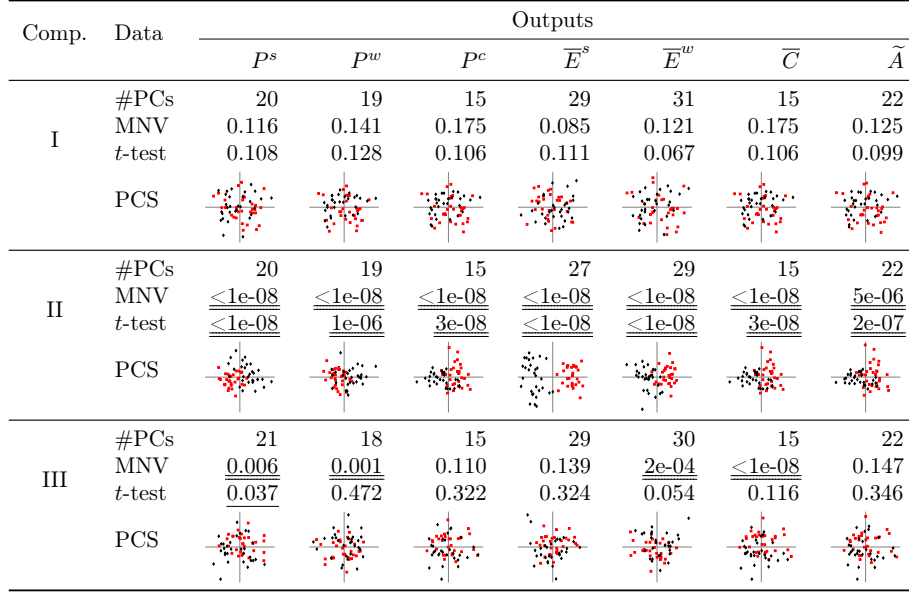   | 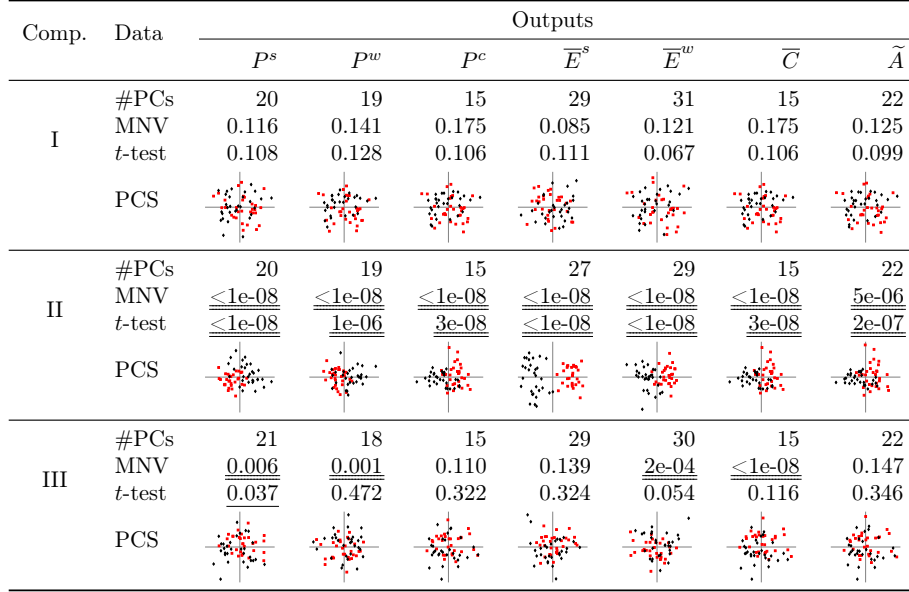   | 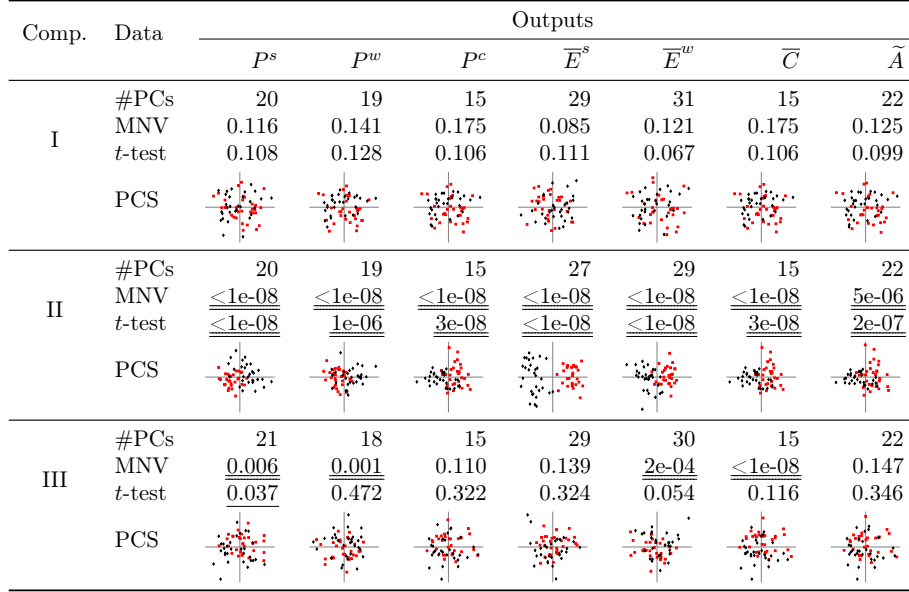   | 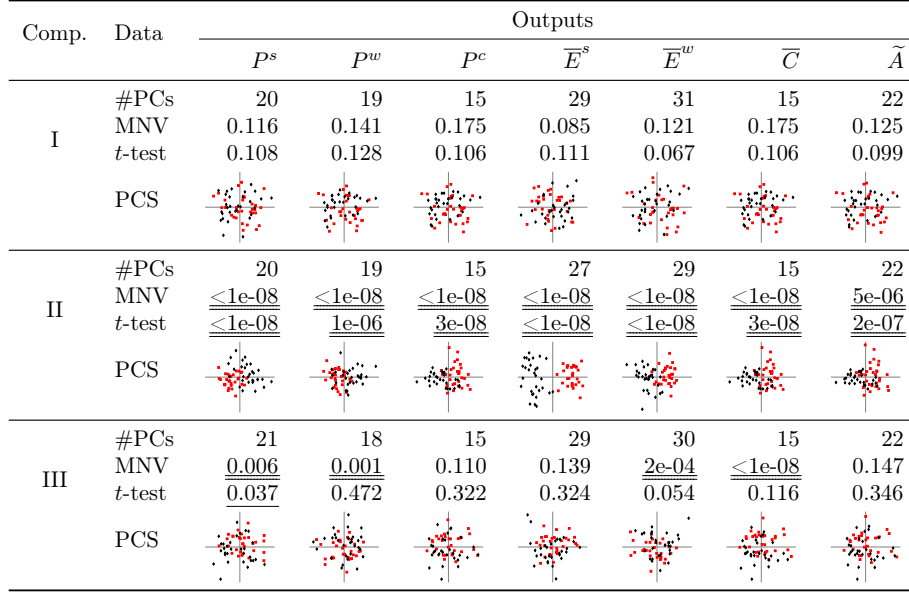   | 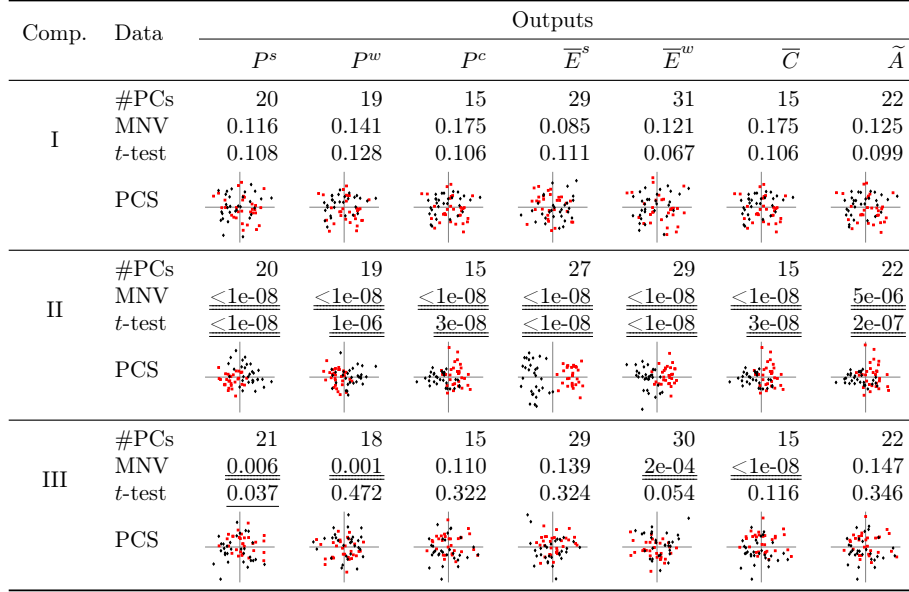   |
| III   | #PCs      | 21                                                                                  | 18                                                                                  | 15                                                                                  | 29                                                                                  | 30                                                                                   | 15                                                                                    | 22                                                                                    |
|       | MNV       | <u>0.006</u>                                                                        | <u>0.001</u>                                                                        | 0.110                                                                               | 0.139                                                                               | <u>2e-04</u>                                                                         | <u>&lt;1e-08</u>                                                                      | 0.147                                                                                 |
|       | $t$ -test | <u>0.037</u>                                                                        | 0.472                                                                               | 0.322                                                                               | 0.324                                                                               | 0.054                                                                                | 0.116                                                                                 | 0.346                                                                                 |
|       | PCS       | 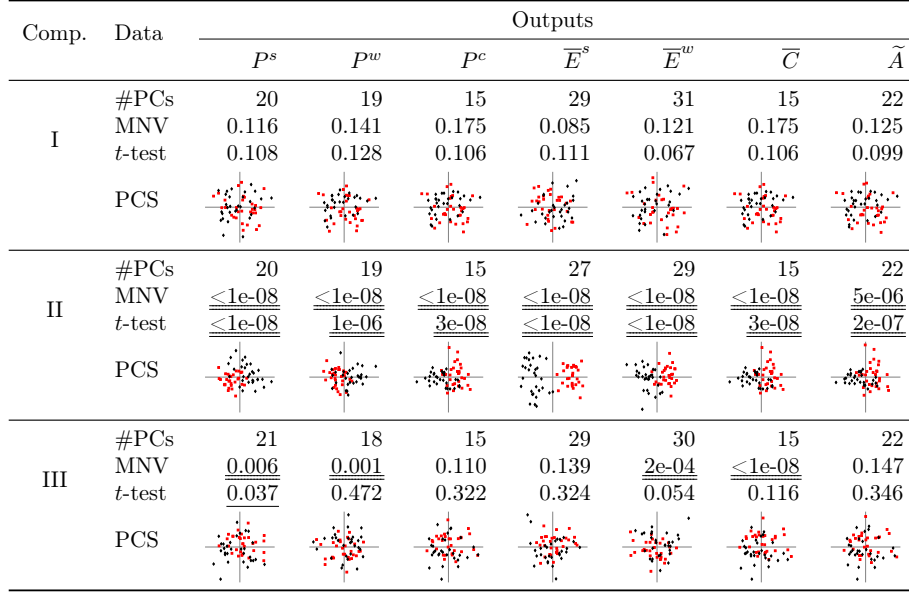 | 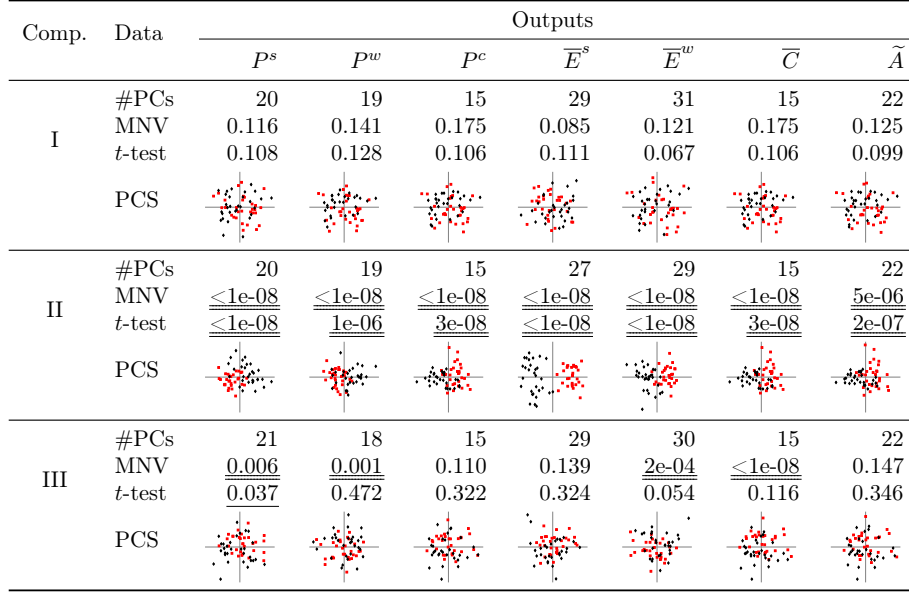 | 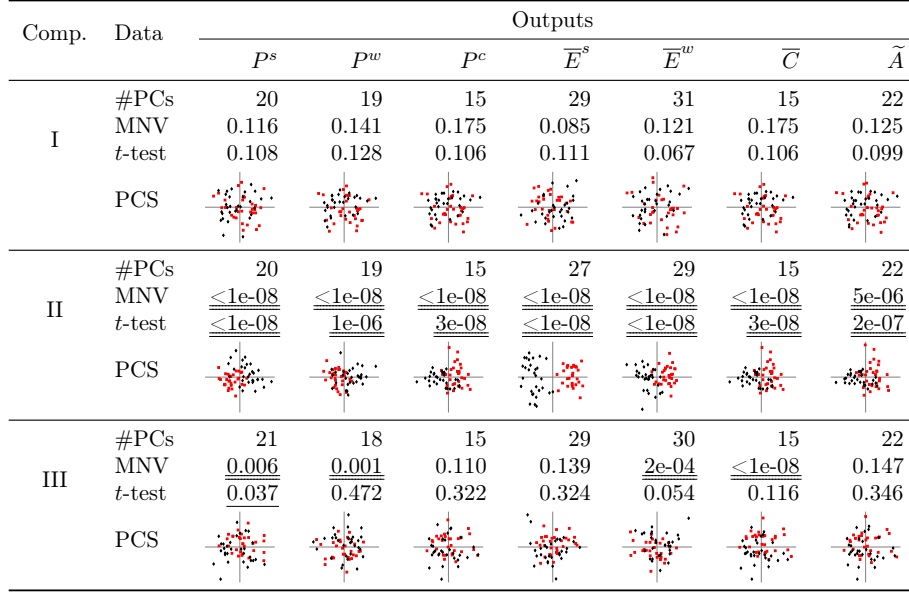 | 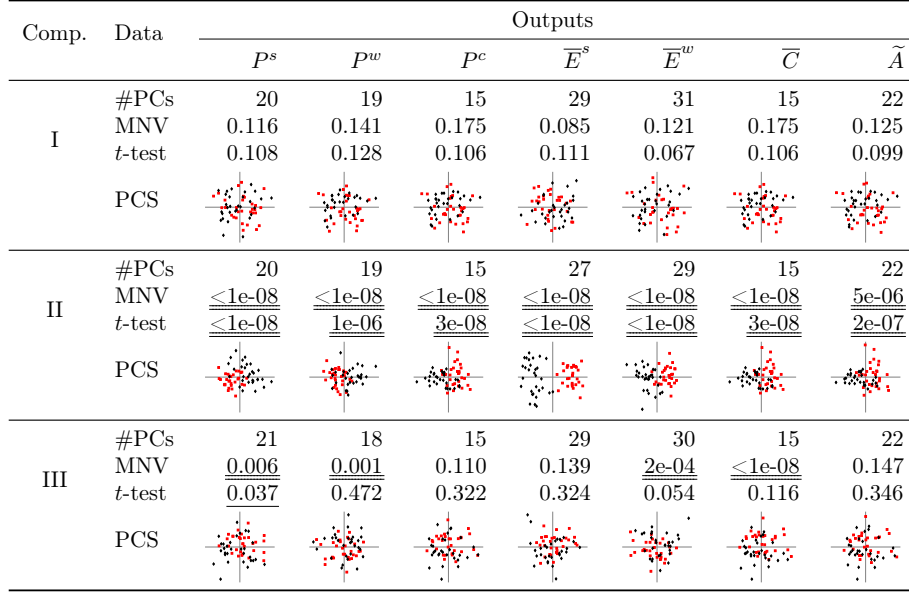 | 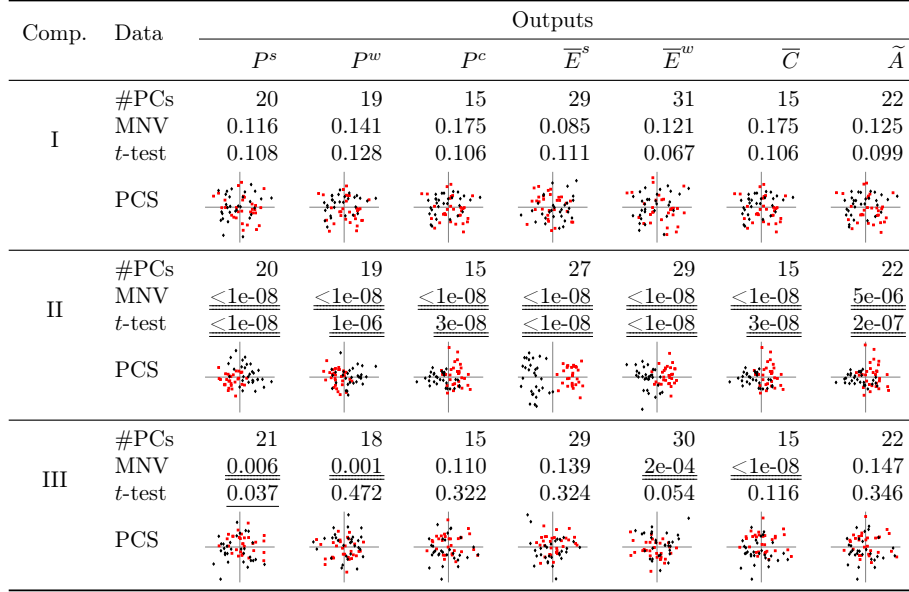 | 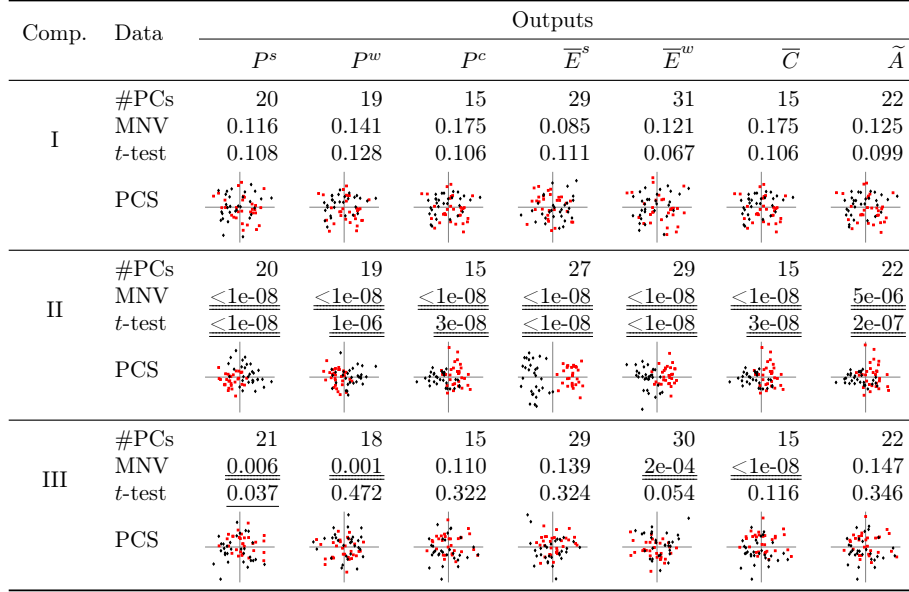 | 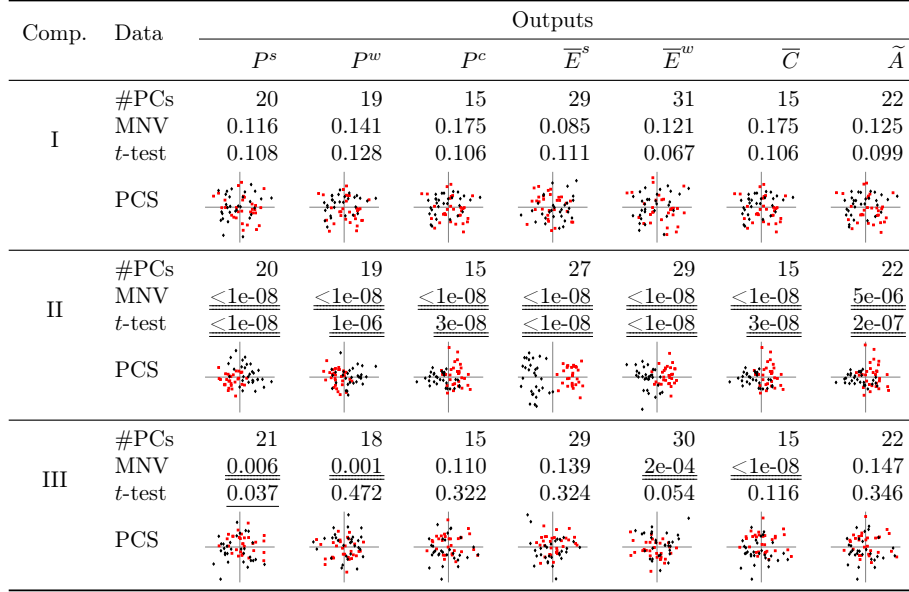 |

**Table S2.2** Model-independent comparison for model size 100, parameter set 2, and  $n = 30$  runs per configuration. Case I weights two similar setups, case II compares setups with a small implementation difference, and case III compares setups with a different parameter. #PCs is the number of PCs which explain at least 90% of variance, while MNV and  $t$ -test refer to the  $p$ -value yielded by the MANOVA (#PCs) and  $t$  (first PC) hypothesis tests, respectively. PCS shows the representation of the respective output in the first two dimensions of the PC space. Output  $\tilde{A}$  refers to the concatenation of all outputs (range scaled). The MANOVA test is not applicable to one PC, and the respective  $p$ -values are replaced with an asterisk (\*).  $P$ -values lower than 0.05 are underlined, while  $p$ -values lower than 0.01 are double-underlined.

| Comp. | Data      | Outputs                                                                             |                                                                                     |                                                                                     |                                                                                     |                                                                                      |                                                                                       |                                                                                       |
|-------|-----------|-------------------------------------------------------------------------------------|-------------------------------------------------------------------------------------|-------------------------------------------------------------------------------------|-------------------------------------------------------------------------------------|--------------------------------------------------------------------------------------|---------------------------------------------------------------------------------------|---------------------------------------------------------------------------------------|
|       |           | $P^s$                                                                               | $P^w$                                                                               | $P^c$                                                                               | $\bar{E}^s$                                                                         | $\bar{E}^w$                                                                          | $\bar{C}$                                                                             | $\tilde{A}$                                                                           |
| I     | #PCs      | 25                                                                                  | 32                                                                                  | 25                                                                                  | 36                                                                                  | 43                                                                                   | 26                                                                                    | 38                                                                                    |
|       | MNV       | 0.287                                                                               | 0.214                                                                               | 0.157                                                                               | 0.123                                                                               | 0.699                                                                                | 0.187                                                                                 | 0.356                                                                                 |
|       | $t$ -test | 0.783                                                                               | 0.810                                                                               | 0.895                                                                               | 0.973                                                                               | 0.830                                                                                | 0.895                                                                                 | 0.979                                                                                 |
|       | PCS       | 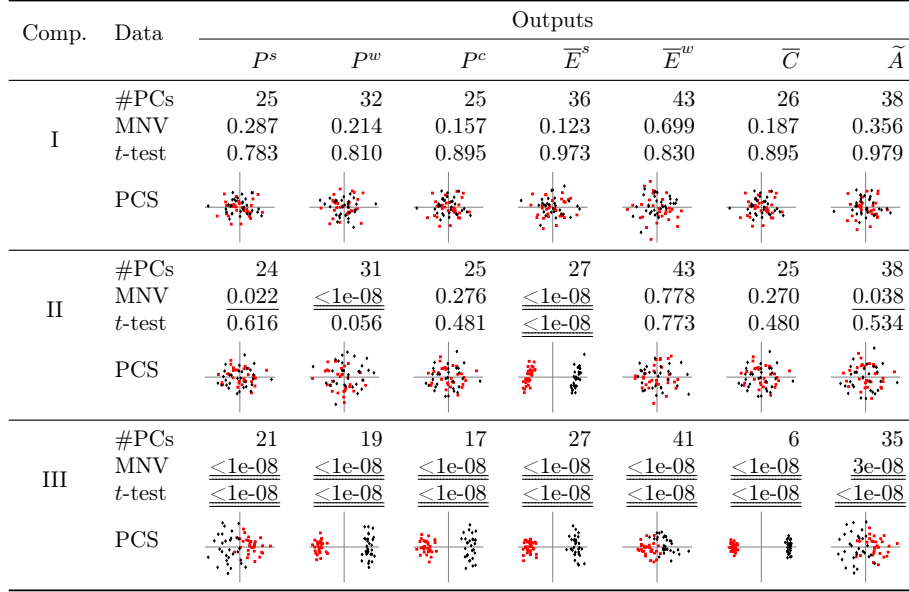   | 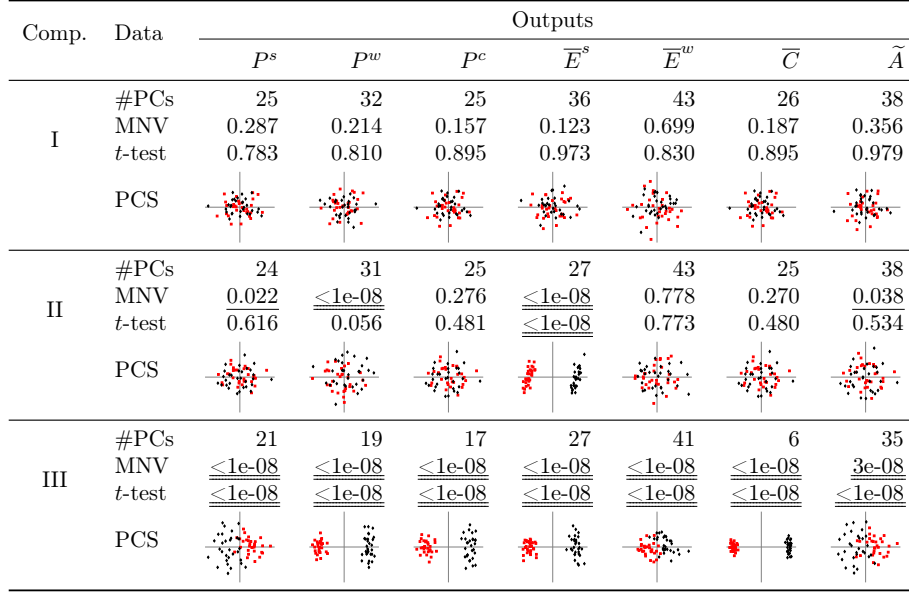   | 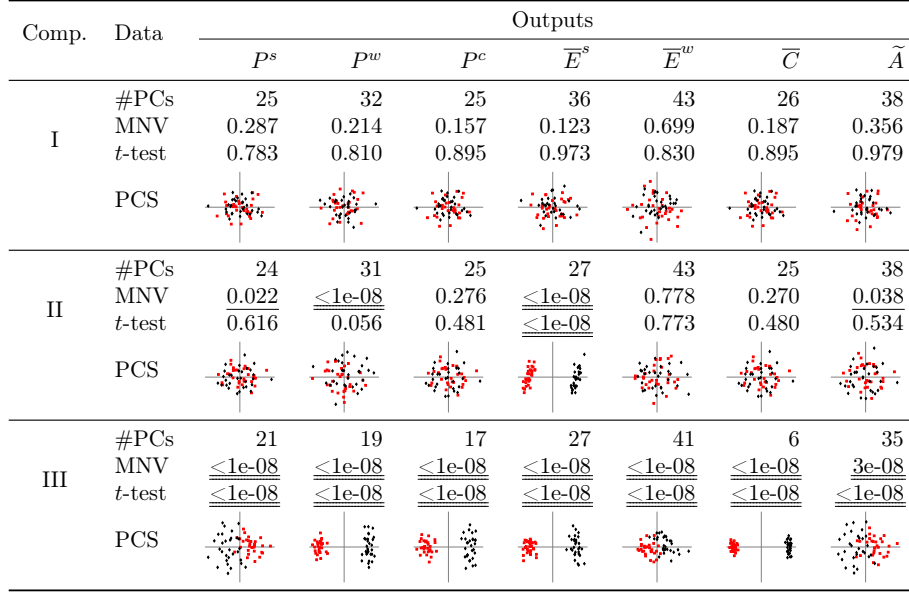   | 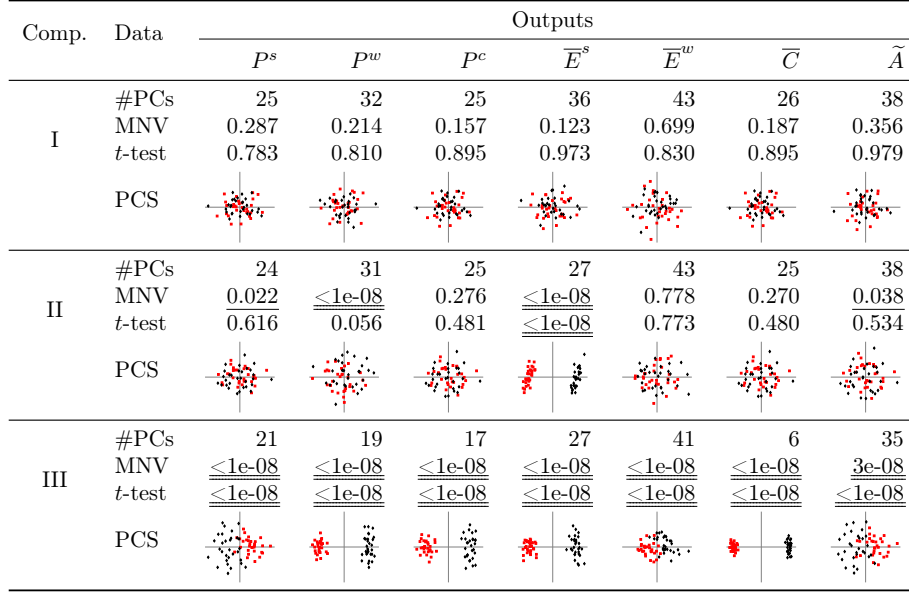   | 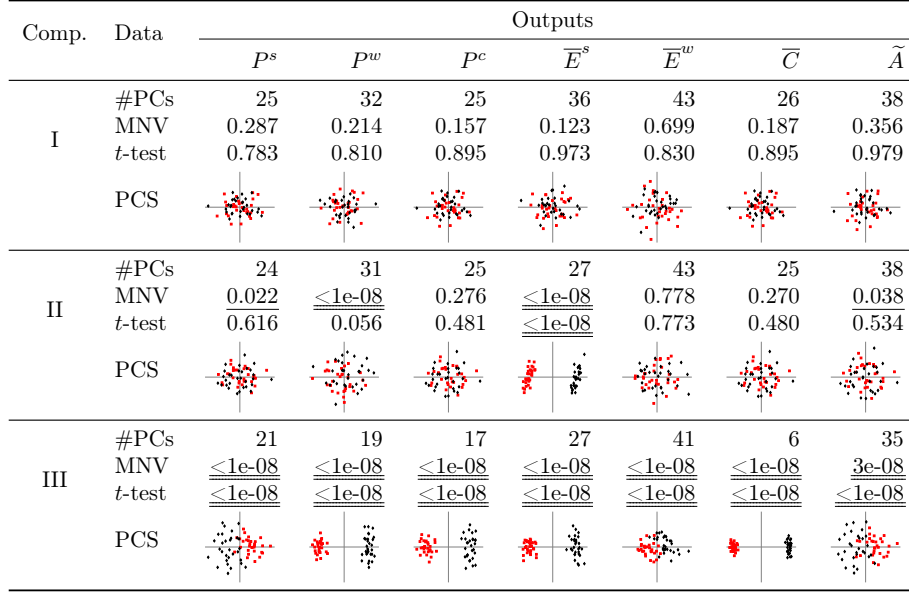   | 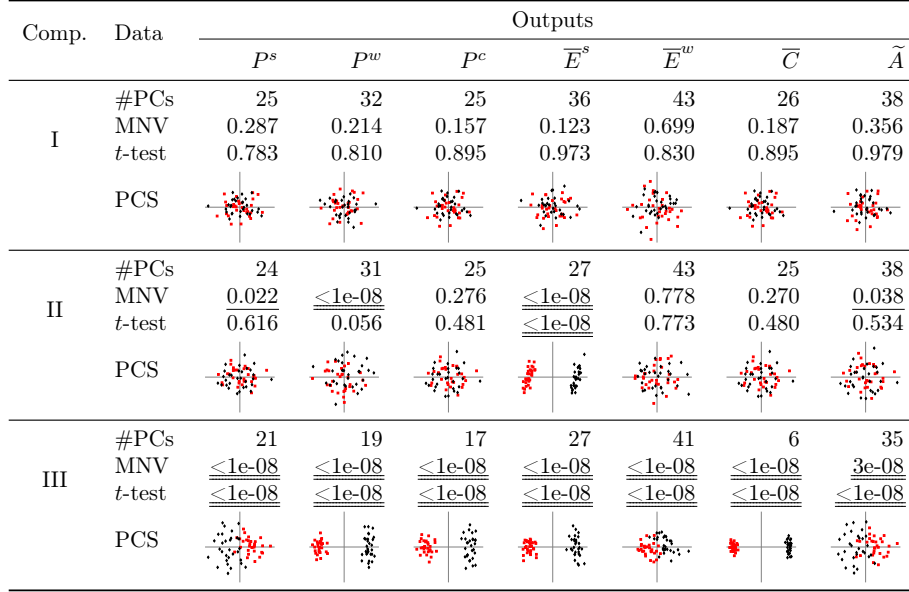   | 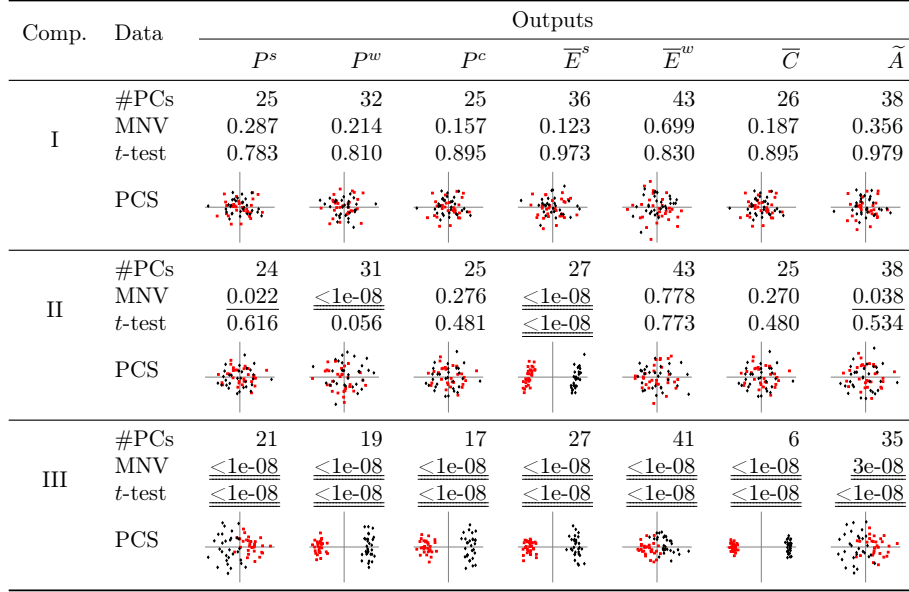   |
| II    | #PCs      | 24                                                                                  | 31                                                                                  | 25                                                                                  | 27                                                                                  | 43                                                                                   | 25                                                                                    | 38                                                                                    |
|       | MNV       | 0.022                                                                               | <u>&lt;1e-08</u>                                                                    | 0.276                                                                               | <u>&lt;1e-08</u>                                                                    | 0.778                                                                                | 0.270                                                                                 | <u>0.038</u>                                                                          |
|       | $t$ -test | 0.616                                                                               | 0.056                                                                               | 0.481                                                                               | <u>&lt;1e-08</u>                                                                    | 0.773                                                                                | 0.480                                                                                 | 0.534                                                                                 |
|       | PCS       | 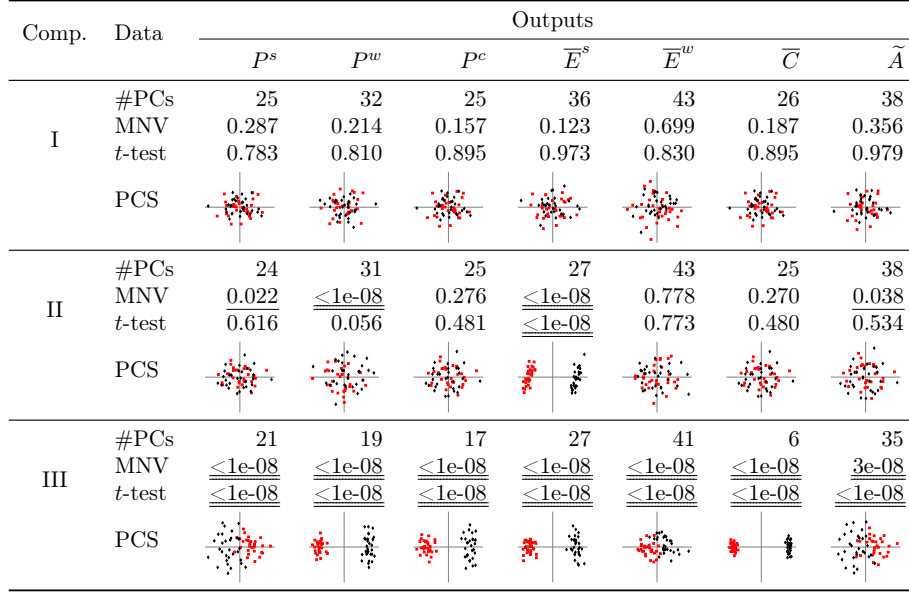   | 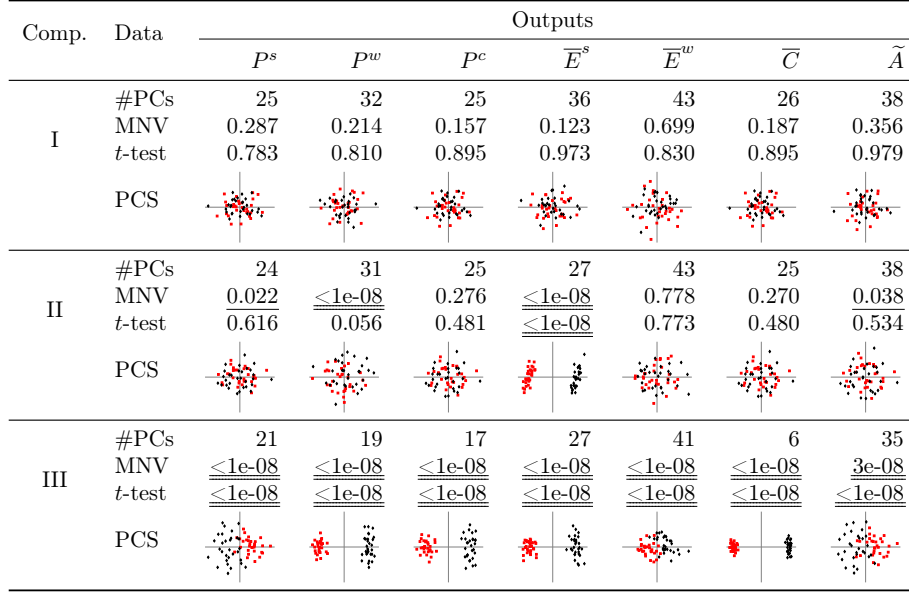   | 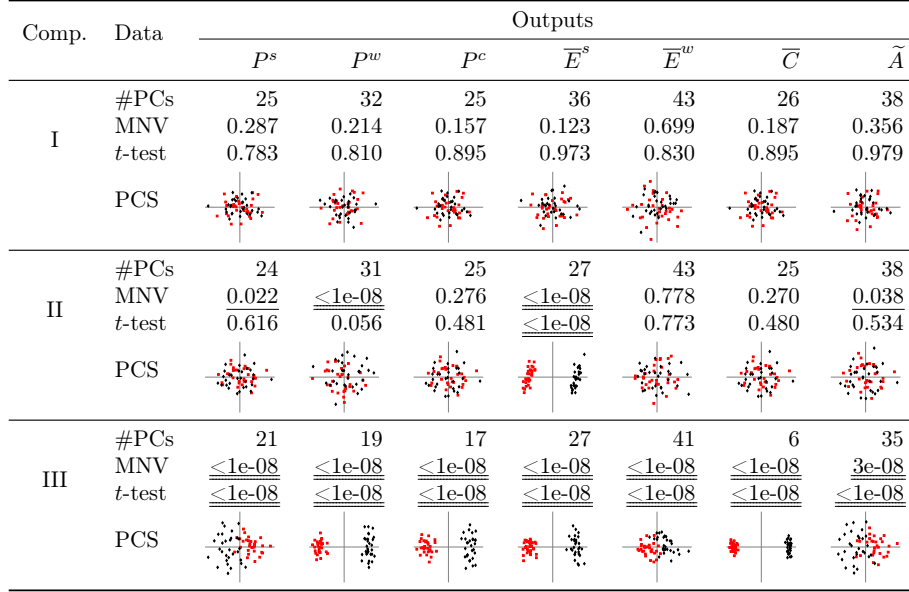   | 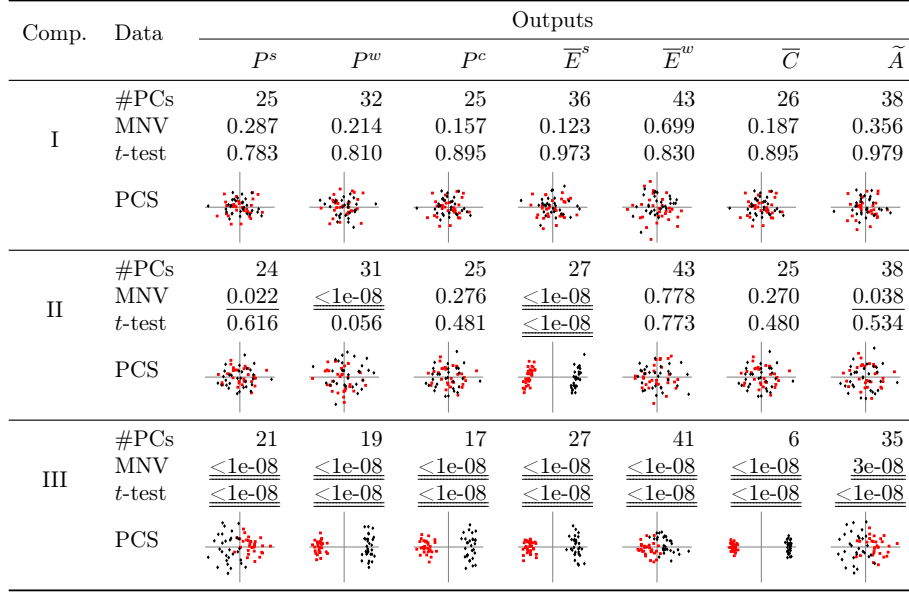   | 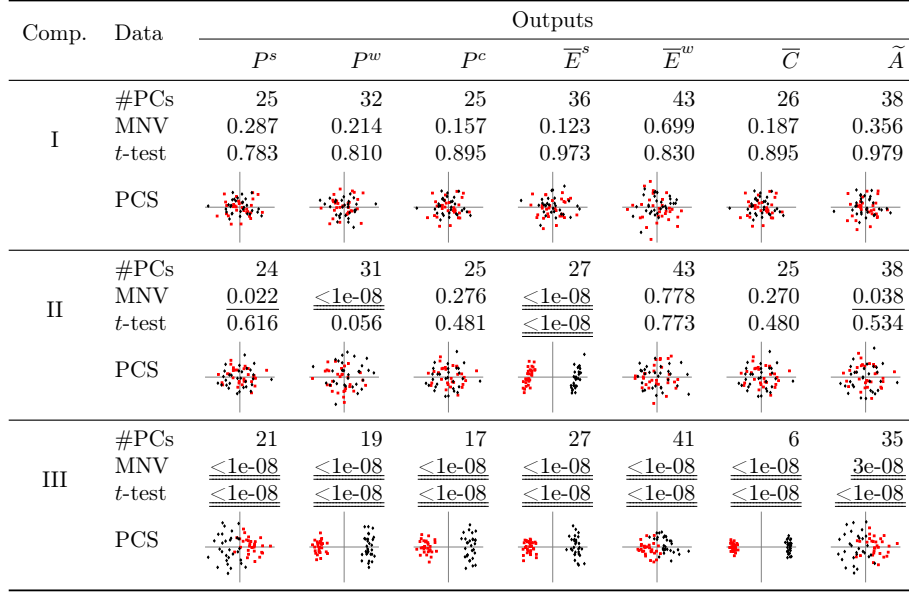   | 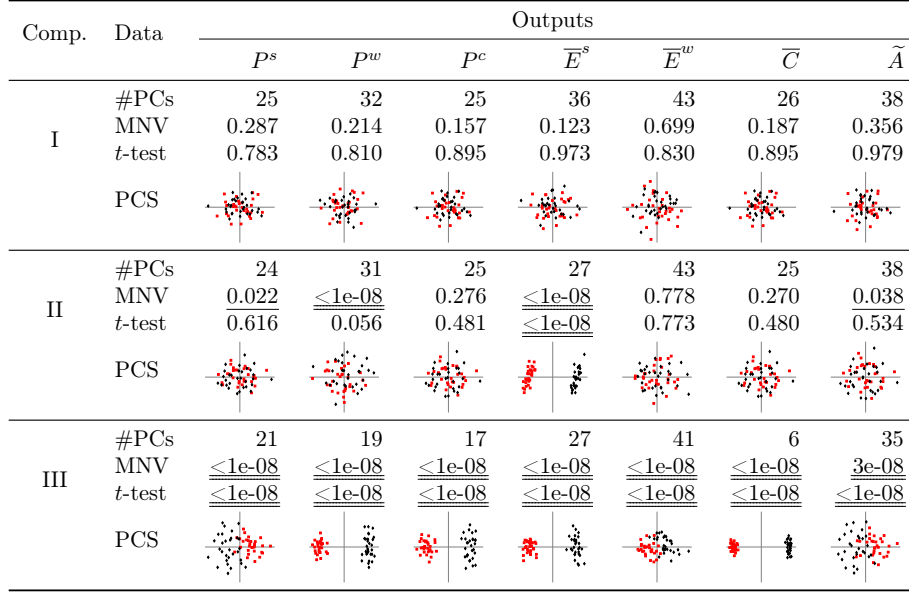   | 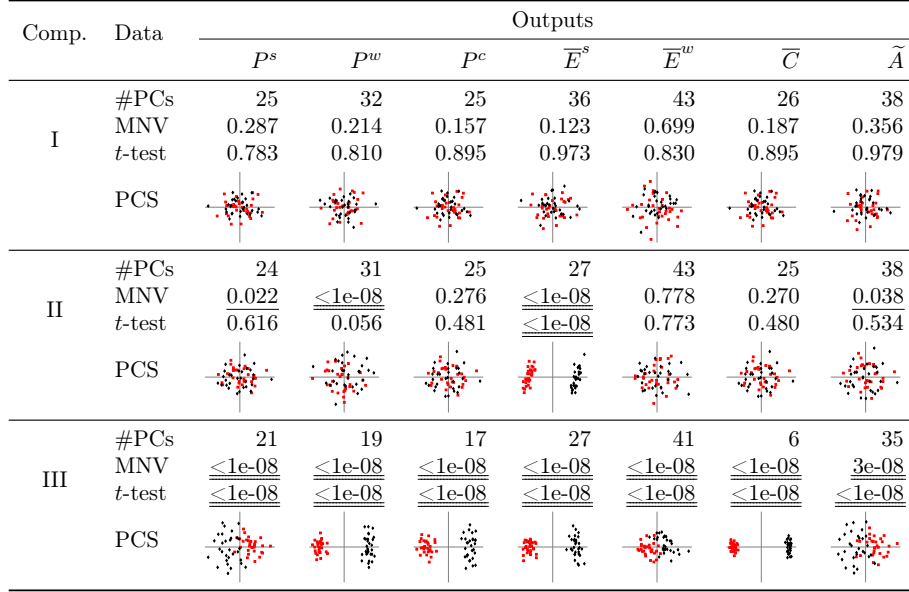   |
| III   | #PCs      | 21                                                                                  | 19                                                                                  | 17                                                                                  | 27                                                                                  | 41                                                                                   | 6                                                                                     | 35                                                                                    |
|       | MNV       | <u>&lt;1e-08</u>                                                                    | <u>&lt;1e-08</u>                                                                    | <u>&lt;1e-08</u>                                                                    | <u>&lt;1e-08</u>                                                                    | <u>&lt;1e-08</u>                                                                     | <u>&lt;1e-08</u>                                                                      | <u>3e-08</u>                                                                          |
|       | $t$ -test | <u>&lt;1e-08</u>                                                                    | <u>&lt;1e-08</u>                                                                    | <u>&lt;1e-08</u>                                                                    | <u>&lt;1e-08</u>                                                                    | <u>&lt;1e-08</u>                                                                     | <u>&lt;1e-08</u>                                                                      | <u>&lt;1e-08</u>                                                                      |
|       | PCS       | 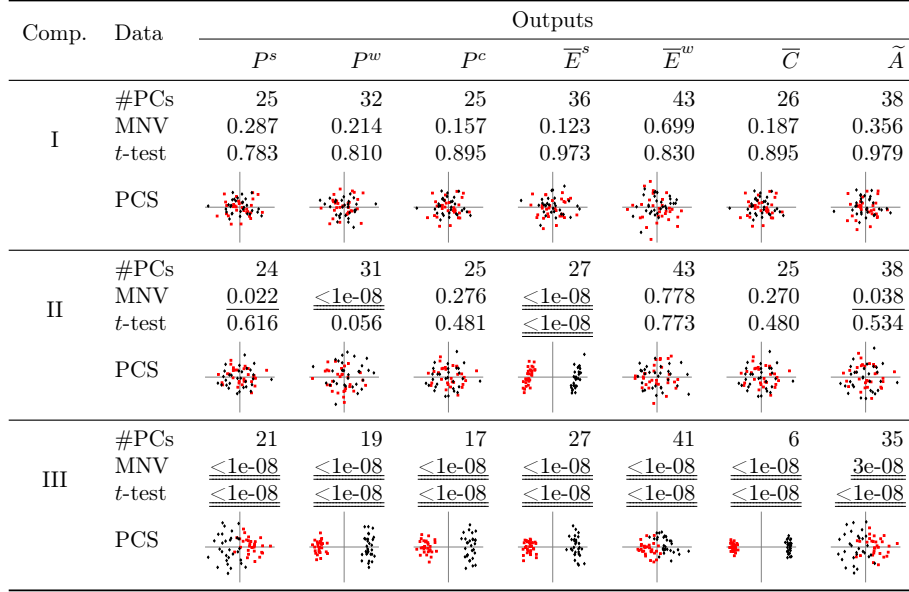 | 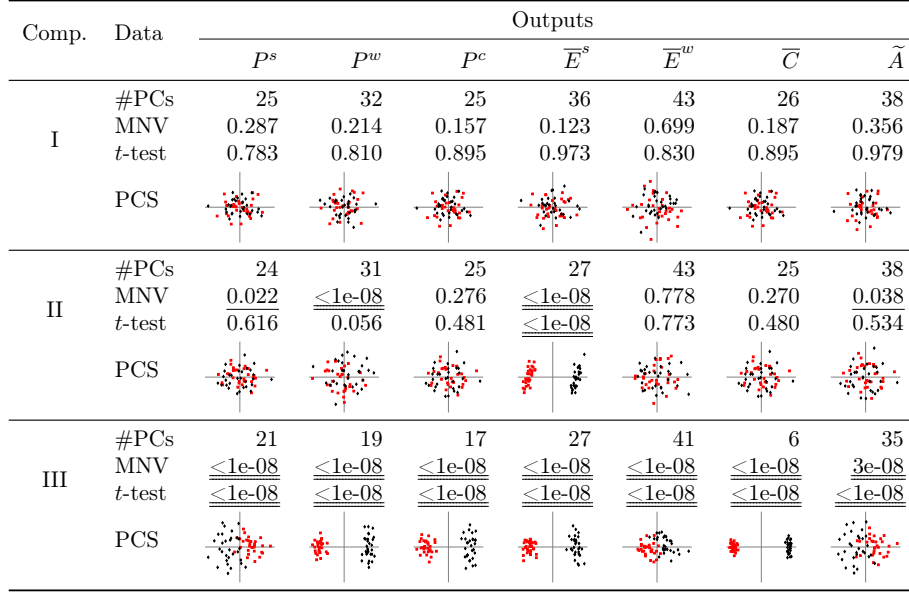 | 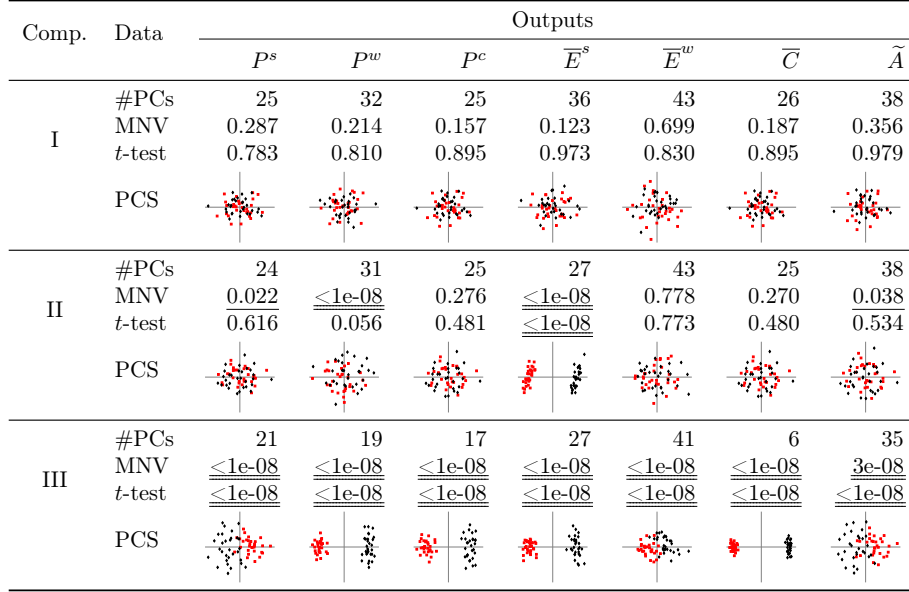 | 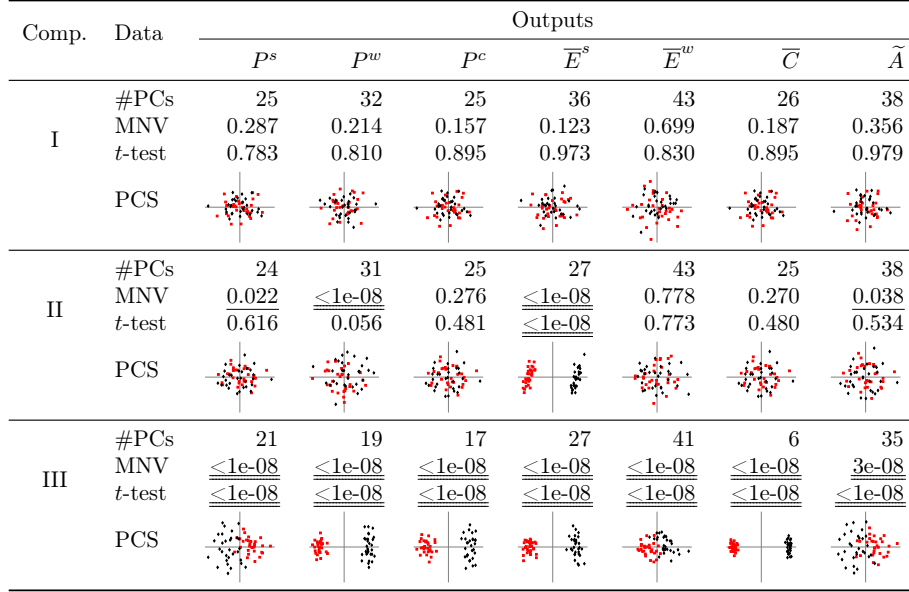 | 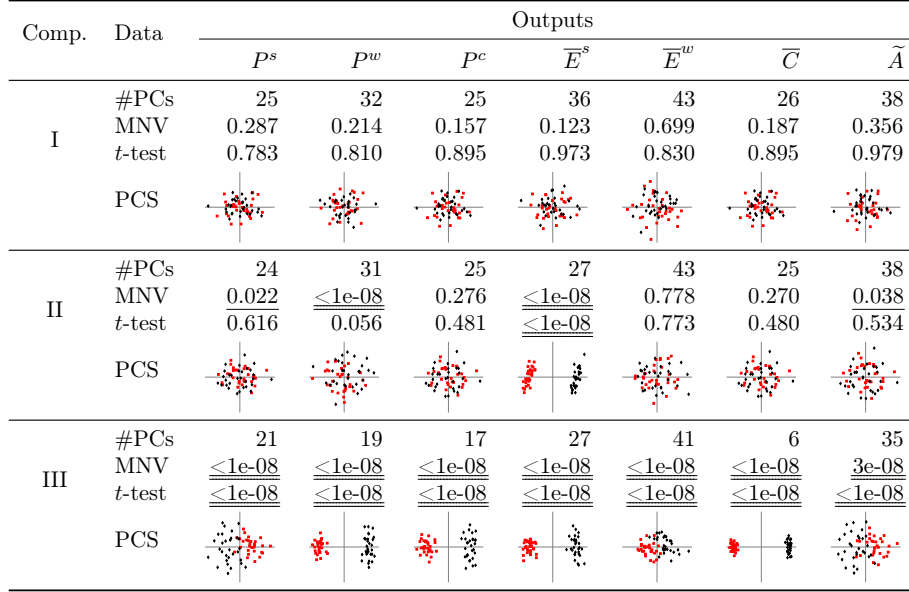 | 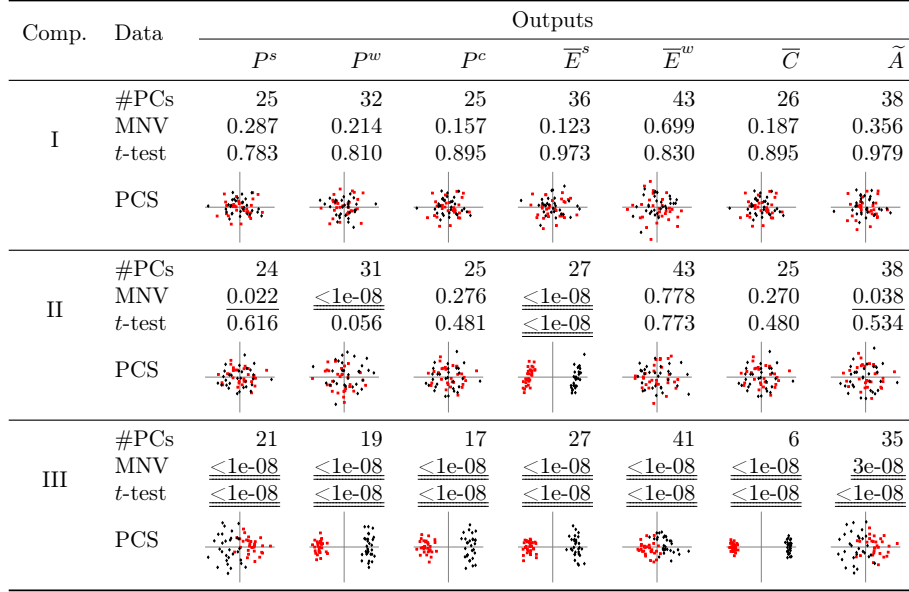 | 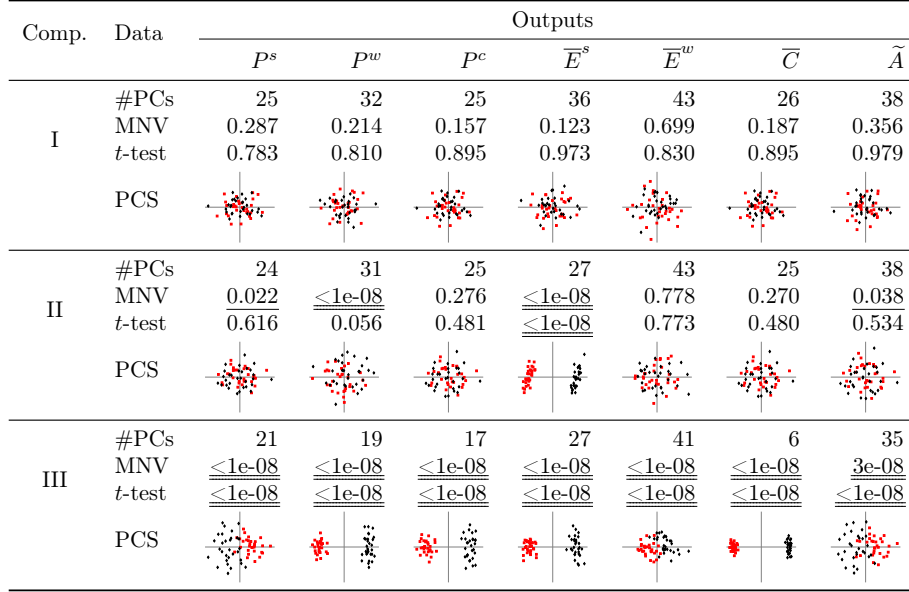 |

**Table S2.3** Model-independent comparison for model size 200, parameter set 1, and  $n = 30$  runs per configuration. Case I weights two similar setups, case II compares setups with a small implementation difference, and case III compares setups with a different parameter. #PCs is the number of PCs which explain at least 90% of variance, while MNV and  $t$ -test refer to the  $p$ -value yielded by the MANOVA (#PCs) and  $t$  (first PC) hypothesis tests, respectively. PCS shows the representation of the respective output in the first two dimensions of the PC space. Output  $\tilde{A}$  refers to the concatenation of all outputs (range scaled). The MANOVA test is not applicable to one PC, and the respective  $p$ -values are replaced with an asterisk (\*).  $P$ -values lower than 0.05 are underlined, while  $p$ -values lower than 0.01 are double-underlined.

| Comp. | Data      | Outputs                                                                             |                                                                                     |                                                                                     |                                                                                     |                                                                                      |                                                                                       |                                                                                       |
|-------|-----------|-------------------------------------------------------------------------------------|-------------------------------------------------------------------------------------|-------------------------------------------------------------------------------------|-------------------------------------------------------------------------------------|--------------------------------------------------------------------------------------|---------------------------------------------------------------------------------------|---------------------------------------------------------------------------------------|
|       |           | $P^s$                                                                               | $P^w$                                                                               | $P^c$                                                                               | $\overline{E}^s$                                                                    | $\overline{E}^w$                                                                     | $\overline{C}$                                                                        | $\tilde{A}$                                                                           |
| I     | #PCs      | 21                                                                                  | 19                                                                                  | 15                                                                                  | 29                                                                                  | 31                                                                                   | 15                                                                                    | 21                                                                                    |
|       | MNV       | 0.138                                                                               | 0.264                                                                               | 0.322                                                                               | 0.342                                                                               | 0.652                                                                                | 0.322                                                                                 | 0.244                                                                                 |
|       | $t$ -test | 0.192                                                                               | 0.294                                                                               | 0.280                                                                               | 0.985                                                                               | 0.378                                                                                | 0.280                                                                                 | 0.240                                                                                 |
|       | PCS       | 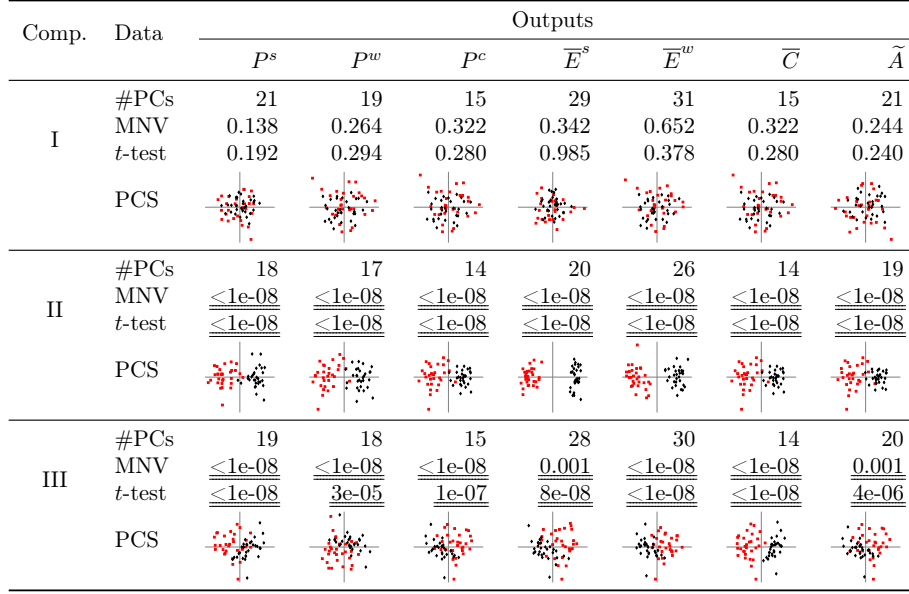   | 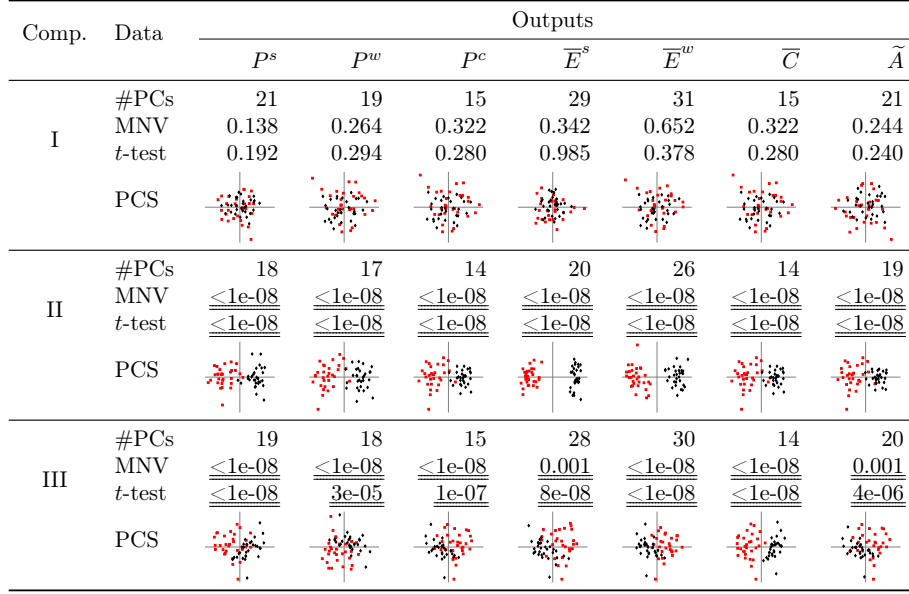   | 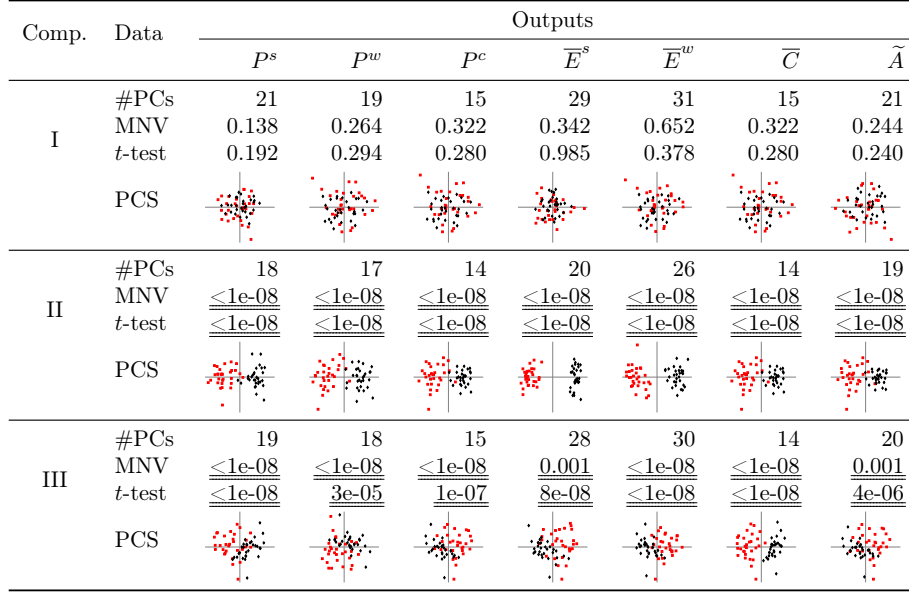   | 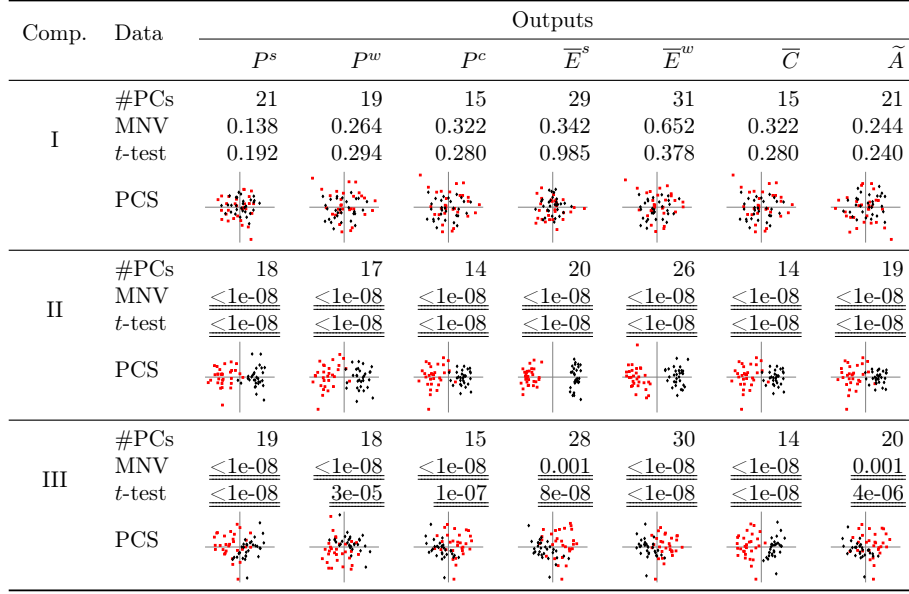   | 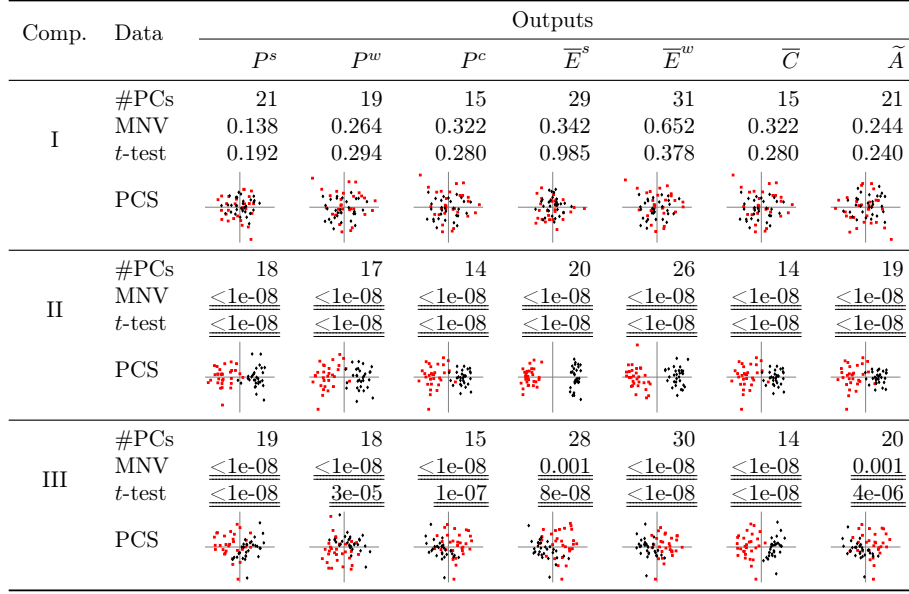   | 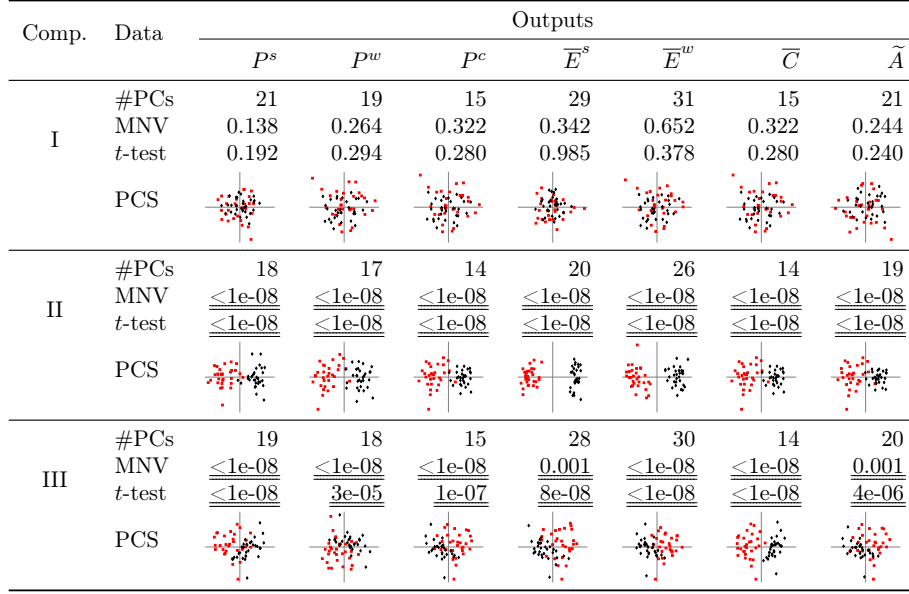   | 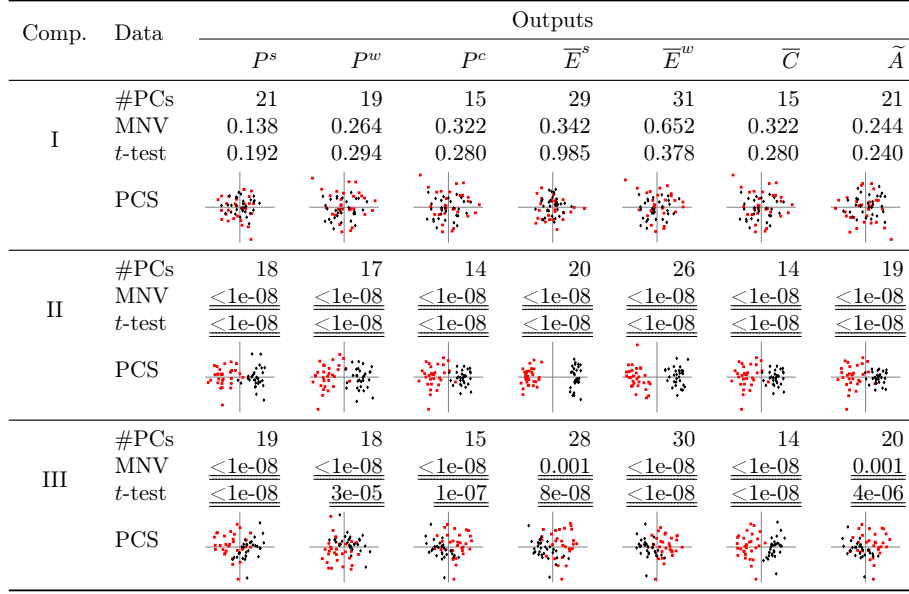   |
| II    | #PCs      | 18                                                                                  | 17                                                                                  | 14                                                                                  | 20                                                                                  | 26                                                                                   | 14                                                                                    | 19                                                                                    |
|       | MNV       | <u>&lt;1e-08</u>                                                                    | <u>&lt;1e-08</u>                                                                    | <u>&lt;1e-08</u>                                                                    | <u>&lt;1e-08</u>                                                                    | <u>&lt;1e-08</u>                                                                     | <u>&lt;1e-08</u>                                                                      | <u>&lt;1e-08</u>                                                                      |
|       | $t$ -test | <u>&lt;1e-08</u>                                                                    | <u>&lt;1e-08</u>                                                                    | <u>&lt;1e-08</u>                                                                    | <u>&lt;1e-08</u>                                                                    | <u>&lt;1e-08</u>                                                                     | <u>&lt;1e-08</u>                                                                      | <u>&lt;1e-08</u>                                                                      |
|       | PCS       | 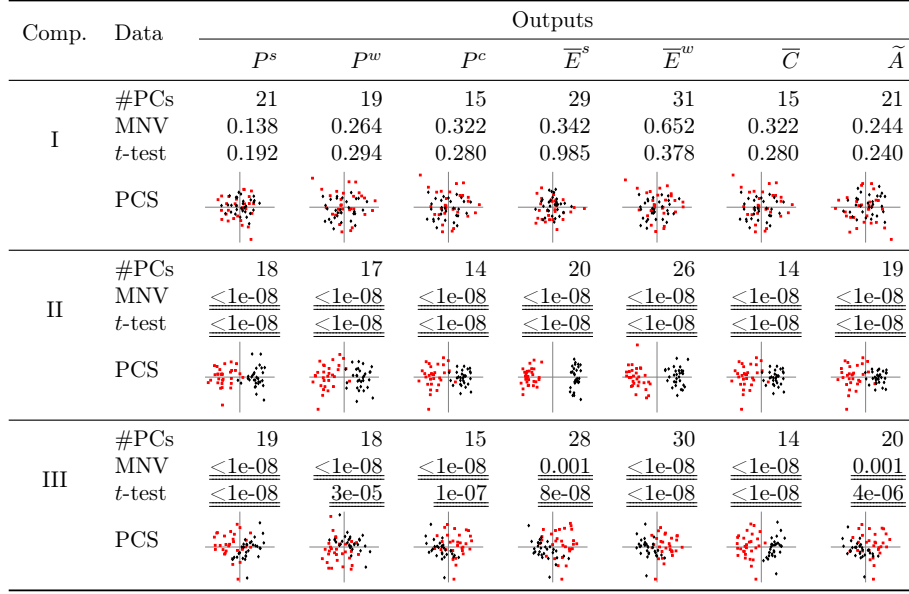   | 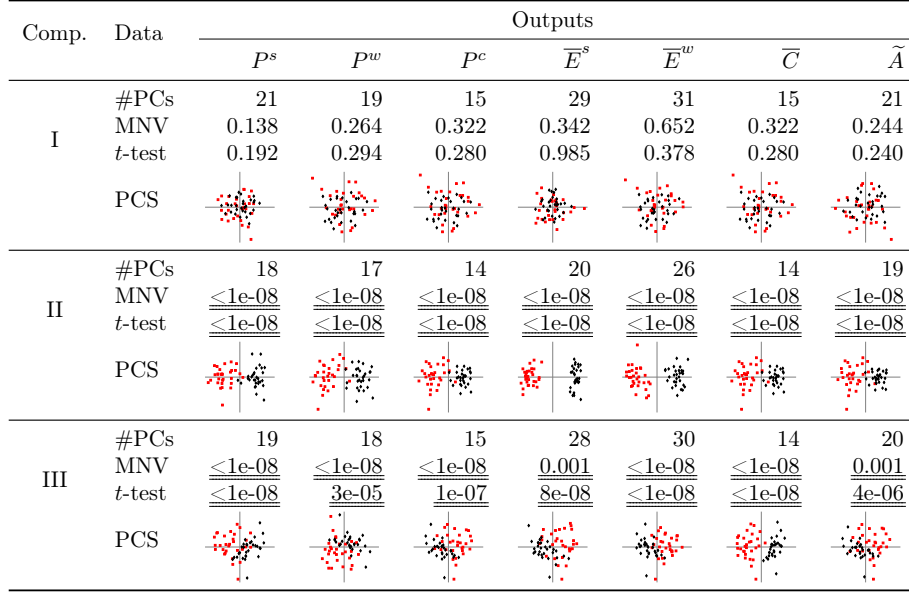   | 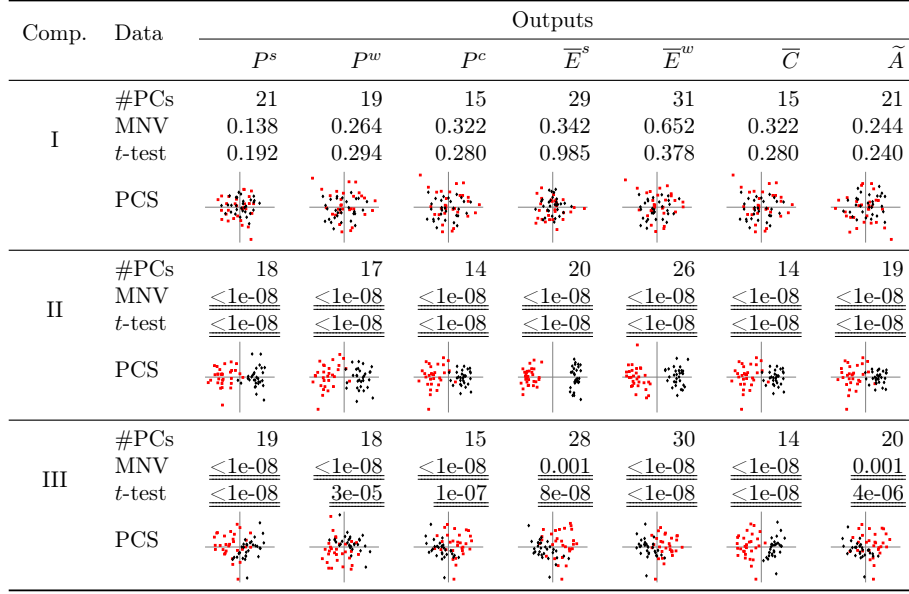   | 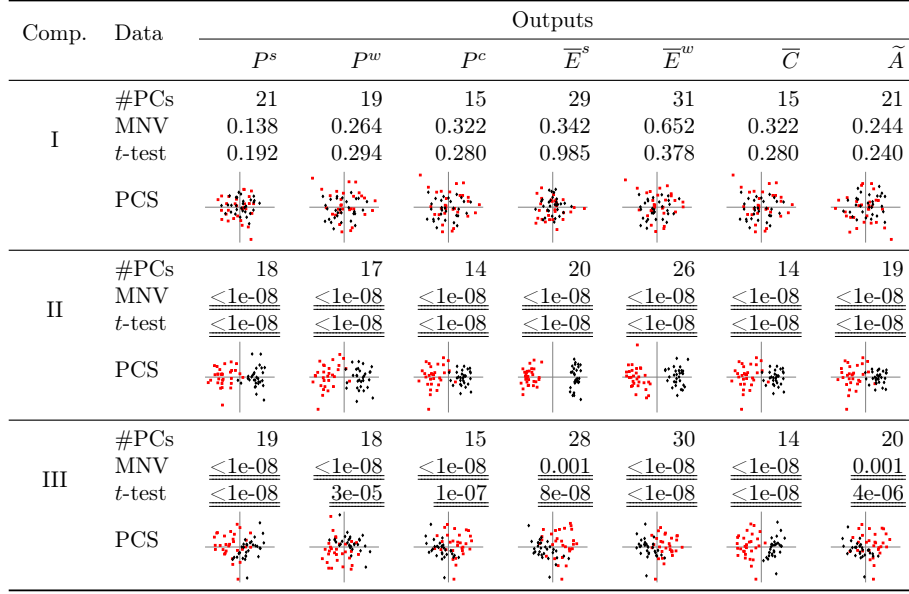   | 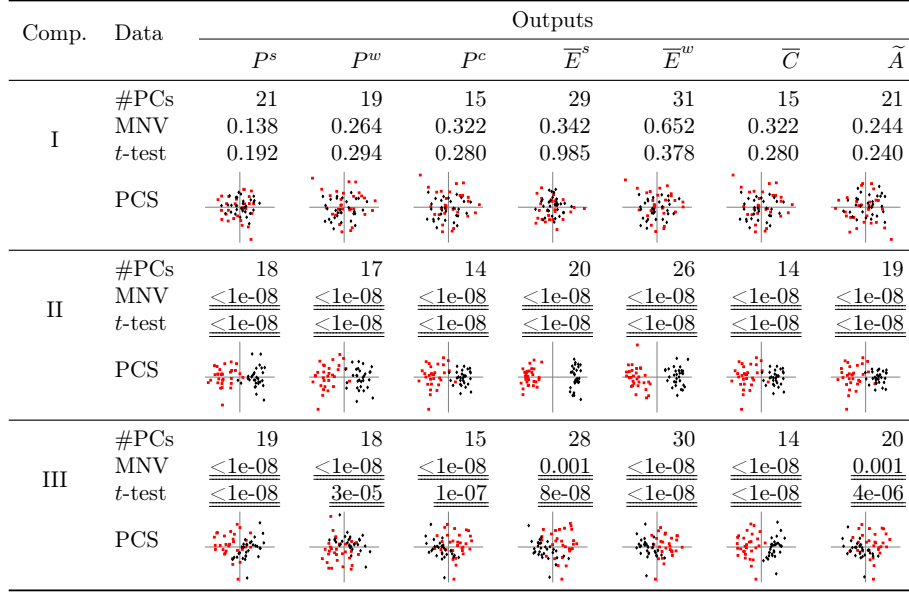   | 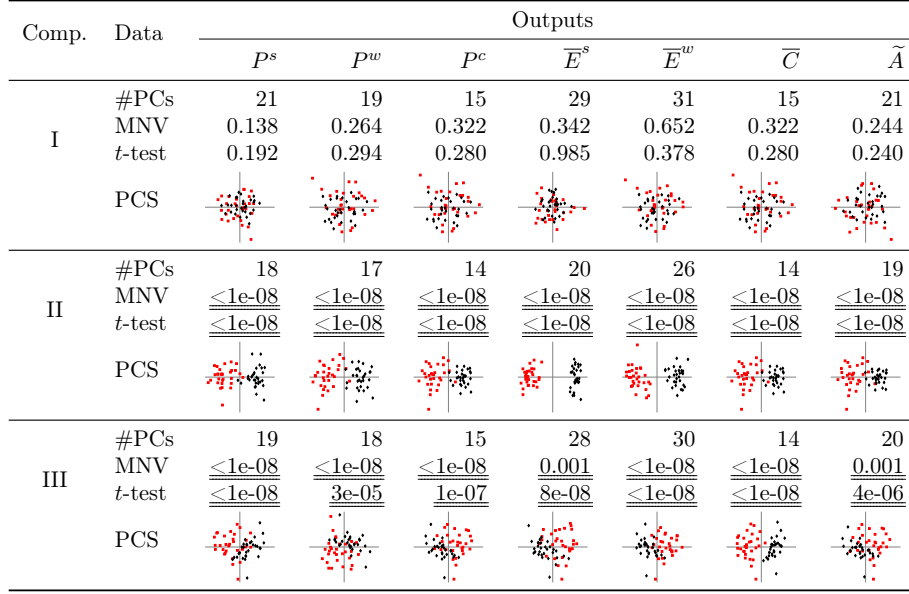   | 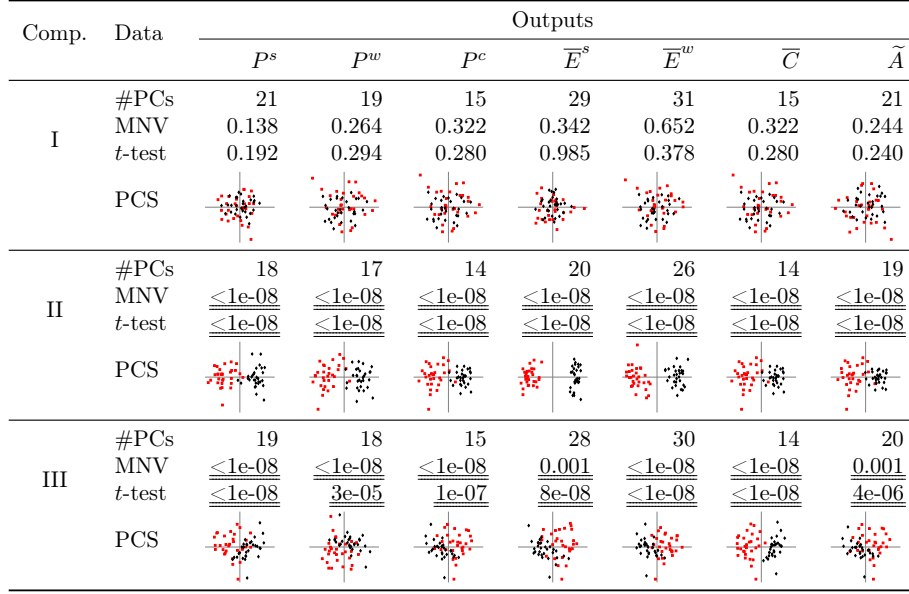   |
| III   | #PCs      | 19                                                                                  | 18                                                                                  | 15                                                                                  | 28                                                                                  | 30                                                                                   | 14                                                                                    | 20                                                                                    |
|       | MNV       | <u>&lt;1e-08</u>                                                                    | <u>&lt;1e-08</u>                                                                    | <u>&lt;1e-08</u>                                                                    | <u>0.001</u>                                                                        | <u>&lt;1e-08</u>                                                                     | <u>&lt;1e-08</u>                                                                      | <u>0.001</u>                                                                          |
|       | $t$ -test | <u>&lt;1e-08</u>                                                                    | <u>3e-05</u>                                                                        | <u>1e-07</u>                                                                        | <u>8e-08</u>                                                                        | <u>&lt;1e-08</u>                                                                     | <u>&lt;1e-08</u>                                                                      | <u>4e-06</u>                                                                          |
|       | PCS       | 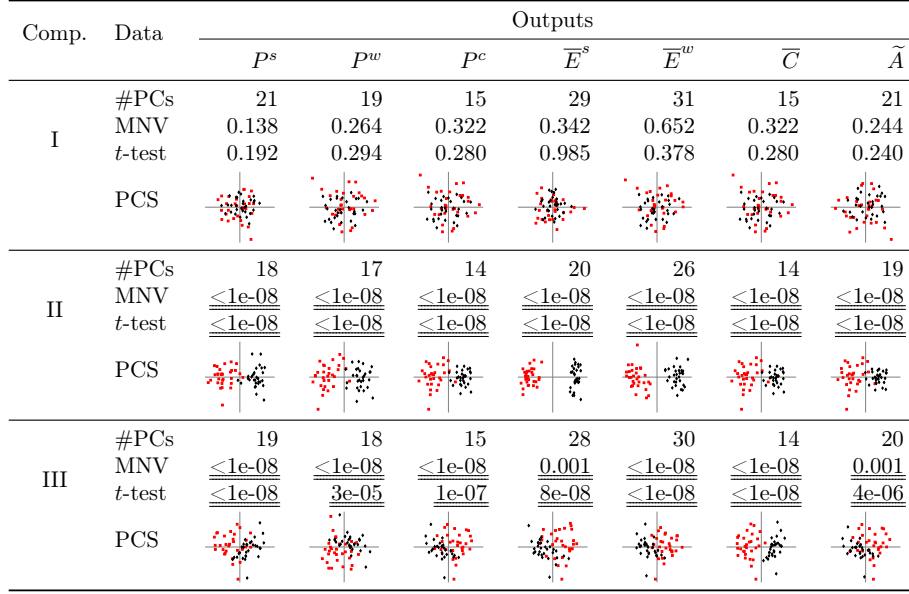 | 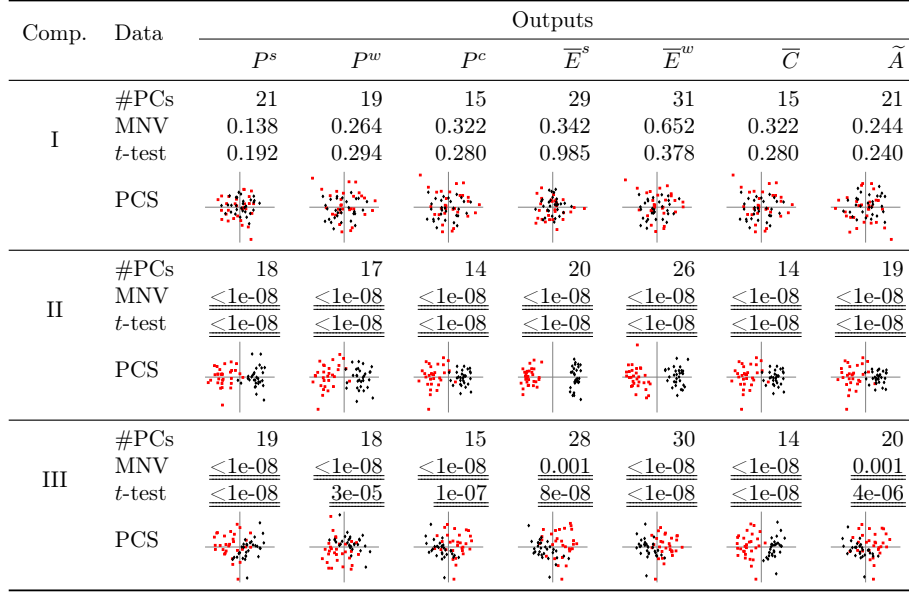 | 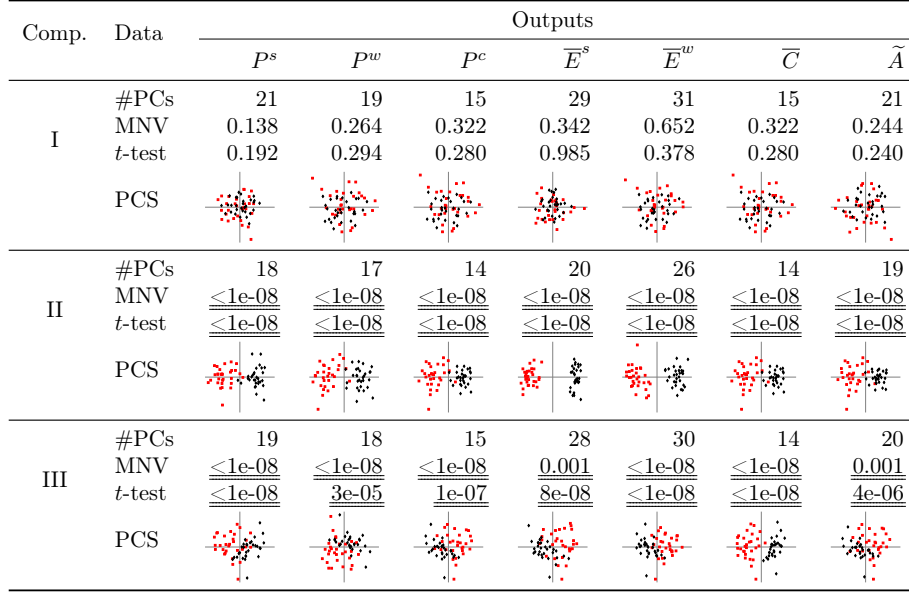 | 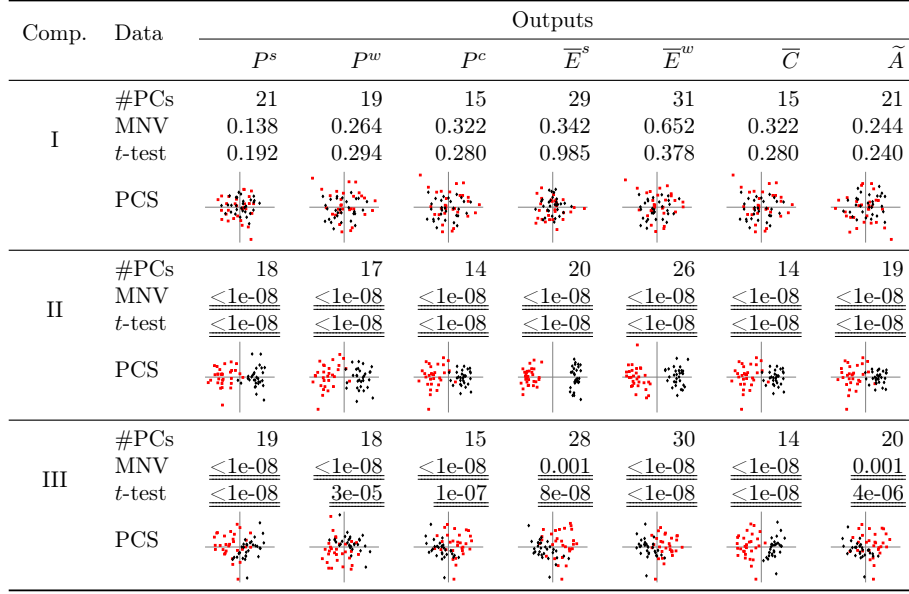 | 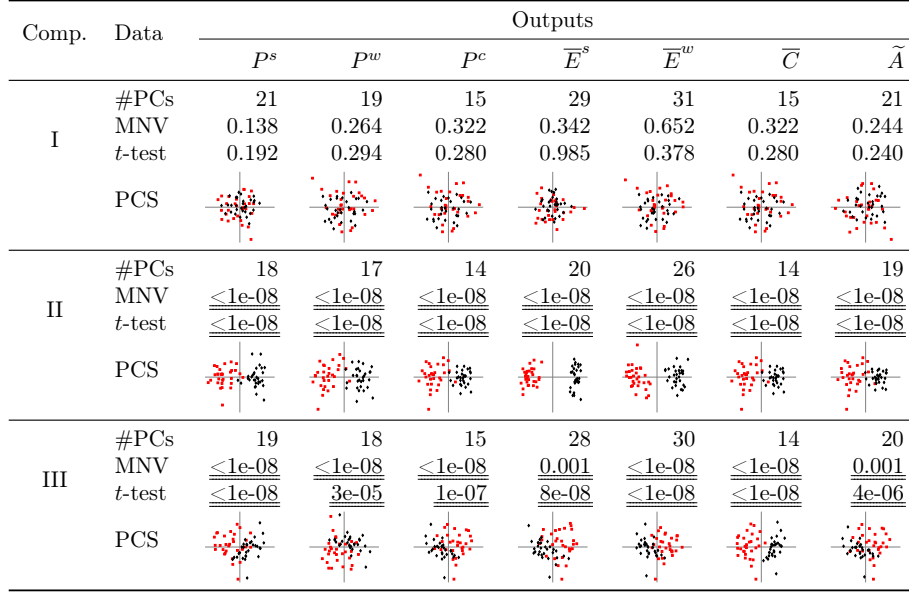 | 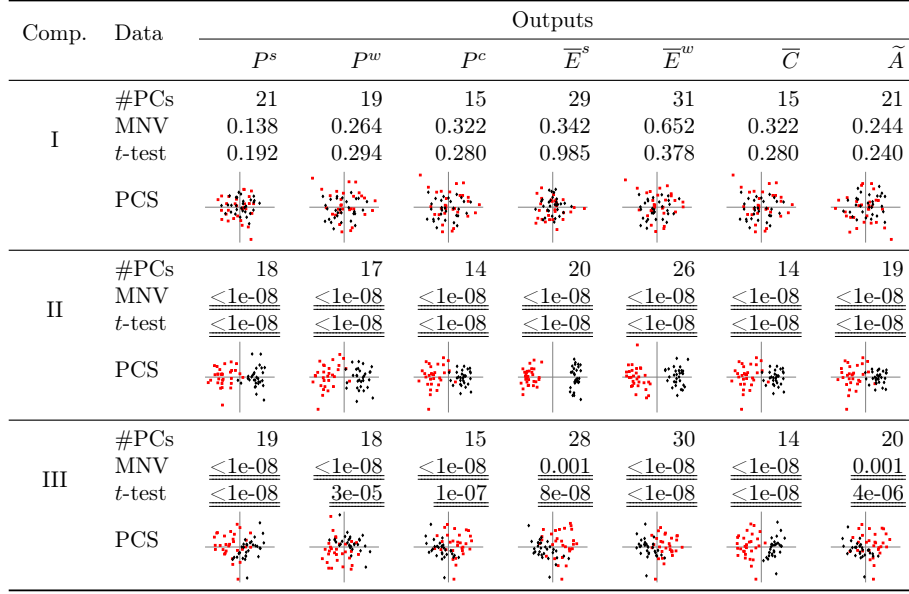 | 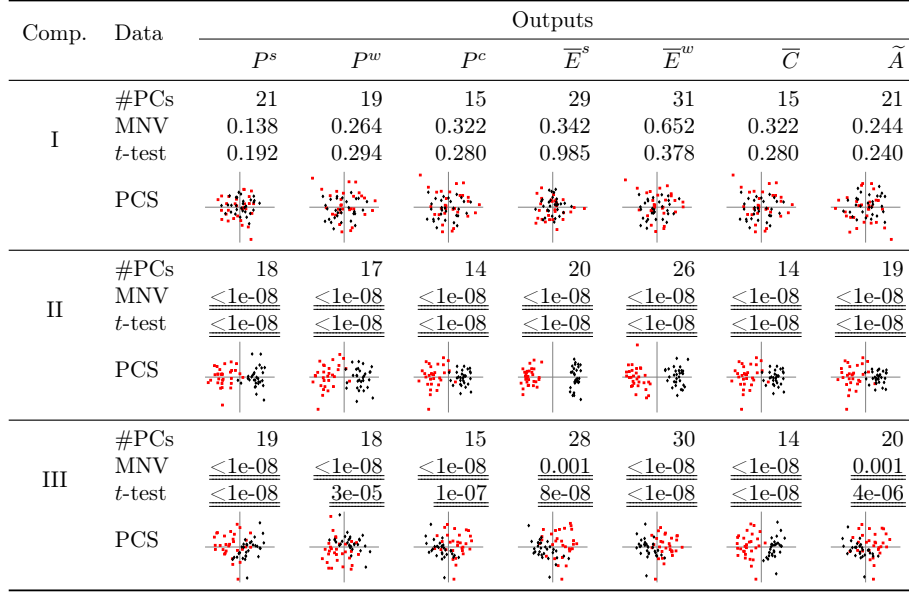 |

**Table S2.4** Model-independent comparison for model size 200, parameter set 2, and  $n = 30$  runs per configuration. Case I weights two similar setups, case II compares setups with a small implementation difference, and case III compares setups with a different parameter. #PCs is the number of PCs which explain at least 90% of variance, while MNV and  $t$ -test refer to the  $p$ -value yielded by the MANOVA (#PCs) and  $t$  (first PC) hypothesis tests, respectively. PCS shows the representation of the respective output in the first two dimensions of the PC space. Output  $\tilde{A}$  refers to the concatenation of all outputs (range scaled). The MANOVA test is not applicable to one PC, and the respective  $p$ -values are replaced with an asterisk (\*).  $P$ -values lower than 0.05 are underlined, while  $p$ -values lower than 0.01 are double-underlined.

| Comp. | Data      | Outputs                                                                             |                                                                                     |                                                                                     |                                                                                     |                                                                                      |                                                                                       |                                                                                       |
|-------|-----------|-------------------------------------------------------------------------------------|-------------------------------------------------------------------------------------|-------------------------------------------------------------------------------------|-------------------------------------------------------------------------------------|--------------------------------------------------------------------------------------|---------------------------------------------------------------------------------------|---------------------------------------------------------------------------------------|
|       |           | $P^s$                                                                               | $P^w$                                                                               | $P^c$                                                                               | $\bar{E}^s$                                                                         | $\bar{E}^w$                                                                          | $\bar{C}$                                                                             | $\tilde{A}$                                                                           |
| I     | #PCs      | 24                                                                                  | 32                                                                                  | 25                                                                                  | 36                                                                                  | 43                                                                                   | 26                                                                                    | 39                                                                                    |
|       | MNV       | 0.528                                                                               | 0.258                                                                               | 0.548                                                                               | 0.105                                                                               | 0.746                                                                                | 0.577                                                                                 | 0.704                                                                                 |
|       | $t$ -test | 0.530                                                                               | 0.836                                                                               | 0.804                                                                               | 0.784                                                                               | 0.378                                                                                | 0.805                                                                                 | 0.879                                                                                 |
|       | PCS       | 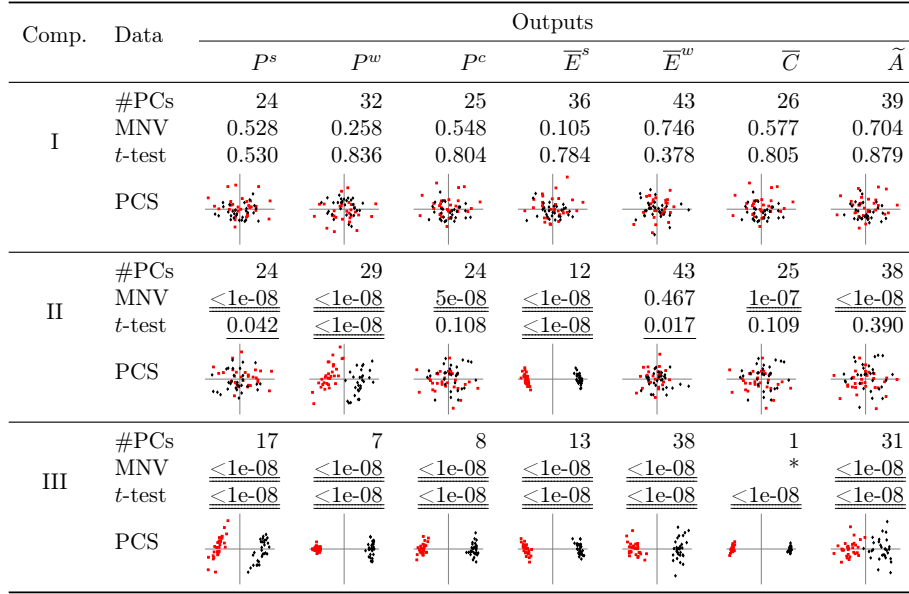   | 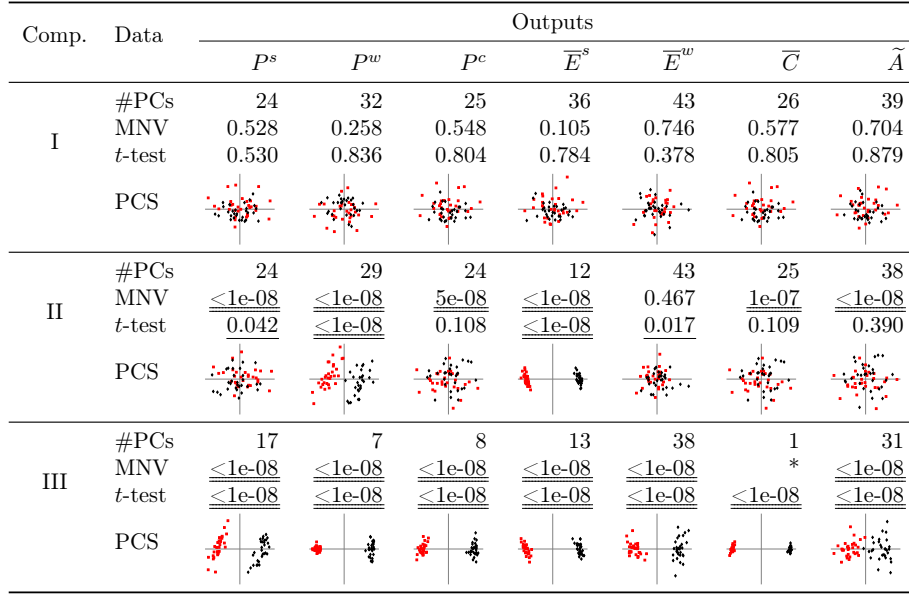   | 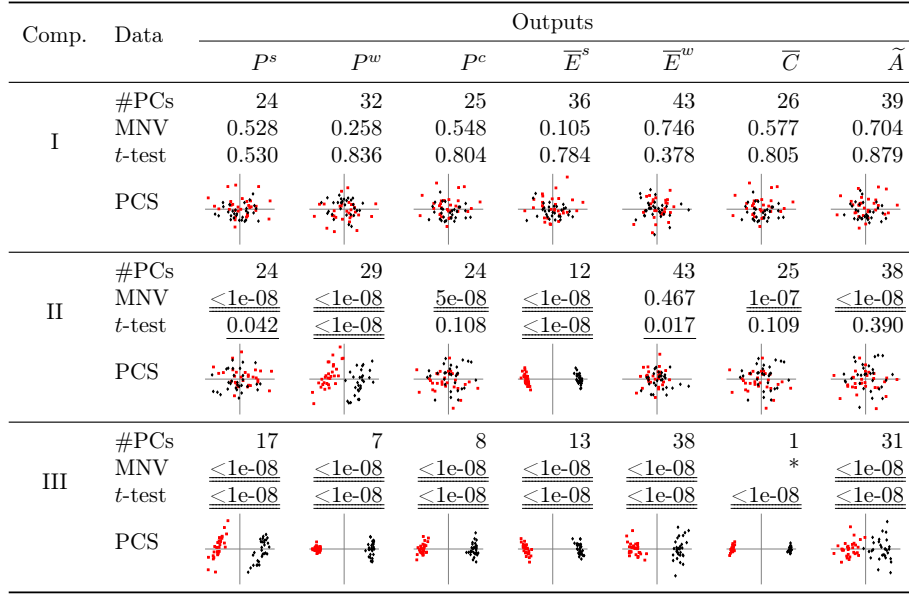   | 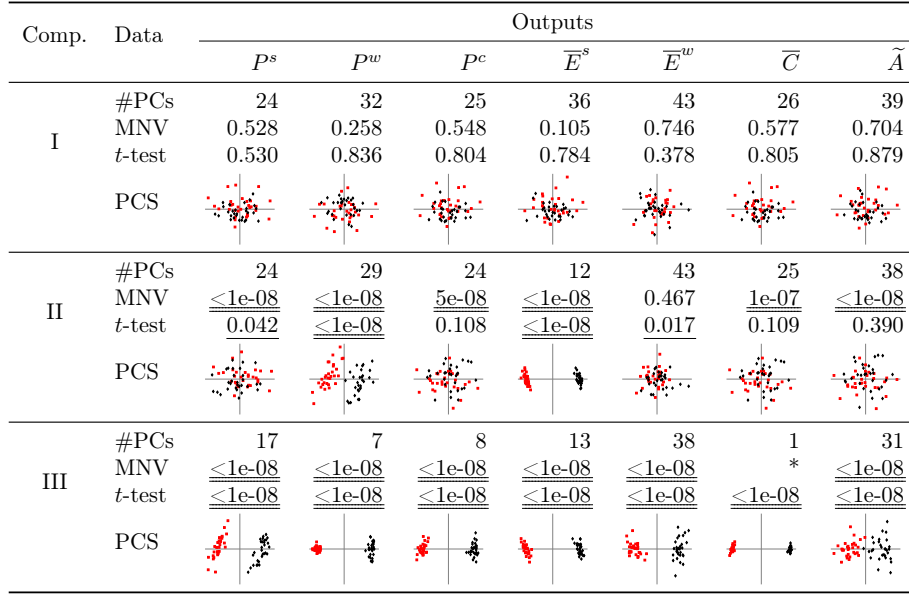   | 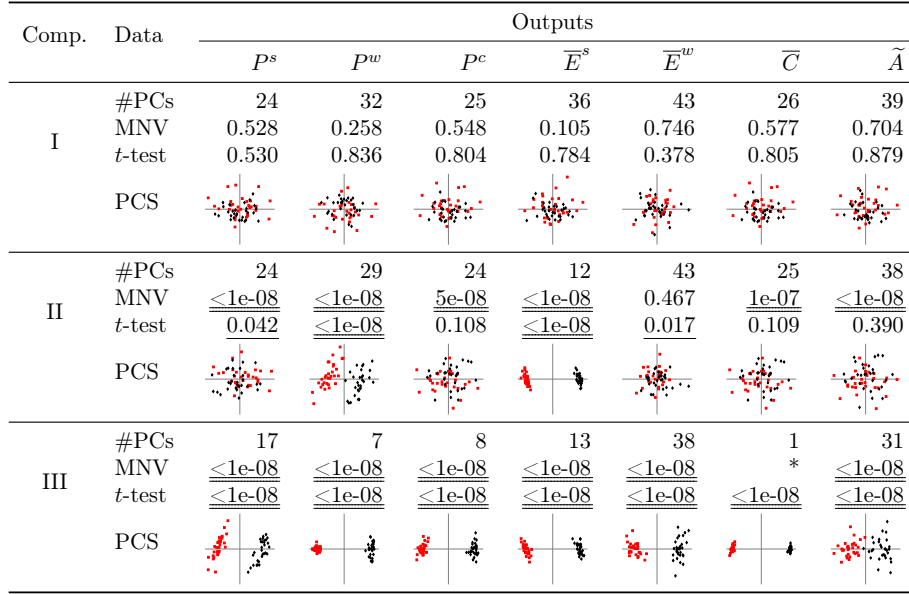   | 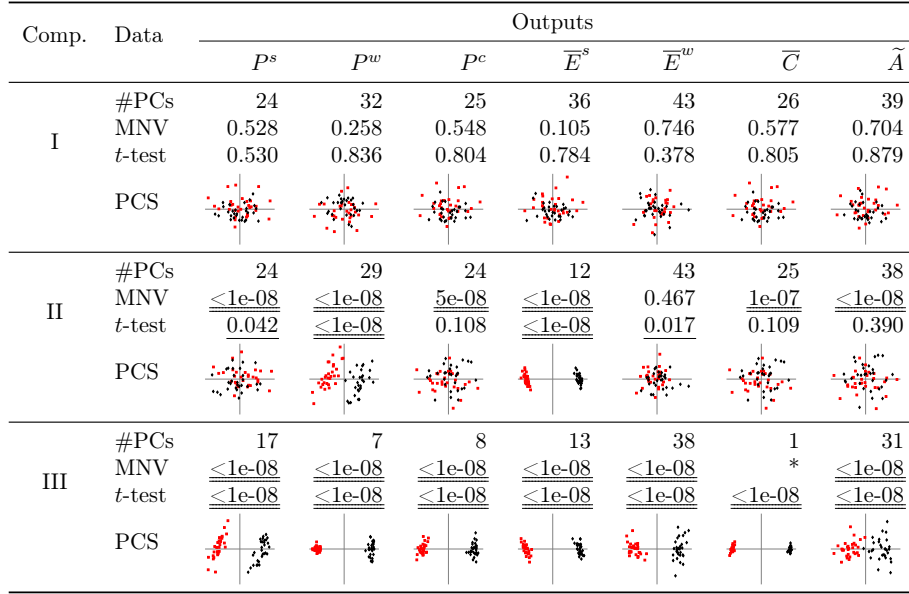   | 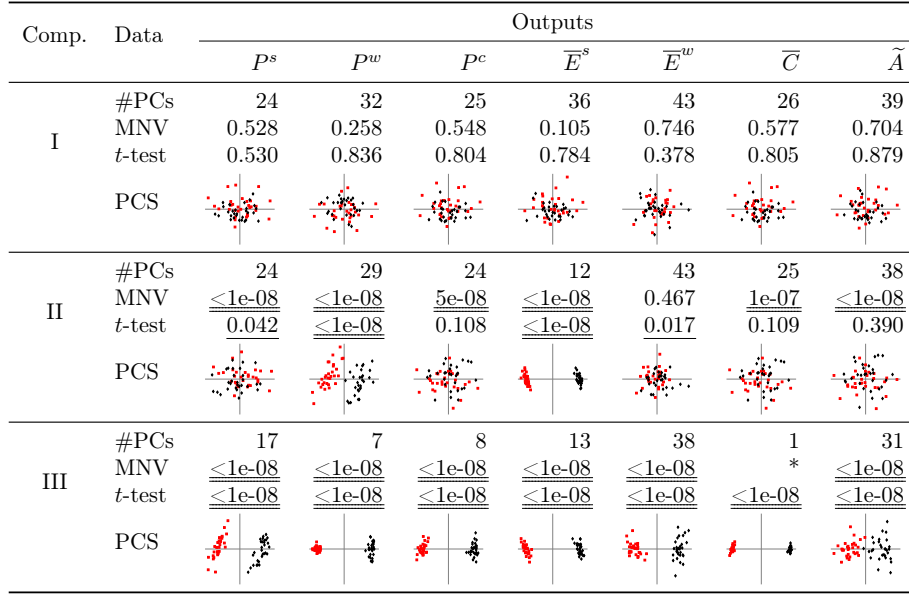   |
| II    | #PCs      | 24                                                                                  | 29                                                                                  | 24                                                                                  | 12                                                                                  | 43                                                                                   | 25                                                                                    | 38                                                                                    |
|       | MNV       | <u>&lt;1e-08</u>                                                                    | <u>&lt;1e-08</u>                                                                    | <u>5e-08</u>                                                                        | <u>&lt;1e-08</u>                                                                    | 0.467                                                                                | <u>1e-07</u>                                                                          | <u>&lt;1e-08</u>                                                                      |
|       | $t$ -test | <u>0.042</u>                                                                        | <u>&lt;1e-08</u>                                                                    | 0.108                                                                               | <u>&lt;1e-08</u>                                                                    | 0.017                                                                                | 0.109                                                                                 | 0.390                                                                                 |
|       | PCS       | 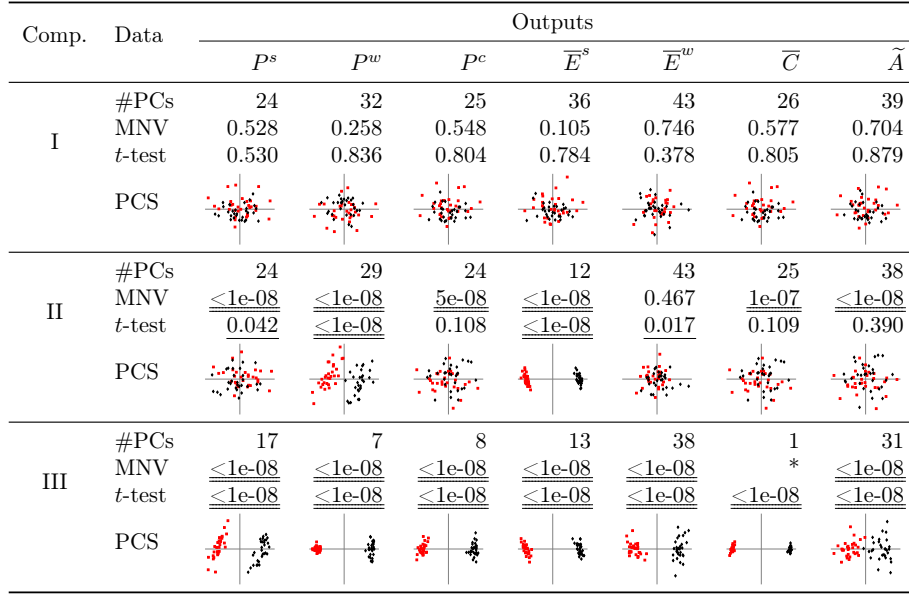   | 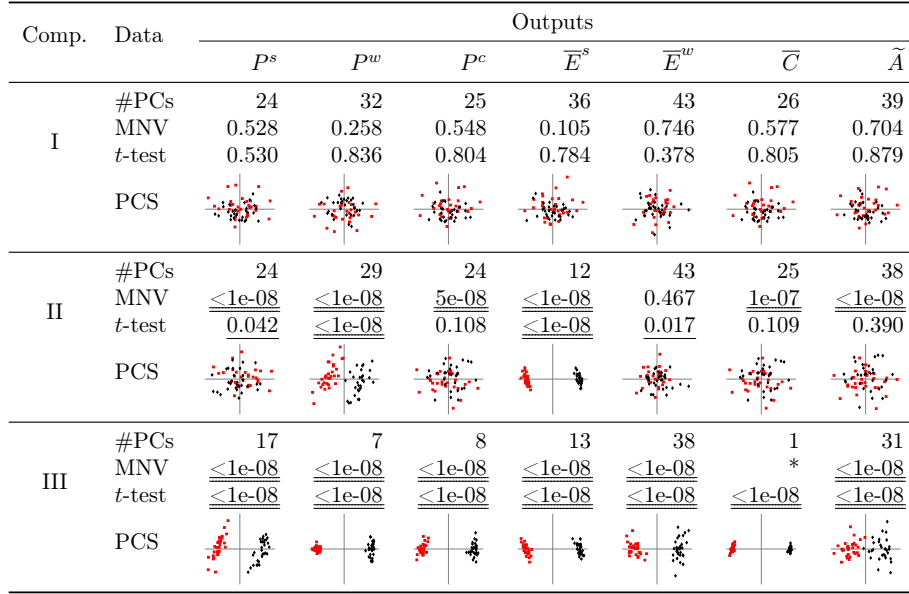   | 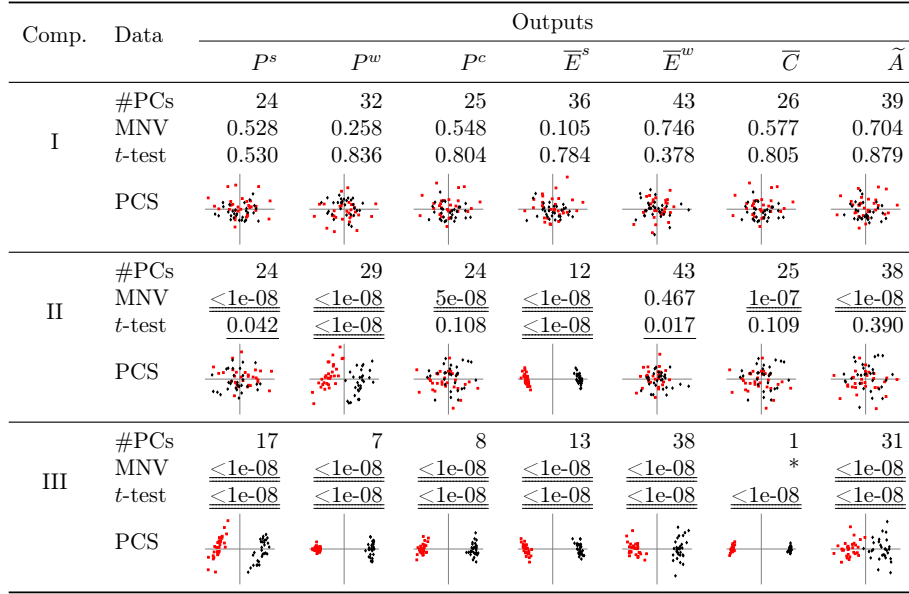   | 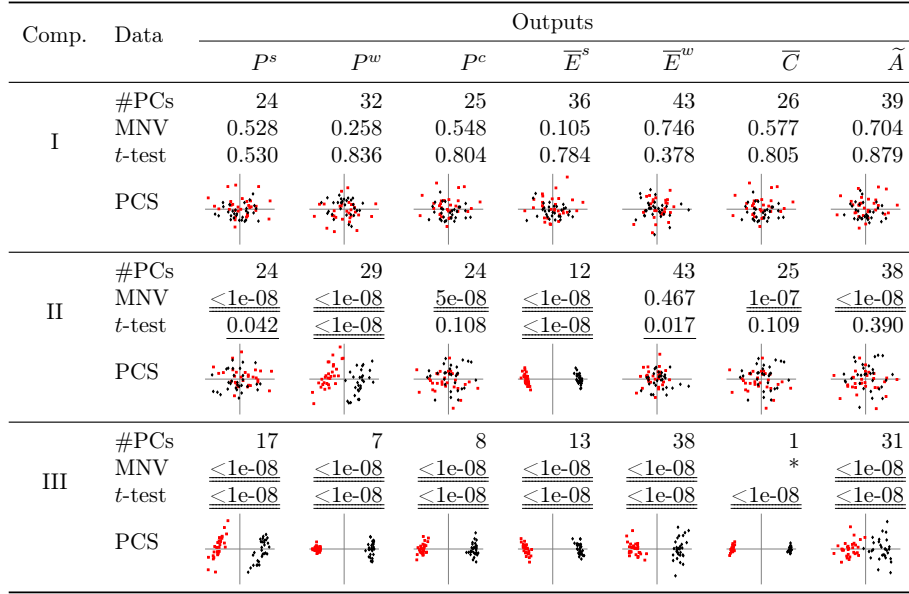   | 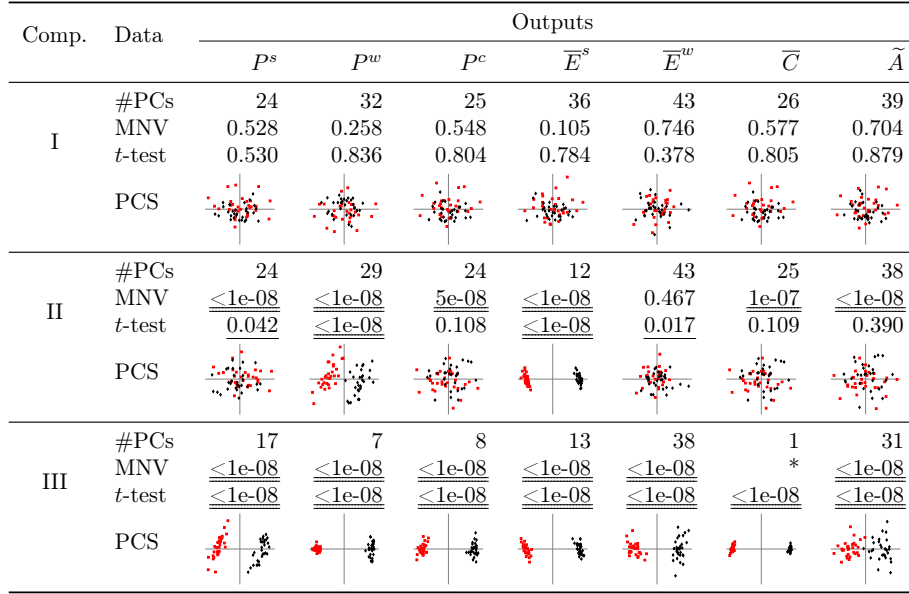   | 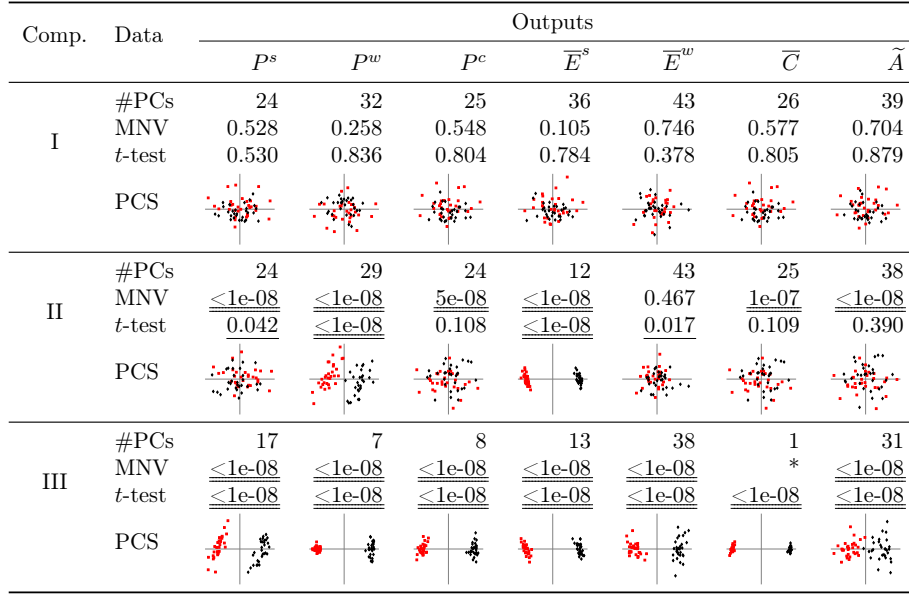   | 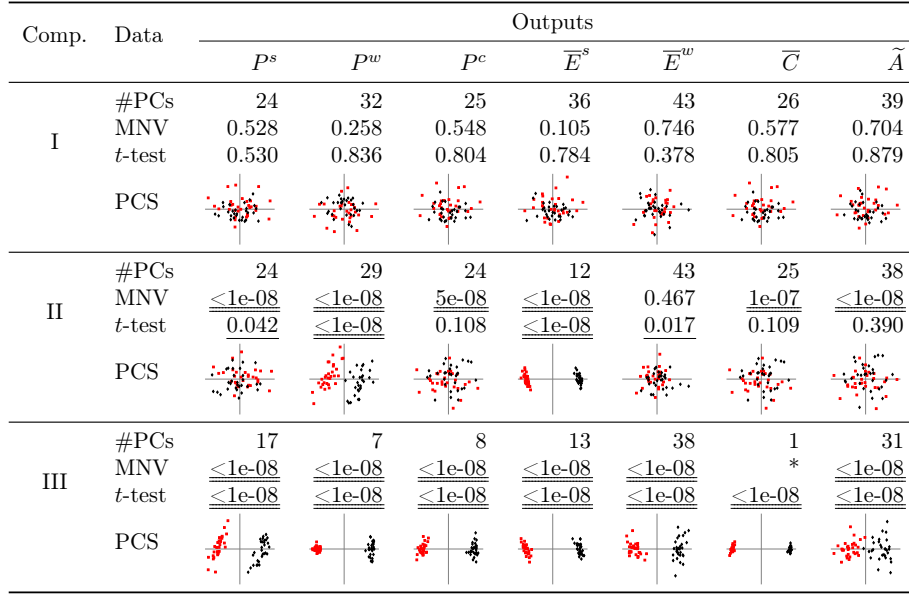   |
| III   | #PCs      | 17                                                                                  | 7                                                                                   | 8                                                                                   | 13                                                                                  | 38                                                                                   | 1                                                                                     | 31                                                                                    |
|       | MNV       | <u>&lt;1e-08</u>                                                                    | <u>&lt;1e-08</u>                                                                    | <u>&lt;1e-08</u>                                                                    | <u>&lt;1e-08</u>                                                                    | <u>&lt;1e-08</u>                                                                     | *                                                                                     | <u>&lt;1e-08</u>                                                                      |
|       | $t$ -test | <u>&lt;1e-08</u>                                                                    | <u>&lt;1e-08</u>                                                                    | <u>&lt;1e-08</u>                                                                    | <u>&lt;1e-08</u>                                                                    | <u>&lt;1e-08</u>                                                                     | <u>&lt;1e-08</u>                                                                      | <u>&lt;1e-08</u>                                                                      |
|       | PCS       | 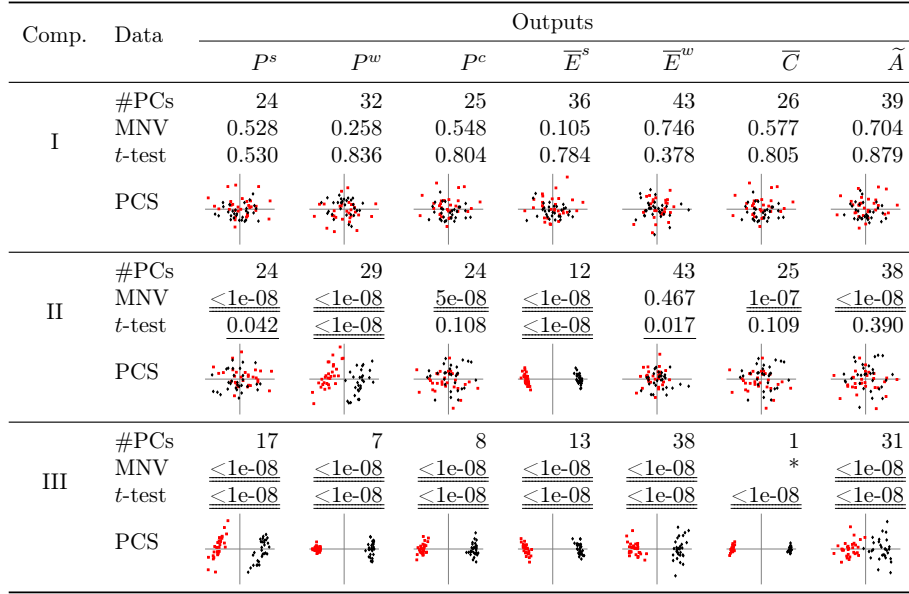 | 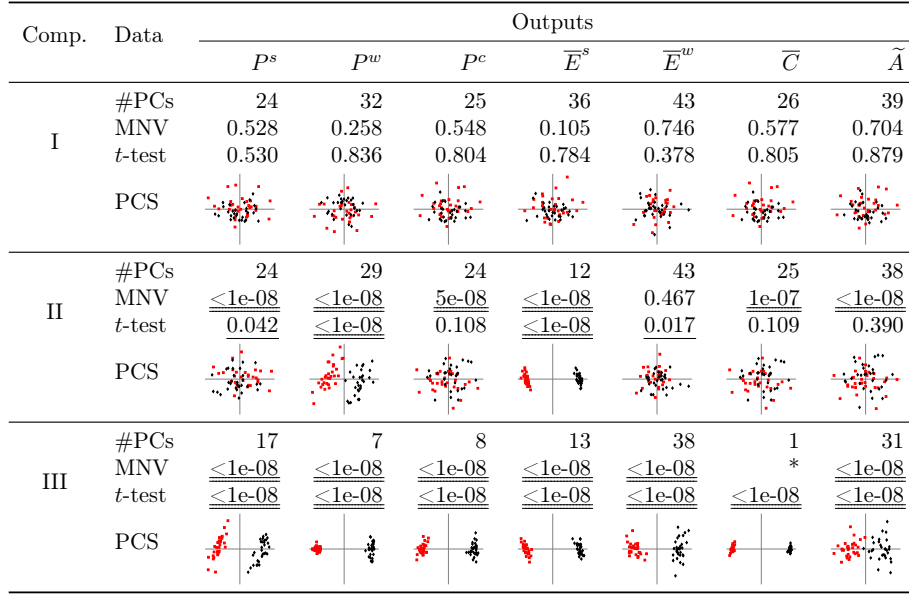 | 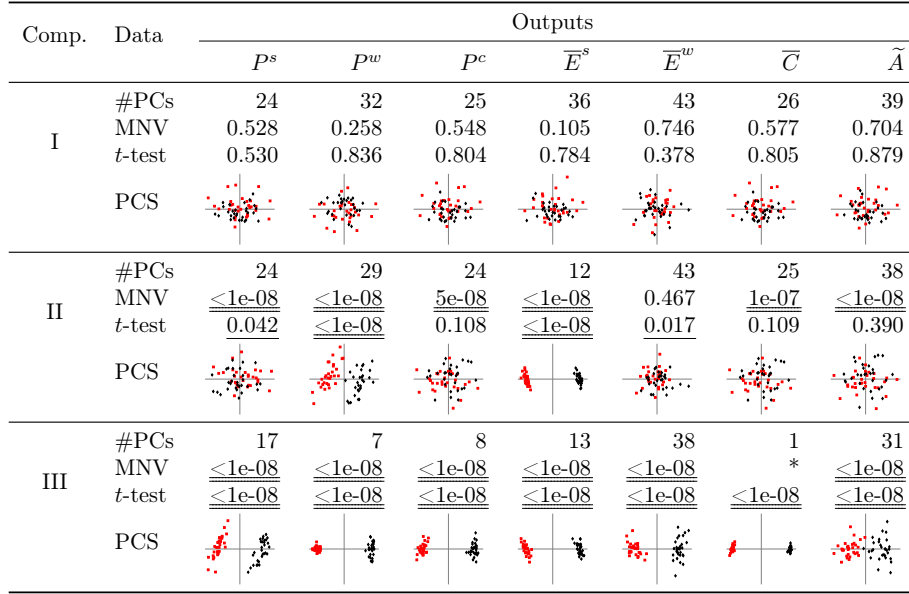 | 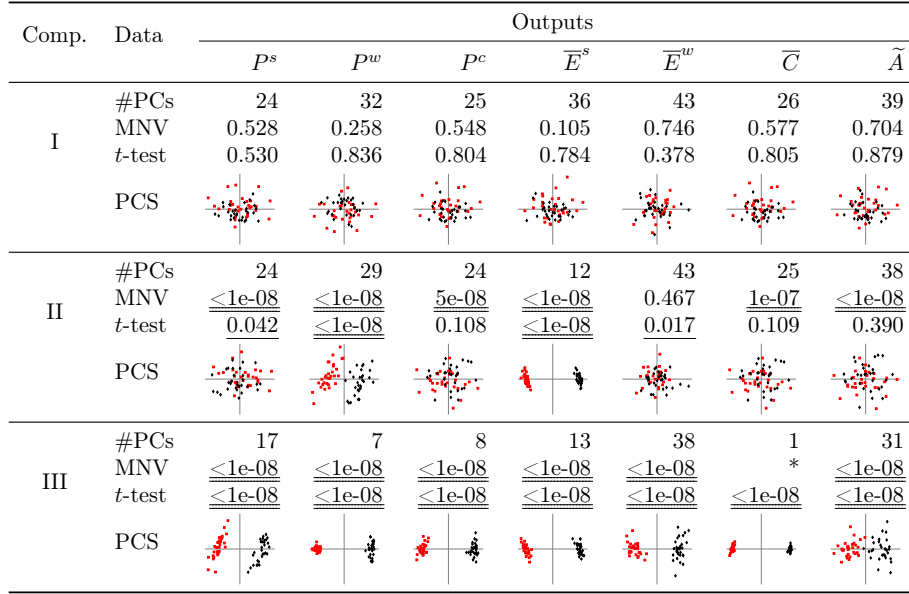 | 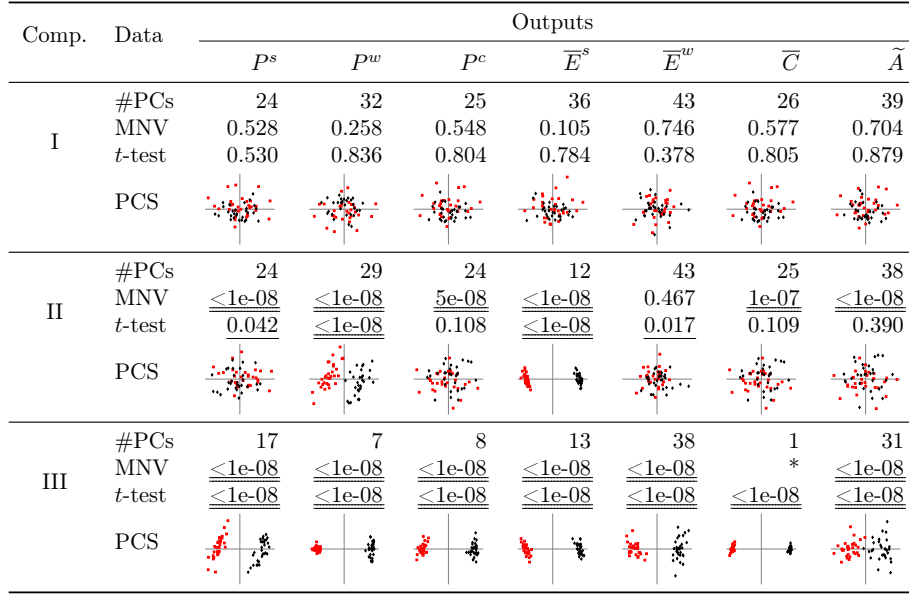 | 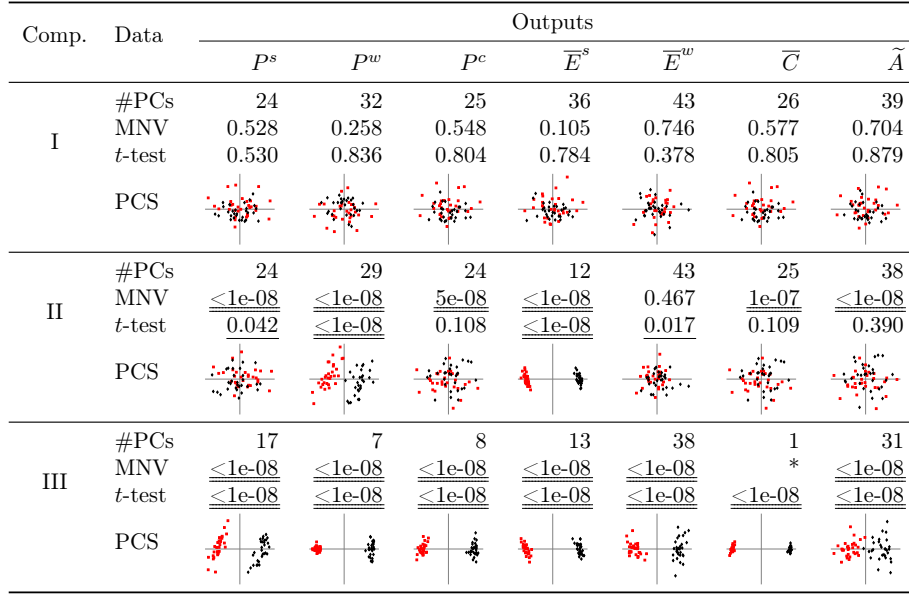 | 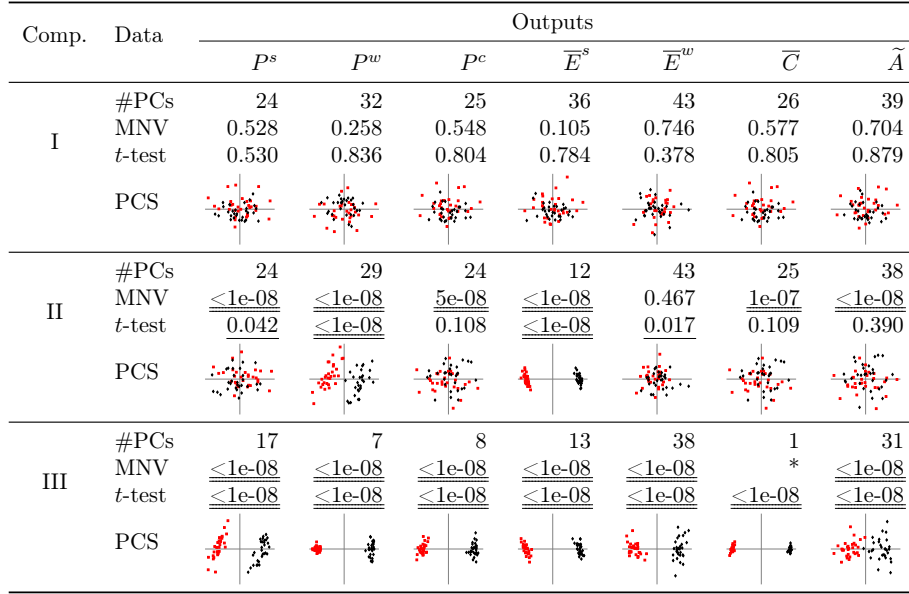 |

**Table S2.5** Model-independent comparison for model size 400, parameter set 1, and  $n = 30$  runs per configuration. Case I weights two similar setups, case II compares setups with a small implementation difference, and case III compares setups with a different parameter. #PCs is the number of PCs which explain at least 90% of variance, while MNV and  $t$ -test refer to the  $p$ -value yielded by the MANOVA (#PCs) and  $t$  (first PC) hypothesis tests, respectively. PCS shows the representation of the respective output in the first two dimensions of the PC space. Output  $\tilde{A}$  refers to the concatenation of all outputs (range scaled). The MANOVA test is not applicable to one PC, and the respective  $p$ -values are replaced with an asterisk (\*).  $P$ -values lower than 0.05 are underlined, while  $p$ -values lower than 0.01 are double-underlined.

| Comp. | Data      | Outputs                                                                             |                                                                                     |                                                                                     |                                                                                     |                                                                                      |                                                                                       |                                                                                       |
|-------|-----------|-------------------------------------------------------------------------------------|-------------------------------------------------------------------------------------|-------------------------------------------------------------------------------------|-------------------------------------------------------------------------------------|--------------------------------------------------------------------------------------|---------------------------------------------------------------------------------------|---------------------------------------------------------------------------------------|
|       |           | $P^s$                                                                               | $P^w$                                                                               | $P^c$                                                                               | $\bar{E}^s$                                                                         | $\bar{E}^w$                                                                          | $\bar{C}$                                                                             | $\tilde{A}$                                                                           |
| I     | #PCs      | 21                                                                                  | 18                                                                                  | 15                                                                                  | 28                                                                                  | 32                                                                                   | 15                                                                                    | 21                                                                                    |
|       | MNV       | 0.740                                                                               | 0.936                                                                               | 0.849                                                                               | 0.776                                                                               | 0.854                                                                                | 0.850                                                                                 | 0.990                                                                                 |
|       | $t$ -test | 0.919                                                                               | 0.925                                                                               | 0.942                                                                               | 0.856                                                                               | 0.778                                                                                | 0.941                                                                                 | 0.992                                                                                 |
|       | PCS       | 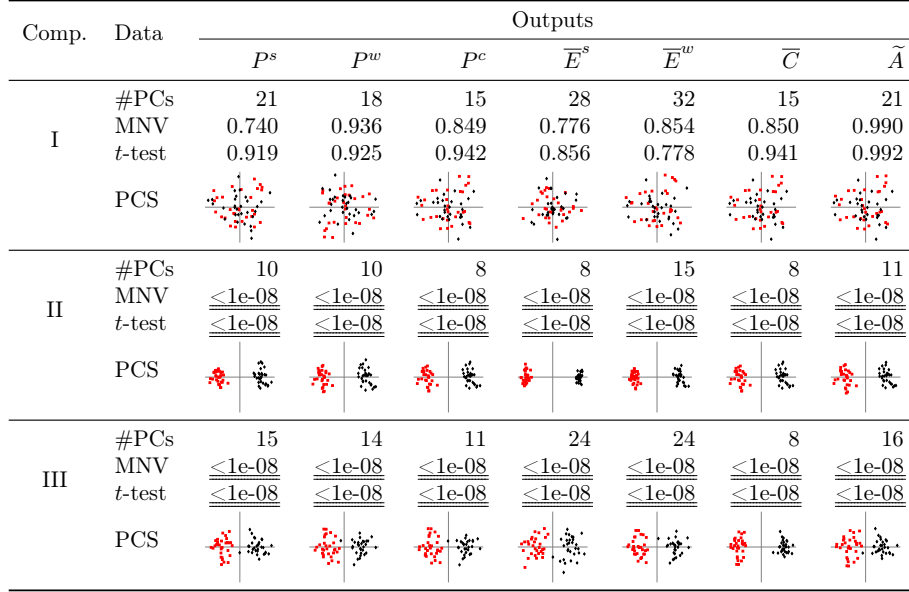   | 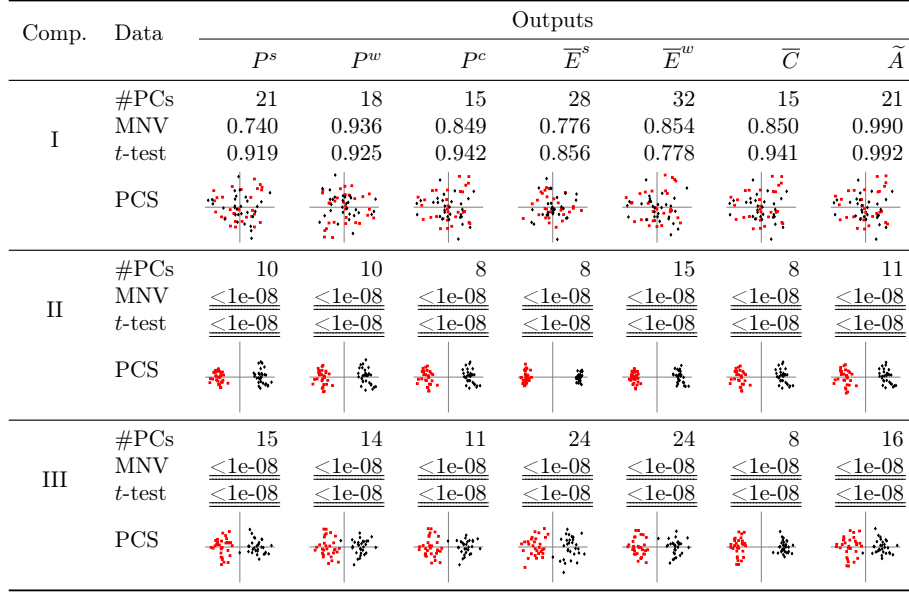   | 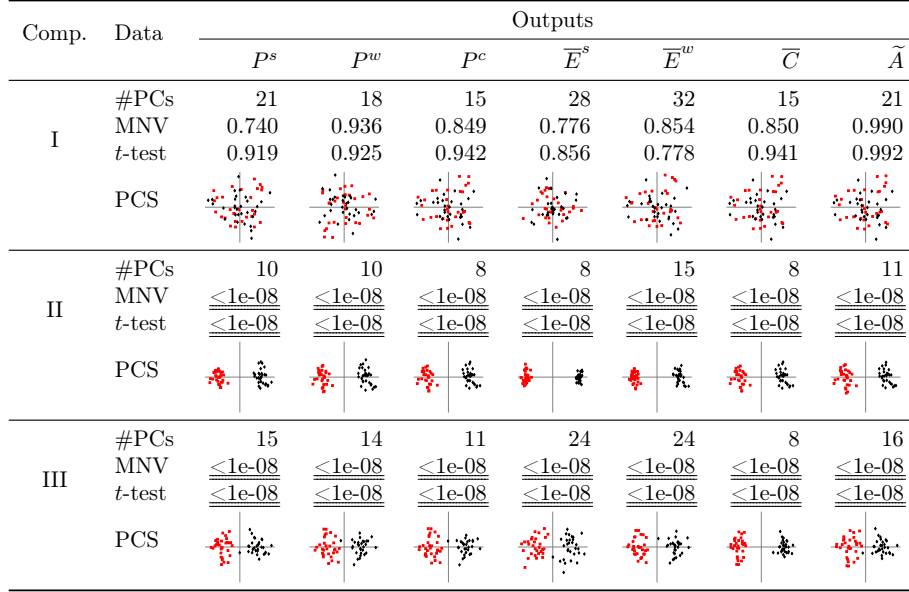   | 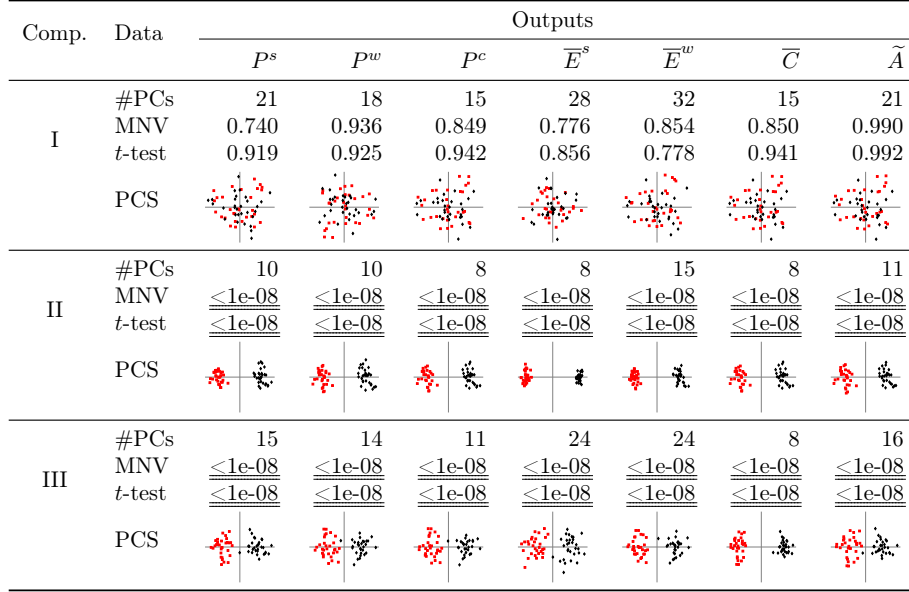   | 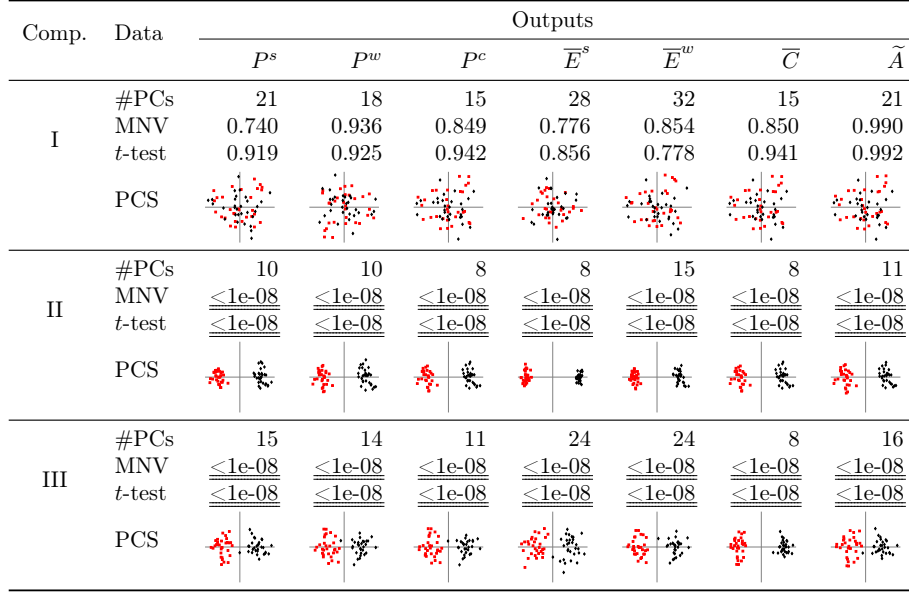   | 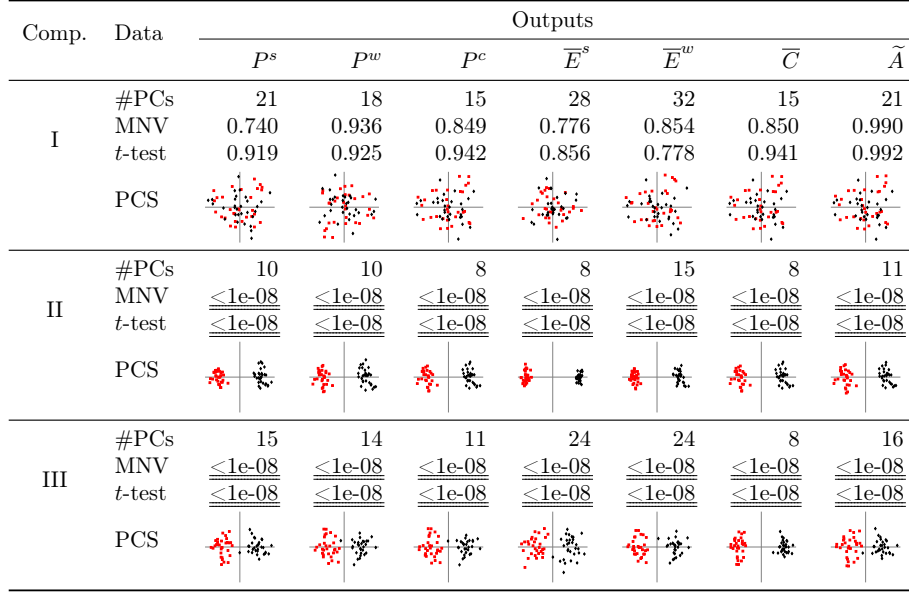   | 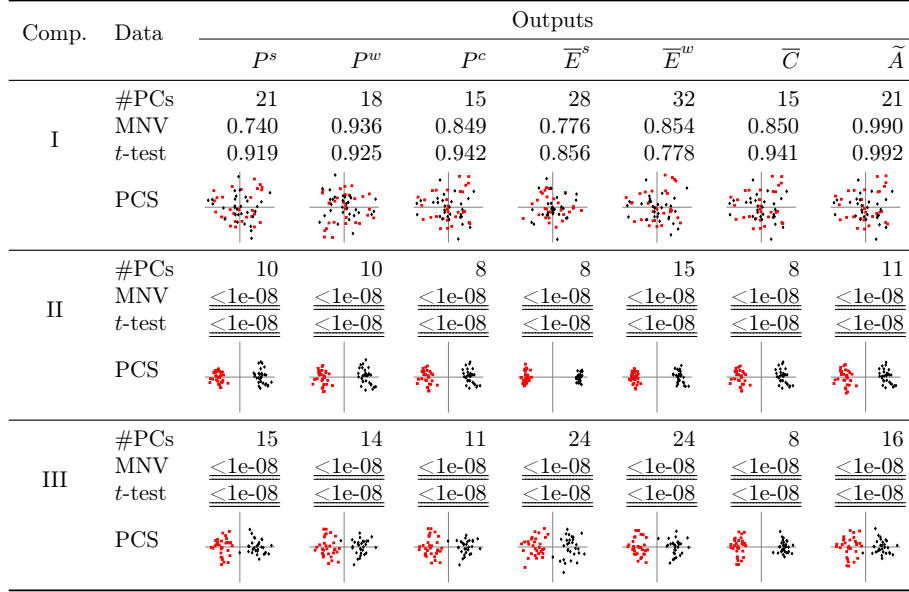   |
| II    | #PCs      | 10                                                                                  | 10                                                                                  | 8                                                                                   | 8                                                                                   | 15                                                                                   | 8                                                                                     | 11                                                                                    |
|       | MNV       | <u>&lt;1e-08</u>                                                                    | <u>&lt;1e-08</u>                                                                    | <u>&lt;1e-08</u>                                                                    | <u>&lt;1e-08</u>                                                                    | <u>&lt;1e-08</u>                                                                     | <u>&lt;1e-08</u>                                                                      | <u>&lt;1e-08</u>                                                                      |
|       | $t$ -test | <u>&lt;1e-08</u>                                                                    | <u>&lt;1e-08</u>                                                                    | <u>&lt;1e-08</u>                                                                    | <u>&lt;1e-08</u>                                                                    | <u>&lt;1e-08</u>                                                                     | <u>&lt;1e-08</u>                                                                      | <u>&lt;1e-08</u>                                                                      |
|       | PCS       | 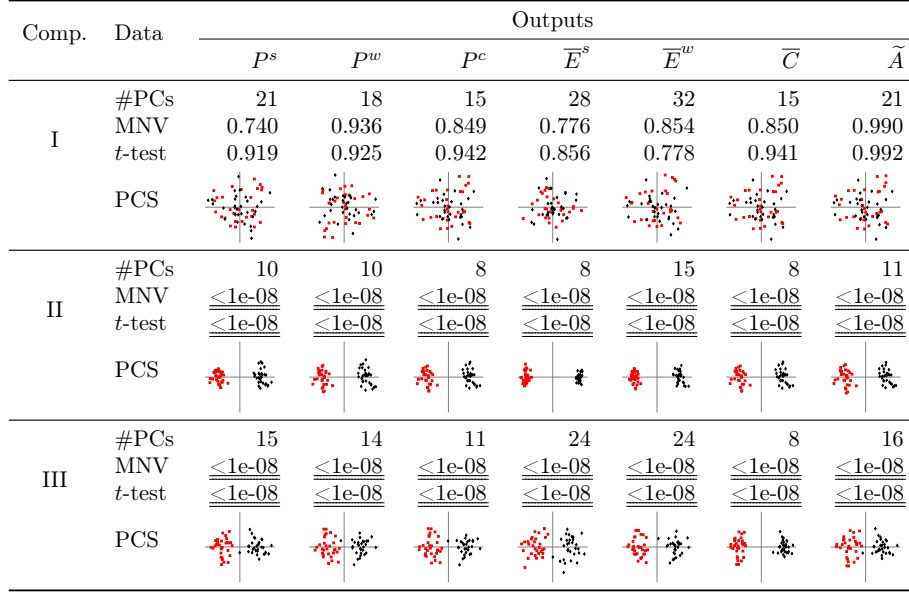   | 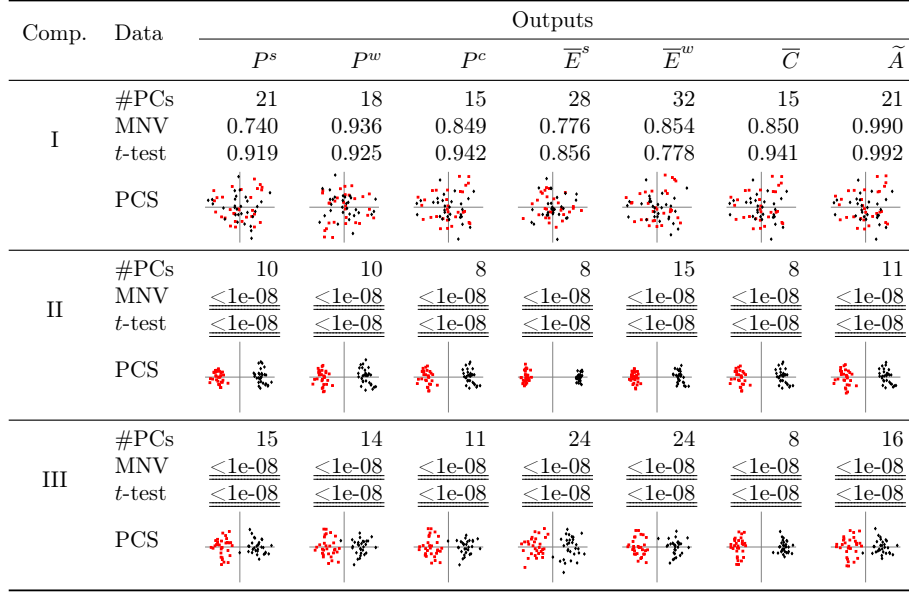   | 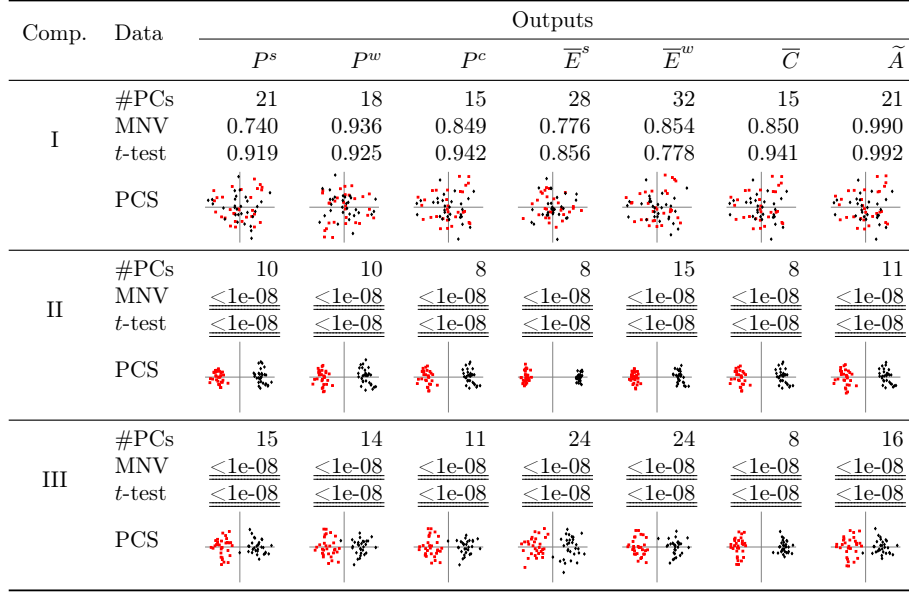   | 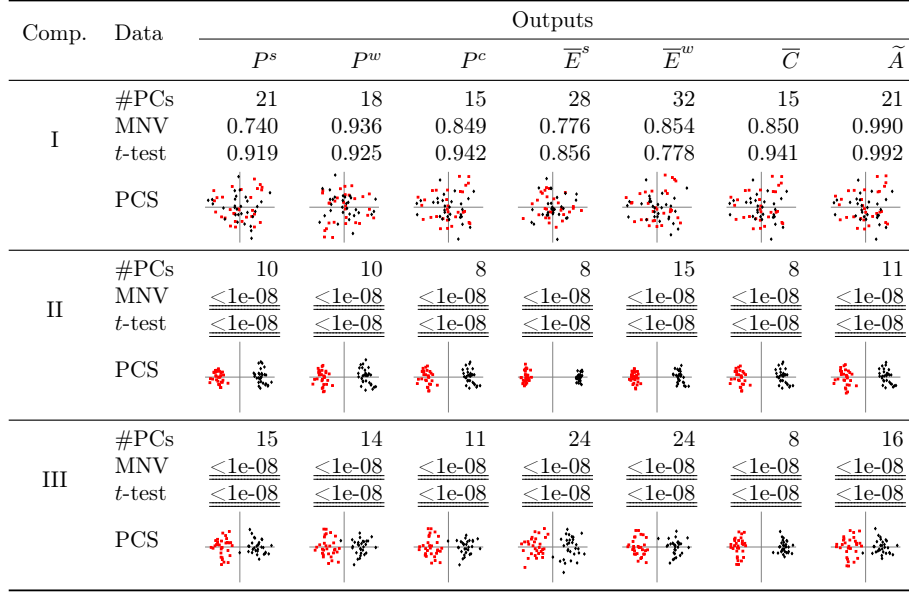   | 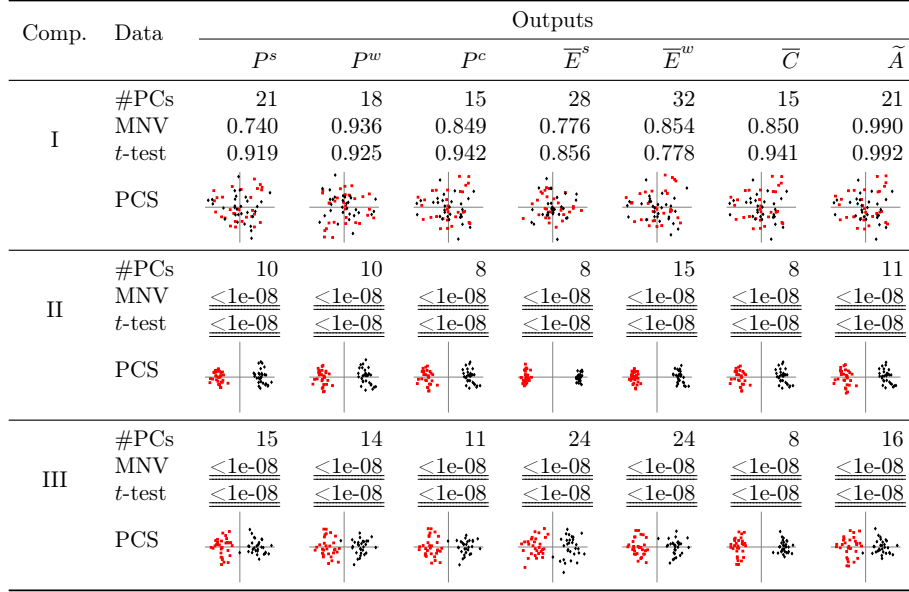   | 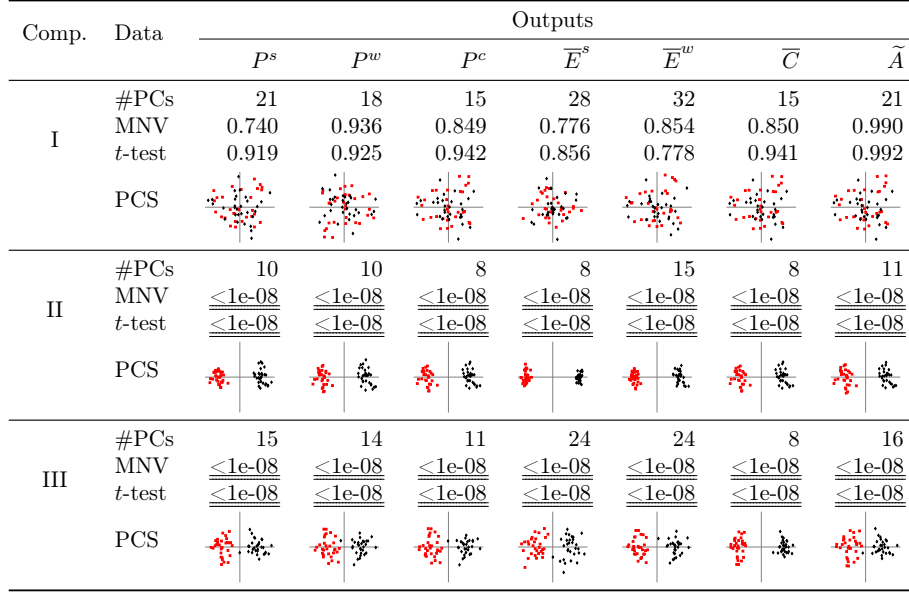   | 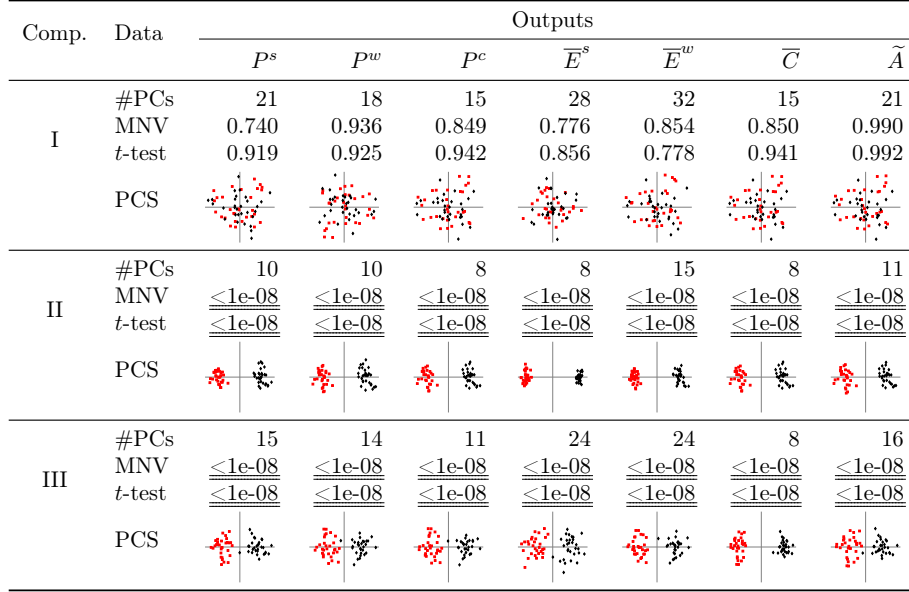   |
| III   | #PCs      | 15                                                                                  | 14                                                                                  | 11                                                                                  | 24                                                                                  | 24                                                                                   | 8                                                                                     | 16                                                                                    |
|       | MNV       | <u>&lt;1e-08</u>                                                                    | <u>&lt;1e-08</u>                                                                    | <u>&lt;1e-08</u>                                                                    | <u>&lt;1e-08</u>                                                                    | <u>&lt;1e-08</u>                                                                     | <u>&lt;1e-08</u>                                                                      | <u>&lt;1e-08</u>                                                                      |
|       | $t$ -test | <u>&lt;1e-08</u>                                                                    | <u>&lt;1e-08</u>                                                                    | <u>&lt;1e-08</u>                                                                    | <u>&lt;1e-08</u>                                                                    | <u>&lt;1e-08</u>                                                                     | <u>&lt;1e-08</u>                                                                      | <u>&lt;1e-08</u>                                                                      |
|       | PCS       | 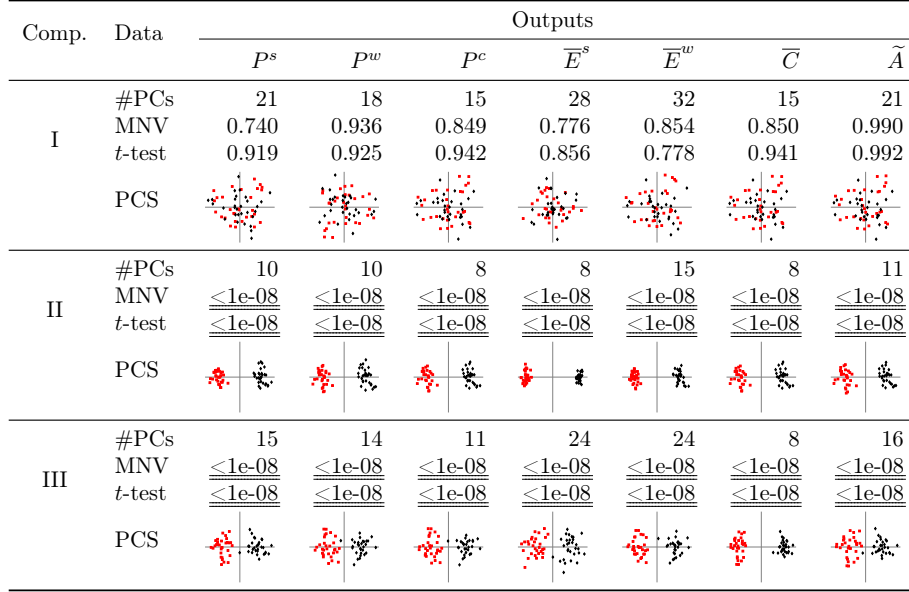 | 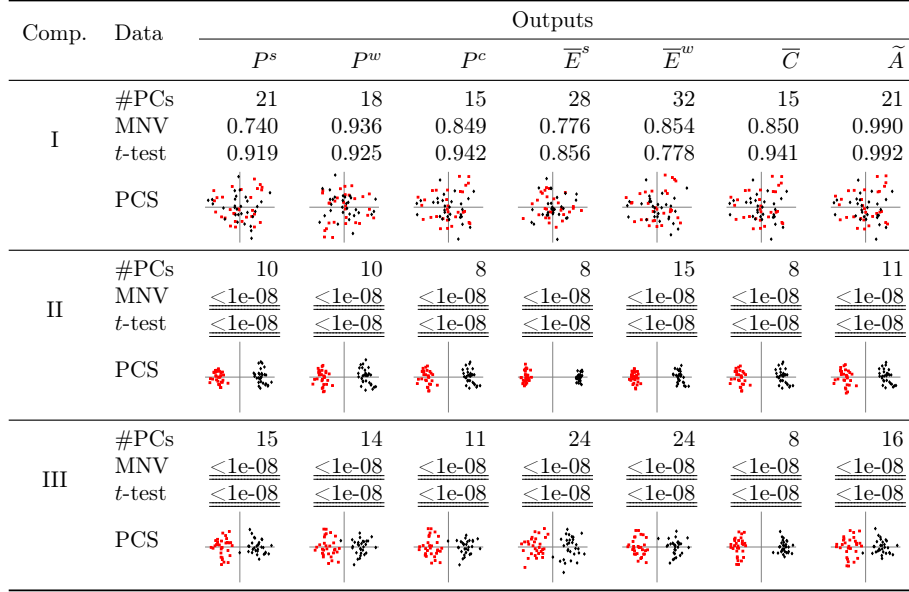 | 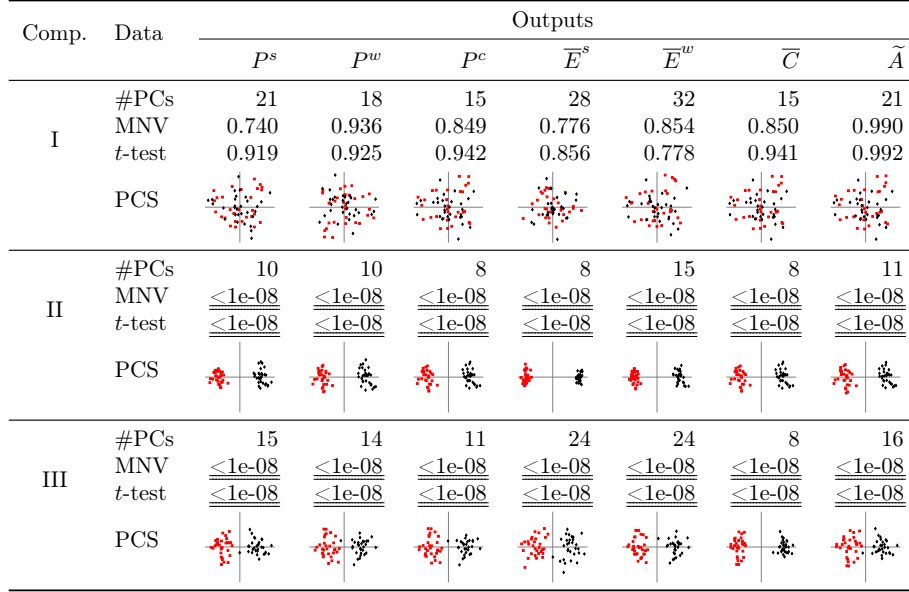 | 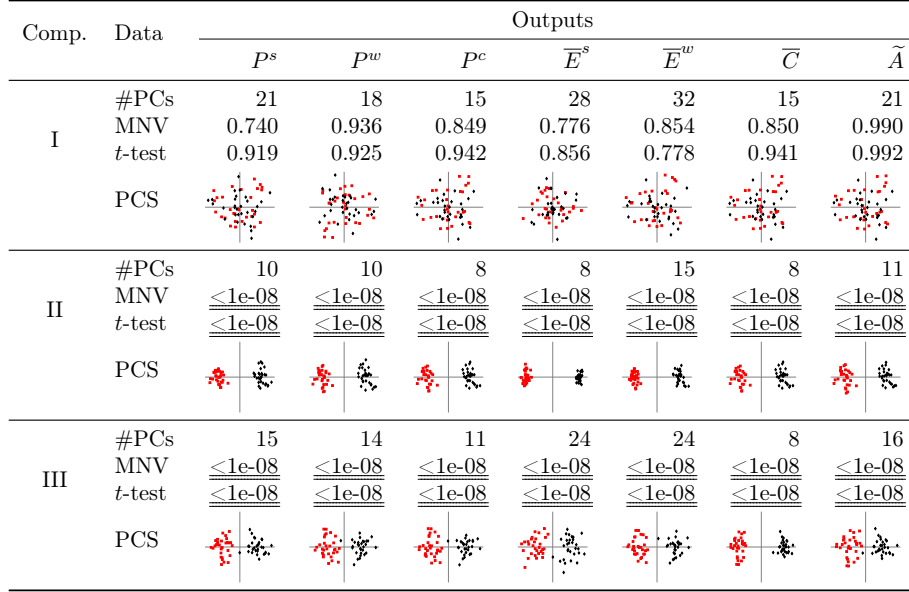 | 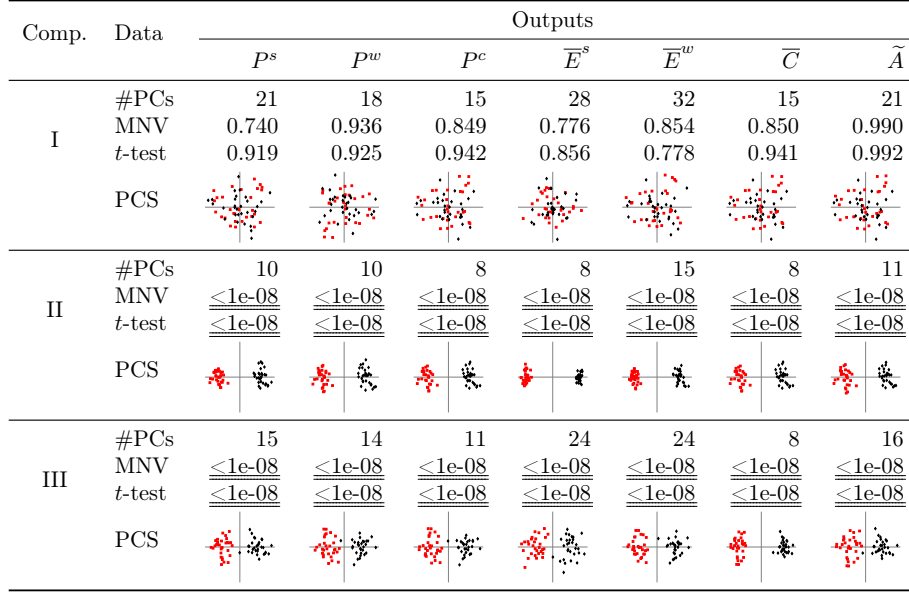 | 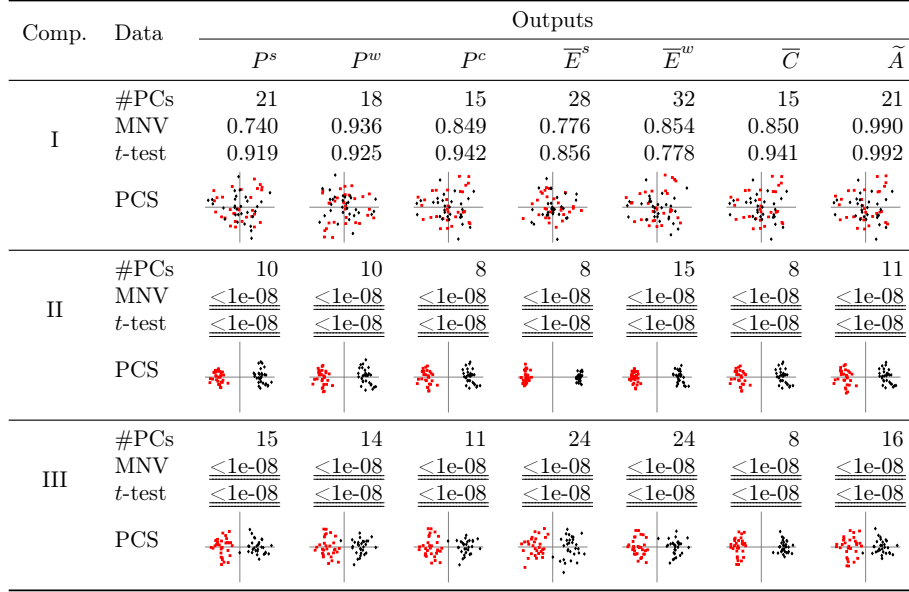 | 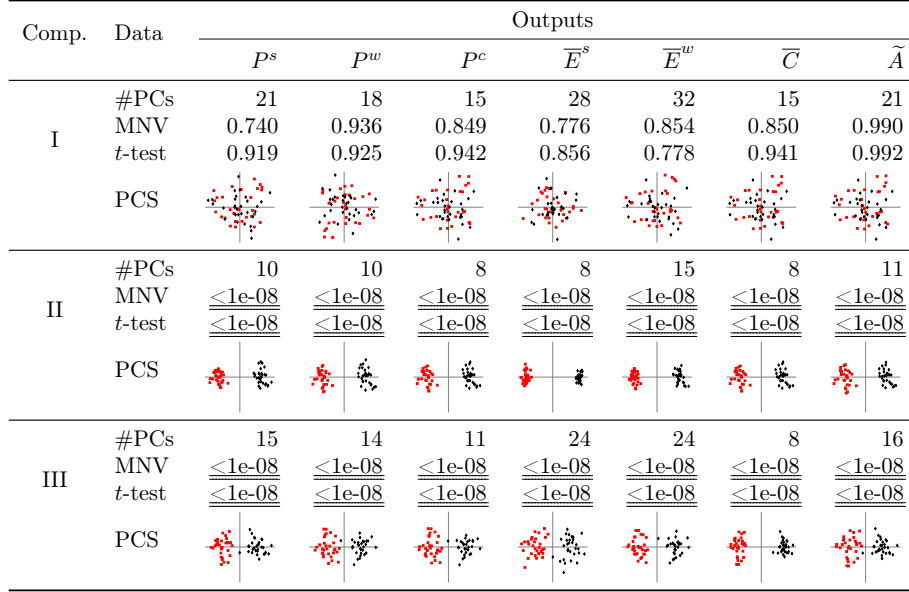 |

**Table S2.6** Model-independent comparison for model size 400, parameter set 2, and  $n = 30$  runs per configuration. Case I weights two similar setups, case II compares setups with a small implementation difference, and case III compares setups with a different parameter. #PCs is the number of PCs which explain at least 90% of variance, while MNV and  $t$ -test refer to the  $p$ -value yielded by the MANOVA (#PCs) and  $t$  (first PC) hypothesis tests, respectively. PCS shows the representation of the respective output in the first two dimensions of the PC space. Output  $\tilde{A}$  refers to the concatenation of all outputs (range scaled). The MANOVA test is not applicable to one PC, and the respective  $p$ -values are replaced with an asterisk (\*).  $P$ -values lower than 0.05 are underlined, while  $p$ -values lower than 0.01 are double-underlined.

| Comp. | Data      | Outputs                                                                             |                                                                                     |                                                                                     |                                                                                     |                                                                                      |                                                                                       |                                                                                       |
|-------|-----------|-------------------------------------------------------------------------------------|-------------------------------------------------------------------------------------|-------------------------------------------------------------------------------------|-------------------------------------------------------------------------------------|--------------------------------------------------------------------------------------|---------------------------------------------------------------------------------------|---------------------------------------------------------------------------------------|
|       |           | $P^s$                                                                               | $P^w$                                                                               | $P^c$                                                                               | $\bar{E}^s$                                                                         | $\bar{E}^w$                                                                          | $\bar{C}$                                                                             | $\tilde{A}$                                                                           |
| I     | #PCs      | 25                                                                                  | 32                                                                                  | 25                                                                                  | 36                                                                                  | 43                                                                                   | 26                                                                                    | 39                                                                                    |
|       | MNV       | 0.521                                                                               | 0.817                                                                               | 0.617                                                                               | <u>0.004</u>                                                                        | 0.338                                                                                | 0.630                                                                                 | 0.276                                                                                 |
|       | $t$ -test | 0.316                                                                               | 0.341                                                                               | 0.307                                                                               | <u>0.502</u>                                                                        | 0.577                                                                                | 0.307                                                                                 | 0.262                                                                                 |
|       | PCS       | 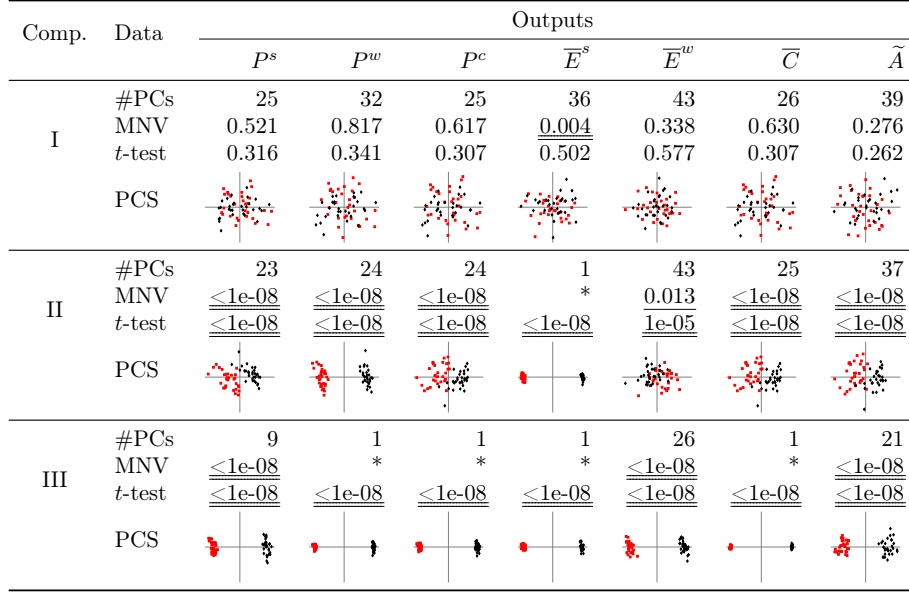   | 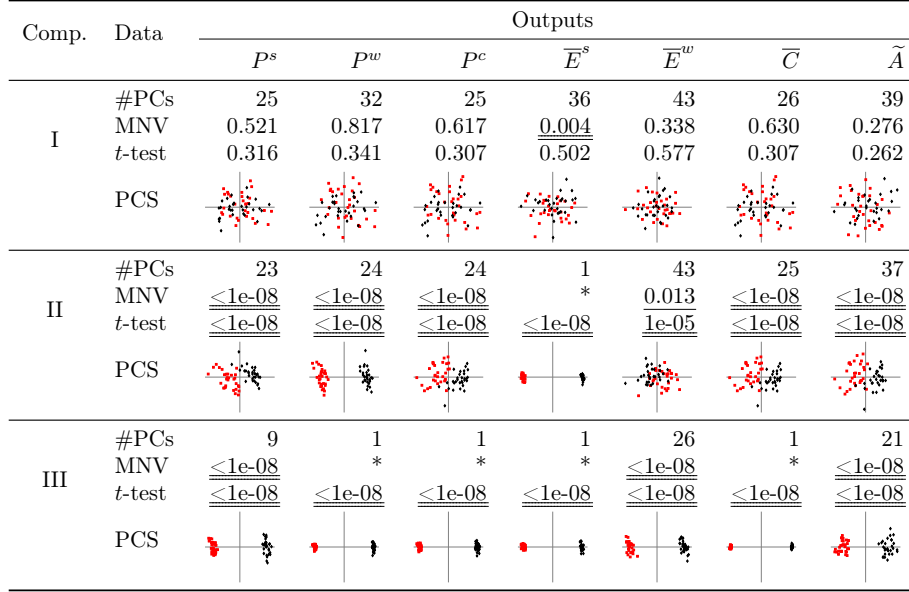   | 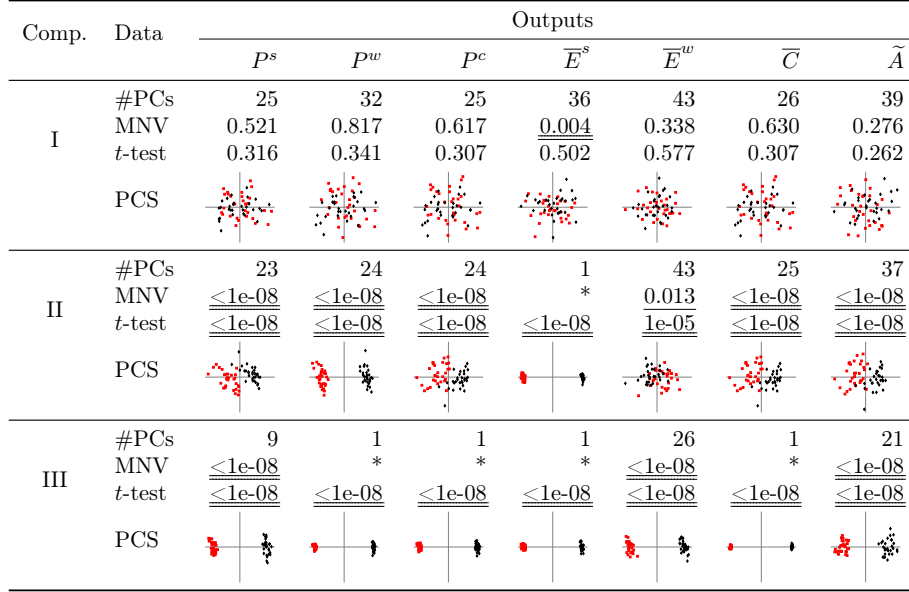   | 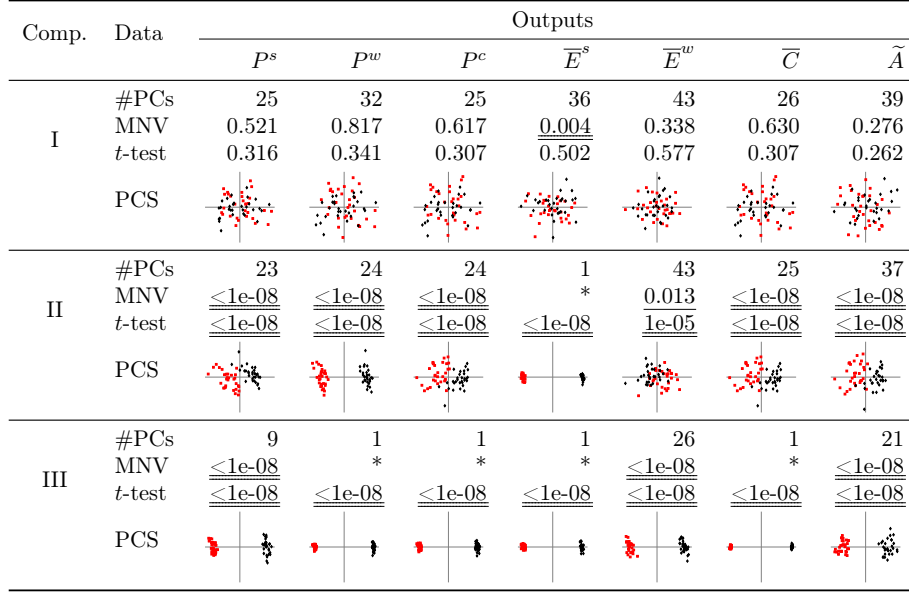   | 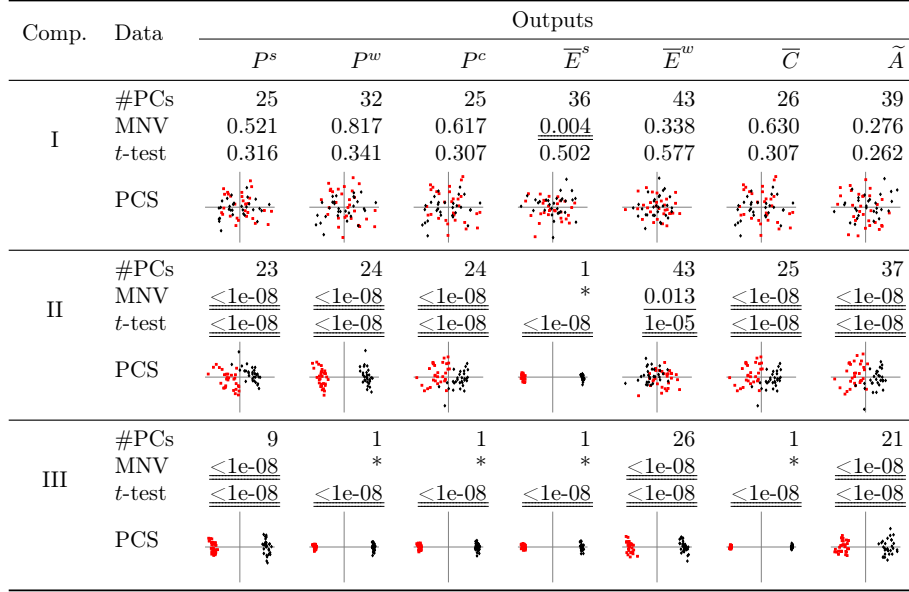   | 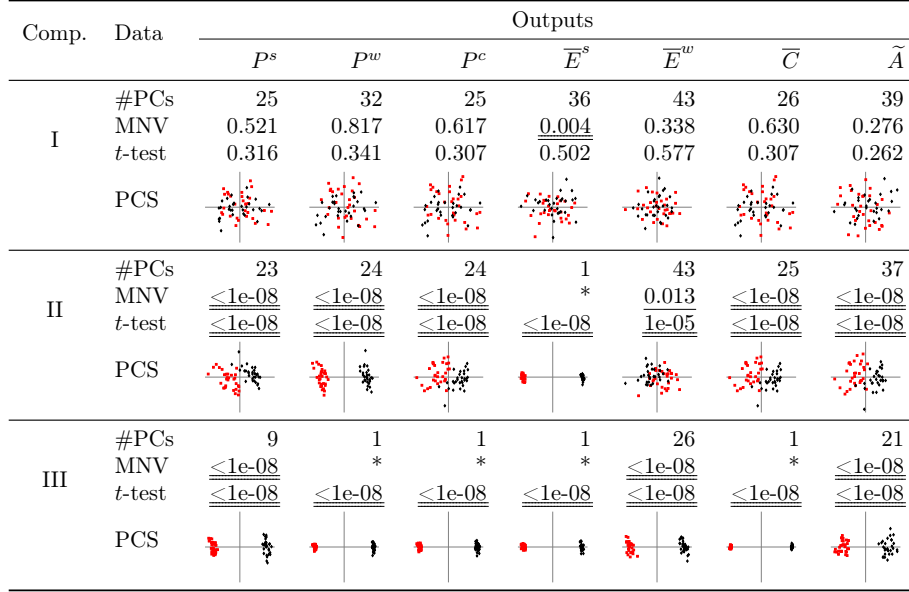   | 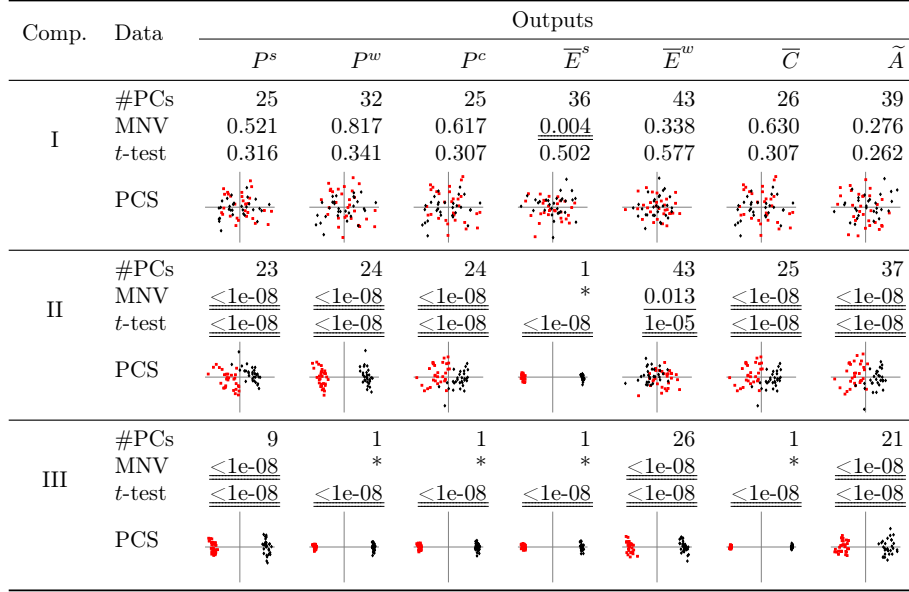   |
| II    | #PCs      | 23                                                                                  | 24                                                                                  | 24                                                                                  | 1                                                                                   | 43                                                                                   | 25                                                                                    | 37                                                                                    |
|       | MNV       | <u>&lt;1e-08</u>                                                                    | <u>&lt;1e-08</u>                                                                    | <u>&lt;1e-08</u>                                                                    | *                                                                                   | 0.013                                                                                | <u>&lt;1e-08</u>                                                                      | <u>&lt;1e-08</u>                                                                      |
|       | $t$ -test | <u>&lt;1e-08</u>                                                                    | <u>&lt;1e-08</u>                                                                    | <u>&lt;1e-08</u>                                                                    | <u>&lt;1e-08</u>                                                                    | <u>1e-05</u>                                                                         | <u>&lt;1e-08</u>                                                                      | <u>&lt;1e-08</u>                                                                      |
|       | PCS       | 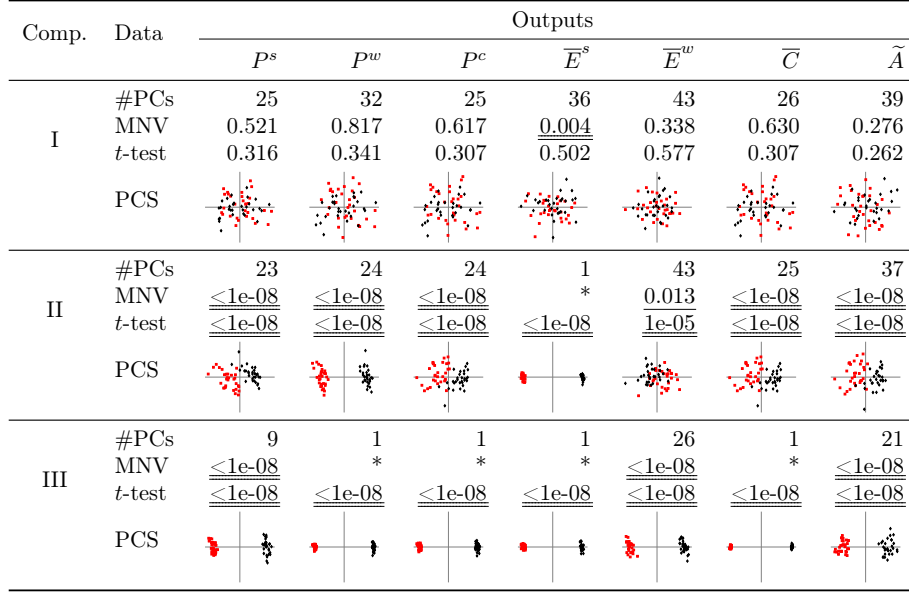   | 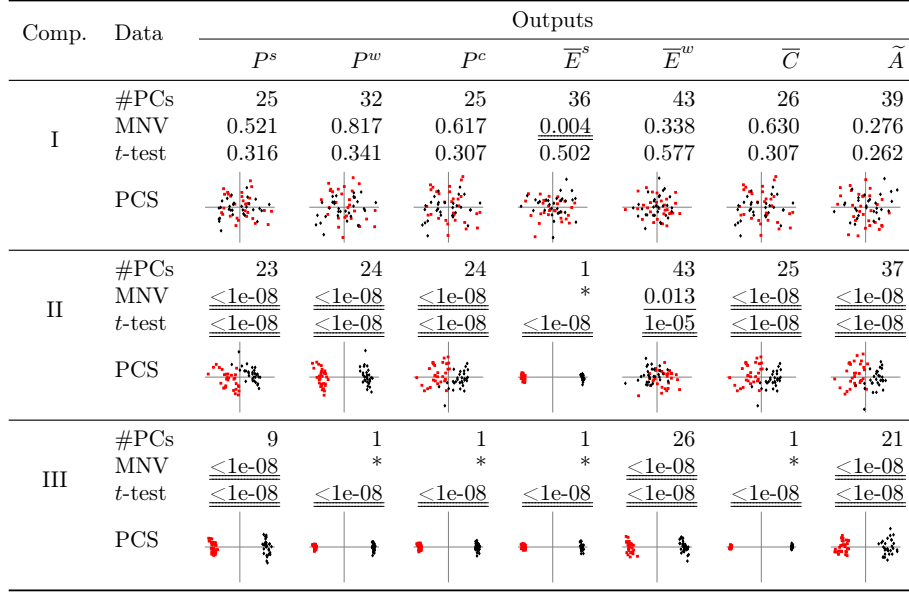   | 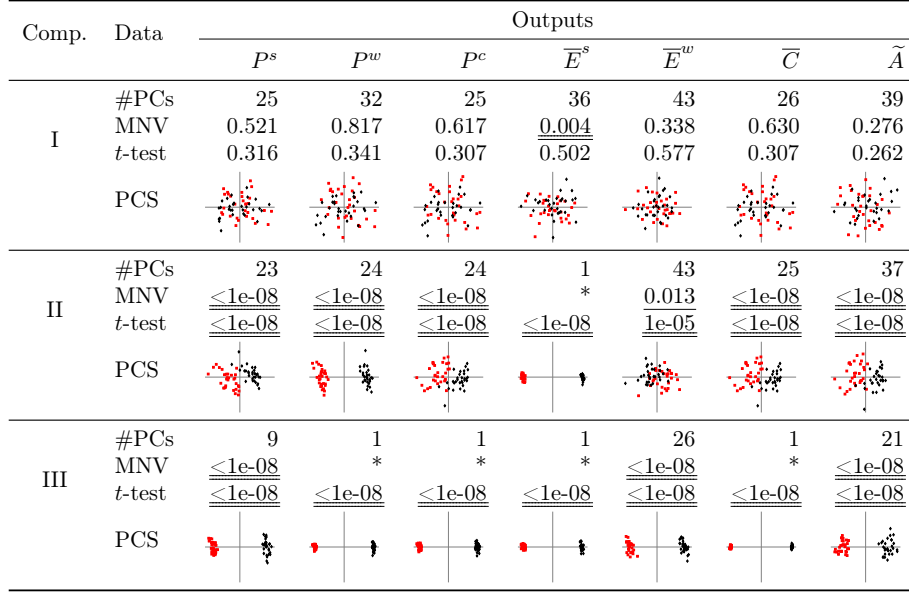   | 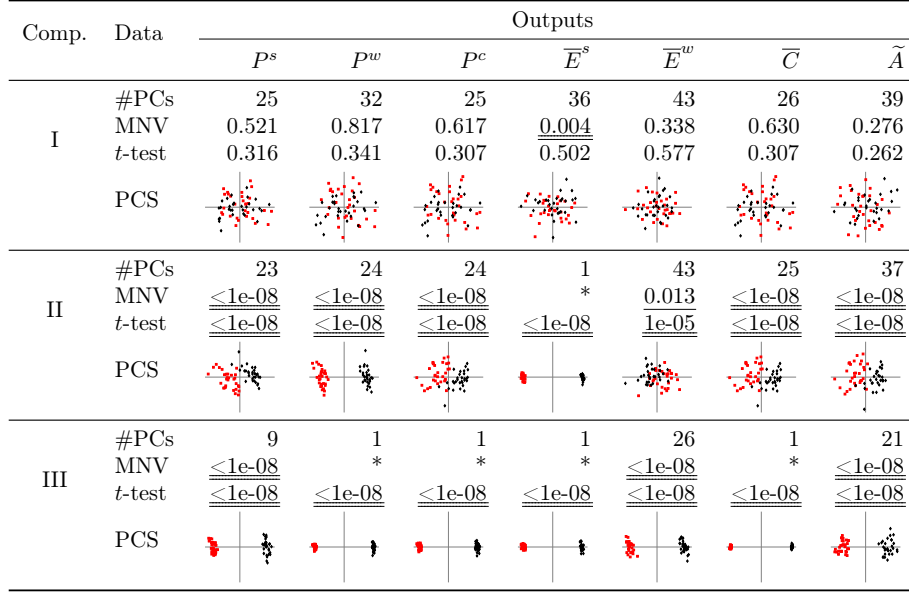   | 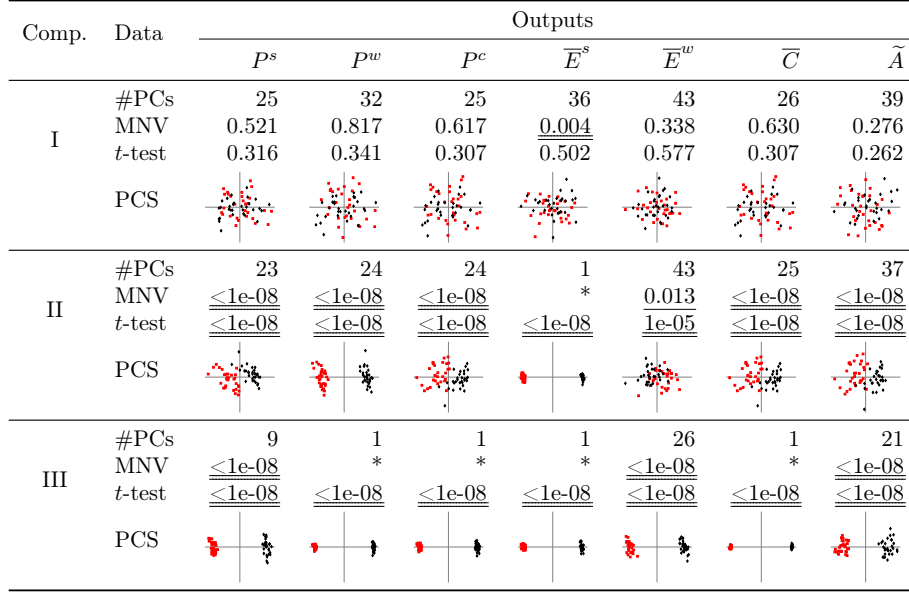   | 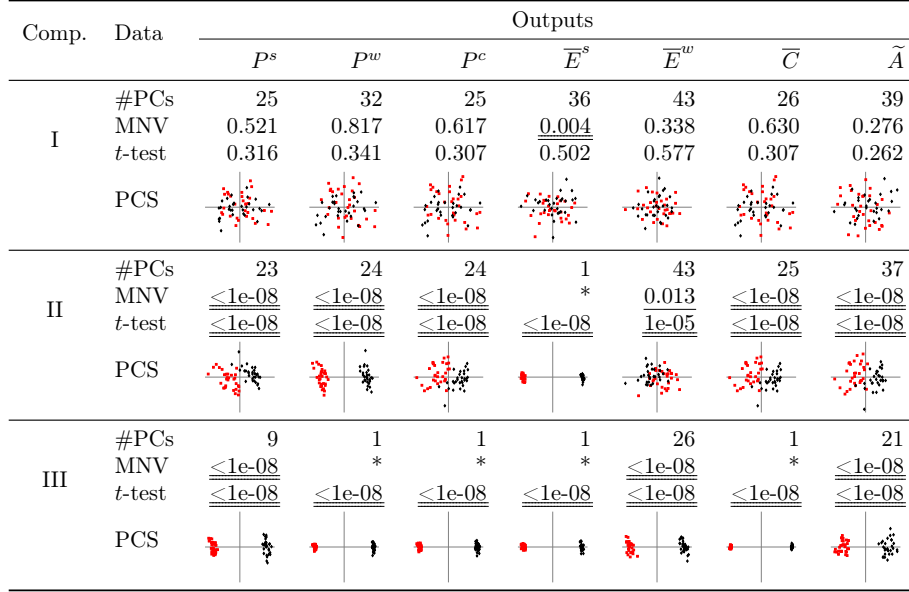   | 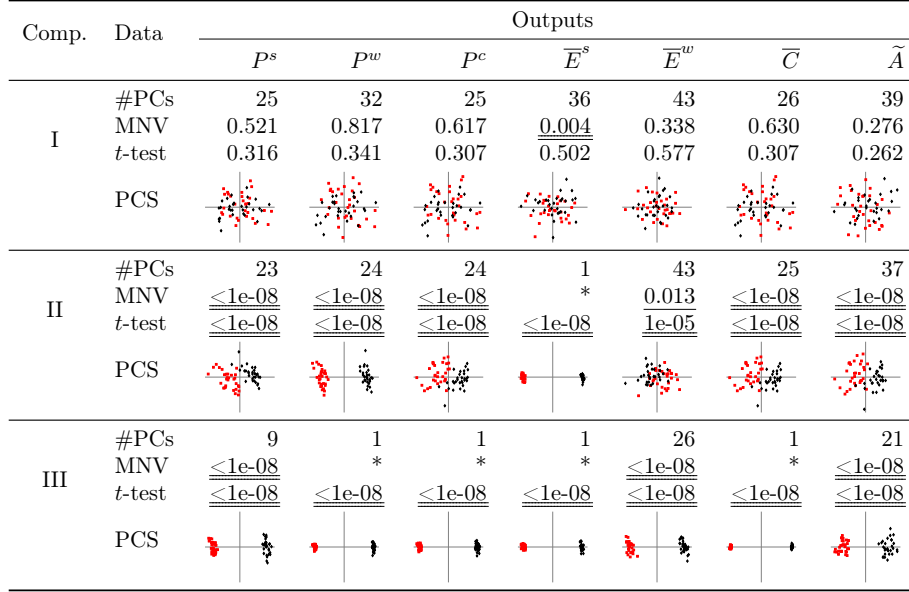   |
| III   | #PCs      | 9                                                                                   | 1                                                                                   | 1                                                                                   | 1                                                                                   | 26                                                                                   | 1                                                                                     | 21                                                                                    |
|       | MNV       | <u>&lt;1e-08</u>                                                                    | *                                                                                   | *                                                                                   | *                                                                                   | <u>&lt;1e-08</u>                                                                     | *                                                                                     | <u>&lt;1e-08</u>                                                                      |
|       | $t$ -test | <u>&lt;1e-08</u>                                                                    | <u>&lt;1e-08</u>                                                                    | <u>&lt;1e-08</u>                                                                    | <u>&lt;1e-08</u>                                                                    | <u>&lt;1e-08</u>                                                                     | <u>&lt;1e-08</u>                                                                      | <u>&lt;1e-08</u>                                                                      |
|       | PCS       | 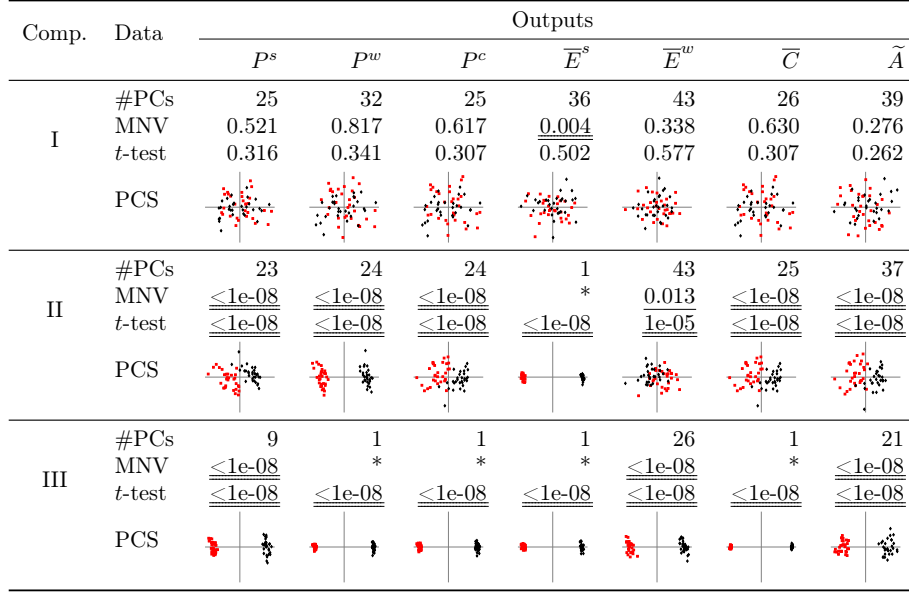 | 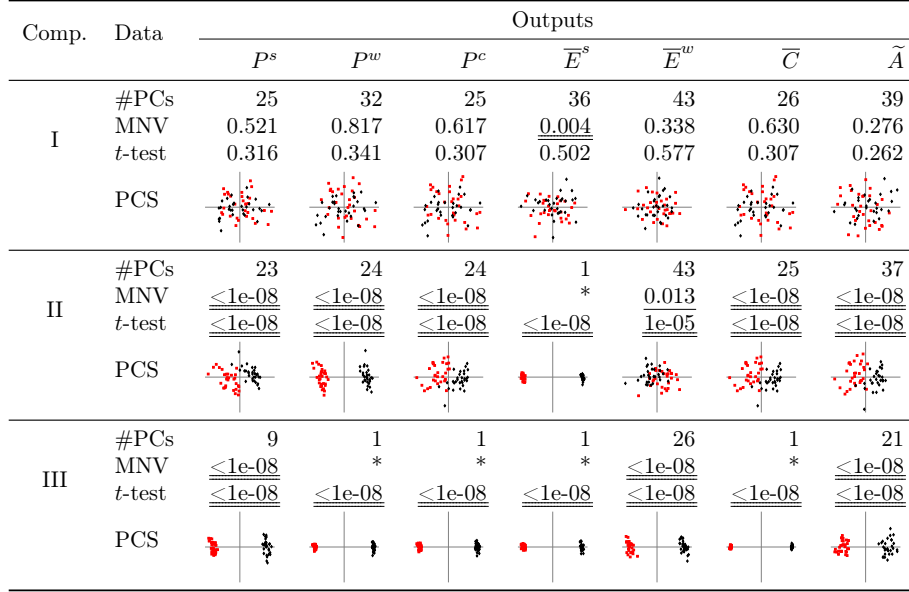 | 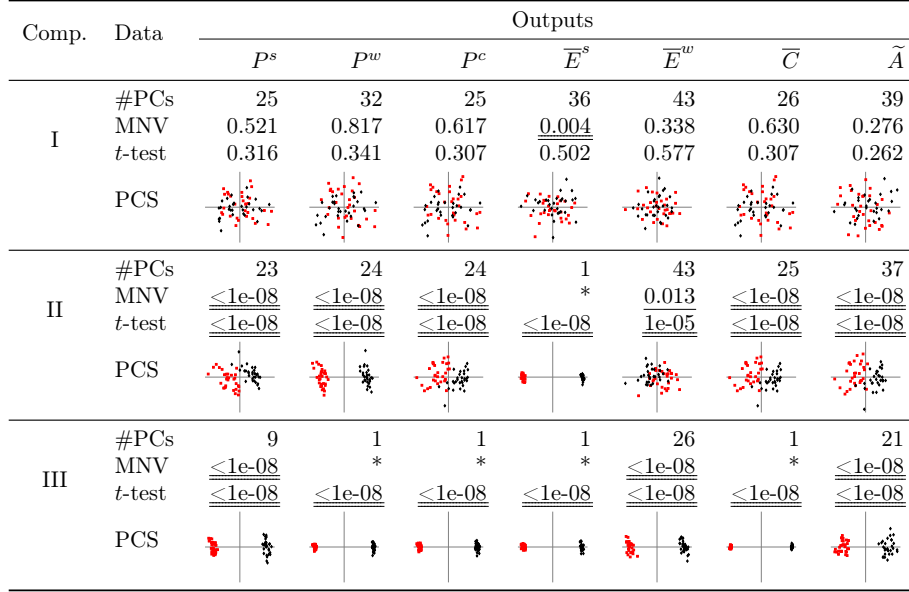 | 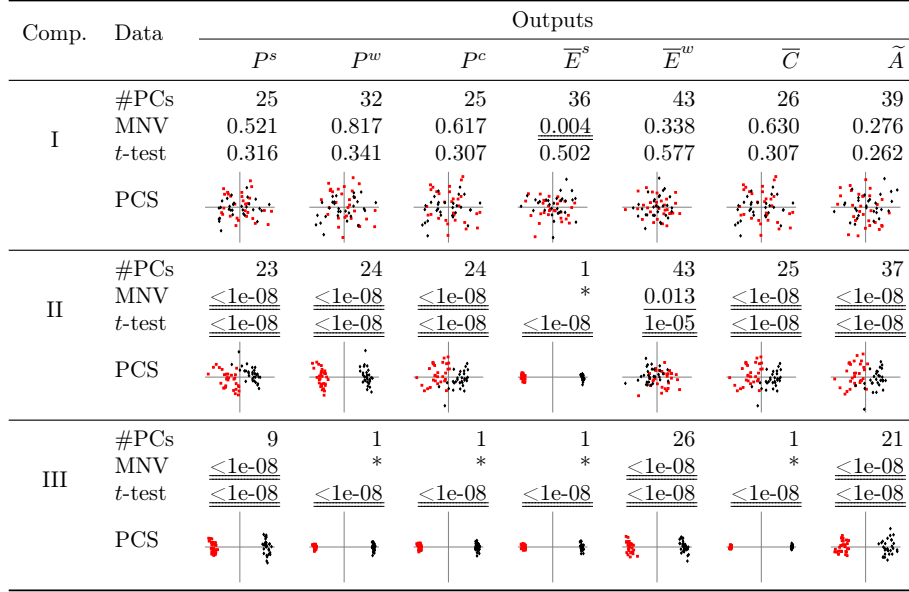 | 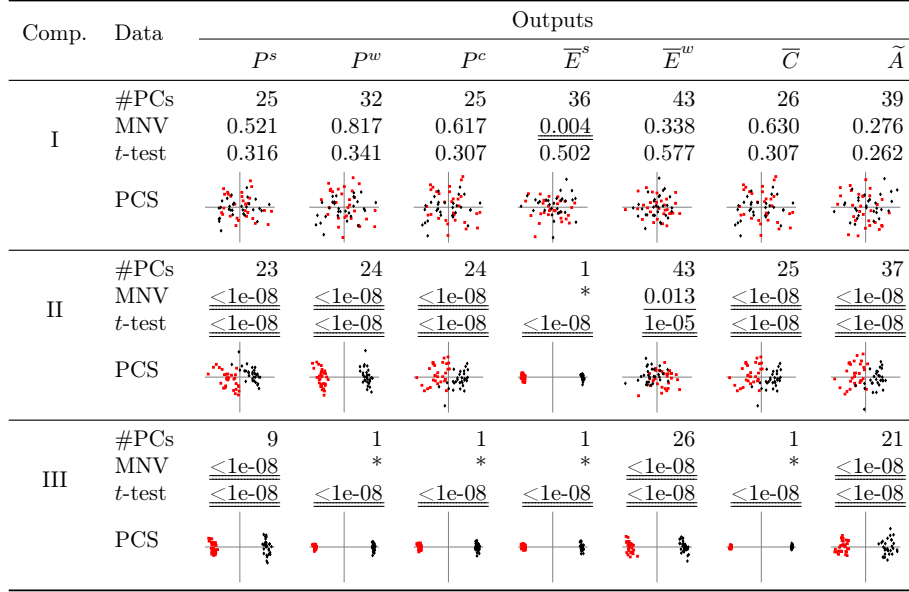 | 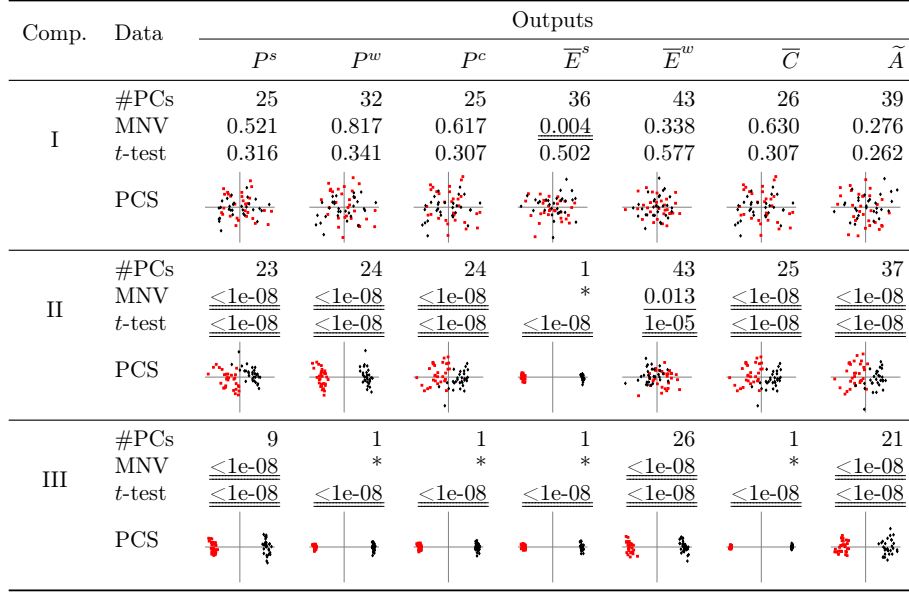 | 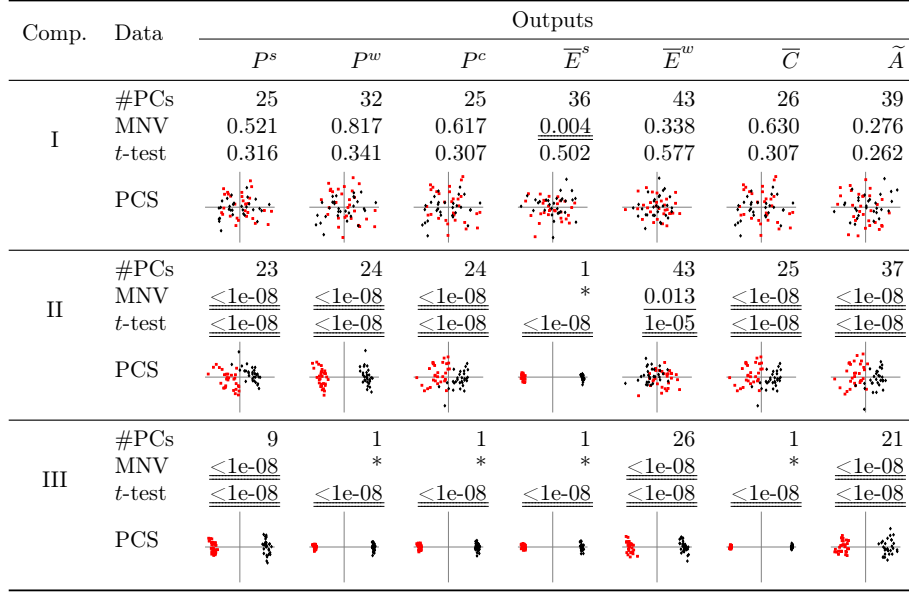 |

**Table S2.7** Model-independent comparison for model size 800, parameter set 1, and  $n = 30$  runs per configuration. Case I weights two similar setups, case II compares setups with a small implementation difference, and case III compares setups with a different parameter. #PCs is the number of PCs which explain at least 90% of variance, while MNV and  $t$ -test refer to the  $p$ -value yielded by the MANOVA (#PCs) and  $t$  (first PC) hypothesis tests, respectively. PCS shows the representation of the respective output in the first two dimensions of the PC space. Output  $\tilde{A}$  refers to the concatenation of all outputs (range scaled). The MANOVA test is not applicable to one PC, and the respective  $p$ -values are replaced with an asterisk (\*).  $P$ -values lower than 0.05 are underlined, while  $p$ -values lower than 0.01 are double-underlined.



| Comp. | Data      | Outputs                                                                             |                                                                                     |                                                                                     |                                                                                     |                                                                                      |                                                                                       |                                                                                       |
|-------|-----------|-------------------------------------------------------------------------------------|-------------------------------------------------------------------------------------|-------------------------------------------------------------------------------------|-------------------------------------------------------------------------------------|--------------------------------------------------------------------------------------|---------------------------------------------------------------------------------------|---------------------------------------------------------------------------------------|
|       |           | $P^s$                                                                               | $P^w$                                                                               | $P^c$                                                                               | $\bar{E}^s$                                                                         | $\bar{E}^w$                                                                          | $\bar{C}$                                                                             | $\tilde{A}$                                                                           |
| I     | #PCs      | 20                                                                                  | 17                                                                                  | 14                                                                                  | 28                                                                                  | 31                                                                                   | 15                                                                                    | 20                                                                                    |
|       | MNV       | 0.242                                                                               | 0.274                                                                               | 0.252                                                                               | <u>0.005</u>                                                                        | 0.379                                                                                | 0.285                                                                                 | 0.322                                                                                 |
|       | $t$ -test | 0.597                                                                               | 0.979                                                                               | 0.819                                                                               | 0.813                                                                               | 0.788                                                                                | 0.819                                                                                 | 0.927                                                                                 |
|       | PCS       | 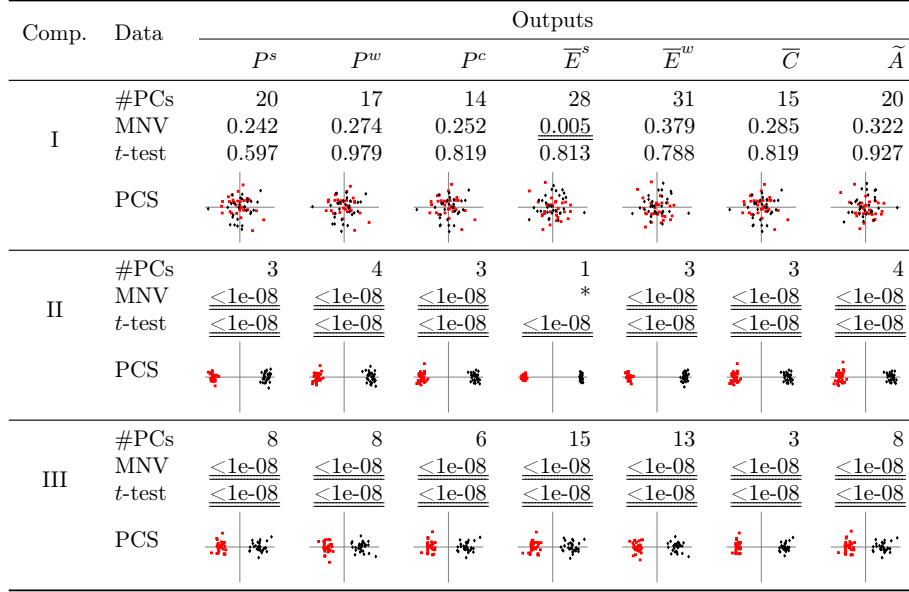   | 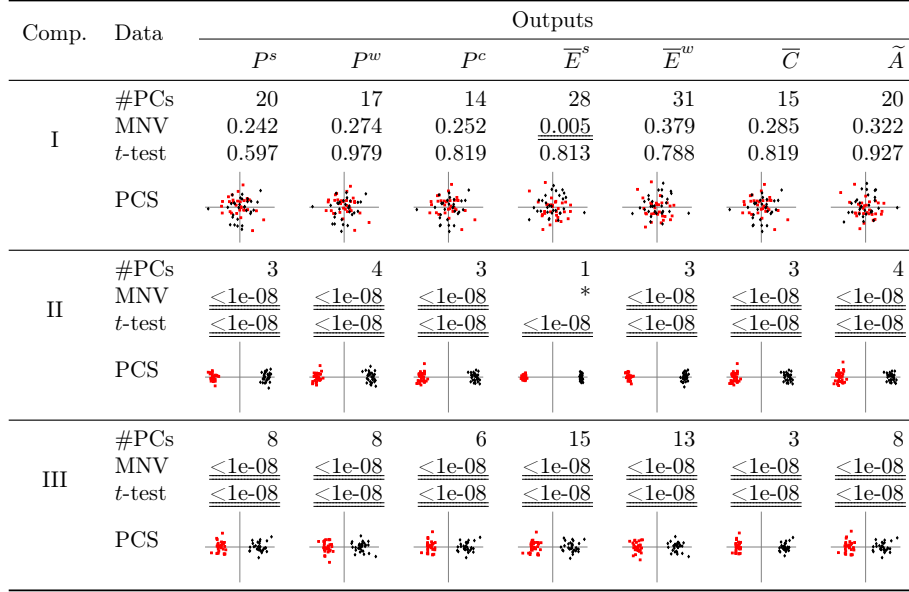   | 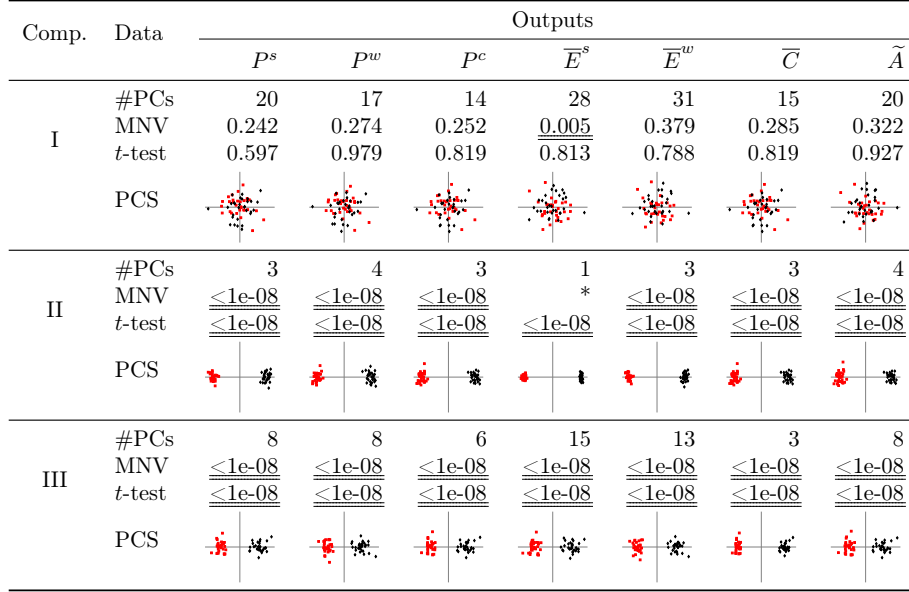   | 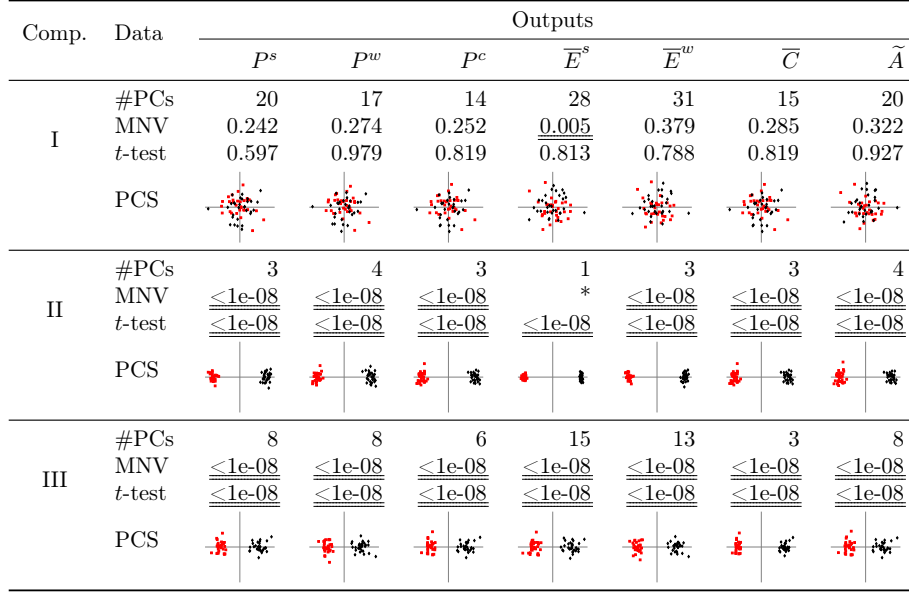   | 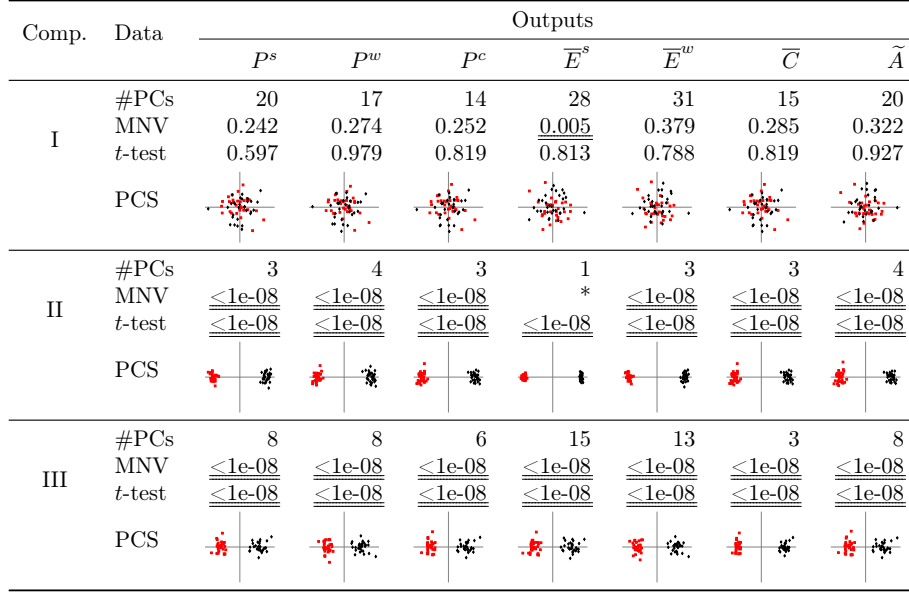   | 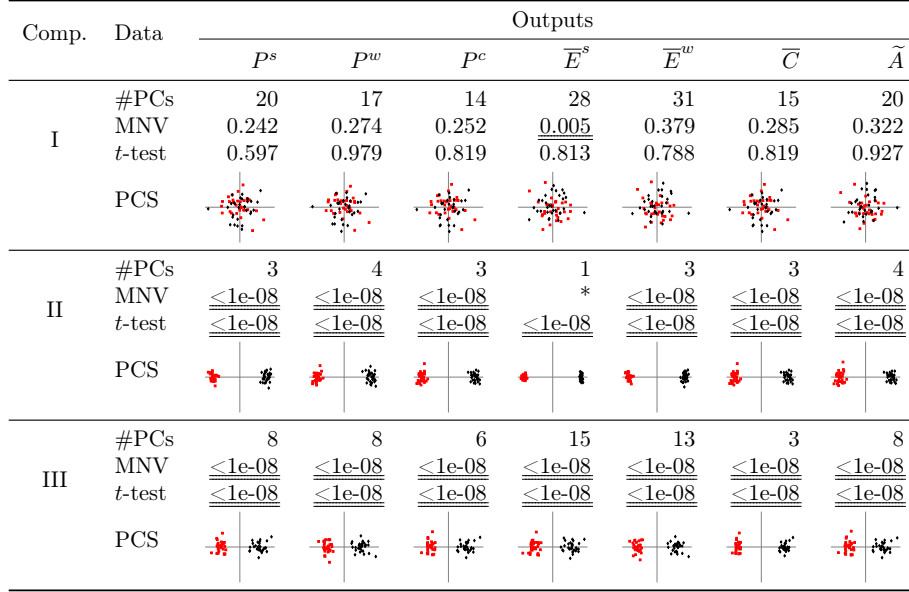   | 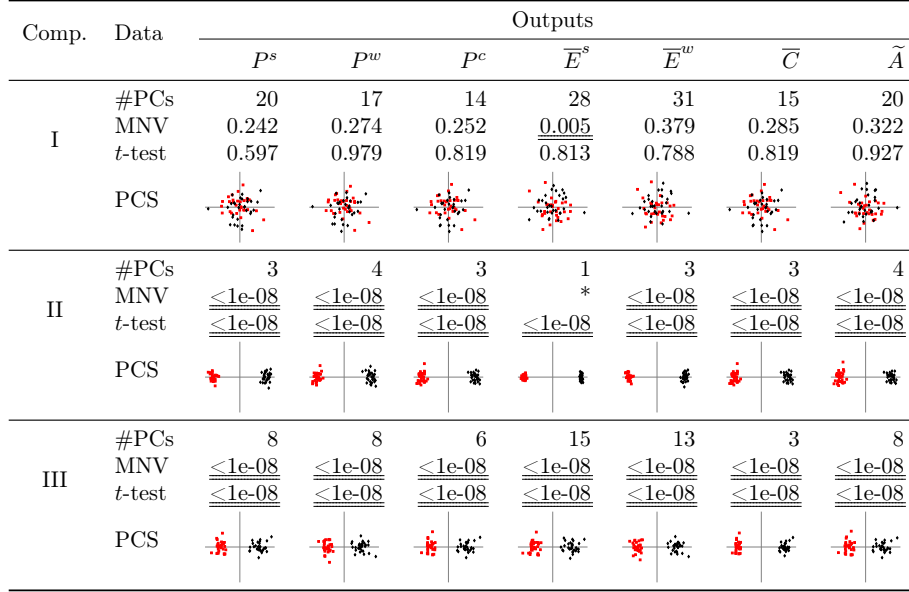   |
| II    | #PCs      | 3                                                                                   | 4                                                                                   | 3                                                                                   | 1                                                                                   | 3                                                                                    | 3                                                                                     | 4                                                                                     |
|       | MNV       | <u>&lt;1e-08</u>                                                                    | <u>&lt;1e-08</u>                                                                    | <u>&lt;1e-08</u>                                                                    | *                                                                                   | <u>&lt;1e-08</u>                                                                     | <u>&lt;1e-08</u>                                                                      | <u>&lt;1e-08</u>                                                                      |
|       | $t$ -test | <u>&lt;1e-08</u>                                                                    | <u>&lt;1e-08</u>                                                                    | <u>&lt;1e-08</u>                                                                    | <u>&lt;1e-08</u>                                                                    | <u>&lt;1e-08</u>                                                                     | <u>&lt;1e-08</u>                                                                      | <u>&lt;1e-08</u>                                                                      |
|       | PCS       | 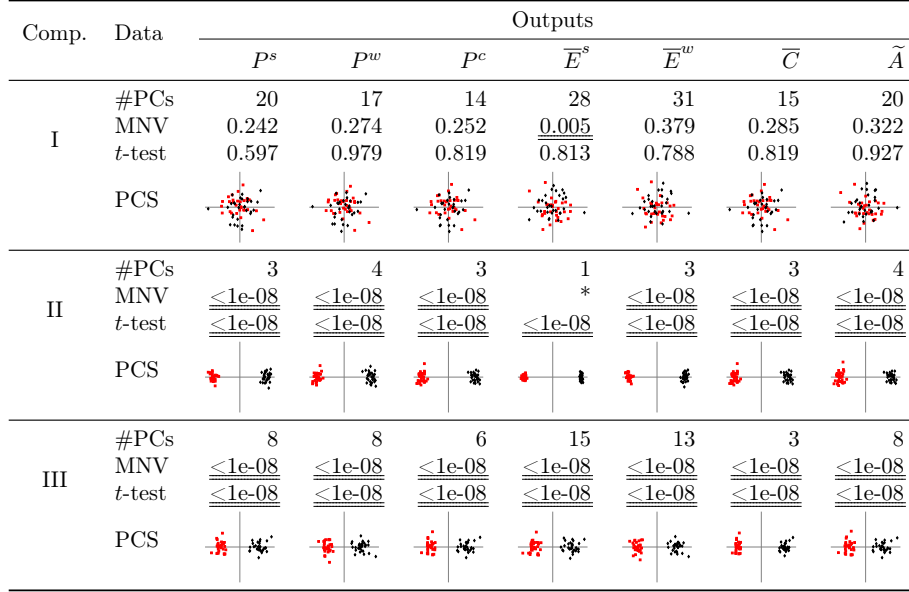   | 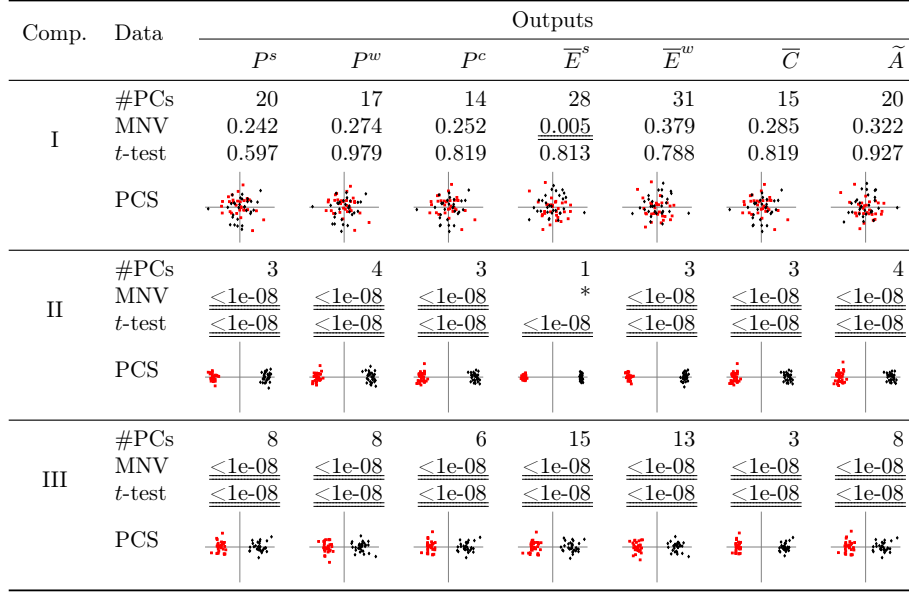   | 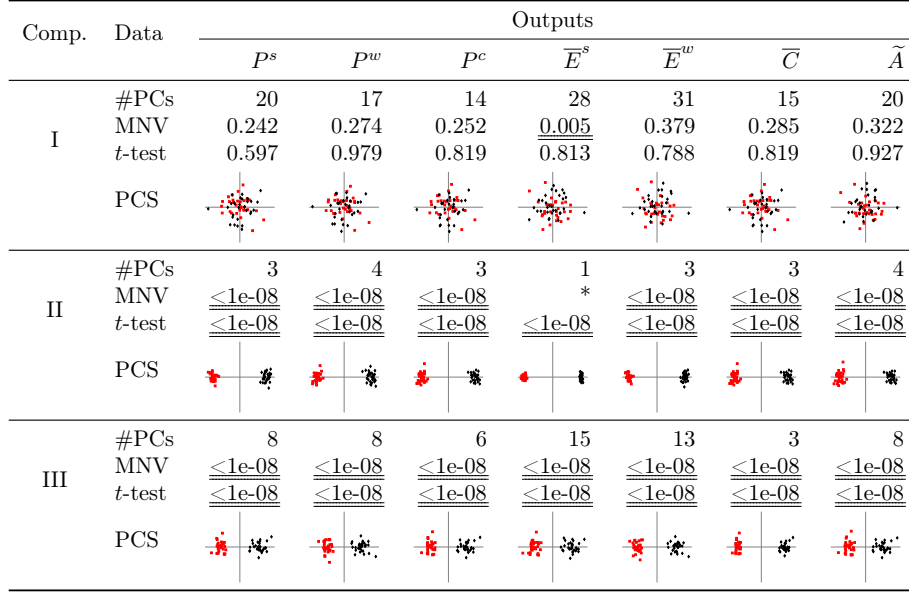   | 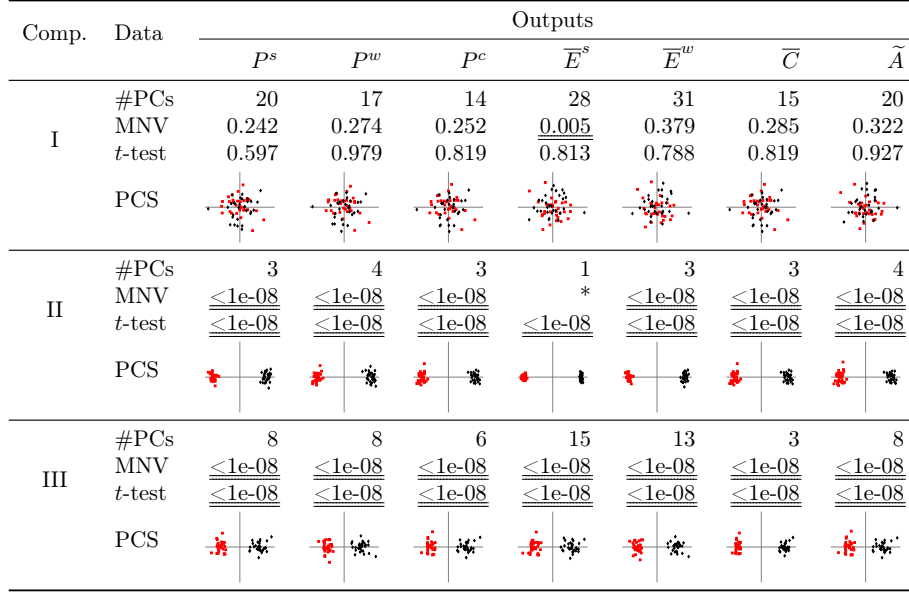   | 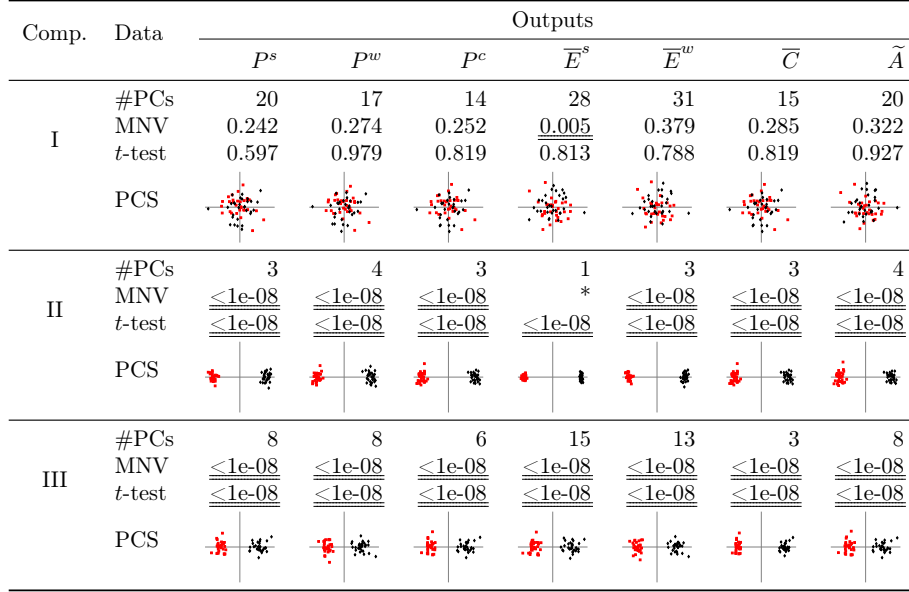   | 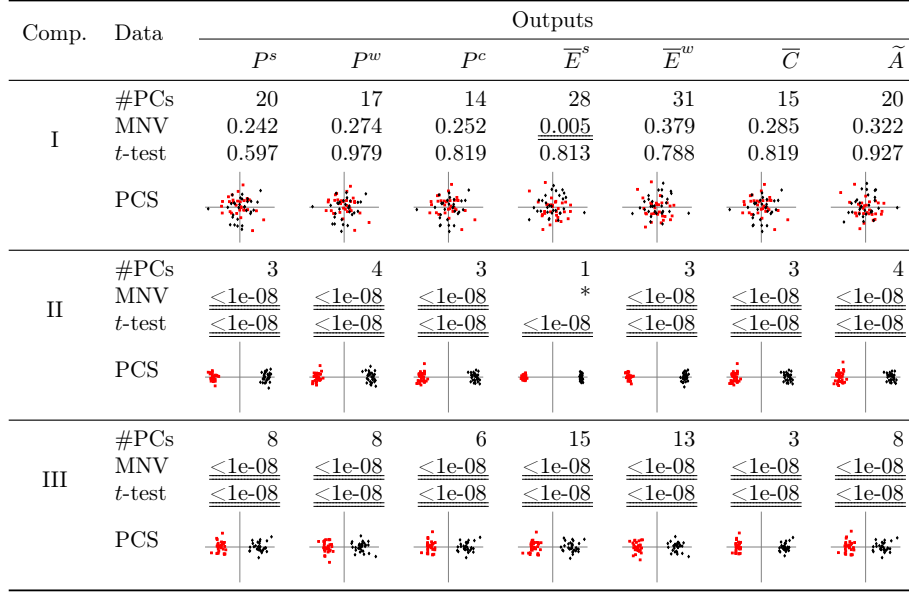   | 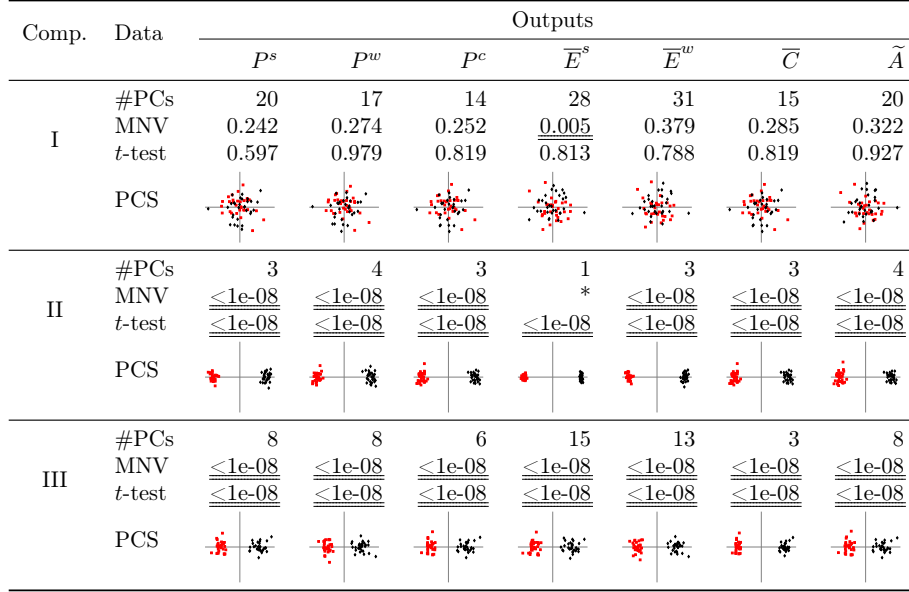   |
| III   | #PCs      | 8                                                                                   | 8                                                                                   | 6                                                                                   | 15                                                                                  | 13                                                                                   | 3                                                                                     | 8                                                                                     |
|       | MNV       | <u>&lt;1e-08</u>                                                                    | <u>&lt;1e-08</u>                                                                    | <u>&lt;1e-08</u>                                                                    | <u>&lt;1e-08</u>                                                                    | <u>&lt;1e-08</u>                                                                     | <u>&lt;1e-08</u>                                                                      | <u>&lt;1e-08</u>                                                                      |
|       | $t$ -test | <u>&lt;1e-08</u>                                                                    | <u>&lt;1e-08</u>                                                                    | <u>&lt;1e-08</u>                                                                    | <u>&lt;1e-08</u>                                                                    | <u>&lt;1e-08</u>                                                                     | <u>&lt;1e-08</u>                                                                      | <u>&lt;1e-08</u>                                                                      |
|       | PCS       | 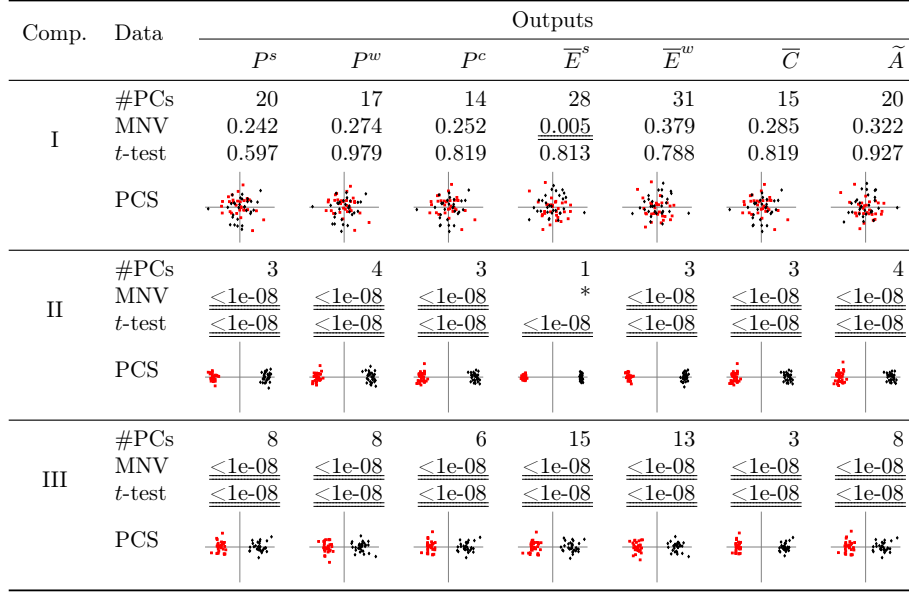 | 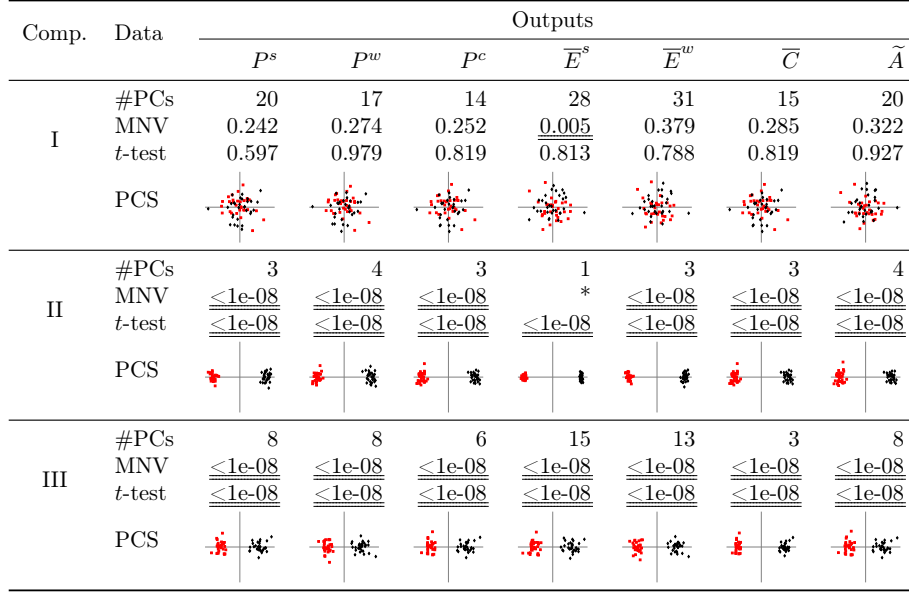 | 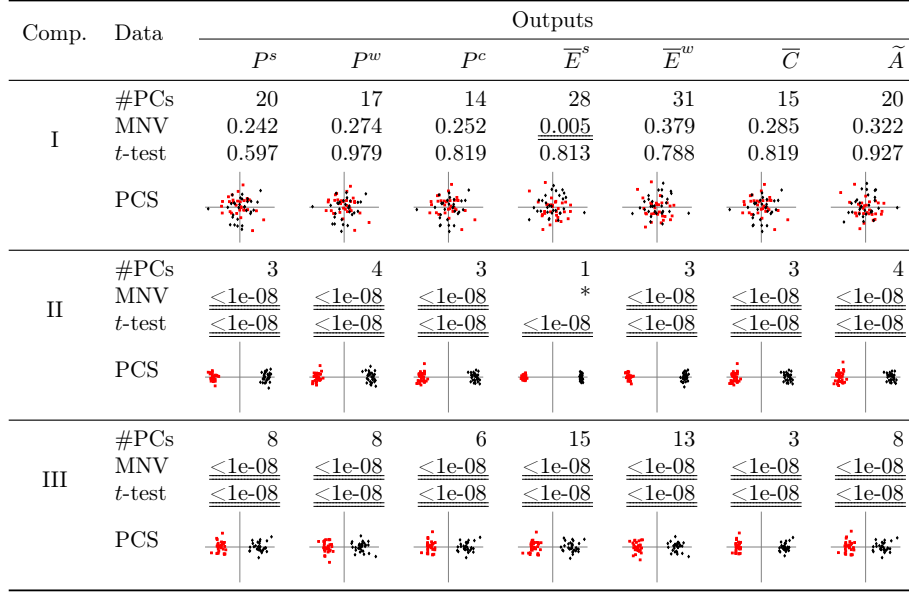 | 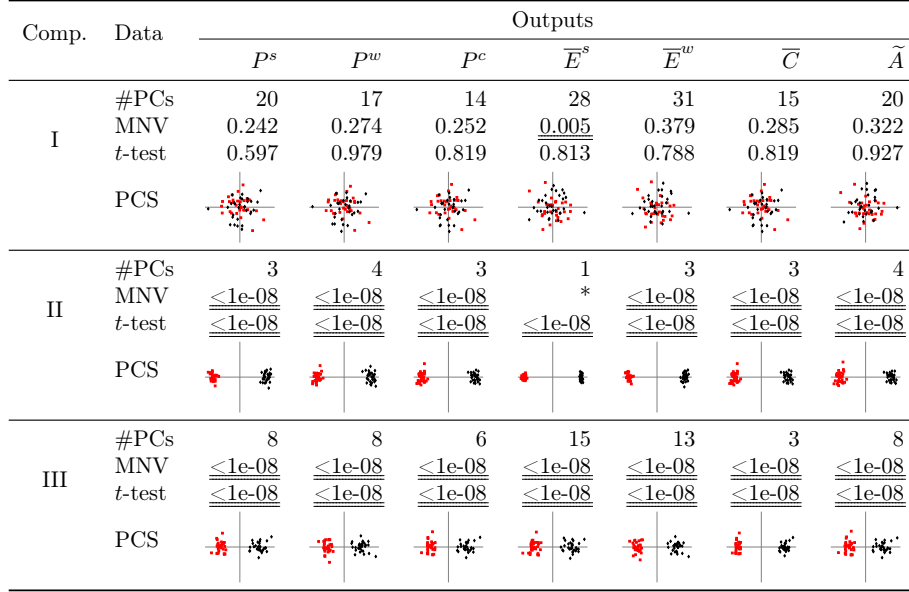 | 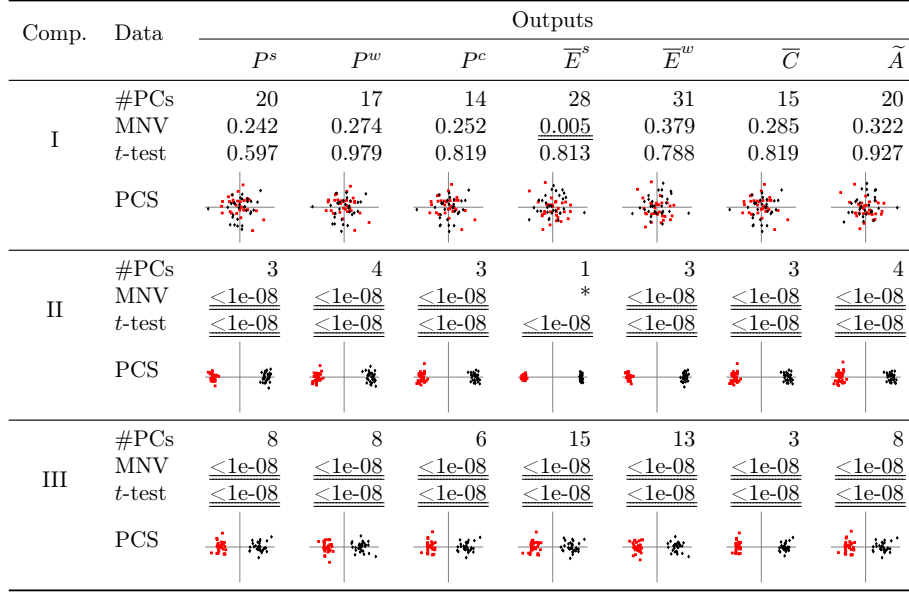 | 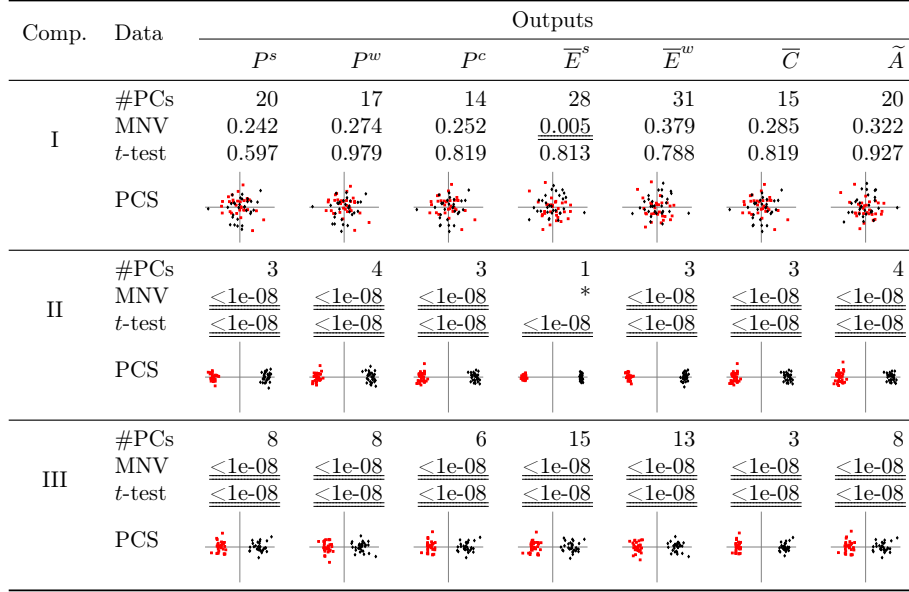 | 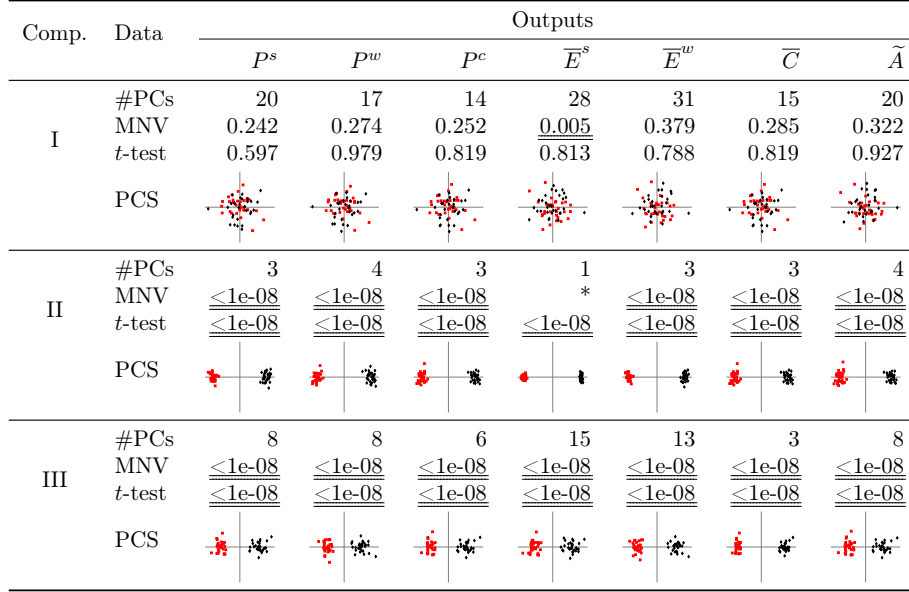 |

**Table S2.8** Model-independent comparison for model size 800, parameter set 2, and  $n = 30$  runs per configuration. Case I weights two similar setups, case II compares setups with a small implementation difference, and case III compares setups with a different parameter. #PCs is the number of PCs which explain at least 90% of variance, while MNV and  $t$ -test refer to the  $p$ -value yielded by the MANOVA (#PCs) and  $t$  (first PC) hypothesis tests, respectively. PCS shows the representation of the respective output in the first two dimensions of the PC space. Output  $\tilde{A}$  refers to the concatenation of all outputs (range scaled). The MANOVA test is not applicable to one PC, and the respective  $p$ -values are replaced with an asterisk (\*).  $P$ -values lower than 0.05 are underlined, while  $p$ -values lower than 0.01 are double-underlined.

| Comp. | Data             | Outputs      |                  |                  |                  |                  |                  |                  |
|-------|------------------|--------------|------------------|------------------|------------------|------------------|------------------|------------------|
|       |                  | $P^s$        | $P^w$            | $P^c$            | $\overline{E}^s$ | $\overline{E}^w$ | $\overline{C}$   | $\widetilde{A}$  |
| I     | % var. (PC1)     | 15.6         | 10.0             | 12.4             | 9.0              | 8.2              | 12.3             | 8.8              |
|       | % var. (PC2)     | 9.1          | 9.2              | 9.7              | 6.6              | 6.5              | 9.6              | 8.0              |
|       | % var. (PC3)     | 7.4          | 7.3              | 7.8              | 5.6              | 4.9              | 7.8              | 6.5              |
|       | % var. (PC4)     | 6.7          | 6.2              | 6.8              | 5.3              | 4.2              | 6.7              | 5.6              |
|       | $t$ -test (PC1)  | <u>0.036</u> | 0.057            | <u>0.049</u>     | <u>0.023</u>     | 0.503            | <u>0.049</u>     | 0.077            |
|       | $t$ -test (PC2)  | <u>0.680</u> | 0.532            | <u>0.495</u>     | <u>0.550</u>     | 0.358            | <u>0.495</u>     | 0.317            |
|       | $t$ -test (PC3)  | 0.997        | 0.762            | 0.853            | 0.941            | 0.445            | 0.849            | 0.863            |
|       | $t$ -test (PC4)  | 0.714        | 0.716            | 0.904            | 0.546            | 0.090            | 0.910            | 0.958            |
|       | $t$ -test* (PC1) | 0.228        | 0.564            | 0.393            | 0.252            | 1.000            | 0.399            | 0.876            |
|       | $t$ -test* (PC2) | 1.000        | 1.000            | 1.000            | 1.000            | 1.000            | 1.000            | 1.000            |
|       | $t$ -test* (PC3) | 1.000        | 1.000            | 1.000            | 1.000            | 1.000            | 1.000            | 1.000            |
|       | $t$ -test* (PC4) | 1.000        | 1.000            | 1.000            | 1.000            | 1.000            | 1.000            | 1.000            |
| II    | % var. (PC1)     | 17.5         | 11.7             | 13.9             | 19.6             | 8.5              | 13.8             | 10.0             |
|       | % var. (PC2)     | 9.2          | 8.9              | 9.8              | 7.4              | 6.0              | 9.7              | 8.1              |
|       | % var. (PC3)     | 7.9          | 7.0              | 8.2              | 5.6              | 4.5              | 8.1              | 6.6              |
|       | % var. (PC4)     | 7.3          | 6.8              | 7.6              | 5.3              | 4.2              | 7.6              | 6.3              |
|       | $t$ -test (PC1)  | <u>0.001</u> | <u>0.001</u>     | <u>0.003</u>     | <u>&lt;1e-08</u> | 0.956            | <u>0.003</u>     | <u>0.003</u>     |
|       | $t$ -test (PC2)  | 0.766        | 0.886            | 0.884            | 0.829            | 0.096            | 0.885            | 0.942            |
|       | $t$ -test (PC3)  | 0.441        | 0.874            | 0.355            | 0.728            | 0.967            | 0.357            | 0.536            |
|       | $t$ -test (PC4)  | 0.515        | 0.250            | 0.287            | 0.887            | 0.160            | 0.285            | 0.220            |
|       | $t$ -test* (PC1) | <u>0.007</u> | <u>0.005</u>     | 0.018            | <u>&lt;1e-08</u> | 1.000            | 0.019            | <u>0.033</u>     |
|       | $t$ -test* (PC2) | 1.000        | 1.000            | 1.000            | 1.000            | 1.000            | 1.000            | 1.000            |
|       | $t$ -test* (PC3) | 1.000        | 1.000            | 1.000            | 1.000            | 1.000            | 1.000            | 1.000            |
|       | $t$ -test* (PC4) | 1.000        | 1.000            | 1.000            | 1.000            | 1.000            | 1.000            | 1.000            |
| III   | % var. (PC1)     | 16.1         | 25.4             | 24.4             | 22.6             | 7.1              | 55.0             | 11.9             |
|       | % var. (PC2)     | 9.8          | 7.8              | 8.9              | 6.4              | 6.0              | 5.1              | 8.7              |
|       | % var. (PC3)     | 8.4          | 6.6              | 7.5              | 6.0              | 5.3              | 4.2              | 7.5              |
|       | % var. (PC4)     | 8.1          | 6.5              | 7.3              | 5.6              | 4.8              | 4.1              | 7.1              |
|       | $t$ -test (PC1)  | <u>6e-08</u> | <u>&lt;1e-08</u> | <u>&lt;1e-08</u> | <u>&lt;1e-08</u> | 0.003            | <u>&lt;1e-08</u> | <u>&lt;1e-08</u> |
|       | $t$ -test (PC2)  | 0.604        | 0.915            | 0.944            | 0.888            | 0.257            | 0.951            | 0.944            |
|       | $t$ -test (PC3)  | 0.951        | 0.851            | 0.921            | 0.820            | <u>1e-06</u>     | 0.972            | 0.983            |
|       | $t$ -test (PC4)  | 0.510        | 0.842            | 0.802            | 0.893            | 0.312            | 0.892            | 0.704            |
|       | $t$ -test* (PC1) | <u>4e-07</u> | <u>&lt;1e-08</u> | <u>&lt;1e-08</u> | <u>&lt;1e-08</u> | 0.041            | <u>&lt;1e-08</u> | <u>&lt;1e-08</u> |
|       | $t$ -test* (PC2) | 1.000        | 1.000            | 1.000            | 1.000            | 1.000            | 1.000            | 1.000            |
|       | $t$ -test* (PC3) | 1.000        | 1.000            | 1.000            | 1.000            | <u>2e-05</u>     | 1.000            | 1.000            |
|       | $t$ -test* (PC4) | 1.000        | 1.000            | 1.000            | 1.000            | 1.000            | 1.000            | 1.000            |

**Table S3.1** Percentage of explained variance (% var.) and  $t$ -test  $p$ -values before ( $t$ -test) and after ( $t$ -test\*) weighted Bonferroni correction of the first four PCs for model size 100, parameter set 1, and  $n = 30$  runs per configuration. Case I weights two similar setups, case II compares setups with a small implementation difference, and case III compares setups with a different parameter.  $P$ -values lower than 0.05 are underlined, while  $p$ -values lower than 0.01 are double-underlined.

| Comp. | Data             | Outputs          |              |              |                  |                  |              |              |
|-------|------------------|------------------|--------------|--------------|------------------|------------------|--------------|--------------|
|       |                  | $P^s$            | $P^w$        | $P^c$        | $\bar{E}^s$      | $\bar{E}^w$      | $\bar{C}$    | $\tilde{A}$  |
| I     | % var. (PC1)     | 17.5             | 21.1         | 21.9         | 13.3             | 14.6             | 21.9         | 19.6         |
|       | % var. (PC2)     | 14.7             | 14.5         | 15.4         | 11.1             | 11.7             | 15.4         | 14.0         |
|       | % var. (PC3)     | 11.6             | 11.9         | 12.7         | 8.8              | 9.1              | 12.7         | 11.5         |
|       | % var. (PC4)     | 7.8              | 9.1          | 9.5          | 7.6              | 6.7              | 9.5          | 8.8          |
|       | $t$ -test (PC1)  | 0.108            | 0.128        | 0.106        | 0.111            | 0.067            | 0.106        | 0.099        |
|       | $t$ -test (PC2)  | 0.579            | 0.039        | 0.073        | 0.419            | 0.354            | 0.072        | 0.110        |
|       | $t$ -test (PC3)  | 0.018            | 0.288        | 0.148        | 0.054            | 0.048            | 0.150        | 0.157        |
|       | $t$ -test (PC4)  | 0.609            | 0.418        | 0.448        | 0.513            | 0.725            | 0.449        | 0.407        |
|       | $t$ -test* (PC1) | 0.616            | 0.608        | 0.484        | 0.837            | 0.461            | 0.486        | 0.505        |
|       | $t$ -test* (PC2) | 1.000            | 0.268        | 0.471        | 1.000            | 1.000            | 0.466        | 0.781        |
|       | $t$ -test* (PC3) | 0.158            | 1.000        | 1.000        | 0.611            | 0.529            | 1.000        | 1.000        |
|       | $t$ -test* (PC4) | 1.000            | 1.000        | 1.000        | 1.000            | 1.000            | 1.000        | 1.000        |
|       | % var. (PC1)     | 18.5             | 19.4         | 20.4         | 20.4             | 15.9             | 20.4         | 18.0         |
|       | % var. (PC2)     | 10.2             | 11.0         | 12.0         | 8.6              | 10.2             | 12.0         | 11.4         |
|       | % var. (PC3)     | 9.6              | 10.5         | 10.8         | 7.6              | 8.0              | 10.8         | 10.2         |
|       | % var. (PC4)     | 8.4              | 9.0          | 9.2          | 6.9              | 6.8              | 9.2          | 8.4          |
| II    | $t$ -test (PC1)  | <u>&lt;1e-08</u> | <u>1e-06</u> | <u>3e-08</u> | <u>&lt;1e-08</u> | <u>&lt;1e-08</u> | <u>3e-08</u> | <u>2e-07</u> |
|       | $t$ -test (PC2)  | <u>0.010</u>     | 0.786        | 0.087        | 0.588            | 0.245            | 0.087        | 0.181        |
|       | $t$ -test (PC3)  | 0.597            | <u>0.004</u> | 0.190        | 0.095            | 0.669            | 0.190        | 0.402        |
|       | $t$ -test (PC4)  | 0.299            | 0.089        | 0.060        | 0.667            | <u>0.034</u>     | 0.061        | <u>0.045</u> |
|       | $t$ -test* (PC1) | <u>2e-08</u>     | <u>5e-06</u> | <u>2e-07</u> | <u>&lt;1e-08</u> | <u>&lt;1e-08</u> | <u>2e-07</u> | <u>9e-07</u> |
|       | $t$ -test* (PC2) | 0.096            | 1.000        | 0.723        | 1.000            | 1.000            | 0.730        | 1.000        |
|       | $t$ -test* (PC3) | 1.000            | <u>0.034</u> | 1.000        | 1.000            | 1.000            | 1.000        | 1.000        |
|       | $t$ -test* (PC4) | 1.000            | 0.990        | 0.656        | 1.000            | 0.500            | 0.661        | 0.538        |
|       | % var. (PC1)     | 17.6             | 18.6         | 19.9         | 13.2             | 13.9             | 19.1         | 18.0         |
|       | % var. (PC2)     | 13.3             | 15.5         | 16.1         | 11.3             | 10.4             | 15.7         | 14.7         |
|       | % var. (PC3)     | 10.6             | 10.7         | 11.7         | 8.9              | 8.5              | 11.9         | 10.5         |
|       | % var. (PC4)     | 7.6              | 8.6          | 9.0          | 7.5              | 6.7              | 8.7          | 8.2          |
| III   | $t$ -test (PC1)  | 0.037            | 0.472        | 0.322        | 0.324            | 0.054            | 0.116        | 0.346        |
|       | $t$ -test (PC2)  | <u>0.028</u>     | 0.067        | <u>0.038</u> | <u>0.046</u>     | 0.052            | <u>0.001</u> | <u>0.041</u> |
|       | $t$ -test (PC3)  | 0.113            | <u>0.028</u> | <u>0.020</u> | 0.141            | 0.116            | <u>0.002</u> | <u>0.027</u> |
|       | $t$ -test (PC4)  | 0.316            | 0.452        | 0.327        | <u>0.022</u>     | 0.894            | 0.105        | 0.283        |
|       | $t$ -test* (PC1) | 0.211            | 1.000        | 1.000        | 1.000            | 0.385            | 0.608        | 1.000        |
|       | $t$ -test* (PC2) | 0.209            | 0.434        | 0.234        | 0.411            | 0.495            | <u>0.006</u> | 0.279        |
|       | $t$ -test* (PC3) | 1.000            | 0.257        | 0.171        | 1.000            | 1.000            | <u>0.013</u> | 0.254        |
|       | $t$ -test* (PC4) | 1.000            | 1.000        | 1.000        | 0.290            | 1.000            | 1.000        | 1.000        |

**Table S3.2** Percentage of explained variance (% var.) and  $t$ -test  $p$ -values before ( $t$ -test) and after ( $t$ -test\*) weighted Bonferroni correction of the first four PCs for model size 100, parameter set 2, and  $n = 30$  runs per configuration. Case I weights two similar setups, case II compares setups with a small implementation difference, and case III compares setups with a different parameter.  $P$ -values lower than 0.05 are underlined, while  $p$ -values lower than 0.01 are double-underlined.

| Comp. | Data             | Outputs                        |                                |                                |                                |                                |                                |                                |
|-------|------------------|--------------------------------|--------------------------------|--------------------------------|--------------------------------|--------------------------------|--------------------------------|--------------------------------|
|       |                  | $P^s$                          | $P^w$                          | $P^c$                          | $\bar{E}^s$                    | $\bar{E}^w$                    | $\bar{C}$                      | $\tilde{A}$                    |
| I     | % var. (PC1)     | 18.2                           | 12.1                           | 14.5                           | 11.7                           | 6.7                            | 14.3                           | 10.3                           |
|       | % var. (PC2)     | 8.5                            | 8.3                            | 9.0                            | 6.6                            | 5.5                            | 9.0                            | 7.3                            |
|       | % var. (PC3)     | 7.3                            | 7.4                            | 8.0                            | 5.5                            | 4.7                            | 7.9                            | 6.5                            |
|       | % var. (PC4)     | 6.6                            | 6.7                            | 6.9                            | 5.4                            | 4.4                            | 6.9                            | 5.9                            |
|       | $t$ -test (PC1)  | 0.783                          | 0.810                          | 0.895                          | 0.973                          | 0.830                          | 0.895                          | 0.979                          |
|       | $t$ -test (PC2)  | 0.505                          | 0.391                          | 0.460                          | 0.304                          | 0.151                          | 0.459                          | 0.332                          |
|       | $t$ -test (PC3)  | 0.141                          | 0.198                          | 0.150                          | 0.856                          | 0.400                          | 0.150                          | 0.248                          |
|       | $t$ -test (PC4)  | 0.546                          | 0.553                          | 0.541                          | 0.427                          | 0.234                          | 0.536                          | 0.409                          |
|       | $t$ -test* (PC1) | 1.000                          | 1.000                          | 1.000                          | 1.000                          | 1.000                          | 1.000                          | 1.000                          |
|       | $t$ -test* (PC2) | 1.000                          | 1.000                          | 1.000                          | 1.000                          | 1.000                          | 1.000                          | 1.000                          |
|       | $t$ -test* (PC3) | 1.000                          | 1.000                          | 1.000                          | 1.000                          | 1.000                          | 1.000                          | 1.000                          |
|       | $t$ -test* (PC4) | 1.000                          | 1.000                          | 1.000                          | 1.000                          | 1.000                          | 1.000                          | 1.000                          |
| II    | % var. (PC1)     | 18.5                           | 11.8                           | 14.7                           | 47.3                           | 8.7                            | 14.5                           | 10.1                           |
|       | % var. (PC2)     | 9.3                            | 9.4                            | 10.0                           | 6.2                            | 5.9                            | 9.9                            | 8.3                            |
|       | % var. (PC3)     | 8.3                            | 7.2                            | 8.9                            | 3.7                            | 4.6                            | 8.8                            | 6.9                            |
|       | % var. (PC4)     | 6.3                            | 6.4                            | 6.7                            | 3.2                            | 4.1                            | 6.6                            | 5.6                            |
|       | $t$ -test (PC1)  | 0.616                          | 0.056                          | 0.481                          | <u><math>\leq 1e-08</math></u> | 0.773                          | 0.480                          | 0.534                          |
|       | $t$ -test (PC2)  | 0.440                          | 0.077                          | 0.489                          | 0.463                          | 0.915                          | 0.490                          | 0.433                          |
|       | $t$ -test (PC3)  | 0.476                          | 0.075                          | 0.448                          | 0.994                          | 0.617                          | 0.448                          | 0.488                          |
|       | $t$ -test (PC4)  | <u>0.036</u>                   | <u>2e-05</u>                   | <u>0.050</u>                   | 0.889                          | 0.831                          | <u>0.050</u>                   | <u>0.030</u>                   |
|       | $t$ -test* (PC1) | 1.000                          | 0.473                          | 1.000                          | <u><math>\leq 1e-08</math></u> | 1.000                          | 1.000                          | 1.000                          |
|       | $t$ -test* (PC2) | 1.000                          | 0.820                          | 1.000                          | 1.000                          | 1.000                          | 1.000                          | 1.000                          |
|       | $t$ -test* (PC3) | 1.000                          | 1.000                          | 1.000                          | 1.000                          | 1.000                          | 1.000                          | 1.000                          |
|       | $t$ -test* (PC4) | 0.576                          | <u>4e-04</u>                   | 0.742                          | 1.000                          | 1.000                          | 0.748                          | 0.534                          |
| III   | % var. (PC1)     | 17.1                           | 49.8                           | 43.9                           | 43.8                           | 14.5                           | 80.7                           | 13.4                           |
|       | % var. (PC2)     | 10.6                           | 6.2                            | 7.4                            | 5.0                            | 6.0                            | 2.4                            | 9.8                            |
|       | % var. (PC3)     | 9.8                            | 5.2                            | 6.6                            | 4.9                            | 5.1                            | 2.3                            | 7.9                            |
|       | % var. (PC4)     | 9.1                            | 4.1                            | 5.0                            | 4.2                            | 4.2                            | 1.8                            | 6.4                            |
|       | $t$ -test (PC1)  | <u><math>\leq 1e-08</math></u> | <u><math>\leq 1e-08</math></u> | <u><math>\leq 1e-08</math></u> | <u><math>\leq 1e-08</math></u> | <u><math>\leq 1e-08</math></u> | <u><math>\leq 1e-08</math></u> | <u><math>\leq 1e-08</math></u> |
|       | $t$ -test (PC2)  | 0.345                          | 0.965                          | 0.939                          | 0.820                          | <u>0.018</u>                   | 0.954                          | 0.785                          |
|       | $t$ -test (PC3)  | <u>4e-05</u>                   | 0.800                          | 0.574                          | 0.559                          | <u>0.008</u>                   | 0.819                          | 0.245                          |
|       | $t$ -test (PC4)  | 0.291                          | 0.544                          | 0.317                          | 0.545                          | 0.418                          | 0.731                          | 0.764                          |
|       | $t$ -test* (PC1) | <u><math>\leq 1e-08</math></u> | <u><math>\leq 1e-08</math></u> | <u><math>\leq 1e-08</math></u> | <u><math>\leq 1e-08</math></u> | <u><math>\leq 1e-08</math></u> | <u><math>\leq 1e-08</math></u> | <u><math>\leq 1e-08</math></u> |
|       | $t$ -test* (PC2) | 1.000                          | 1.000                          | 1.000                          | 1.000                          | 0.309                          | 1.000                          | 1.000                          |
|       | $t$ -test* (PC3) | <u>5e-04</u>                   | 1.000                          | 1.000                          | 1.000                          | 0.154                          | 1.000                          | 1.000                          |
|       | $t$ -test* (PC4) | 1.000                          | 1.000                          | 1.000                          | 1.000                          | 1.000                          | 1.000                          | 1.000                          |

**Table S3.3** Percentage of explained variance (% var.) and  $t$ -test  $p$ -values before ( $t$ -test) and after ( $t$ -test\*) weighted Bonferroni correction of the first four PCs for model size 200, parameter set 1, and  $n = 30$  runs per configuration. Case I weights two similar setups, case II compares setups with a small implementation difference, and case III compares setups with a different parameter.  $P$ -values lower than 0.05 are underlined, while  $p$ -values lower than 0.01 are double-underlined.

| Comp. | Data             | Outputs          |                  |                  |                  |                  |                  |                  |
|-------|------------------|------------------|------------------|------------------|------------------|------------------|------------------|------------------|
|       |                  | $P^s$            | $P^w$            | $P^c$            | $\bar{E}^s$      | $\bar{E}^w$      | $\bar{C}$        | $\tilde{A}$      |
| I     | % var. (PC1)     | 17.3             | 20.2             | 21.0             | 13.5             | 13.7             | 20.9             | 18.8             |
|       | % var. (PC2)     | 16.2             | 16.7             | 18.2             | 12.6             | 12.0             | 18.2             | 16.5             |
|       | % var. (PC3)     | 9.7              | 9.4              | 10.0             | 9.2              | 7.8              | 10.1             | 9.0              |
|       | % var. (PC4)     | 8.6              | 8.5              | 9.2              | 6.4              | 7.0              | 9.1              | 8.3              |
|       | $t$ -test (PC1)  | 0.192            | 0.294            | 0.280            | 0.985            | 0.378            | 0.280            | 0.240            |
|       | $t$ -test (PC2)  | 0.362            | 0.109            | 0.163            | 0.194            | 0.136            | 0.162            | 0.210            |
|       | $t$ -test (PC3)  | 0.996            | <u>0.050</u>     | <u>0.036</u>     | 0.565            | 0.301            | <u>0.036</u>     | <u>0.023</u>     |
|       | $t$ -test (PC4)  | <u>0.014</u>     | <u>0.445</u>     | <u>0.737</u>     | <u>0.015</u>     | <u>0.025</u>     | <u>0.746</u>     | <u>0.877</u>     |
|       | $t$ -test* (PC1) | 1.000            | 1.000            | 1.000            | 1.000            | 1.000            | 1.000            | 1.000            |
|       | $t$ -test* (PC2) | 1.000            | 0.650            | 0.891            | 1.000            | 1.000            | 0.892            | 1.000            |
|       | $t$ -test* (PC3) | 1.000            | 0.528            | 0.362            | 1.000            | 1.000            | 0.360            | 0.260            |
|       | $t$ -test* (PC4) | 0.166            | 1.000            | 1.000            | 0.238            | 0.360            | 1.000            | 1.000            |
| II    | % var. (PC1)     | 32.7             | 30.6             | 34.1             | 48.1             | 33.6             | 34.0             | 29.8             |
|       | % var. (PC2)     | 9.0              | 10.9             | 11.1             | 7.7              | 7.0              | 11.1             | 10.8             |
|       | % var. (PC3)     | 8.7              | 9.4              | 9.0              | 5.8              | 6.6              | 9.0              | 8.7              |
|       | % var. (PC4)     | 7.1              | 6.9              | 7.3              | 3.9              | 5.7              | 7.3              | 6.6              |
|       | $t$ -test (PC1)  | <u>&lt;1e-08</u> | <u>&lt;1e-08</u> | <u>&lt;1e-08</u> | <u>&lt;1e-08</u> | <u>&lt;1e-08</u> | <u>&lt;1e-08</u> | <u>&lt;1e-08</u> |
|       | $t$ -test (PC2)  | 0.703            | 0.430            | 0.553            | 0.798            | 0.563            | 0.552            | 0.589            |
|       | $t$ -test (PC3)  | 0.887            | 0.703            | 0.451            | 0.772            | 0.664            | 0.450            | 0.306            |
|       | $t$ -test (PC4)  | 0.584            | 0.840            | 0.936            | 0.674            | 0.933            | 0.937            | 0.857            |
|       | $t$ -test* (PC1) | <u>&lt;1e-08</u> | <u>&lt;1e-08</u> | <u>&lt;1e-08</u> | <u>&lt;1e-08</u> | <u>&lt;1e-08</u> | <u>&lt;1e-08</u> | <u>&lt;1e-08</u> |
|       | $t$ -test* (PC2) | 1.000            | 1.000            | 1.000            | 1.000            | 1.000            | 1.000            | 1.000            |
|       | $t$ -test* (PC3) | 1.000            | 1.000            | 1.000            | 1.000            | 1.000            | 1.000            | 1.000            |
|       | $t$ -test* (PC4) | 1.000            | 1.000            | 1.000            | 1.000            | 1.000            | 1.000            | 1.000            |
| III   | % var. (PC1)     | 21.4             | 20.1             | 22.4             | 15.9             | 17.6             | 29.0             | 20.4             |
|       | % var. (PC2)     | 14.9             | 18.0             | 18.6             | 12.7             | 12.4             | 16.2             | 17.0             |
|       | % var. (PC3)     | 9.8              | 9.9              | 9.9              | 10.1             | 7.2              | 9.5              | 9.0              |
|       | % var. (PC4)     | 7.4              | 7.8              | 8.3              | 6.2              | 6.6              | 7.3              | 7.6              |
|       | $t$ -test (PC1)  | <u>&lt;1e-08</u> | <u>3e-05</u>     | <u>1e-07</u>     | <u>8e-08</u>     | <u>&lt;1e-08</u> | <u>&lt;1e-08</u> | <u>4e-06</u>     |
|       | $t$ -test (PC2)  | 0.171            | <u>0.003</u>     | 0.060            | <u>0.039</u>     | 0.416            | 0.502            | <u>0.044</u>     |
|       | $t$ -test (PC3)  | 0.609            | 0.092            | 0.111            | 0.950            | 0.066            | <u>0.027</u>     | 0.141            |
|       | $t$ -test (PC4)  | 0.611            | 0.229            | 0.742            | 0.087            | 0.448            | 0.381            | 0.651            |
|       | $t$ -test* (PC1) | <u>&lt;1e-08</u> | <u>2e-04</u>     | <u>6e-07</u>     | <u>5e-07</u>     | <u>&lt;1e-08</u> | <u>&lt;1e-08</u> | <u>2e-05</u>     |
|       | $t$ -test* (PC2) | 1.000            | 0.019            | 0.323            | 0.304            | 1.000            | 1.000            | 0.261            |
|       | $t$ -test* (PC3) | 1.000            | 0.929            | 1.000            | 1.000            | 0.919            | 0.286            | 1.000            |
|       | $t$ -test* (PC4) | 1.000            | 1.000            | 1.000            | 1.000            | 1.000            | 1.000            | 1.000            |

**Table S3.4** Percentage of explained variance (% var.) and  $t$ -test  $p$ -values before ( $t$ -test) and after ( $t$ -test\*) weighted Bonferroni correction of the first four PCs for model size 200, parameter set 2, and  $n = 30$  runs per configuration. Case I weights two similar setups, case II compares setups with a small implementation difference, and case III compares setups with a different parameter.  $P$ -values lower than 0.05 are underlined, while  $p$ -values lower than 0.01 are double-underlined.

| Comp. | Data             | Outputs          |                  |                  |                  |                  |                  |                  |
|-------|------------------|------------------|------------------|------------------|------------------|------------------|------------------|------------------|
|       |                  | $P^s$            | $P^w$            | $P^c$            | $\bar{E}^s$      | $\bar{E}^w$      | $\bar{C}$        | $\tilde{A}$      |
| I     | % var. (PC1)     | 19.1             | 13.0             | 15.9             | 11.7             | 8.2              | 15.8             | 10.9             |
|       | % var. (PC2)     | 8.6              | 7.5              | 8.7              | 6.4              | 6.2              | 8.6              | 6.4              |
|       | % var. (PC3)     | 7.1              | 6.8              | 7.5              | 5.6              | 4.5              | 7.4              | 6.1              |
|       | % var. (PC4)     | 6.4              | 6.5              | 6.6              | 5.3              | 4.3              | 6.6              | 5.8              |
|       | $t$ -test (PC1)  | 0.530            | 0.836            | 0.804            | 0.784            | 0.378            | 0.805            | 0.879            |
|       | $t$ -test (PC2)  | <u>0.021</u>     | 0.057            | <u>0.012</u>     | 0.115            | 0.915            | <u>0.012</u>     | <u>0.041</u>     |
|       | $t$ -test (PC3)  | 0.319            | 0.608            | 0.491            | 0.081            | 0.372            | 0.496            | 0.389            |
|       | $t$ -test (PC4)  | 0.763            | 0.200            | 0.872            | 0.473            | 0.327            | 0.868            | 0.524            |
|       | $t$ -test* (PC1) | 1.000            | 1.000            | 1.000            | 1.000            | 1.000            | 1.000            | 1.000            |
|       | $t$ -test* (PC2) | 0.240            | 0.757            | 0.135            | 1.000            | 1.000            | 0.136            | 0.633            |
|       | $t$ -test* (PC3) | 1.000            | 1.000            | 1.000            | 1.000            | 1.000            | 1.000            | 1.000            |
|       | $t$ -test* (PC4) | 1.000            | 1.000            | 1.000            | 1.000            | 1.000            | 1.000            | 1.000            |
| II    | % var. (PC1)     | 20.1             | 19.3             | 16.4             | 77.2             | 8.0              | 16.2             | 11.4             |
|       | % var. (PC2)     | 10.7             | 10.5             | 11.1             | 2.6              | 6.1              | 11.0             | 8.8              |
|       | % var. (PC3)     | 7.0              | 8.0              | 7.3              | 1.9              | 4.7              | 7.2              | 6.2              |
|       | % var. (PC4)     | 5.9              | 5.3              | 6.3              | 1.3              | 4.1              | 6.3              | 5.5              |
|       | $t$ -test (PC1)  | 0.042            | <u>&lt;1e-08</u> | 0.108            | <u>&lt;1e-08</u> | 0.017            | 0.109            | 0.390            |
|       | $t$ -test (PC2)  | 0.128            | <u>0.029</u>     | 0.106            | 0.720            | 0.175            | 0.107            | 0.086            |
|       | $t$ -test (PC3)  | <u>0.004</u>     | 0.110            | <u>0.006</u>     | 0.885            | 0.909            | <u>0.006</u>     | <u>0.002</u>     |
|       | $t$ -test (PC4)  | 0.767            | 0.401            | 0.966            | 0.978            | 0.060            | 0.954            | 0.631            |
|       | $t$ -test* (PC1) | 0.209            | <u>&lt;1e-08</u> | 0.661            | <u>&lt;1e-08</u> | 0.211            | 0.669            | 1.000            |
|       | $t$ -test* (PC2) | 1.000            | 0.276            | 0.955            | 1.000            | 1.000            | 0.971            | 0.975            |
|       | $t$ -test* (PC3) | 0.055            | 1.000            | 0.079            | 1.000            | 1.000            | 0.077            | <u>0.028</u>     |
|       | $t$ -test* (PC4) | 1.000            | 1.000            | 1.000            | 1.000            | 1.000            | 1.000            | 1.000            |
| III   | % var. (PC1)     | 38.6             | 79.2             | 74.3             | 73.6             | 32.4             | 94.0             | 29.1             |
|       | % var. (PC2)     | 9.4              | 2.6              | 3.4              | 2.8              | 4.4              | 0.8              | 7.9              |
|       | % var. (PC3)     | 7.6              | 2.4              | 3.2              | 2.4              | 4.2              | 0.7              | 7.7              |
|       | % var. (PC4)     | 6.9              | 2.0              | 2.7              | 2.0              | 3.7              | 0.6              | 5.7              |
|       | $t$ -test (PC1)  | <u>&lt;1e-08</u> | <u>&lt;1e-08</u> | <u>&lt;1e-08</u> | <u>&lt;1e-08</u> | <u>&lt;1e-08</u> | <u>&lt;1e-08</u> | <u>&lt;1e-08</u> |
|       | $t$ -test (PC2)  | 0.183            | 0.966            | 0.792            | 0.662            | 0.979            | 0.878            | 0.792            |
|       | $t$ -test (PC3)  | 0.734            | 0.906            | 0.826            | 0.976            | 0.777            | 0.951            | 0.754            |
|       | $t$ -test (PC4)  | 0.602            | 0.800            | 0.587            | 0.827            | 0.979            | 0.875            | 0.555            |
|       | $t$ -test* (PC1) | <u>&lt;1e-08</u> | <u>&lt;1e-08</u> | <u>&lt;1e-08</u> | <u>&lt;1e-08</u> | <u>&lt;1e-08</u> | <u>&lt;1e-08</u> | <u>&lt;1e-08</u> |
|       | $t$ -test* (PC2) | 1.000            | 1.000            | 1.000            | 1.000            | 1.000            | 1.000            | 1.000            |
|       | $t$ -test* (PC3) | 1.000            | 1.000            | 1.000            | 1.000            | 1.000            | 1.000            | 1.000            |
|       | $t$ -test* (PC4) | 1.000            | 1.000            | 1.000            | 1.000            | 1.000            | 1.000            | 1.000            |

**Table S3.5** Percentage of explained variance (% var.) and  $t$ -test  $p$ -values before ( $t$ -test) and after ( $t$ -test\*) weighted Bonferroni correction of the first four PCs for model size 400, parameter set 1, and  $n = 30$  runs per configuration. Case I weights two similar setups, case II compares setups with a small implementation difference, and case III compares setups with a different parameter.  $P$ -values lower than 0.05 are underlined, while  $p$ -values lower than 0.01 are double-underlined.

| Comp. | Data             | Outputs          |                  |                  |                  |                  |                  |                  |
|-------|------------------|------------------|------------------|------------------|------------------|------------------|------------------|------------------|
|       |                  | $P^s$            | $P^w$            | $P^c$            | $\bar{E}^s$      | $\bar{E}^w$      | $\bar{C}$        | $\tilde{A}$      |
| I     | % var. (PC1)     | 16.4             | 19.2             | 20.0             | 12.7             | 13.1             | 19.9             | 17.8             |
|       | % var. (PC2)     | 13.9             | 16.5             | 17.0             | 11.5             | 11.2             | 16.9             | 15.1             |
|       | % var. (PC3)     | 12.1             | 10.8             | 11.8             | 9.8              | 8.0              | 11.8             | 11.0             |
|       | % var. (PC4)     | 8.8              | 9.2              | 9.9              | 8.5              | 6.8              | 9.8              | 8.9              |
|       | $t$ -test (PC1)  | 0.919            | 0.925            | 0.942            | 0.856            | 0.778            | 0.941            | 0.992            |
|       | $t$ -test (PC2)  | 0.694            | 0.474            | 0.492            | 0.867            | 0.444            | 0.490            | 0.483            |
|       | $t$ -test (PC3)  | 0.278            | 0.228            | 0.268            | 0.514            | 0.250            | 0.268            | 0.298            |
|       | $t$ -test (PC4)  | 0.923            | 0.884            | 0.998            | 0.350            | 0.721            | 0.999            | 0.956            |
|       | $t$ -test* (PC1) | 1.000            | 1.000            | 1.000            | 1.000            | 1.000            | 1.000            | 1.000            |
|       | $t$ -test* (PC2) | 1.000            | 1.000            | 1.000            | 1.000            | 1.000            | 1.000            | 1.000            |
|       | $t$ -test* (PC3) | 1.000            | 1.000            | 1.000            | 1.000            | 1.000            | 1.000            | 1.000            |
|       | $t$ -test* (PC4) | 1.000            | 1.000            | 1.000            | 1.000            | 1.000            | 1.000            | 1.000            |
| II    | % var. (PC1)     | 66.1             | 62.7             | 66.7             | 80.2             | 68.2             | 66.6             | 61.2             |
|       | % var. (PC2)     | 5.1              | 6.8              | 6.3              | 2.3              | 3.9              | 6.3              | 6.6              |
|       | % var. (PC3)     | 4.1              | 5.0              | 4.7              | 1.9              | 3.0              | 4.7              | 4.9              |
|       | % var. (PC4)     | 3.2              | 4.2              | 3.9              | 1.7              | 2.5              | 3.9              | 4.2              |
|       | $t$ -test (PC1)  | <u>&lt;1e-08</u> | <u>&lt;1e-08</u> | <u>&lt;1e-08</u> | <u>&lt;1e-08</u> | <u>&lt;1e-08</u> | <u>&lt;1e-08</u> | <u>&lt;1e-08</u> |
|       | $t$ -test (PC2)  | 0.726            | 0.631            | 0.631            | 0.908            | 0.739            | 0.631            | 0.608            |
|       | $t$ -test (PC3)  | 0.601            | 0.763            | 0.773            | 0.838            | 0.827            | 0.774            | 0.842            |
|       | $t$ -test (PC4)  | 0.732            | 0.694            | 0.651            | 0.963            | 0.799            | 0.650            | 0.600            |
|       | $t$ -test* (PC1) | <u>&lt;1e-08</u> | <u>&lt;1e-08</u> | <u>&lt;1e-08</u> | <u>&lt;1e-08</u> | <u>&lt;1e-08</u> | <u>&lt;1e-08</u> | <u>&lt;1e-08</u> |
|       | $t$ -test* (PC2) | 1.000            | 1.000            | 1.000            | 1.000            | 1.000            | 1.000            | 1.000            |
|       | $t$ -test* (PC3) | 1.000            | 1.000            | 1.000            | 1.000            | 1.000            | 1.000            | 1.000            |
|       | $t$ -test* (PC4) | 1.000            | 1.000            | 1.000            | 1.000            | 1.000            | 1.000            | 1.000            |
| III   | % var. (PC1)     | 49.1             | 46.8             | 51.3             | 36.3             | 43.7             | 65.5             | 45.1             |
|       | % var. (PC2)     | 8.3              | 10.2             | 9.9              | 9.7              | 7.2              | 6.8              | 10.1             |
|       | % var. (PC3)     | 6.1              | 7.4              | 7.2              | 7.0              | 5.3              | 5.1              | 7.1              |
|       | % var. (PC4)     | 5.7              | 5.7              | 5.6              | 5.5              | 4.3              | 3.8              | 5.7              |
|       | $t$ -test (PC1)  | <u>&lt;1e-08</u> | <u>&lt;1e-08</u> | <u>&lt;1e-08</u> | <u>&lt;1e-08</u> | <u>&lt;1e-08</u> | <u>&lt;1e-08</u> | <u>&lt;1e-08</u> |
|       | $t$ -test (PC2)  | 0.833            | 0.855            | 0.963            | 0.572            | 0.854            | 0.970            | 0.968            |
|       | $t$ -test (PC3)  | 0.686            | 0.522            | 0.527            | 0.923            | 0.510            | 0.560            | 0.519            |
|       | $t$ -test (PC4)  | 0.709            | 0.711            | 0.814            | 0.623            | 0.985            | 0.815            | 0.749            |
|       | $t$ -test* (PC1) | <u>&lt;1e-08</u> | <u>&lt;1e-08</u> | <u>&lt;1e-08</u> | <u>&lt;1e-08</u> | <u>&lt;1e-08</u> | <u>&lt;1e-08</u> | <u>&lt;1e-08</u> |
|       | $t$ -test* (PC2) | 1.000            | 1.000            | 1.000            | 1.000            | 1.000            | 1.000            | 1.000            |
|       | $t$ -test* (PC3) | 1.000            | 1.000            | 1.000            | 1.000            | 1.000            | 1.000            | 1.000            |
|       | $t$ -test* (PC4) | 1.000            | 1.000            | 1.000            | 1.000            | 1.000            | 1.000            | 1.000            |

**Table S3.6** Percentage of explained variance (% var.) and  $t$ -test  $p$ -values before ( $t$ -test) and after ( $t$ -test\*) weighted Bonferroni correction of the first four PCs for model size 400, parameter set 2, and  $n = 30$  runs per configuration. Case I weights two similar setups, case II compares setups with a small implementation difference, and case III compares setups with a different parameter.  $P$ -values lower than 0.05 are underlined, while  $p$ -values lower than 0.01 are double-underlined.

| Comp. | Data             | Outputs          |                  |                  |                  |                  |                  |                  |
|-------|------------------|------------------|------------------|------------------|------------------|------------------|------------------|------------------|
|       |                  | $P^s$            | $P^w$            | $P^c$            | $\bar{E}^s$      | $\bar{E}^w$      | $\bar{C}$        | $\tilde{A}$      |
| I     | % var. (PC1)     | 16.4             | 10.6             | 13.0             | 10.4             | 6.8              | 12.9             | 9.1              |
|       | % var. (PC2)     | 9.0              | 8.6              | 9.6              | 6.4              | 5.5              | 9.5              | 7.7              |
|       | % var. (PC3)     | 7.8              | 7.7              | 8.2              | 5.8              | 4.9              | 8.2              | 6.9              |
|       | % var. (PC4)     | 6.4              | 6.0              | 6.8              | 5.2              | 4.5              | 6.7              | 5.5              |
|       | $t$ -test (PC1)  | 0.316            | 0.341            | 0.307            | 0.502            | 0.577            | 0.307            | 0.262            |
|       | $t$ -test (PC2)  | 0.376            | 0.320            | 0.414            | 0.146            | 0.823            | 0.414            | 0.359            |
|       | $t$ -test (PC3)  | 0.783            | 0.785            | 0.832            | 0.613            | 0.280            | 0.837            | 0.872            |
|       | $t$ -test (PC4)  | 0.496            | 0.646            | 0.491            | 0.141            | 0.581            | 0.492            | 0.507            |
|       | $t$ -test* (PC1) | 1.000            | 1.000            | 1.000            | 1.000            | 1.000            | 1.000            | 1.000            |
|       | $t$ -test* (PC2) | 1.000            | 1.000            | 1.000            | 1.000            | 1.000            | 1.000            | 1.000            |
|       | $t$ -test* (PC3) | 1.000            | 1.000            | 1.000            | 1.000            | 1.000            | 1.000            | 1.000            |
|       | $t$ -test* (PC4) | 1.000            | 1.000            | 1.000            | 1.000            | 1.000            | 1.000            | 1.000            |
|       | % var. (PC1)     | 23.3             | 44.2             | 18.2             | 93.1             | 9.6              | 18.0             | 12.0             |
|       | % var. (PC2)     | 8.7              | 5.9              | 9.1              | 0.6              | 5.0              | 9.0              | 7.8              |
|       | % var. (PC3)     | 6.3              | 4.1              | 7.0              | 0.5              | 4.5              | 6.9              | 5.7              |
|       | % var. (PC4)     | 5.9              | 3.9              | 6.6              | 0.4              | 4.2              | 6.6              | 5.6              |
| II    | $t$ -test (PC1)  | <u>&lt;1e-08</u> | <u>&lt;1e-08</u> | <u>&lt;1e-08</u> | <u>&lt;1e-08</u> | <u>1e-05</u>     | <u>&lt;1e-08</u> | <u>&lt;1e-08</u> |
|       | $t$ -test (PC2)  | <u>0.005</u>     | 0.609            | <u>0.015</u>     | 0.906            | 0.066            | <u>0.015</u>     | 0.060            |
|       | $t$ -test (PC3)  | 0.819            | 0.792            | 0.956            | 0.948            | 0.395            | 0.952            | 0.759            |
|       | $t$ -test (PC4)  | 0.775            | 0.913            | 0.826            | 0.959            | 0.485            | 0.827            | 0.875            |
|       | $t$ -test* (PC1) | <u>&lt;1e-08</u> | <u>&lt;1e-08</u> | <u>&lt;1e-08</u> | <u>&lt;1e-08</u> | <u>1e-04</u>     | <u>&lt;1e-08</u> | <u>&lt;1e-08</u> |
|       | $t$ -test* (PC2) | 0.055            | 1.000            | 0.162            | 1.000            | 1.000            | 0.163            | 0.767            |
|       | $t$ -test* (PC3) | 1.000            | 1.000            | 1.000            | 1.000            | 1.000            | 1.000            | 1.000            |
|       | $t$ -test* (PC4) | 1.000            | 1.000            | 1.000            | 1.000            | 1.000            | 1.000            | 1.000            |
|       | % var. (PC1)     | 73.6             | 94.0             | 92.6             | 92.6             | 64.2             | 98.6             | 60.0             |
|       | % var. (PC2)     | 3.7              | 0.8              | 1.0              | 0.7              | 2.5              | 0.2              | 4.6              |
|       | % var. (PC3)     | 2.8              | 0.6              | 0.8              | 0.6              | 2.3              | 0.1              | 3.6              |
|       | % var. (PC4)     | 2.7              | 0.5              | 0.6              | 0.5              | 1.9              | 0.1              | 2.6              |
|       | $t$ -test (PC1)  | <u>&lt;1e-08</u> | <u>&lt;1e-08</u> | <u>&lt;1e-08</u> | <u>&lt;1e-08</u> | <u>&lt;1e-08</u> | <u>&lt;1e-08</u> | <u>&lt;1e-08</u> |
|       | $t$ -test (PC2)  | 0.813            | 0.966            | 0.934            | 0.920            | 0.697            | 0.972            | 0.789            |
|       | $t$ -test (PC3)  | 0.723            | 0.996            | 0.993            | 0.880            | 0.830            | 0.994            | 0.954            |
|       | $t$ -test (PC4)  | 0.819            | 0.981            | 0.804            | 0.986            | 0.876            | 0.933            | 0.891            |
| III   | $t$ -test* (PC1) | <u>&lt;1e-08</u> | <u>&lt;1e-08</u> | <u>&lt;1e-08</u> | <u>&lt;1e-08</u> | <u>&lt;1e-08</u> | <u>&lt;1e-08</u> | <u>&lt;1e-08</u> |
|       | $t$ -test* (PC2) | 1.000            | 1.000            | 1.000            | 1.000            | 1.000            | 1.000            | 1.000            |
|       | $t$ -test* (PC3) | 1.000            | 1.000            | 1.000            | 1.000            | 1.000            | 1.000            | 1.000            |
|       | $t$ -test* (PC4) | 1.000            | 1.000            | 1.000            | 1.000            | 1.000            | 1.000            | 1.000            |

**Table S3.7** Percentage of explained variance (% var.) and  $t$ -test  $p$ -values before ( $t$ -test) and after ( $t$ -test\*) weighted Bonferroni correction of the first four PCs for model size 800, parameter set 1, and  $n = 30$  runs per configuration. Case I weights two similar setups, case II compares setups with a small implementation difference, and case III compares setups with a different parameter.  $P$ -values lower than 0.05 are underlined, while  $p$ -values lower than 0.01 are double-underlined.



| Comp. | Data             | Outputs          |                  |                  |                  |                  |                  |                  |
|-------|------------------|------------------|------------------|------------------|------------------|------------------|------------------|------------------|
|       |                  | $P^s$            | $P^w$            | $P^c$            | $\bar{E}^s$      | $\bar{E}^w$      | $\bar{C}$        | $\tilde{A}$      |
| I     | % var. (PC1)     | 18.0             | 21.2             | 21.8             | 13.9             | 14.3             | 21.8             | 19.8             |
|       | % var. (PC2)     | 16.4             | 19.0             | 19.6             | 12.3             | 13.6             | 19.6             | 17.7             |
|       | % var. (PC3)     | 11.0             | 10.4             | 11.4             | 9.1              | 9.1              | 11.4             | 10.8             |
|       | % var. (PC4)     | 7.9              | 8.6              | 8.9              | 6.6              | 6.8              | 8.9              | 8.2              |
|       | $t$ -test (PC1)  | 0.597            | 0.979            | 0.819            | 0.813            | 0.788            | 0.819            | 0.927            |
|       | $t$ -test (PC2)  | 0.236            | 0.168            | 0.187            | 0.150            | 0.150            | 0.187            | 0.181            |
|       | $t$ -test (PC3)  | <u>0.035</u>     | <u>0.028</u>     | <u>0.026</u>     | <u>0.038</u>     | 0.071            | <u>0.026</u>     | <u>0.021</u>     |
|       | $t$ -test (PC4)  | <u>0.170</u>     | <u>0.295</u>     | <u>0.227</u>     | <u>0.144</u>     | 0.139            | <u>0.230</u>     | <u>0.215</u>     |
|       | $t$ -test* (PC1) | 1.000            | 1.000            | 1.000            | 1.000            | 1.000            | 1.000            | 1.000            |
|       | $t$ -test* (PC2) | 1.000            | 0.885            | 0.953            | 1.000            | 1.000            | 0.954            | 1.000            |
|       | $t$ -test* (PC3) | 0.319            | 0.266            | 0.224            | 0.418            | 0.776            | 0.225            | 0.198            |
|       | $t$ -test* (PC4) | 1.000            | 1.000            | 1.000            | 1.000            | 1.000            | 1.000            | 1.000            |
| II    | % var. (PC1)     | 87.4             | 85.1             | 87.4             | 94.0             | 88.3             | 87.3             | 84.2             |
|       | % var. (PC2)     | 1.8              | 2.3              | 2.1              | 0.7              | 1.2              | 2.1              | 2.4              |
|       | % var. (PC3)     | 1.4              | 2.0              | 1.8              | 0.6              | 1.1              | 1.8              | 2.0              |
|       | % var. (PC4)     | 1.3              | 1.8              | 1.6              | 0.5              | 1.0              | 1.6              | 1.8              |
|       | $t$ -test (PC1)  | <u>&lt;1e-08</u> | <u>&lt;1e-08</u> | <u>&lt;1e-08</u> | <u>&lt;1e-08</u> | <u>&lt;1e-08</u> | <u>&lt;1e-08</u> | <u>&lt;1e-08</u> |
|       | $t$ -test (PC2)  | 0.987            | 0.952            | 0.978            | 0.996            | 0.999            | 0.978            | 0.988            |
|       | $t$ -test (PC3)  | 0.945            | 0.917            | 0.963            | 0.973            | 0.932            | 0.963            | 0.955            |
|       | $t$ -test (PC4)  | 0.975            | 0.996            | 0.988            | 0.986            | 0.972            | 0.988            | 0.995            |
|       | $t$ -test* (PC1) | <u>&lt;1e-08</u> | <u>&lt;1e-08</u> | <u>&lt;1e-08</u> | <u>&lt;1e-08</u> | <u>&lt;1e-08</u> | <u>&lt;1e-08</u> | <u>&lt;1e-08</u> |
|       | $t$ -test* (PC2) | 1.000            | 1.000            | 1.000            | 1.000            | 1.000            | 1.000            | 1.000            |
|       | $t$ -test* (PC3) | 1.000            | 1.000            | 1.000            | 1.000            | 1.000            | 1.000            | 1.000            |
|       | $t$ -test* (PC4) | 1.000            | 1.000            | 1.000            | 1.000            | 1.000            | 1.000            | 1.000            |
| III   | % var. (PC1)     | 75.9             | 72.8             | 76.4             | 66.0             | 71.7             | 86.0             | 71.8             |
|       | % var. (PC2)     | 4.2              | 5.6              | 5.1              | 4.2              | 3.7              | 2.8              | 5.5              |
|       | % var. (PC3)     | 2.9              | 3.7              | 3.3              | 3.9              | 2.8              | 1.8              | 3.7              |
|       | % var. (PC4)     | 2.1              | 2.7              | 2.5              | 2.7              | 2.0              | 1.7              | 2.7              |
|       | $t$ -test (PC1)  | <u>&lt;1e-08</u> | <u>&lt;1e-08</u> | <u>&lt;1e-08</u> | <u>&lt;1e-08</u> | <u>&lt;1e-08</u> | <u>&lt;1e-08</u> | <u>&lt;1e-08</u> |
|       | $t$ -test (PC2)  | 0.889            | 0.758            | 0.810            | 0.884            | 0.813            | 0.836            | 0.790            |
|       | $t$ -test (PC3)  | 0.755            | 0.810            | 0.857            | 0.748            | 0.794            | 0.788            | 0.891            |
|       | $t$ -test (PC4)  | 0.713            | 0.791            | 0.772            | 0.962            | 0.595            | 0.511            | 0.840            |
|       | $t$ -test* (PC1) | <u>&lt;1e-08</u> | <u>&lt;1e-08</u> | <u>&lt;1e-08</u> | <u>&lt;1e-08</u> | <u>&lt;1e-08</u> | <u>&lt;1e-08</u> | <u>&lt;1e-08</u> |
|       | $t$ -test* (PC2) | 1.000            | 1.000            | 1.000            | 1.000            | 1.000            | 1.000            | 1.000            |
|       | $t$ -test* (PC3) | 1.000            | 1.000            | 1.000            | 1.000            | 1.000            | 1.000            | 1.000            |
|       | $t$ -test* (PC4) | 1.000            | 1.000            | 1.000            | 1.000            | 1.000            | 1.000            | 1.000            |

**Table S3.8** Percentage of explained variance (% var.) and  $t$ -test  $p$ -values before ( $t$ -test) and after ( $t$ -test\*) weighted Bonferroni correction of the first four PCs for model size 800, parameter set 2, and  $n = 30$  runs per configuration. Case I weights two similar setups, case II compares setups with a small implementation difference, and case III compares setups with a different parameter.  $P$ -values lower than 0.05 are underlined, while  $p$ -values lower than 0.01 are double-underlined.

| Comp. | Data            | Outputs          |                  |                  |                  |                  |                  |              |
|-------|-----------------|------------------|------------------|------------------|------------------|------------------|------------------|--------------|
|       |                 | $P^s$            | $P^w$            | $P^c$            | $\overline{E}^s$ | $\overline{E}^w$ | $\overline{C}$   | $\tilde{A}$  |
| I     | #PCs (30% var.) | 3                | 4                | 4                | 5                | 6                | 4                | 5            |
|       | #PCs (50% var.) | 7                | 8                | 7                | 11               | 13               | 7                | 9            |
|       | #PCs (70% var.) | 12               | 15               | 13               | 19               | 24               | 13               | 18           |
|       | #PCs (90% var.) | 26               | 32               | 26               | 37               | 43               | 27               | 38           |
|       | MNV (30% var.)  | 0.211            | 0.383            | 0.365            | 0.322            | 0.553            | 0.365            | 0.517        |
|       | MNV (50% var.)  | 0.652            | 0.159            | 0.664            | 0.507            | 0.545            | 0.663            | 0.202        |
|       | MNV (70% var.)  | 0.215            | 0.312            | 0.193            | 0.729            | 0.663            | 0.192            | 0.406        |
|       | MNV (90% var.)  | 0.852            | 0.509            | 0.851            | 0.966            | 0.285            | 0.879            | 0.486        |
| II    | #PCs (30% var.) | 3                | 4                | 3                | 3                | 6                | 3                | 4            |
|       | #PCs (50% var.) | 6                | 8                | 6                | 8                | 13               | 6                | 9            |
|       | #PCs (70% var.) | 12               | 15               | 12               | 16               | 24               | 12               | 18           |
|       | #PCs (90% var.) | 25               | 32               | 25               | 34               | 43               | 26               | 38           |
|       | MNV (30% var.)  | <u>0.011</u>     | <u>0.010</u>     | 0.019            | <u>&lt;1e-08</u> | 0.273            | 0.019            | 0.032        |
|       | MNV (50% var.)  | <u>0.041</u>     | 0.060            | <u>0.044</u>     | <u>&lt;1e-08</u> | 0.176            | <u>0.044</u>     | <u>0.169</u> |
|       | MNV (70% var.)  | 0.070            | 0.013            | 0.152            | <u>&lt;1e-08</u> | 0.405            | 0.150            | 0.262        |
|       | MNV (90% var.)  | <u>0.023</u>     | <u>4e-05</u>     | 0.276            | <u>&lt;1e-08</u> | 0.448            | 0.256            | 0.496        |
| III   | #PCs (30% var.) | 3                | 2                | 2                | 3                | 6                | 1                | 4            |
|       | #PCs (50% var.) | 6                | 5                | 5                | 7                | 13               | 1                | 7            |
|       | #PCs (70% var.) | 10               | 11               | 9                | 14               | 24               | 5                | 15           |
|       | #PCs (90% var.) | 22               | 26               | 21               | 32               | 42               | 15               | 35           |
|       | MNV (30% var.)  | <u>2e-06</u>     | <u>&lt;1e-08</u> | <u>&lt;1e-08</u> | <u>&lt;1e-08</u> | <u>2e-08</u>     | *                | <u>3e-08</u> |
|       | MNV (50% var.)  | <u>9e-06</u>     | <u>&lt;1e-08</u> | <u>&lt;1e-08</u> | <u>&lt;1e-08</u> | <u>&lt;1e-08</u> | *                | <u>1e-06</u> |
|       | MNV (70% var.)  | <u>&lt;1e-08</u> | <u>&lt;1e-08</u> | <u>&lt;1e-08</u> | <u>&lt;1e-08</u> | <u>1e-08</u>     | <u>&lt;1e-08</u> | <u>5e-05</u> |
|       | MNV (90% var.)  | <u>&lt;1e-08</u> | <u>&lt;1e-08</u> | <u>&lt;1e-08</u> | <u>&lt;1e-08</u> | <u>0.001</u>     | <u>&lt;1e-08</u> | <u>6e-06</u> |

**Table S4.1** Number of principal components (#PCs) and MANOVA test  $p$ -values (MNV) for several percentages of explained variance for model size 100, parameter set 1, and  $n = 30$  runs per configuration. Case I weights two similar setups, case II compares setups with a small implementation difference, and case III compares setups with a different parameter. Output  $\tilde{A}$  refers to the concatenation of all outputs (range scaled). The MANOVA test is not applicable to one PC, and the respective  $p$ -values are replace with an asterisk (\*).  $P$ -values lower than 0.05 are underlined, while  $p$ -values lower than 0.01 are double-underlined.

| Comp. | Data            | Outputs          |                  |                  |                  |                  |                  |                  |
|-------|-----------------|------------------|------------------|------------------|------------------|------------------|------------------|------------------|
|       |                 | $P^s$            | $P^w$            | $P^c$            | $\bar{E}^s$      | $\bar{E}^w$      | $\bar{C}$        | $\tilde{A}$      |
| I     | #PCs (30% var.) | 2                | 2                | 2                | 3                | 3                | 2                | 2                |
|       | #PCs (50% var.) | 4                | 4                | 3                | 6                | 6                | 4                | 4                |
|       | #PCs (70% var.) | 8                | 7                | 6                | 13               | 13               | 6                | 8                |
|       | #PCs (90% var.) | 20               | 19               | 15               | 29               | 31               | 15               | 22               |
|       | MNV (30% var.)  | 0.236            | <u>0.035</u>     | 0.051            | 0.071            | <u>0.040</u>     | 0.051            | 0.068            |
|       | MNV (50% var.)  | 0.065            | <u>0.073</u>     | 0.043            | 0.150            | <u>0.198</u>     | 0.068            | 0.085            |
|       | MNV (70% var.)  | 0.292            | 0.303            | 0.189            | 0.106            | 0.570            | 0.189            | 0.425            |
|       | MNV (90% var.)  | 0.116            | 0.141            | 0.175            | 0.085            | 0.121            | 0.175            | 0.125            |
| II    | #PCs (30% var.) | 3                | 2                | 2                | 3                | 3                | 2                | 3                |
|       | #PCs (50% var.) | 5                | 5                | 4                | 6                | 6                | 4                | 5                |
|       | #PCs (70% var.) | 9                | 8                | 7                | 11               | 12               | 7                | 8                |
|       | #PCs (90% var.) | 20               | 19               | 15               | 27               | 29               | 15               | 22               |
|       | MNV (30% var.)  | <u>&lt;1e-08</u> | <u>7e-06</u>     | <u>2e-08</u>     | <u>&lt;1e-08</u> | <u>&lt;1e-08</u> | <u>2e-08</u>     | <u>8e-07</u>     |
|       | MNV (50% var.)  | <u>&lt;1e-08</u> | <u>&lt;1e-08</u> | <u>&lt;1e-08</u> | <u>&lt;1e-08</u> | <u>&lt;1e-08</u> | <u>&lt;1e-08</u> | <u>&lt;1e-08</u> |
|       | MNV (70% var.)  | <u>&lt;1e-08</u> | <u>&lt;1e-08</u> | <u>&lt;1e-08</u> | <u>&lt;1e-08</u> | <u>&lt;1e-08</u> | <u>&lt;1e-08</u> | <u>4e-08</u>     |
|       | MNV (90% var.)  | <u>&lt;1e-08</u> | <u>&lt;1e-08</u> | <u>&lt;1e-08</u> | <u>&lt;1e-08</u> | <u>&lt;1e-08</u> | <u>&lt;1e-08</u> | <u>5e-06</u>     |
| III   | #PCs (30% var.) | 2                | 2                | 2                | 3                | 3                | 2                | 2                |
|       | #PCs (50% var.) | 5                | 4                | 4                | 6                | 6                | 4                | 4                |
|       | #PCs (70% var.) | 9                | 8                | 7                | 13               | 13               | 7                | 8                |
|       | #PCs (90% var.) | 21               | 18               | 15               | 29               | 30               | 15               | 22               |
|       | MNV (30% var.)  | <u>0.009</u>     | 0.145            | 0.069            | 0.064            | 0.015            | <u>0.001</u>     | 0.078            |
|       | MNV (50% var.)  | <u>0.020</u>     | 0.050            | 0.016            | 0.034            | 0.036            | <u>4e-06</u>     | 0.021            |
|       | MNV (70% var.)  | 0.090            | 0.106            | 0.042            | 0.270            | <u>0.001</u>     | <u>2e-08</u>     | 0.078            |
|       | MNV (90% var.)  | <u>0.006</u>     | <u>0.001</u>     | 0.110            | 0.139            | <u>2e-04</u>     | <u>&lt;1e-08</u> | 0.147            |

**Table S4.2** Number of principal components (#PCs) and MANOVA test  $p$ -values (MNV) for several percentages of explained variance for model size 100, parameter set 2, and  $n = 30$  runs per configuration. Case I weights two similar setups, case II compares setups with a small implementation difference, and case III compares setups with a different parameter. Output  $\tilde{A}$  refers to the concatenation of all outputs (range scaled). The MANOVA test is not applicable to one PC, and the respective  $p$ -values are replace with an asterisk (\*).  $P$ -values lower than 0.05 are underlined, while  $p$ -values lower than 0.01 are double-underlined.

| Comp. | Data            | Outputs          |                  |                  |                  |                  |                  |                  |
|-------|-----------------|------------------|------------------|------------------|------------------|------------------|------------------|------------------|
|       |                 | $P^s$            | $P^w$            | $P^c$            | $\bar{E}^s$      | $\bar{E}^w$      | $\bar{C}$        | $\tilde{A}$      |
| I     | #PCs (30% var.) | 3                | 4                | 3                | 5                | 7                | 3                | 4                |
|       | #PCs (50% var.) | 6                | 8                | 6                | 10               | 14               | 7                | 9                |
|       | #PCs (70% var.) | 12               | 15               | 12               | 19               | 25               | 12               | 18               |
|       | #PCs (90% var.) | 25               | 32               | 25               | 36               | 43               | 26               | 38               |
|       | MNV (30% var.)  | 0.446            | 0.598            | 0.456            | 0.863            | 0.117            | 0.456            | 0.570            |
|       | MNV (50% var.)  | 0.788            | 0.102            | 0.767            | 0.293            | 0.521            | 0.846            | 0.143            |
|       | MNV (70% var.)  | 0.142            | 0.208            | 0.158            | 0.800            | 0.762            | 0.159            | 0.522            |
|       | MNV (90% var.)  | 0.287            | 0.214            | 0.157            | 0.123            | 0.699            | 0.187            | 0.356            |
| II    | #PCs (30% var.) | 3                | 4                | 3                | 1                | 6                | 3                | 4                |
|       | #PCs (50% var.) | 6                | 8                | 6                | 2                | 13               | 6                | 9                |
|       | #PCs (70% var.) | 11               | 15               | 12               | 8                | 24               | 12               | 18               |
|       | #PCs (90% var.) | 24               | 31               | 25               | 27               | 43               | 25               | 38               |
|       | MNV (30% var.)  | 0.719            | <u>2e-06</u>     | 0.674            | *                | 0.847            | 0.674            | 0.186            |
|       | MNV (50% var.)  | 0.400            | <u>&lt;1e-08</u> | 0.471            | <u>&lt;1e-08</u> | 0.780            | 0.471            | 0.547            |
|       | MNV (70% var.)  | 0.618            | <u>&lt;1e-08</u> | 0.800            | <u>&lt;1e-08</u> | 0.305            | 0.799            | 0.457            |
|       | MNV (90% var.)  | <u>0.022</u>     | <u>&lt;1e-08</u> | 0.276            | <u>&lt;1e-08</u> | 0.778            | 0.270            | <u>0.038</u>     |
| III   | #PCs (30% var.) | 3                | 1                | 1                | 1                | 5                | 1                | 3                |
|       | #PCs (50% var.) | 5                | 2                | 2                | 3                | 11               | 1                | 7                |
|       | #PCs (70% var.) | 9                | 6                | 6                | 9                | 21               | 1                | 15               |
|       | #PCs (90% var.) | 21               | 19               | 17               | 27               | 41               | 6                | 35               |
|       | MNV (30% var.)  | <u>&lt;1e-08</u> | *                | *                | *                | <u>&lt;1e-08</u> | *                | <u>&lt;1e-08</u> |
|       | MNV (50% var.)  | <u>&lt;1e-08</u> | <u>&lt;1e-08</u> | <u>&lt;1e-08</u> | <u>&lt;1e-08</u> | <u>&lt;1e-08</u> | *                | <u>6e-08</u>     |
|       | MNV (70% var.)  | <u>&lt;1e-08</u> | <u>&lt;1e-08</u> | <u>&lt;1e-08</u> | <u>&lt;1e-08</u> | <u>&lt;1e-08</u> | *                | <u>&lt;1e-08</u> |
|       | MNV (90% var.)  | <u>&lt;1e-08</u> | <u>&lt;1e-08</u> | <u>&lt;1e-08</u> | <u>&lt;1e-08</u> | <u>&lt;1e-08</u> | <u>&lt;1e-08</u> | <u>3e-08</u>     |

**Table S4.3** Number of principal components (#PCs) and MANOVA test  $p$ -values (MNV) for several percentages of explained variance for model size 200, parameter set 1, and  $n = 30$  runs per configuration. Case I weights two similar setups, case II compares setups with a small implementation difference, and case III compares setups with a different parameter. Output  $\tilde{A}$  refers to the concatenation of all outputs (range scaled). The MANOVA test is not applicable to one PC, and the respective  $p$ -values are replaced with an asterisk (\*).  $P$ -values lower than 0.05 are underlined, while  $p$ -values lower than 0.01 are double-underlined.

| Comp. | Data            | Outputs          |                  |                  |                  |                  |                  |                  |
|-------|-----------------|------------------|------------------|------------------|------------------|------------------|------------------|------------------|
|       |                 | $P^s$            | $P^w$            | $P^c$            | $\bar{E}^s$      | $\bar{E}^w$      | $\bar{C}$        | $\tilde{A}$      |
| I     | #PCs (30% var.) | 2                | 2                | 2                | 3                | 3                | 2                | 2                |
|       | #PCs (50% var.) | 4                | 4                | 4                | 6                | 6                | 4                | 4                |
|       | #PCs (70% var.) | 9                | 8                | 7                | 13               | 14               | 7                | 8                |
|       | #PCs (90% var.) | 21               | 19               | 15               | 29               | 31               | 15               | 21               |
|       | MNV (30% var.)  | 0.282            | 0.158            | 0.209            | 0.575            | 0.252            | 0.209            | 0.227            |
|       | MNV (50% var.)  | 0.072            | 0.082            | 0.102            | 0.205            | 0.165            | 0.102            | 0.084            |
|       | MNV (70% var.)  | 0.121            | 0.106            | 0.273            | 0.317            | 0.274            | 0.279            | 0.099            |
|       | MNV (90% var.)  | 0.138            | 0.264            | 0.322            | 0.342            | 0.652            | 0.322            | 0.244            |
| II    | #PCs (30% var.) | 1                | 1                | 1                | 1                | 1                | 1                | 2                |
|       | #PCs (50% var.) | 3                | 3                | 3                | 2                | 4                | 3                | 4                |
|       | #PCs (70% var.) | 7                | 7                | 6                | 6                | 9                | 6                | 7                |
|       | #PCs (90% var.) | 18               | 17               | 14               | 20               | 26               | 14               | 19               |
|       | MNV (30% var.)  | *                | *                | *                | *                | *                | *                | <u>&lt;1e-08</u> |
|       | MNV (50% var.)  | <u>&lt;1e-08</u> | <u>&lt;1e-08</u> | <u>&lt;1e-08</u> | <u>&lt;1e-08</u> | <u>&lt;1e-08</u> | <u>&lt;1e-08</u> | <u>&lt;1e-08</u> |
|       | MNV (70% var.)  | <u>&lt;1e-08</u> | <u>&lt;1e-08</u> | <u>&lt;1e-08</u> | <u>&lt;1e-08</u> | <u>&lt;1e-08</u> | <u>&lt;1e-08</u> | <u>&lt;1e-08</u> |
|       | MNV (90% var.)  | <u>&lt;1e-08</u> | <u>&lt;1e-08</u> | <u>&lt;1e-08</u> | <u>&lt;1e-08</u> | <u>&lt;1e-08</u> | <u>&lt;1e-08</u> | <u>&lt;1e-08</u> |
| III   | #PCs (30% var.) | 2                | 2                | 2                | 3                | 2                | 2                | 2                |
|       | #PCs (50% var.) | 4                | 4                | 3                | 5                | 6                | 3                | 4                |
|       | #PCs (70% var.) | 8                | 7                | 6                | 11               | 12               | 6                | 8                |
|       | #PCs (90% var.) | 19               | 18               | 15               | 28               | 30               | 14               | 20               |
|       | MNV (30% var.)  | <u>&lt;1e-08</u> | <u>6e-07</u>     | <u>6e-08</u>     | <u>1e-07</u>     | <u>&lt;1e-08</u> | <u>&lt;1e-08</u> | <u>1e-06</u>     |
|       | MNV (50% var.)  | <u>5e-08</u>     | <u>4e-07</u>     | <u>3e-08</u>     | <u>1e-07</u>     | <u>&lt;1e-08</u> | <u>&lt;1e-08</u> | <u>4e-06</u>     |
|       | MNV (70% var.)  | <u>1e-06</u>     | <u>&lt;1e-08</u> | <u>5e-07</u>     | <u>3e-05</u>     | <u>&lt;1e-08</u> | <u>&lt;1e-08</u> | <u>9e-07</u>     |
|       | MNV (90% var.)  | <u>&lt;1e-08</u> | <u>&lt;1e-08</u> | <u>&lt;1e-08</u> | <u>0.001</u>     | <u>&lt;1e-08</u> | <u>&lt;1e-08</u> | <u>0.001</u>     |

**Table S4.4** Number of principal components (#PCs) and MANOVA test  $p$ -values (MNV) for several percentages of explained variance for model size 200, parameter set 2, and  $n = 30$  runs per configuration. Case I weights two similar setups, case II compares setups with a small implementation difference, and case III compares setups with a different parameter. Output  $\tilde{A}$  refers to the concatenation of all outputs (range scaled). The MANOVA test is not applicable to one PC, and the respective  $p$ -values are replace with an asterisk (\*).  $P$ -values lower than 0.05 are underlined, while  $p$ -values lower than 0.01 are double-underlined.

| Comp. | Data            | Outputs          |                  |                  |                  |                  |              |                  |
|-------|-----------------|------------------|------------------|------------------|------------------|------------------|--------------|------------------|
|       |                 | $P^s$            | $P^w$            | $P^c$            | $\bar{E}^s$      | $\bar{E}^w$      | $\bar{C}$    | $\tilde{A}$      |
| I     | #PCs (30% var.) | 3                | 4                | 3                | 5                | 6                | 3            | 5                |
|       | #PCs (50% var.) | 6                | 8                | 6                | 10               | 13               | 7            | 9                |
|       | #PCs (70% var.) | 11               | 15               | 12               | 19               | 25               | 12           | 19               |
|       | #PCs (90% var.) | 24               | 32               | 25               | 36               | 43               | 26           | 39               |
|       | MNV (30% var.)  | 0.080            | 0.235            | 0.078            | 0.185            | 0.696            | 0.078        | 0.297            |
|       | MNV (50% var.)  | 0.267            | 0.514            | 0.278            | <u>0.020</u>     | 0.530            | 0.311        | 0.614            |
|       | MNV (70% var.)  | 0.241            | 0.611            | 0.344            | <u>0.044</u>     | 0.682            | 0.344        | 0.527            |
|       | MNV (90% var.)  | 0.528            | 0.258            | 0.548            | 0.105            | 0.746            | 0.577        | 0.704            |
| II    | #PCs (30% var.) | 2                | 3                | 3                | 1                | 6                | 3            | 4                |
|       | #PCs (50% var.) | 6                | 6                | 6                | 1                | 13               | 6            | 9                |
|       | #PCs (70% var.) | 11               | 12               | 11               | 1                | 24               | 12           | 18               |
|       | #PCs (90% var.) | 24               | 29               | 24               | 12               | 43               | 25           | 38               |
|       | MNV (30% var.)  | <u>0.038</u>     | <u>&lt;1e-08</u> | <u>0.004</u>     | *                | 0.035            | <u>0.004</u> | <u>0.007</u>     |
|       | MNV (50% var.)  | <u>2e-06</u>     | <u>&lt;1e-08</u> | <u>3e-04</u>     | *                | <u>0.034</u>     | <u>3e-04</u> | <u>3e-04</u>     |
|       | MNV (70% var.)  | <u>4e-05</u>     | <u>&lt;1e-08</u> | <u>0.002</u>     | *                | 0.049            | <u>0.001</u> | <u>2e-06</u>     |
|       | MNV (90% var.)  | <u>&lt;1e-08</u> | <u>&lt;1e-08</u> | <u>5e-08</u>     | <u>&lt;1e-08</u> | 0.467            | <u>1e-07</u> | <u>&lt;1e-08</u> |
| III   | #PCs (30% var.) | 1                | 1                | 1                | 1                | 1                | 1            | 2                |
|       | #PCs (50% var.) | 3                | 1                | 1                | 1                | 6                | 1            | 4                |
|       | #PCs (70% var.) | 6                | 1                | 1                | 1                | 17               | 1            | 11               |
|       | #PCs (90% var.) | 17               | 7                | 8                | 13               | 38               | 1            | 31               |
|       | MNV (30% var.)  | *                | *                | *                | *                | *                | *            | <u>&lt;1e-08</u> |
|       | MNV (50% var.)  | <u>&lt;1e-08</u> | *                | *                | *                | <u>&lt;1e-08</u> | *            | <u>&lt;1e-08</u> |
|       | MNV (70% var.)  | <u>&lt;1e-08</u> | *                | *                | *                | <u>&lt;1e-08</u> | *            | <u>&lt;1e-08</u> |
|       | MNV (90% var.)  | <u>&lt;1e-08</u> | <u>&lt;1e-08</u> | <u>&lt;1e-08</u> | <u>&lt;1e-08</u> | <u>&lt;1e-08</u> | *            | <u>&lt;1e-08</u> |

**Table S4.5** Number of principal components (#PCs) and MANOVA test  $p$ -values (MNV) for several percentages of explained variance for model size 400, parameter set 1, and  $n = 30$  runs per configuration. Case I weights two similar setups, case II compares setups with a small implementation difference, and case III compares setups with a different parameter. Output  $\tilde{A}$  refers to the concatenation of all outputs (range scaled). The MANOVA test is not applicable to one PC, and the respective  $p$ -values are replace with an asterisk (\*).  $P$ -values lower than 0.05 are underlined, while  $p$ -values lower than 0.01 are double-underlined.

| Comp. | Data            | Outputs          |                  |                  |                  |                  |                  |                  |
|-------|-----------------|------------------|------------------|------------------|------------------|------------------|------------------|------------------|
|       |                 | $P^s$            | $P^w$            | $P^c$            | $\bar{E}^s$      | $\bar{E}^w$      | $\bar{C}$        | $\tilde{A}$      |
| I     | #PCs (30% var.) | 2                | 2                | 2                | 3                | 3                | 2                | 2                |
|       | #PCs (50% var.) | 4                | 4                | 4                | 6                | 7                | 4                | 4                |
|       | #PCs (70% var.) | 8                | 7                | 6                | 12               | 14               | 6                | 8                |
|       | #PCs (90% var.) | 21               | 18               | 15               | 28               | 32               | 15               | 21               |
|       | MNV (30% var.)  | 0.921            | 0.772            | 0.790            | 0.924            | 0.579            | 0.788            | 0.783            |
|       | MNV (50% var.)  | 0.858            | 0.743            | 0.796            | 0.962            | 0.486            | 0.795            | 0.818            |
|       | MNV (70% var.)  | 0.836            | 0.801            | 0.775            | 0.897            | 0.734            | 0.775            | 0.895            |
|       | MNV (90% var.)  | 0.740            | 0.936            | 0.849            | 0.776            | 0.854            | 0.850            | 0.990            |
| II    | #PCs (30% var.) | 1                | 1                | 1                | 1                | 1                | 1                | 1                |
|       | #PCs (50% var.) | 1                | 1                | 1                | 1                | 1                | 1                | 1                |
|       | #PCs (70% var.) | 2                | 3                | 2                | 1                | 2                | 2                | 3                |
|       | #PCs (90% var.) | 10               | 10               | 8                | 8                | 15               | 8                | 11               |
|       | MNV (30% var.)  | *                | *                | *                | *                | *                | *                | *                |
|       | MNV (50% var.)  | *                | *                | *                | *                | *                | *                | *                |
|       | MNV (70% var.)  | <u>&lt;1e-08</u> | <u>&lt;1e-08</u> | <u>&lt;1e-08</u> | *                | <u>&lt;1e-08</u> | <u>&lt;1e-08</u> | <u>&lt;1e-08</u> |
|       | MNV (90% var.)  | <u>&lt;1e-08</u> | <u>&lt;1e-08</u> | <u>&lt;1e-08</u> | <u>&lt;1e-08</u> | <u>&lt;1e-08</u> | <u>&lt;1e-08</u> | <u>&lt;1e-08</u> |
| III   | #PCs (30% var.) | 1                | 1                | 1                | 1                | 1                | 1                | 1                |
|       | #PCs (50% var.) | 2                | 2                | 1                | 3                | 2                | 1                | 2                |
|       | #PCs (70% var.) | 5                | 4                | 4                | 8                | 7                | 2                | 5                |
|       | #PCs (90% var.) | 15               | 14               | 11               | 24               | 24               | 8                | 16               |
|       | MNV (30% var.)  | *                | *                | *                | *                | *                | *                | *                |
|       | MNV (50% var.)  | <u>&lt;1e-08</u> | <u>&lt;1e-08</u> | *                | <u>&lt;1e-08</u> | <u>&lt;1e-08</u> | *                | <u>&lt;1e-08</u> |
|       | MNV (70% var.)  | <u>&lt;1e-08</u> | <u>&lt;1e-08</u> | <u>&lt;1e-08</u> | <u>&lt;1e-08</u> | <u>&lt;1e-08</u> | <u>&lt;1e-08</u> | <u>&lt;1e-08</u> |
|       | MNV (90% var.)  | <u>&lt;1e-08</u> | <u>&lt;1e-08</u> | <u>&lt;1e-08</u> | <u>&lt;1e-08</u> | <u>&lt;1e-08</u> | <u>&lt;1e-08</u> | <u>&lt;1e-08</u> |

**Table S4.6** Number of principal components (#PCs) and MANOVA test  $p$ -values (MNV) for several percentages of explained variance for model size 400, parameter set 2, and  $n = 30$  runs per configuration. Case I weights two similar setups, case II compares setups with a small implementation difference, and case III compares setups with a different parameter. Output  $\tilde{A}$  refers to the concatenation of all outputs (range scaled). The MANOVA test is not applicable to one PC, and the respective  $p$ -values are replace with an asterisk (\*).  $P$ -values lower than 0.05 are underlined, while  $p$ -values lower than 0.01 are double-underlined.

| Comp. | Data            | Outputs          |                  |                  |              |                  |                  |                  |
|-------|-----------------|------------------|------------------|------------------|--------------|------------------|------------------|------------------|
|       |                 | $P^s$            | $P^w$            | $P^c$            | $\bar{E}^s$  | $\bar{E}^w$      | $\bar{C}$        | $\tilde{A}$      |
| I     | #PCs (30% var.) | 3                | 4                | 3                | 5            | 7                | 3                | 5                |
|       | #PCs (50% var.) | 6                | 8                | 7                | 10           | 14               | 7                | 10               |
|       | #PCs (70% var.) | 12               | 15               | 12               | 19           | 25               | 13               | 19               |
|       | #PCs (90% var.) | 25               | 32               | 25               | 36           | 43               | 26               | 39               |
|       | MNV (30% var.)  | 0.605            | 0.709            | 0.629            | 0.373        | 0.496            | 0.629            | 0.765            |
|       | MNV (50% var.)  | 0.879            | 0.633            | 0.904            | 0.295        | 0.265            | 0.904            | 0.738            |
|       | MNV (70% var.)  | 0.506            | 0.530            | 0.757            | <u>0.014</u> | 0.483            | 0.795            | 0.687            |
|       | MNV (90% var.)  | 0.521            | 0.817            | 0.617            | <u>0.004</u> | 0.338            | 0.630            | 0.276            |
| II    | #PCs (30% var.) | 2                | 1                | 3                | 1            | 6                | 3                | 4                |
|       | #PCs (50% var.) | 6                | 2                | 6                | 1            | 13               | 6                | 9                |
|       | #PCs (70% var.) | 11               | 8                | 12               | 1            | 24               | 12               | 17               |
|       | #PCs (90% var.) | 23               | 24               | 24               | 1            | 43               | 25               | 37               |
|       | MNV (30% var.)  | <u>&lt;1e-08</u> | *                | <u>&lt;1e-08</u> | *            | <u>1e-06</u>     | <u>&lt;1e-08</u> | <u>&lt;1e-08</u> |
|       | MNV (50% var.)  | <u>&lt;1e-08</u> | <u>&lt;1e-08</u> | <u>&lt;1e-08</u> | *            | <u>2e-04</u>     | <u>&lt;1e-08</u> | <u>&lt;1e-08</u> |
|       | MNV (70% var.)  | <u>&lt;1e-08</u> | <u>&lt;1e-08</u> | <u>&lt;1e-08</u> | *            | <u>0.001</u>     | <u>&lt;1e-08</u> | <u>&lt;1e-08</u> |
|       | MNV (90% var.)  | <u>&lt;1e-08</u> | <u>&lt;1e-08</u> | <u>&lt;1e-08</u> | *            | <u>0.013</u>     | <u>&lt;1e-08</u> | <u>&lt;1e-08</u> |
| III   | #PCs (30% var.) | 1                | 1                | 1                | 1            | 1                | 1                | 1                |
|       | #PCs (50% var.) | 1                | 1                | 1                | 1            | 1                | 1                | 1                |
|       | #PCs (70% var.) | 1                | 1                | 1                | 1            | 4                | 1                | 4                |
|       | #PCs (90% var.) | 9                | 1                | 1                | 1            | 26               | 1                | 21               |
|       | MNV (30% var.)  | *                | *                | *                | *            | *                | *                | *                |
|       | MNV (50% var.)  | *                | *                | *                | *            | *                | *                | *                |
|       | MNV (70% var.)  | *                | *                | *                | *            | <u>&lt;1e-08</u> | *                | <u>&lt;1e-08</u> |
|       | MNV (90% var.)  | <u>&lt;1e-08</u> | *                | *                | *            | <u>&lt;1e-08</u> | *                | <u>&lt;1e-08</u> |

**Table S4.7** Number of principal components (#PCs) and MANOVA test  $p$ -values (MNV) for several percentages of explained variance for model size 800, parameter set 1, and  $n = 30$  runs per configuration. Case I weights two similar setups, case II compares setups with a small implementation difference, and case III compares setups with a different parameter. Output  $\tilde{A}$  refers to the concatenation of all outputs (range scaled). The MANOVA test is not applicable to one PC, and the respective  $p$ -values are replace with an asterisk (\*).  $P$ -values lower than 0.05 are underlined, while  $p$ -values lower than 0.01 are double-underlined.



| Comp. | Data            | Outputs                 |                         |                         |                         |                         |                         |                         |
|-------|-----------------|-------------------------|-------------------------|-------------------------|-------------------------|-------------------------|-------------------------|-------------------------|
|       |                 | $P^s$                   | $P^w$                   | $P^c$                   | $\bar{E}^s$             | $\bar{E}^w$             | $\bar{C}$               | $\tilde{A}$             |
| I     | #PCs (30% var.) | 2                       | 2                       | 2                       | 3                       | 3                       | 2                       | 2                       |
|       | #PCs (50% var.) | 4                       | 3                       | 3                       | 6                       | 6                       | 3                       | 4                       |
|       | #PCs (70% var.) | 8                       | 7                       | 6                       | 13                      | 13                      | 6                       | 8                       |
|       | #PCs (90% var.) | 20                      | 17                      | 14                      | 28                      | 31                      | 15                      | 20                      |
|       | MNV (30% var.)  | 0.433                   | 0.389                   | 0.410                   | 0.090                   | 0.142                   | 0.410                   | 0.410                   |
|       | MNV (50% var.)  | 0.086                   | 0.078                   | 0.078                   | 0.087                   | 0.237                   | 0.078                   | 0.067                   |
|       | MNV (70% var.)  | 0.158                   | 0.240                   | 0.182                   | <u>0.022</u>            | 0.363                   | 0.182                   | 0.205                   |
|       | MNV (90% var.)  | 0.242                   | 0.274                   | 0.252                   | <u><u>0.005</u></u>     | 0.379                   | 0.285                   | 0.322                   |
| II    | #PCs (30% var.) | 1                       | 1                       | 1                       | 1                       | 1                       | 1                       | 1                       |
|       | #PCs (50% var.) | 1                       | 1                       | 1                       | 1                       | 1                       | 1                       | 1                       |
|       | #PCs (70% var.) | 1                       | 1                       | 1                       | 1                       | 1                       | 1                       | 1                       |
|       | #PCs (90% var.) | 3                       | 4                       | 3                       | 1                       | 3                       | 3                       | 4                       |
|       | MNV (30% var.)  | *                       | *                       | *                       | *                       | *                       | *                       | *                       |
|       | MNV (50% var.)  | *                       | *                       | *                       | *                       | *                       | *                       | *                       |
|       | MNV (70% var.)  | *                       | *                       | *                       | *                       | *                       | *                       | *                       |
|       | MNV (90% var.)  | <u><u>&lt;1e-08</u></u> | <u><u>&lt;1e-08</u></u> | <u><u>&lt;1e-08</u></u> | *                       | <u><u>&lt;1e-08</u></u> | <u><u>&lt;1e-08</u></u> | <u><u>&lt;1e-08</u></u> |
| III   | #PCs (30% var.) | 1                       | 1                       | 1                       | 1                       | 1                       | 1                       | 1                       |
|       | #PCs (50% var.) | 1                       | 1                       | 1                       | 1                       | 1                       | 1                       | 1                       |
|       | #PCs (70% var.) | 1                       | 1                       | 1                       | 2                       | 1                       | 1                       | 1                       |
|       | #PCs (90% var.) | 8                       | 8                       | 6                       | 15                      | 13                      | 3                       | 8                       |
|       | MNV (30% var.)  | *                       | *                       | *                       | *                       | *                       | *                       | *                       |
|       | MNV (50% var.)  | *                       | *                       | *                       | *                       | *                       | *                       | *                       |
|       | MNV (70% var.)  | *                       | *                       | *                       | <u>&lt;1e-08</u>        | *                       | *                       | *                       |
|       | MNV (90% var.)  | <u><u>&lt;1e-08</u></u> | <u><u>&lt;1e-08</u></u> | <u><u>&lt;1e-08</u></u> | <u><u>&lt;1e-08</u></u> | <u><u>&lt;1e-08</u></u> | <u><u>&lt;1e-08</u></u> | <u><u>&lt;1e-08</u></u> |

**Table S4.8** Number of principal components (#PCs) and MANOVA test  $p$ -values (MNV) for several percentages of explained variance for model size 800, parameter set 2, and  $n = 30$  runs per configuration. Case I weights two similar setups, case II compares setups with a small implementation difference, and case III compares setups with a different parameter. Output  $\tilde{A}$  refers to the concatenation of all outputs (range scaled). The MANOVA test is not applicable to one PC, and the respective  $p$ -values are replace with an asterisk (\*).  $P$ -values lower than 0.05 are underlined, while  $p$ -values lower than 0.01 are double-underlined.

| Comp. | Stat.          | Outputs          |                  |                  |                  |                  |                  |
|-------|----------------|------------------|------------------|------------------|------------------|------------------|------------------|
|       |                | $P^s$            | $P^w$            | $P^c$            | $\bar{E}^s$      | $\bar{E}^w$      | $\bar{C}$        |
| I     | max            | 0.841            | 0.340            | 0.293            | 0.499            | 0.471            | 0.828            |
|       | arg max        | 0.593            | 0.273            | 0.301            | 0.170            | 0.596            | 0.518            |
|       | min            | 0.598            | 0.896            | 0.900            | 0.326            | <u>0.012</u>     | 0.356            |
|       | arg min        | 0.284            | 0.343            | 0.519            | 1.000            | <u>0.555</u>     | 1.000            |
|       | $\bar{X}^{ss}$ | 0.995            | 0.415            | 0.967            | 0.679            | <u>0.017</u>     | 0.962            |
|       | $S^{ss}$       | 0.402            | 0.326            | 0.415            | 0.593            | 0.343            | 0.415            |
| II    | max            | <u>0.014</u>     | <u>3e-4</u>      | <u>0.024</u>     | <u>0.023</u>     | 0.494            | 0.171            |
|       | arg max        | <u>0.019</u>     | 0.307            | <u>0.077</u>     | 0.206            | 0.140            | <u>0.025</u>     |
|       | min            | 0.063            | 0.173            | 0.209            | 0.237            | <u>0.017</u>     | <u>0.037</u>     |
|       | arg min        | 0.720            | 0.184            | <u>0.017</u>     | 1.000            | 0.294            | 1.000            |
|       | $\bar{X}^{ss}$ | 0.244            | <u>&lt; 1e-8</u> | <u>0.012</u>     | <u>&lt; 1e-8</u> | 0.456            | <u>0.013</u>     |
|       | $S^{ss}$       | 0.751            | 0.685            | 0.826            | 0.196            | 0.404            | <u>0.826</u>     |
| III   | max            | <u>&lt; 1e-8</u> | <u>&lt; 1e-8</u> | <u>&lt; 1e-8</u> | <u>1e-7</u>      | <u>4e-4</u>      | <u>&lt; 1e-8</u> |
|       | arg max        | 0.066            | 0.345            | <u>0.001</u>     | <u>0.009</u>     | <u>0.044</u>     | 0.015            |
|       | min            | <u>0.004</u>     | <u>8e-5</u>      | <u>5e-5</u>      | 0.949            | <u>0.010</u>     | <u>&lt; 1e-8</u> |
|       | arg min        | <u>0.047</u>     | 0.402            | <u>0.015</u>     | 1.000            | <u>0.044</u>     | <u>2e-5</u>      |
|       | $\bar{X}^{ss}$ | <u>8e-8</u>      | <u>&lt; 1e-8</u> | <u>&lt; 1e-8</u> | <u>&lt; 1e-8</u> | <u>&lt; 1e-8</u> | <u>&lt; 1e-8</u> |
|       | $S^{ss}$       | <u>0.010</u>     | <u>0.014</u>     | 0.074            | <u>0.001</u>     | 0.388            | 0.457            |

**Table S5.1**  $P$ -values for the empirical selection of FMs for model size 400, parameter set 1,  $n = 10$  runs per configuration.  $P$ -values were obtained with the  $t$ -test for max, min,  $\bar{X}^{ss}$  and  $S^{ss}$  statistics, and with the Mann-Whitney U test for the arg max and arg min statistics. Case I weights two similar configurations, case II compares configurations with a small implementation difference, and case III compares configurations with a different parameter. Values lower than 0.05 are underlined, while values lower than 0.01 are double-underlined.

| Comp. | Data      | Outputs                                                                           |                                                                                   |                                                                                   |                                                                                   |                                                                                    |                                                                                     |                                                                                     |
|-------|-----------|-----------------------------------------------------------------------------------|-----------------------------------------------------------------------------------|-----------------------------------------------------------------------------------|-----------------------------------------------------------------------------------|------------------------------------------------------------------------------------|-------------------------------------------------------------------------------------|-------------------------------------------------------------------------------------|
|       |           | $P^s$                                                                             | $P^w$                                                                             | $P^c$                                                                             | $\overline{E}^s$                                                                  | $\overline{E}^w$                                                                   | $\overline{C}$                                                                      | $\tilde{A}$                                                                         |
| I     | #PCs      | 12                                                                                | 14                                                                                | 13                                                                                | 15                                                                                | 16                                                                                 | 13                                                                                  | 15                                                                                  |
|       | MNV       | 0.591                                                                             | 0.120                                                                             | 0.503                                                                             | 0.858                                                                             | 0.927                                                                              | 0.505                                                                               | 0.790                                                                               |
|       | $t$ -test | 0.662                                                                             | 0.575                                                                             | 0.539                                                                             | 0.492                                                                             | 0.364                                                                              | 0.539                                                                               | 0.504                                                                               |
|       | PCS       | 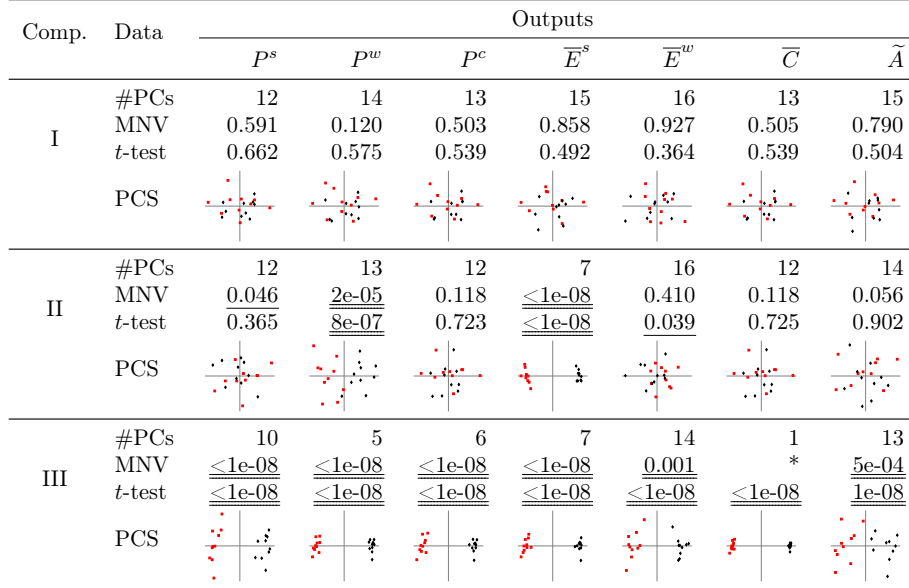 | 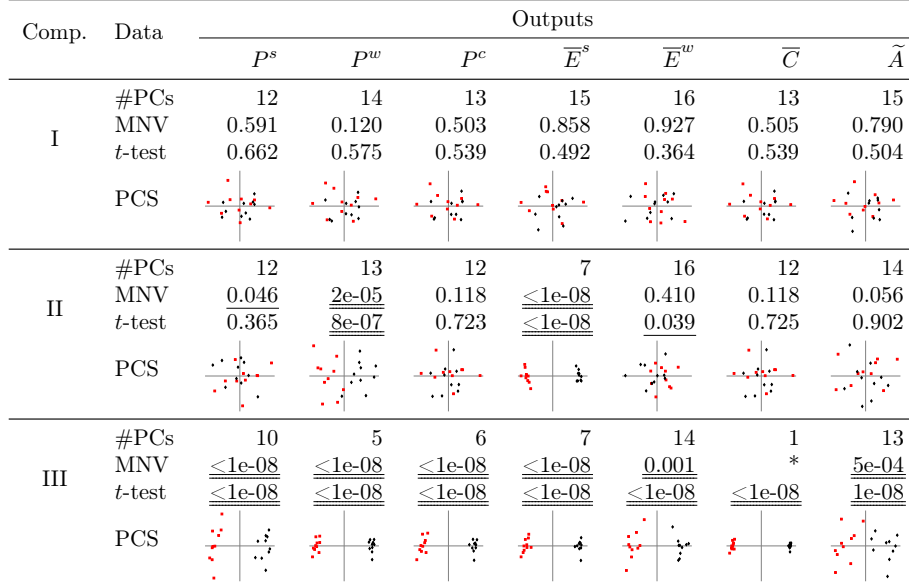 | 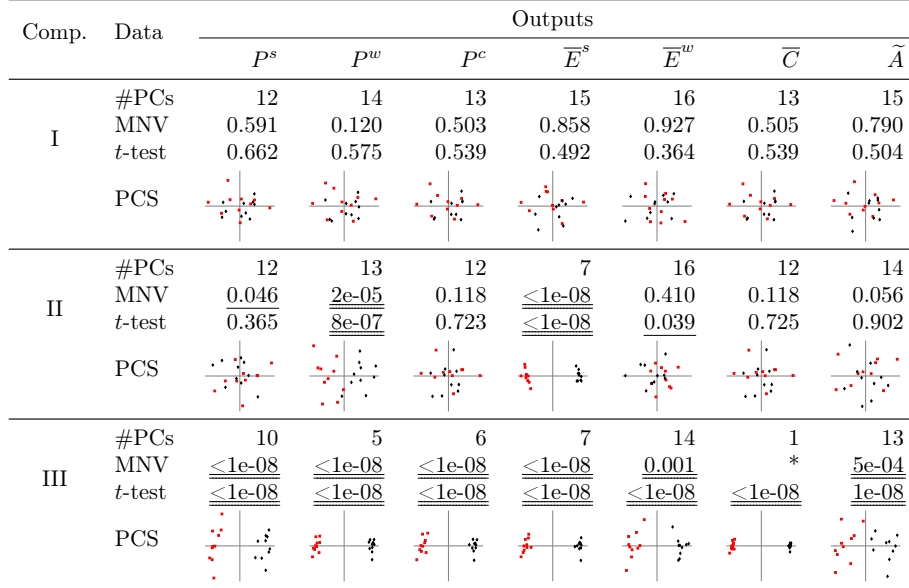 | 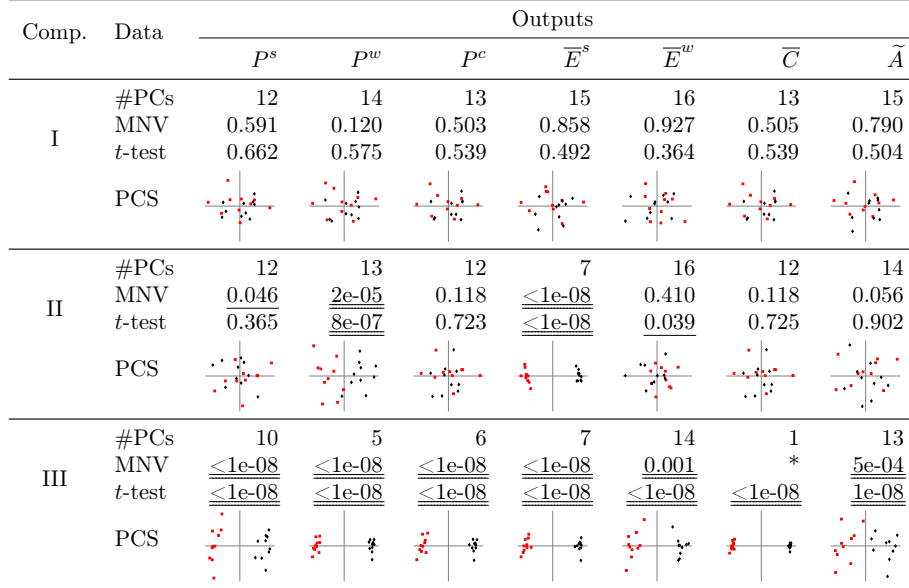 | 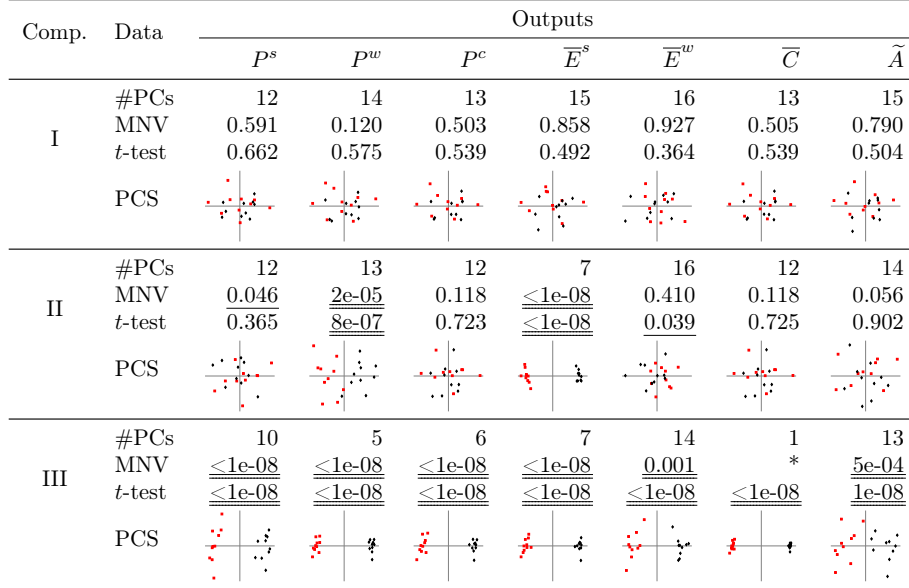 | 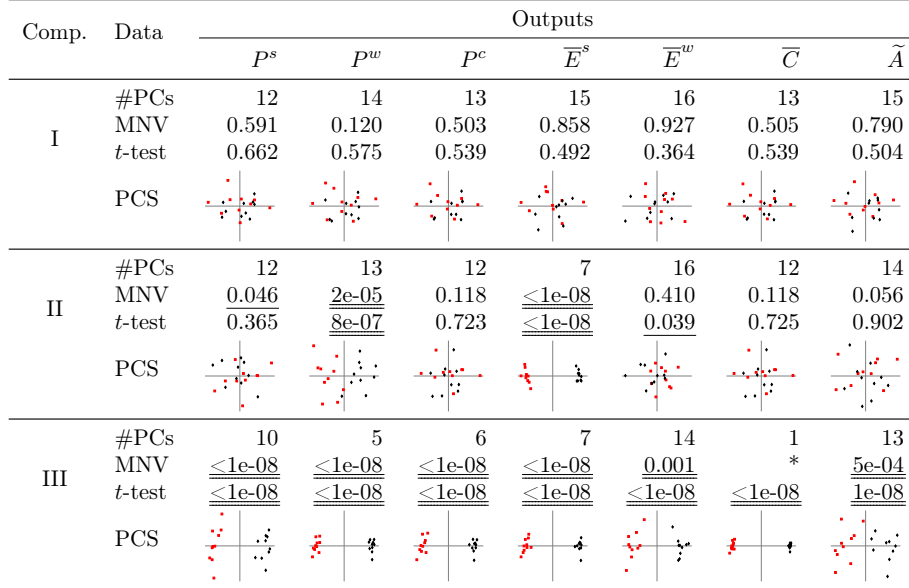 | 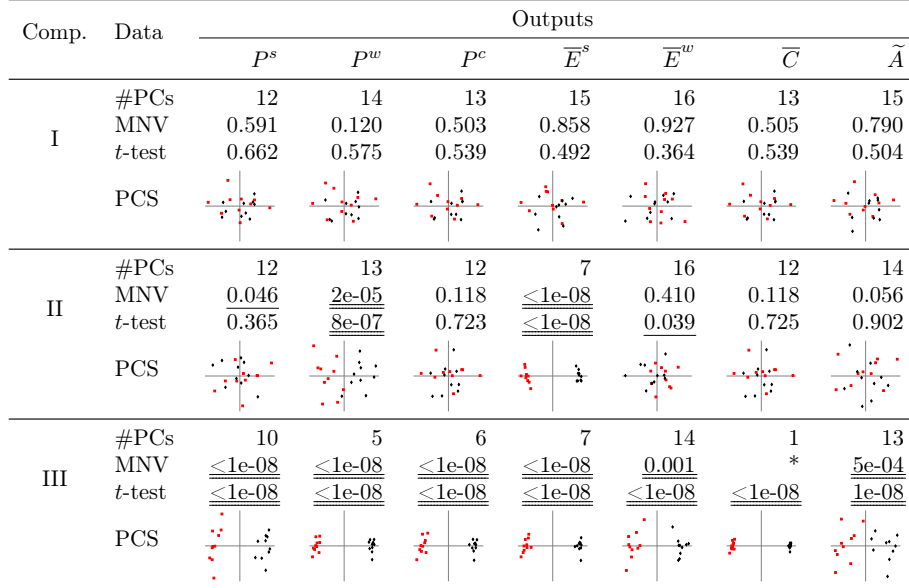 |
| II    | #PCs      | 12                                                                                | 13                                                                                | 12                                                                                | 7                                                                                 | 16                                                                                 | 12                                                                                  | 14                                                                                  |
|       | MNV       | 0.046                                                                             | <u>2e-05</u>                                                                      | 0.118                                                                             | <u>&lt;1e-08</u>                                                                  | 0.410                                                                              | 0.118                                                                               | 0.056                                                                               |
|       | $t$ -test | 0.365                                                                             | <u>8e-07</u>                                                                      | 0.723                                                                             | <u>&lt;1e-08</u>                                                                  | 0.039                                                                              | 0.725                                                                               | 0.902                                                                               |
|       | PCS       | 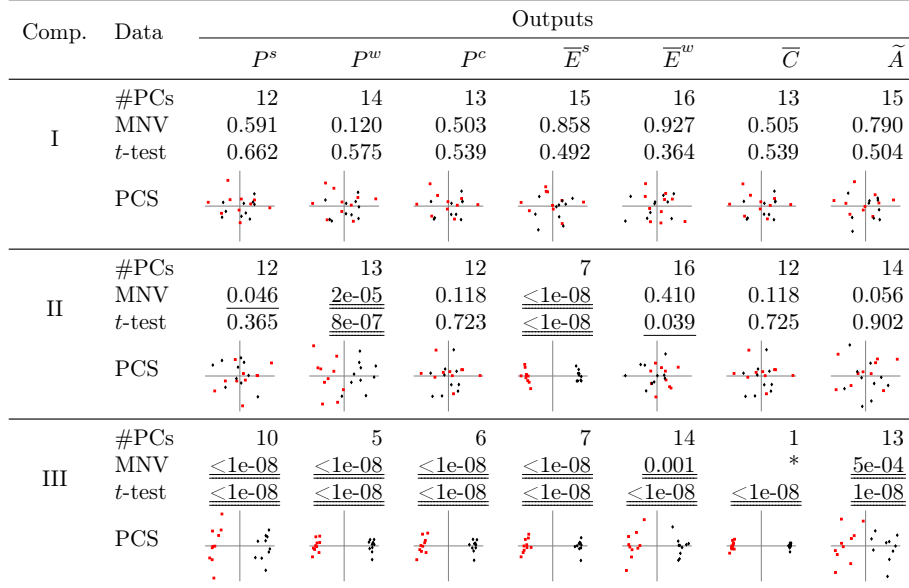 | 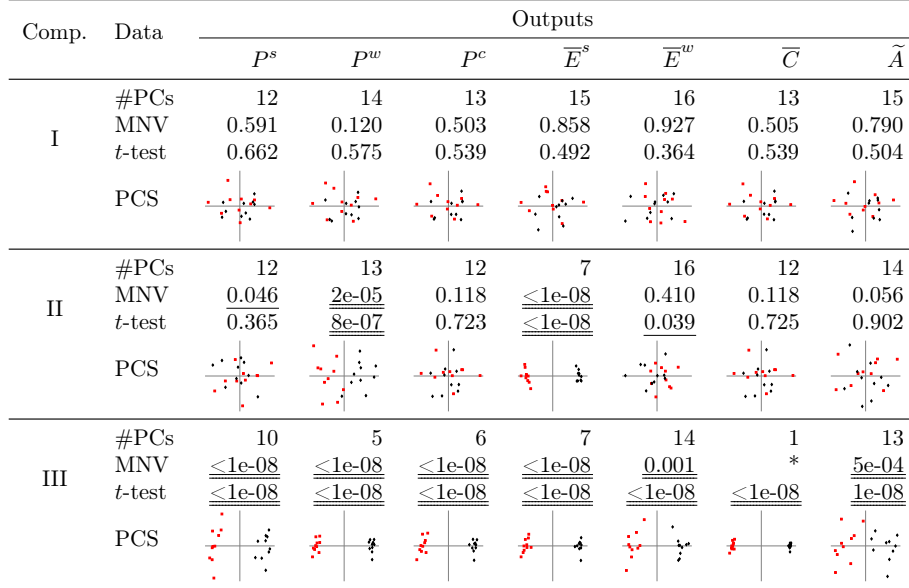 | 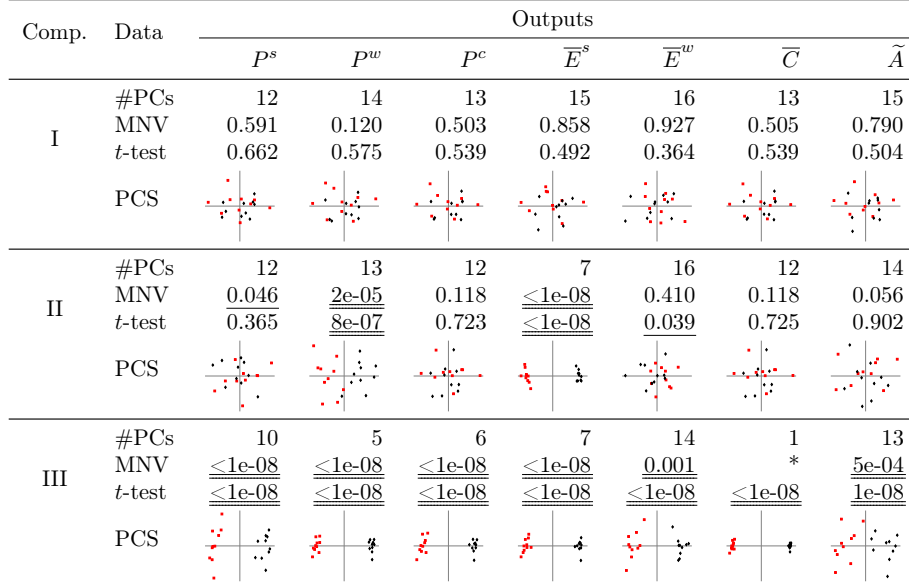 | 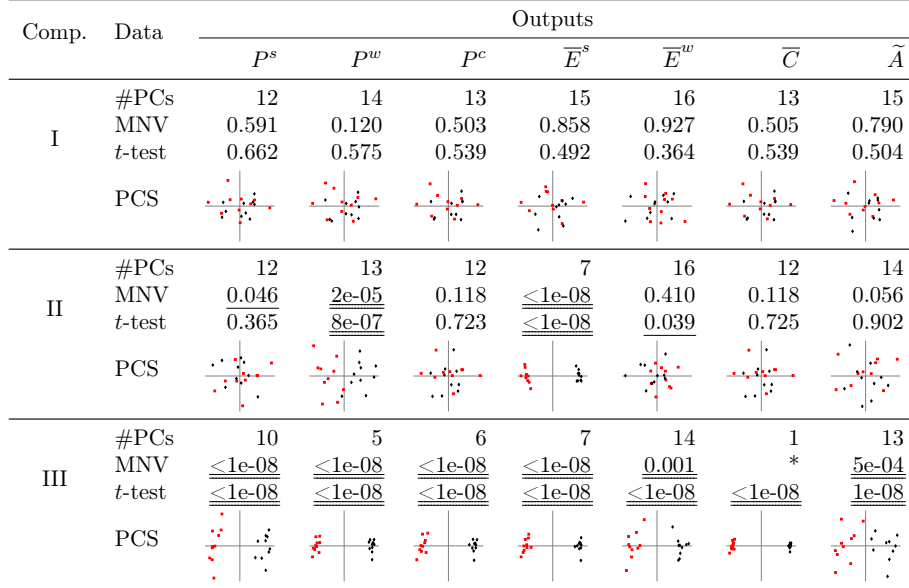 | 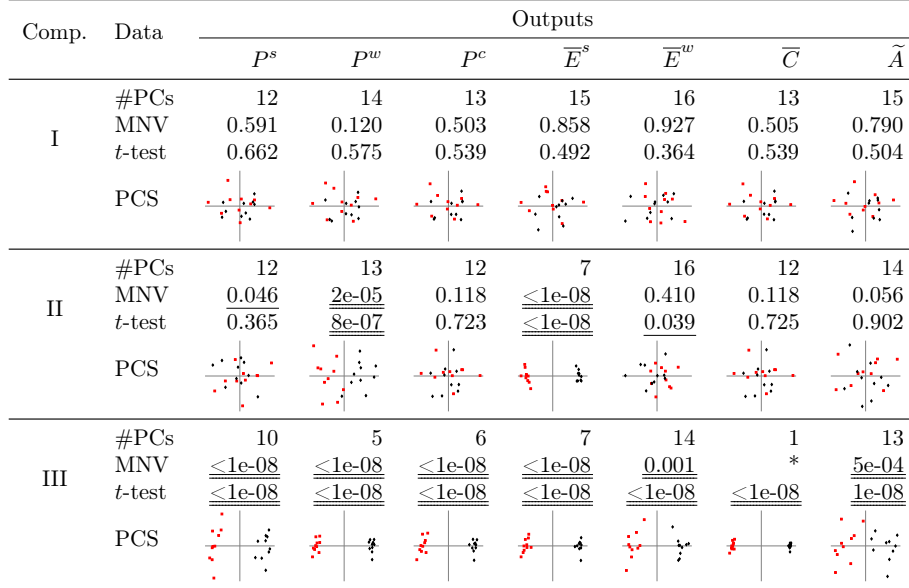 | 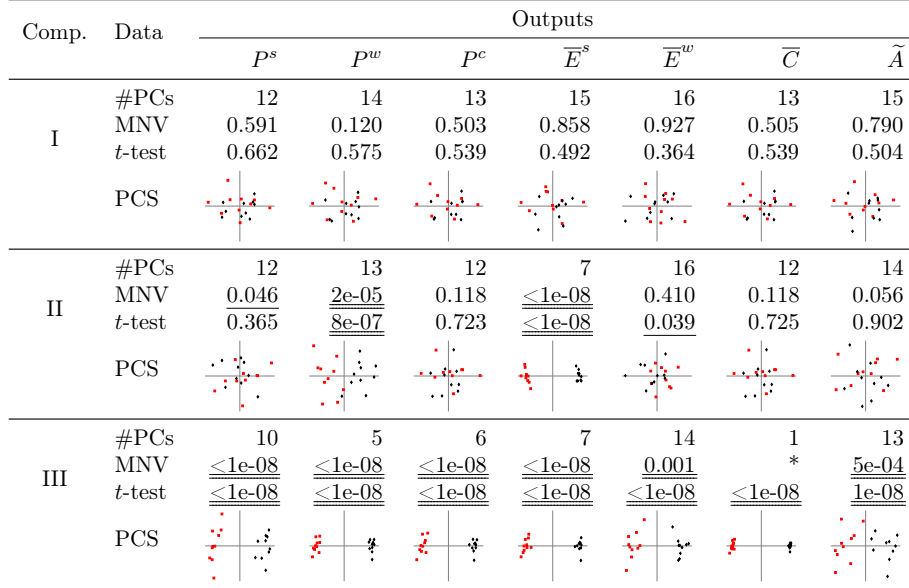 | 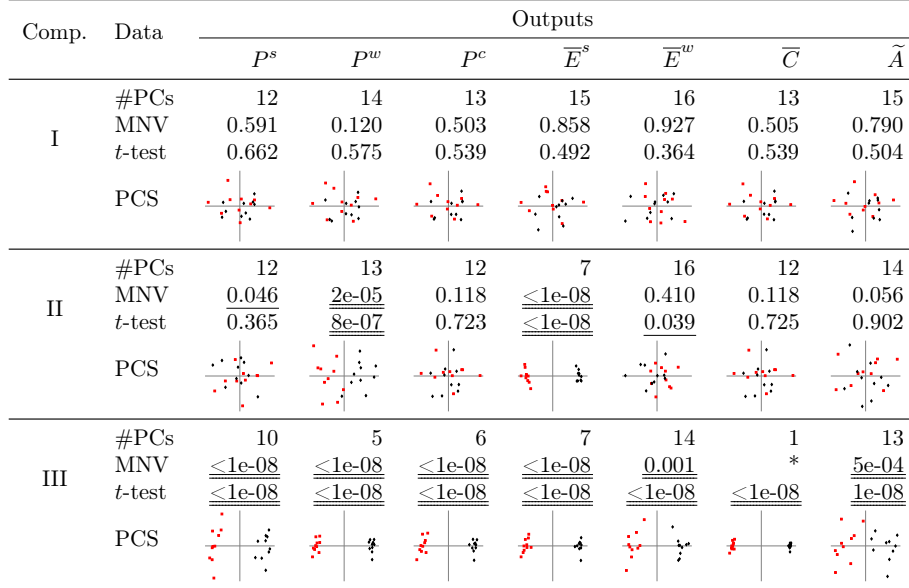 |
| III   | #PCs      | 10                                                                                | 5                                                                                 | 6                                                                                 | 7                                                                                 | 14                                                                                 | 1                                                                                   | 13                                                                                  |
|       | MNV       | <u>&lt;1e-08</u>                                                                  | <u>&lt;1e-08</u>                                                                  | <u>&lt;1e-08</u>                                                                  | <u>&lt;1e-08</u>                                                                  | <u>0.001</u>                                                                       | *                                                                                   | <u>5e-04</u>                                                                        |
|       | $t$ -test | <u>&lt;1e-08</u>                                                                  | <u>&lt;1e-08</u>                                                                  | <u>&lt;1e-08</u>                                                                  | <u>&lt;1e-08</u>                                                                  | <u>&lt;1e-08</u>                                                                   | <u>&lt;1e-08</u>                                                                    | <u>1e-08</u>                                                                        |
|       | PCS       | 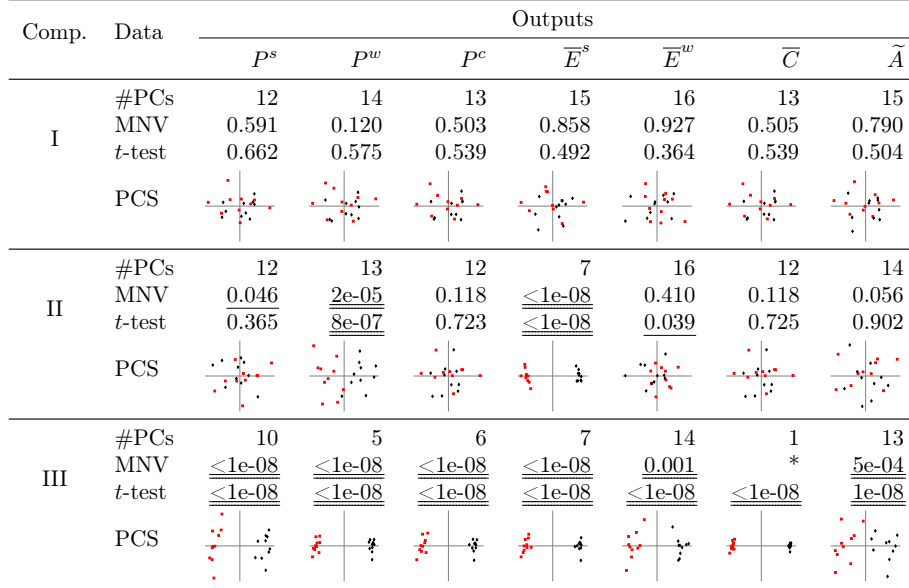 | 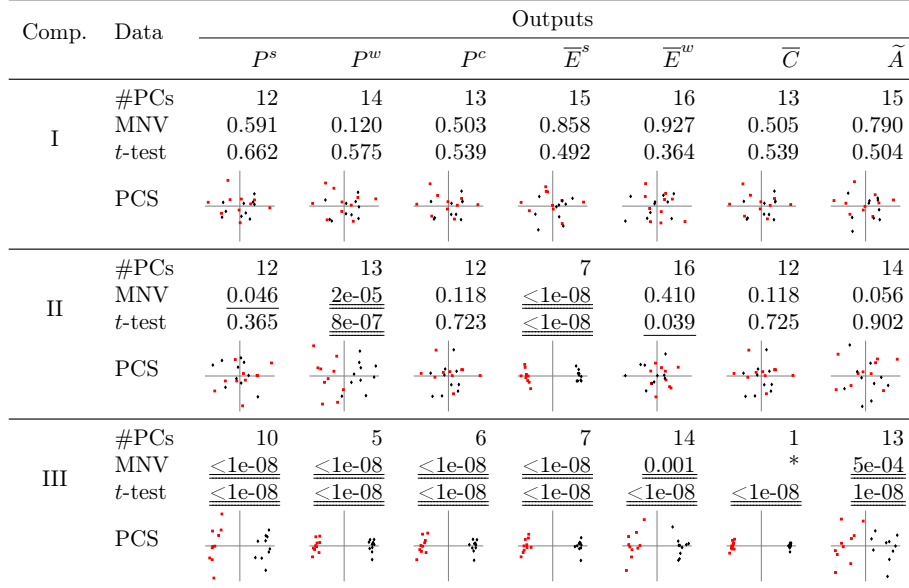 | 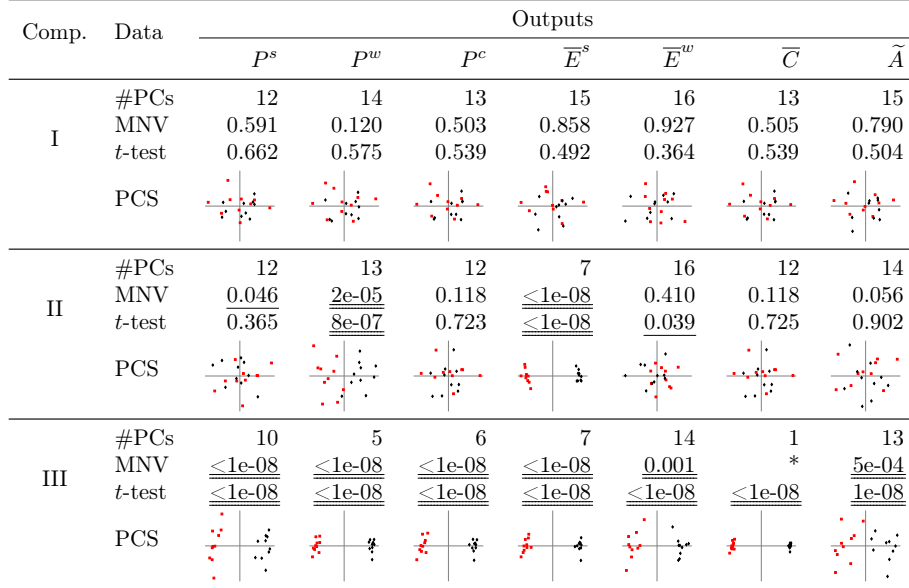 | 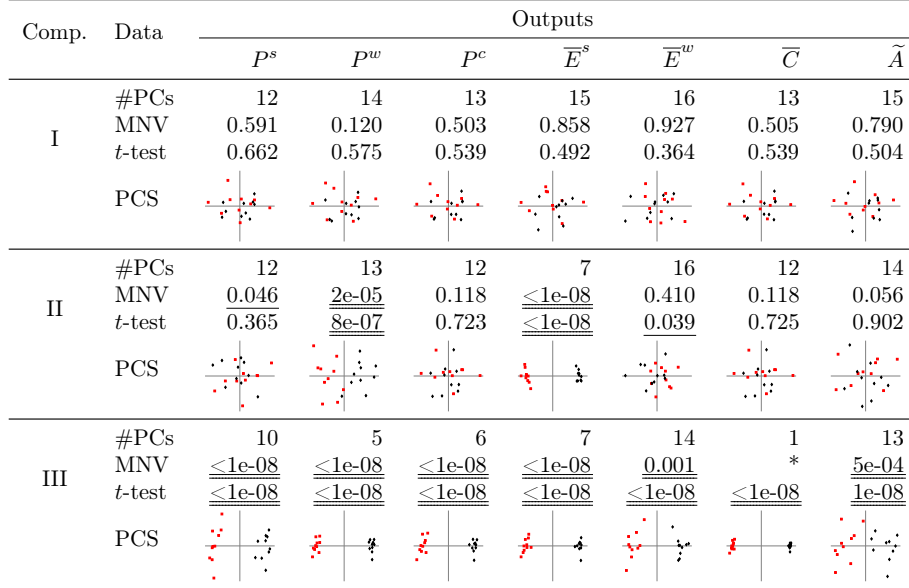 | 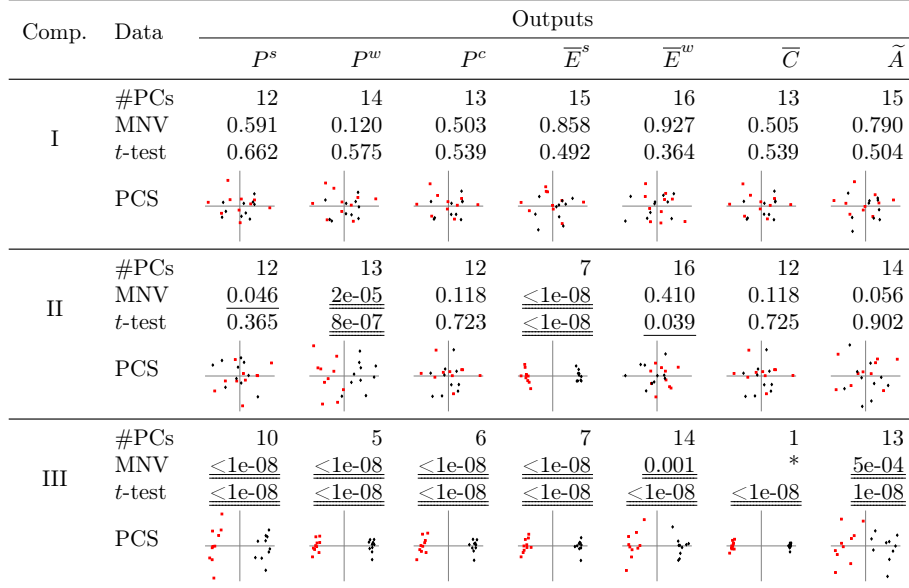 | 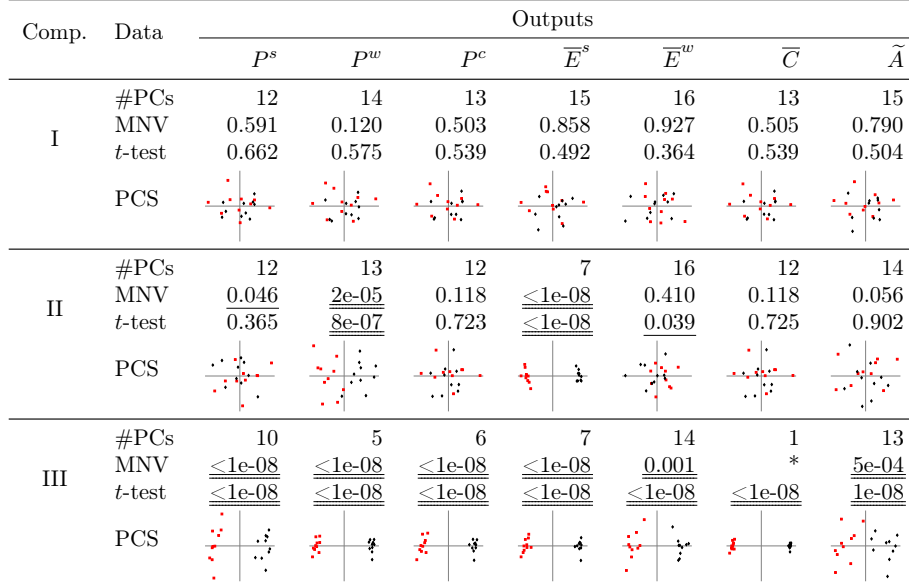 | 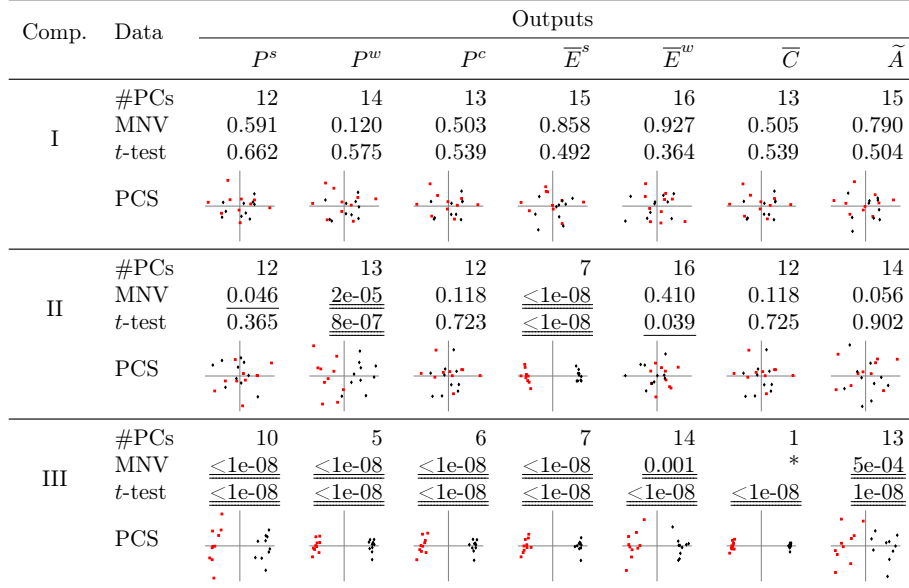 |

**Table S5.2** Results for the model-independent comparison for model size 400, parameter set 1, and  $n = 10$  runs per configuration. Case I weights two similar setups, case II compares setups with a small implementation difference, and case III compares setups with a different parameter. #PCs is the number of PCs which explain at least 90% of variance, while MNV and  $t$ -test refer to the  $p$ -value yielded by the MANOVA (#PCs) and  $t$  (first PC) statistical tests, respectively. PCS shows the representation of the respective output in the first two dimensions of the PC space. Output  $\tilde{A}$  refers to the concatenation of all outputs (range scaled). Values lower than 0.05 are underlined, while values lower than 0.01 are double-underlined. The MANOVA test is not applicable to one PC, and the respective  $p$ -values are replace with an asterisk (\*).

| Comp. | Stat.          | Outputs          |                  |                  |                  |                  |                  |
|-------|----------------|------------------|------------------|------------------|------------------|------------------|------------------|
|       |                | $P^s$            | $P^w$            | $P^c$            | $\bar{E}^s$      | $\bar{E}^w$      | $\bar{C}$        |
| I     | max            | 0.289            | 0.085            | 0.093            | 0.249            | 0.205            | 0.595            |
|       | arg max        | <u>0.024</u>     | 0.159            | <u>0.018</u>     | 0.090            | 0.779            | 0.535            |
|       | min            | 0.991            | 0.406            | 0.679            | 0.622            | 0.918            | 0.264            |
|       | arg min        | 0.152            | 0.445            | 0.177            | 1.000            | <u>0.005</u>     | 0.158            |
|       | $\bar{X}^{ss}$ | 0.547            | 0.052            | 0.491            | 0.080            | 0.209            | 0.481            |
|       | $S^{ss}$       | 0.259            | 0.100            | 0.228            | 0.973            | 0.467            | 0.228            |
| II    | max            | <u>&lt; 1e-8</u> | <u>&lt; 1e-8</u> | <u>&lt; 1e-8</u> | <u>&lt; 1e-8</u> | 0.042            | <u>3e-7</u>      |
|       | arg max        | <u>&lt; 1e-8</u> | 0.143            | 0.078            | <u>3e-4</u>      | 0.155            | <u>&lt; 1e-8</u> |
|       | min            | <u>&lt; 1e-8</u> | <u>&lt; 1e-8</u> | <u>9e-7</u>      | 0.225            | 0.056            | <u>&lt; 1e-8</u> |
|       | arg min        | 0.324            | 0.225            | <u>&lt; 1e-8</u> | 1.000            | 0.136            | 0.158            |
|       | $\bar{X}^{ss}$ | <u>3e-5</u>      | <u>&lt; 1e-8</u> | <u>&lt; 1e-8</u> | <u>&lt; 1e-8</u> | 0.034            | <u>&lt; 1e-8</u> |
|       | $S^{ss}$       | 0.082            | 0.097            | 0.136            | <u>2e-4</u>      | 0.862            | 0.138            |
| III   | max            | <u>&lt; 1e-8</u> | <u>&lt; 1e-8</u> | <u>&lt; 1e-8</u> | <u>&lt; 1e-8</u> | <u>&lt; 1e-8</u> | <u>&lt; 1e-8</u> |
|       | arg max        | <u>&lt; 1e-8</u> | <u>5e-5</u>      | <u>&lt; 1e-8</u> | 0.015            | 0.024            | <u>&lt; 1e-8</u> |
|       | min            | <u>&lt; 1e-8</u> | <u>&lt; 1e-8</u> | <u>&lt; 1e-8</u> | 0.248            | <u>0.001</u>     | <u>&lt; 1e-8</u> |
|       | arg min        | <u>&lt; 1e-8</u> | <u>4e-7</u>      | <u>&lt; 1e-8</u> | 1.000            | <u>8e-5</u>      | <u>&lt; 1e-8</u> |
|       | $\bar{X}^{ss}$ | <u>&lt; 1e-8</u> | <u>&lt; 1e-8</u> | <u>&lt; 1e-8</u> | <u>&lt; 1e-8</u> | <u>&lt; 1e-8</u> | <u>&lt; 1e-8</u> |
|       | $S^{ss}$       | <u>&lt; 1e-8</u> | <u>&lt; 1e-8</u> | <u>&lt; 1e-8</u> | <u>&lt; 1e-8</u> | <u>&lt; 1e-8</u> | <u>2e-5</u>      |

**Table S6.1**  $P$ -values for the empirical selection of FMs for model size 400, parameter set 1, and  $n = 100$  runs per configuration.  $P$ -values were obtained with the  $t$ -test for max, min,  $\bar{X}^{ss}$  and  $S^{ss}$  statistics, and with the Mann-Whitney U test for the arg max and arg min statistics. Case I weights two similar configurations, case II compares configurations with a small implementation difference, and case III compares configurations with a different parameter. Values lower than 0.05 are underlined, while values lower than 0.01 are double-underlined.

| Comp. | Data      | Outputs                                                                           |                                                                                   |                                                                                   |                                                                                   |                                                                                    |                                                                                     |                                                                                     |
|-------|-----------|-----------------------------------------------------------------------------------|-----------------------------------------------------------------------------------|-----------------------------------------------------------------------------------|-----------------------------------------------------------------------------------|------------------------------------------------------------------------------------|-------------------------------------------------------------------------------------|-------------------------------------------------------------------------------------|
|       |           | $P^s$                                                                             | $P^w$                                                                             | $P^c$                                                                             | $\overline{E}^s$                                                                  | $\overline{E}^w$                                                                   | $\overline{C}$                                                                      | $\tilde{A}$                                                                         |
| I     | #PCs      | 35                                                                                | 56                                                                                | 36                                                                                | 72                                                                                | 108                                                                                | 38                                                                                  | 93                                                                                  |
|       | MNV       | 0.750                                                                             | 0.164                                                                             | 0.756                                                                             | <u>1e-05</u>                                                                      | 0.521                                                                              | 0.657                                                                               | <u>3e-05</u>                                                                        |
|       | $t$ -test | 0.522                                                                             | 0.528                                                                             | 0.479                                                                             | 0.164                                                                             | 0.909                                                                              | 0.479                                                                               | 0.352                                                                               |
|       | PCS       | 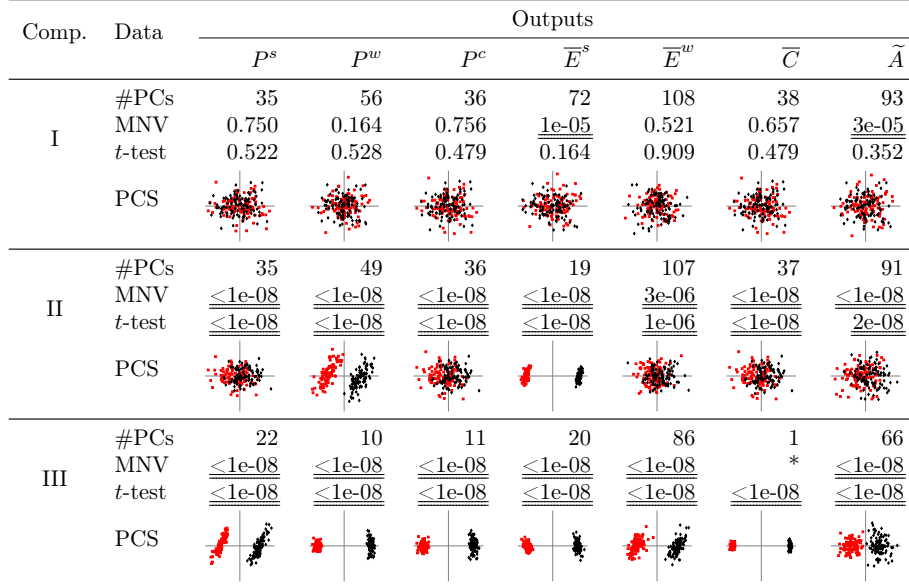 | 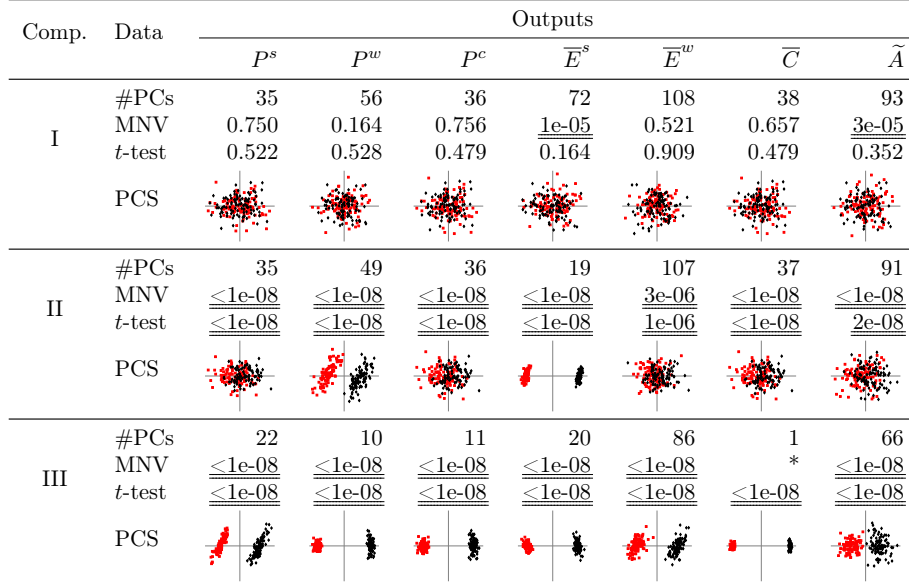 | 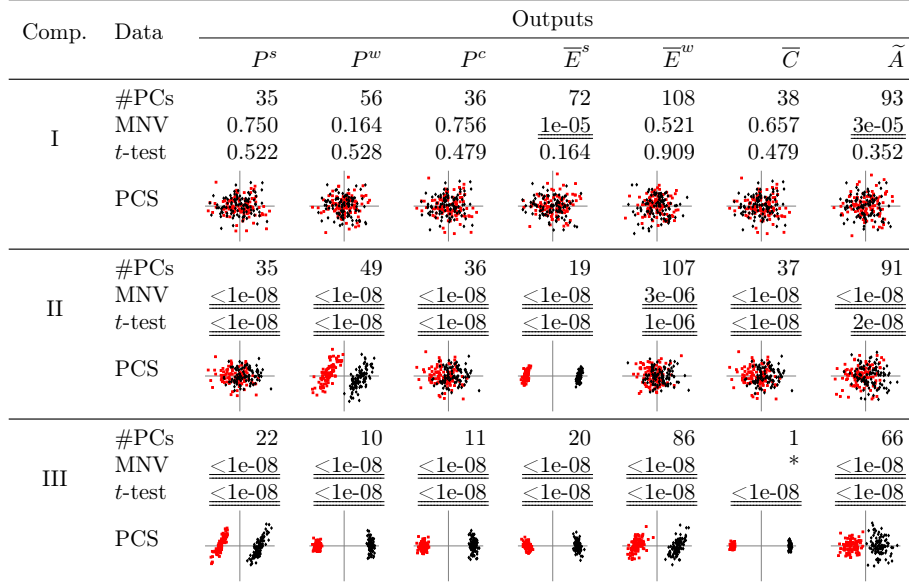 | 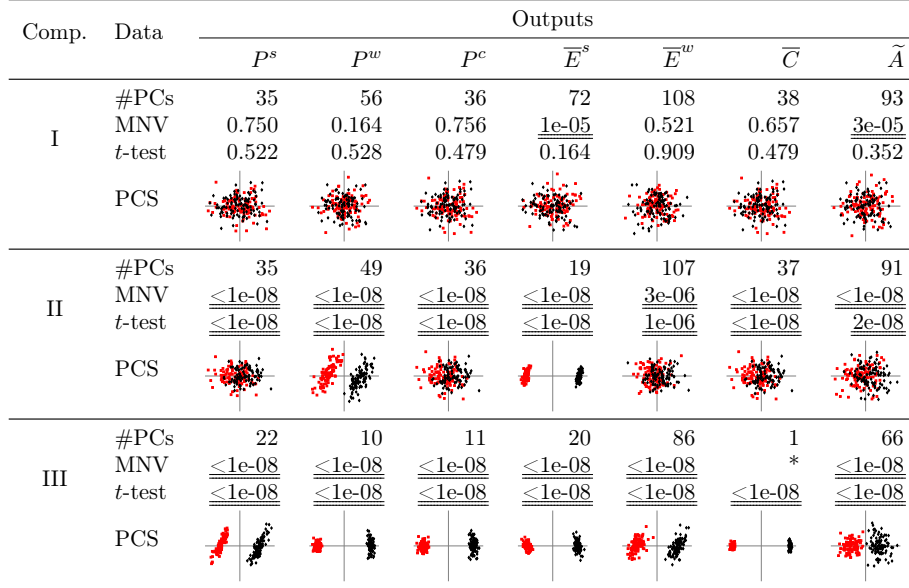 | 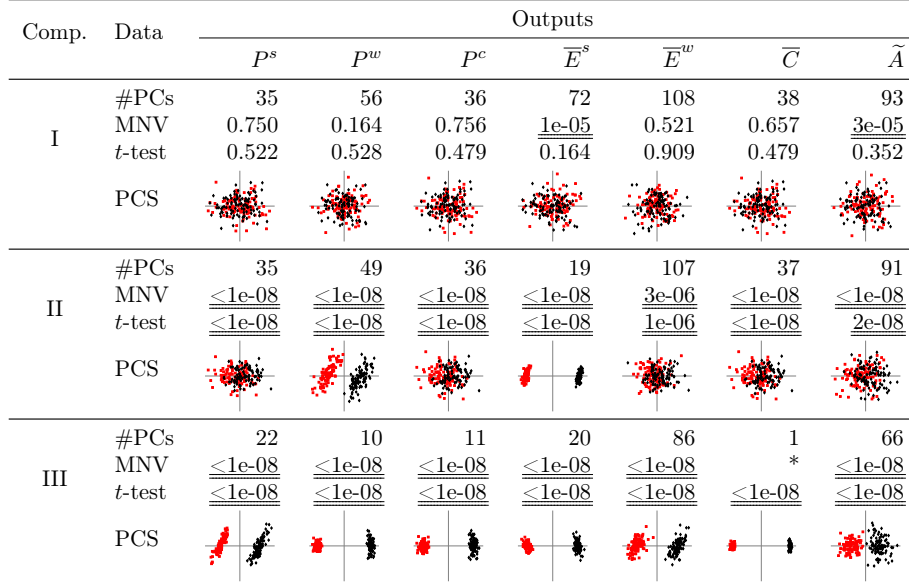 | 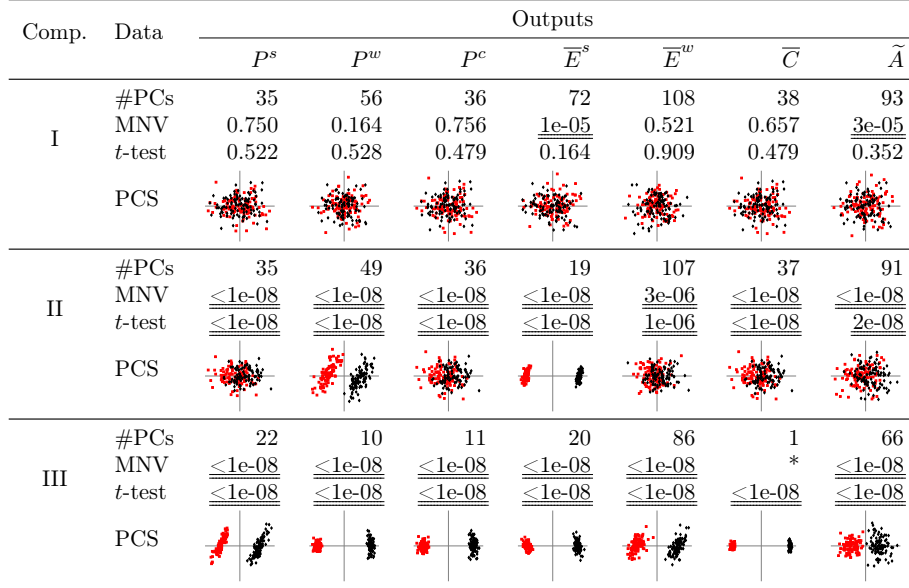 | 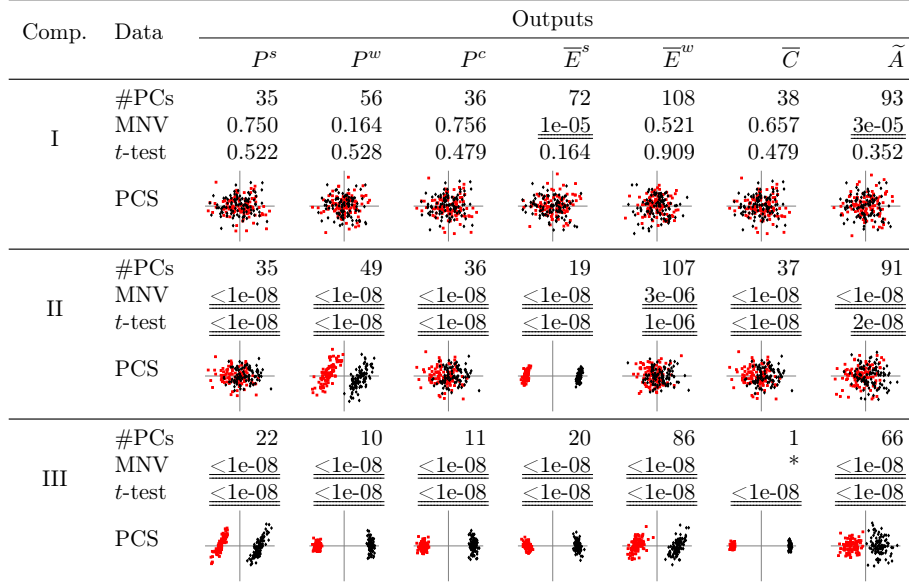 |
| II    | #PCs      | 35                                                                                | 49                                                                                | 36                                                                                | 19                                                                                | 107                                                                                | 37                                                                                  | 91                                                                                  |
|       | MNV       | <u>&lt;1e-08</u>                                                                  | <u>&lt;1e-08</u>                                                                  | <u>&lt;1e-08</u>                                                                  | <u>&lt;1e-08</u>                                                                  | <u>3e-06</u>                                                                       | <u>&lt;1e-08</u>                                                                    | <u>&lt;1e-08</u>                                                                    |
|       | $t$ -test | <u>&lt;1e-08</u>                                                                  | <u>&lt;1e-08</u>                                                                  | <u>&lt;1e-08</u>                                                                  | <u>&lt;1e-08</u>                                                                  | <u>1e-06</u>                                                                       | <u>&lt;1e-08</u>                                                                    | <u>2e-08</u>                                                                        |
|       | PCS       | 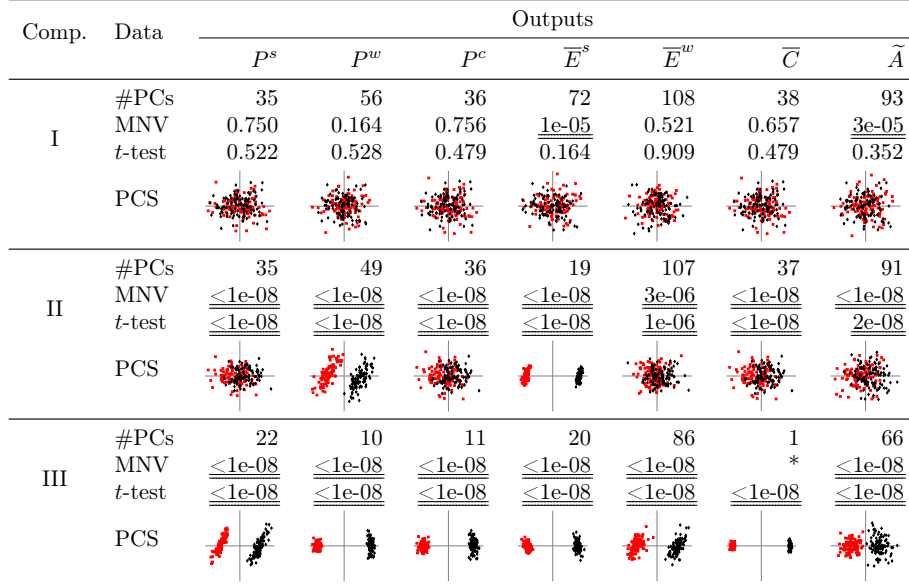 | 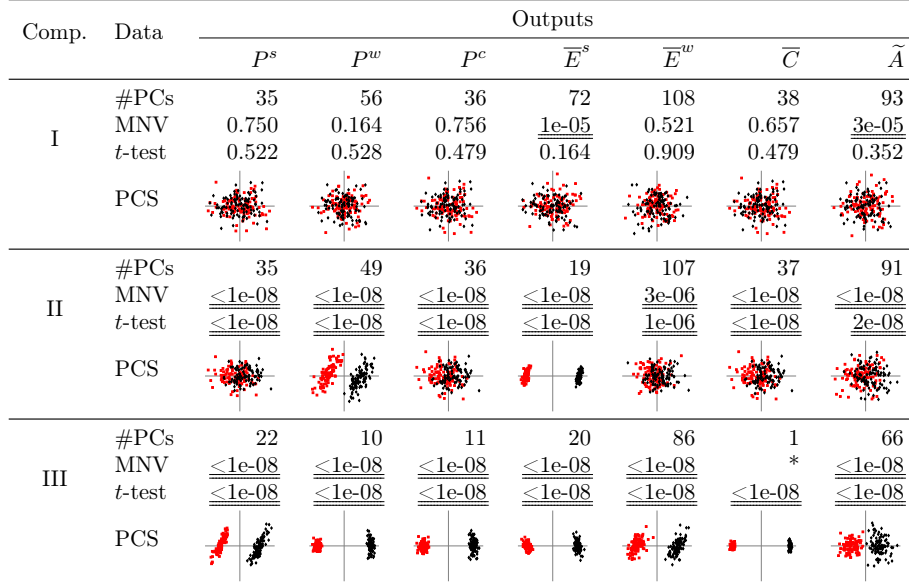 | 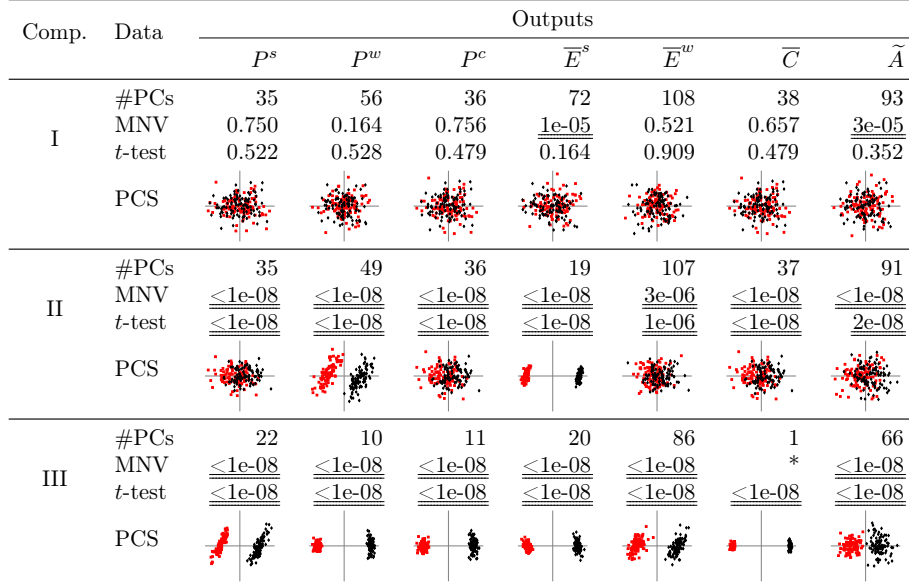 | 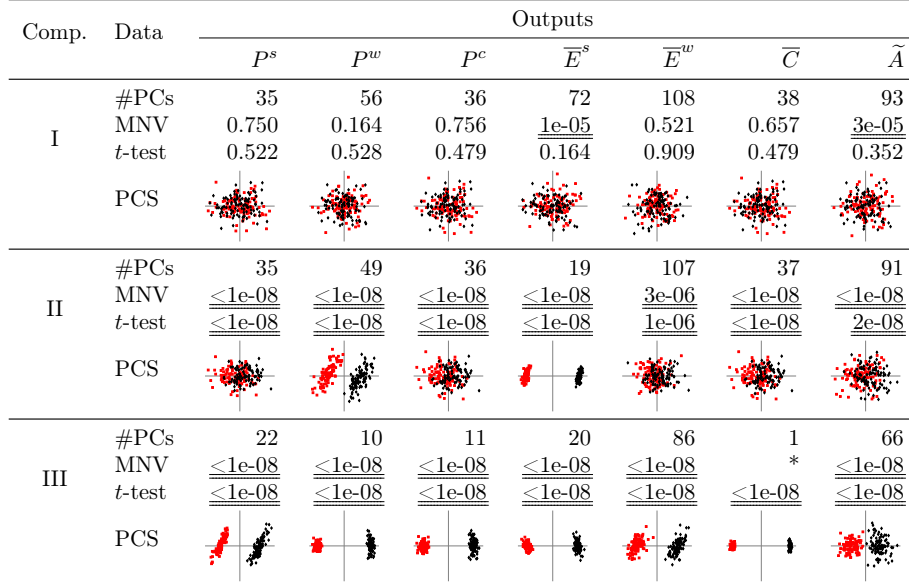 | 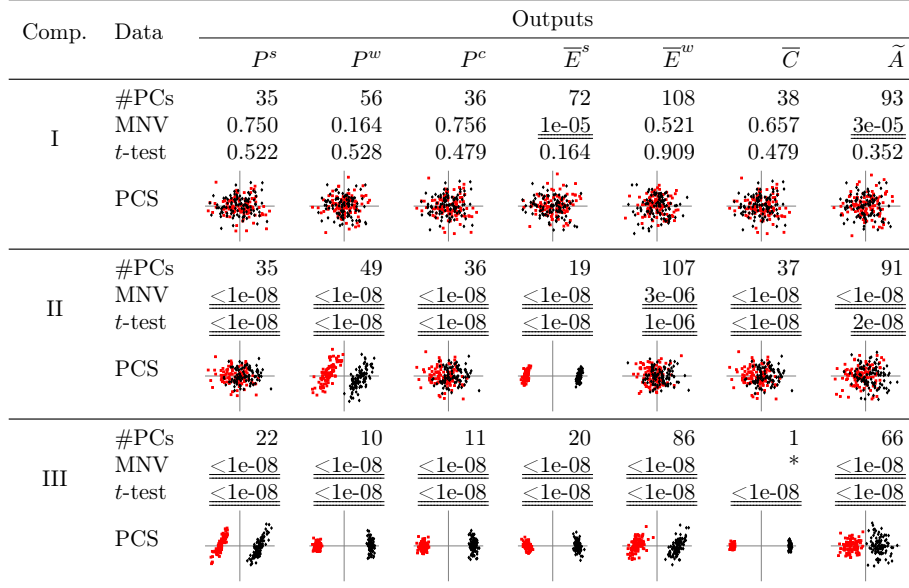 | 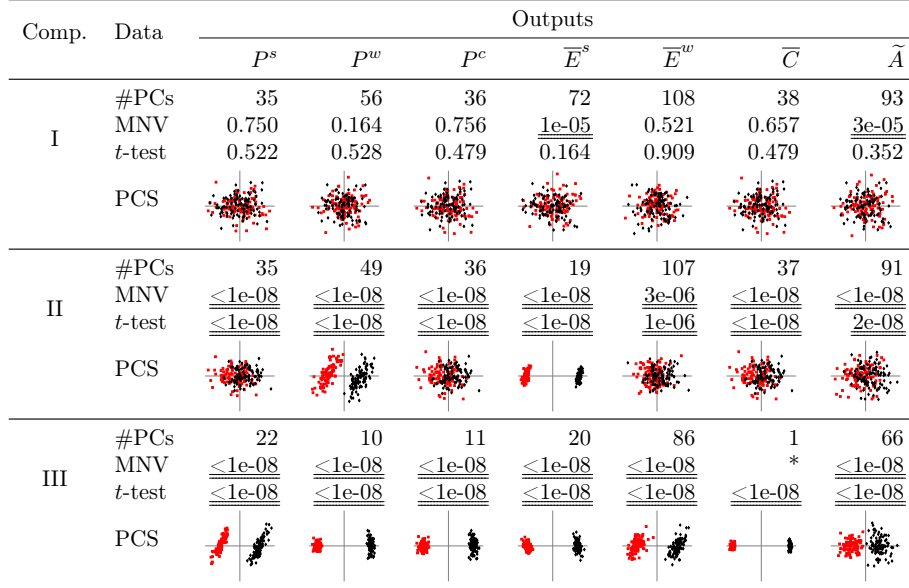 | 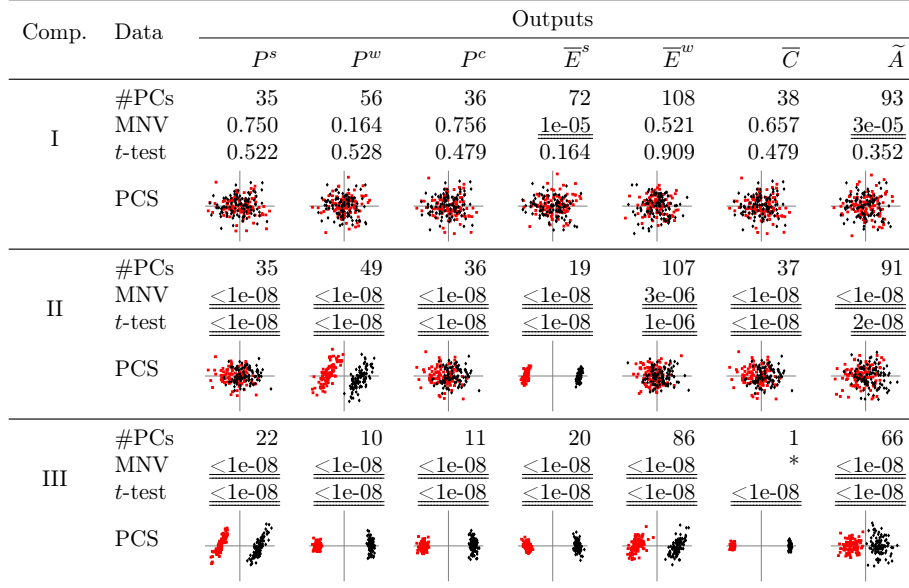 |
| III   | #PCs      | 22                                                                                | 10                                                                                | 11                                                                                | 20                                                                                | 86                                                                                 | 1                                                                                   | 66                                                                                  |
|       | MNV       | <u>&lt;1e-08</u>                                                                  | <u>&lt;1e-08</u>                                                                  | <u>&lt;1e-08</u>                                                                  | <u>&lt;1e-08</u>                                                                  | <u>&lt;1e-08</u>                                                                   | *                                                                                   | <u>&lt;1e-08</u>                                                                    |
|       | $t$ -test | <u>&lt;1e-08</u>                                                                  | <u>&lt;1e-08</u>                                                                  | <u>&lt;1e-08</u>                                                                  | <u>&lt;1e-08</u>                                                                  | <u>&lt;1e-08</u>                                                                   | <u>&lt;1e-08</u>                                                                    | <u>&lt;1e-08</u>                                                                    |
|       | PCS       | 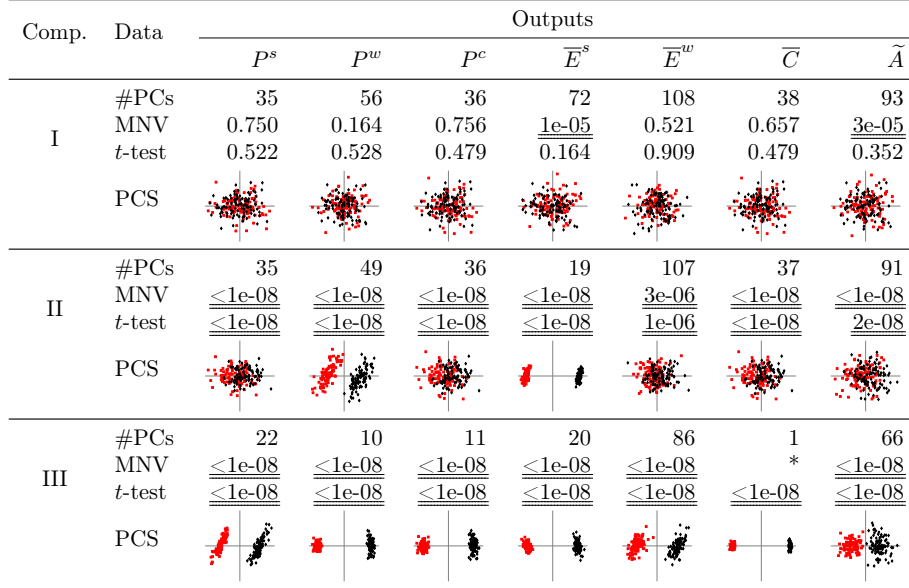 | 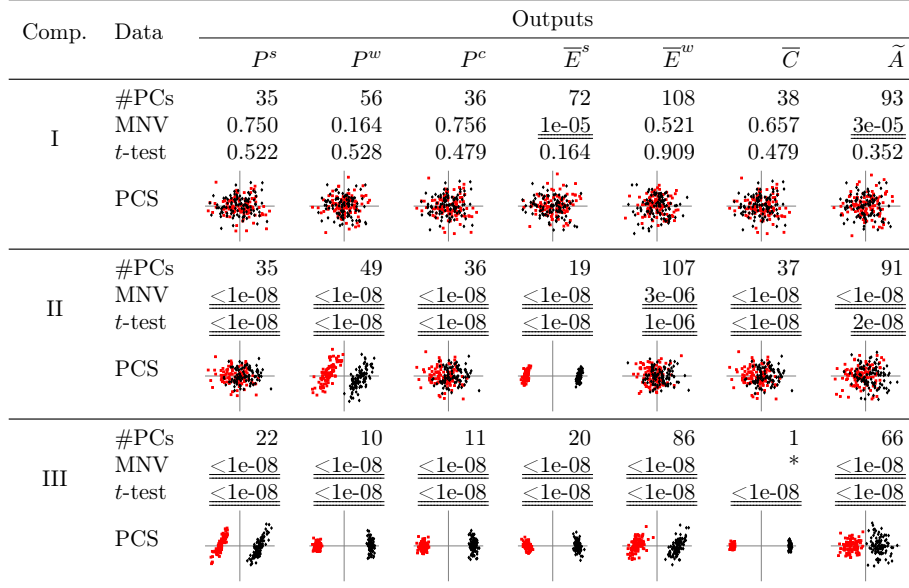 | 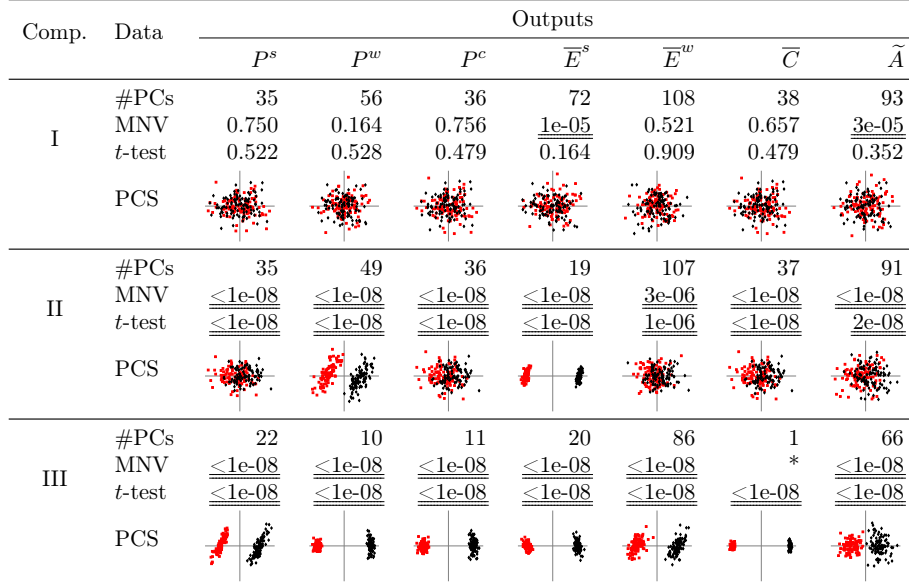 | 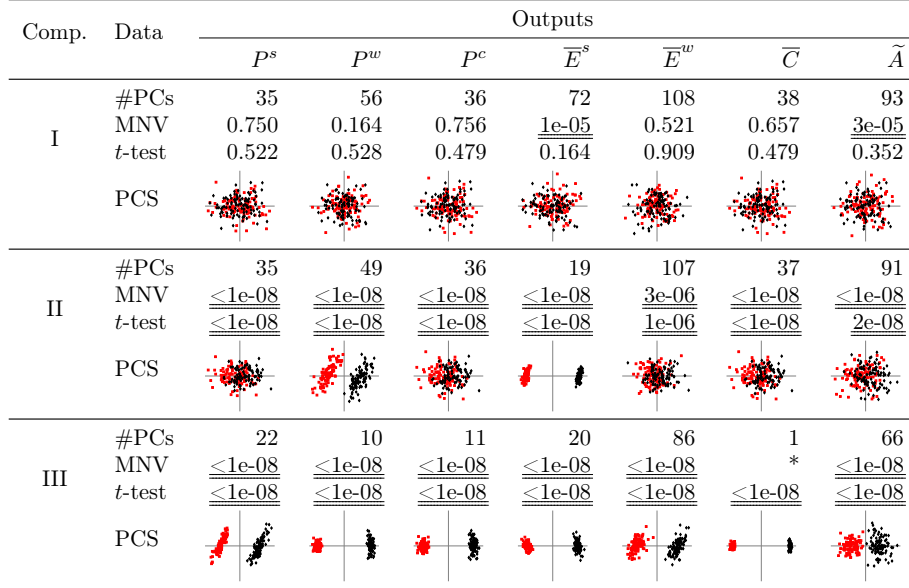 | 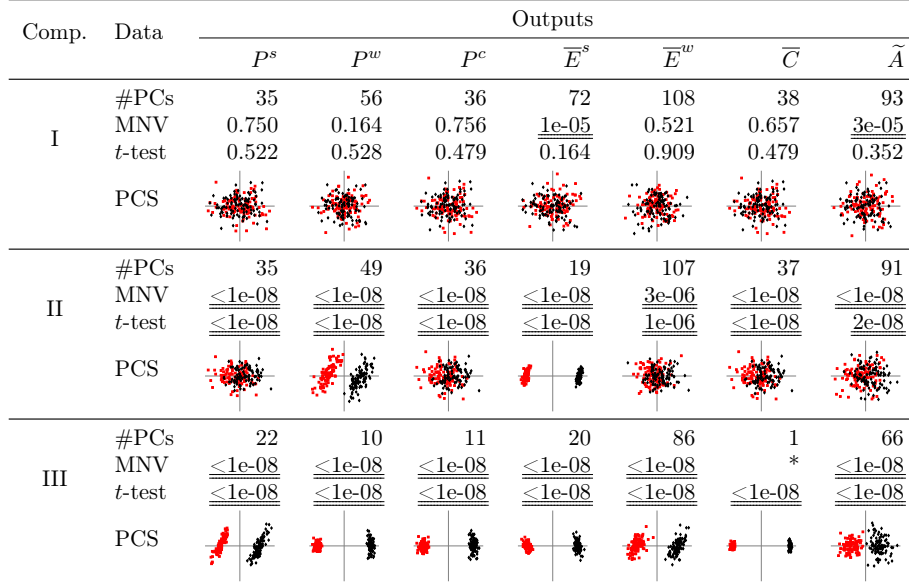 | 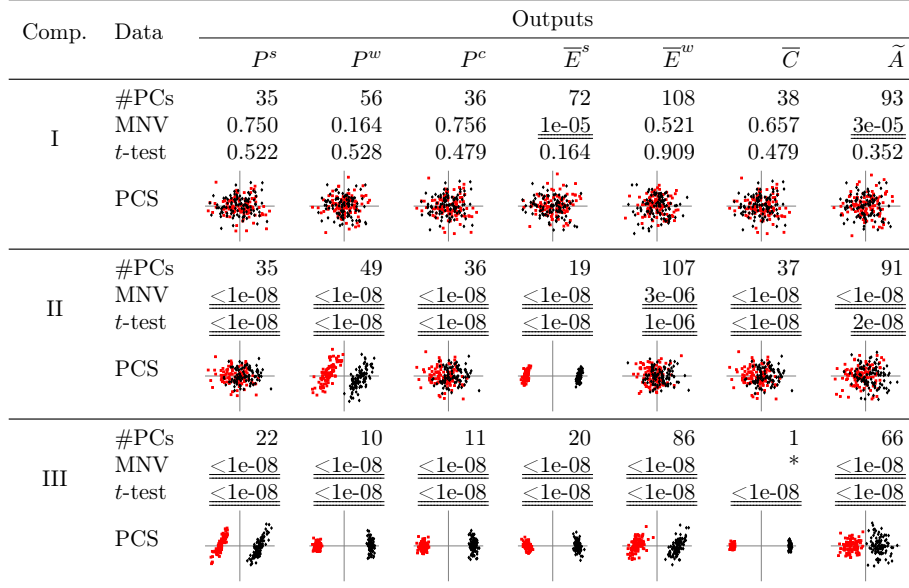 | 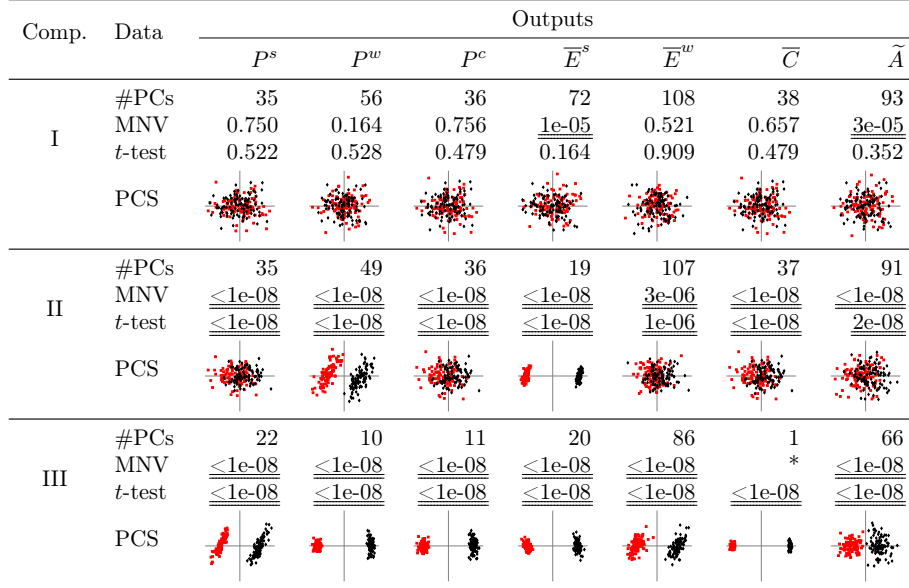 |

**Table S6.2** Results for the model-independent comparison for model size 400, parameter set 1, and  $n = 100$  runs per configuration. Case I weights two similar setups, case II compares setups with a small implementation difference, and case III compares setups with a different parameter. #PCs is the number of PCs which explain at least 90% of variance, while MNV and  $t$ -test refer to the  $p$ -value yielded by the MANOVA (#PCs) and  $t$  (first PC) statistical tests, respectively. PCS shows the representation of the respective output in the first two dimensions of the PC space. Output  $\tilde{A}$  refers to the concatenation of all outputs (range scaled). The MANOVA test is not applicable to one PC, and the respective  $p$ -values are replace with an asterisk (\*).  $P$ -values lower than 0.05 are underlined, while  $p$ -values lower than 0.01 are double-underlined.
